# Supplementary material for: Debugging Tests for Model Explanations
Source: arXiv:2011.05429 source file (2020-11-10)

# Figure 1: Framework

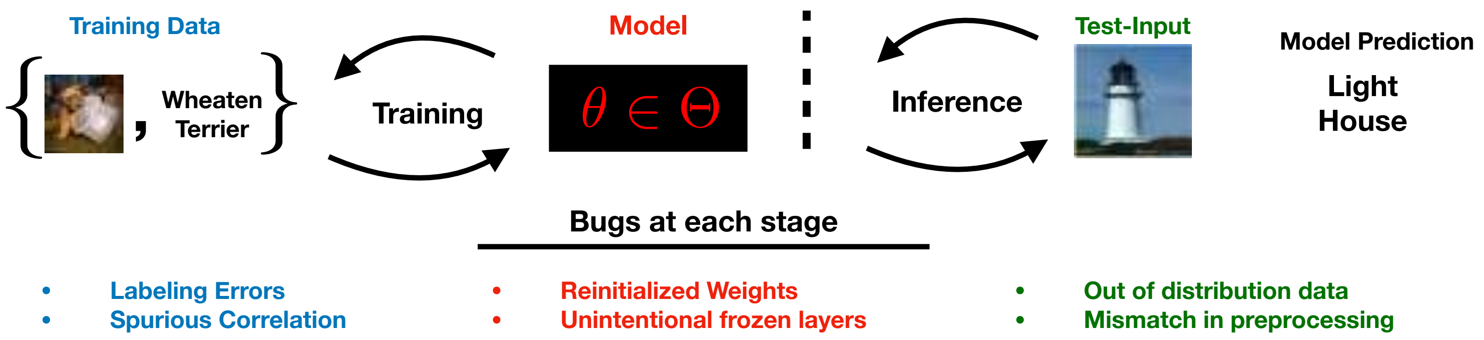

# Figure 2: Framework

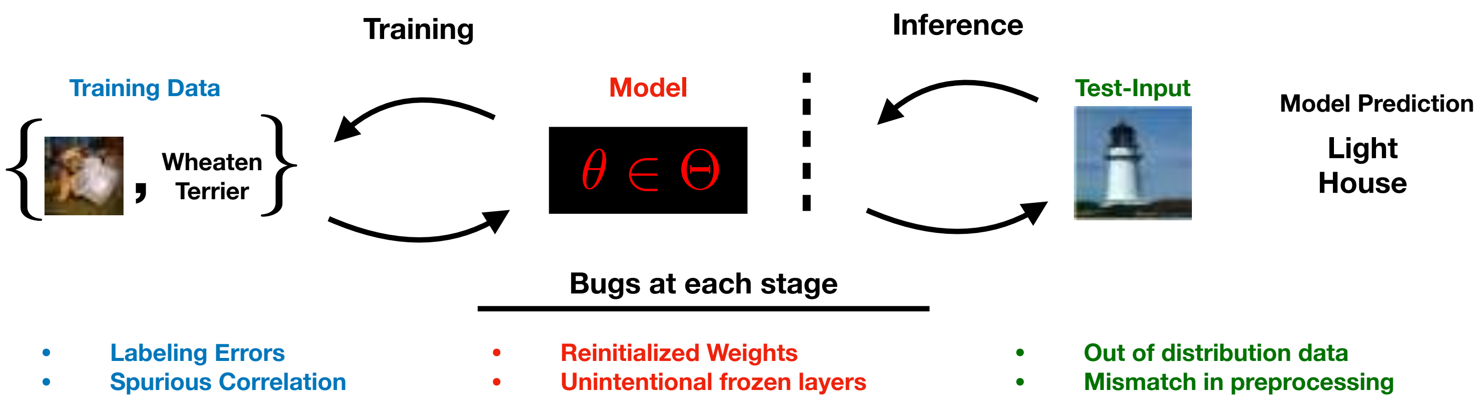

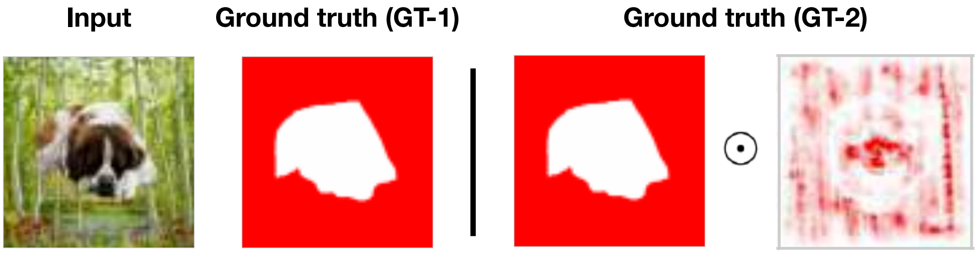
Input
Ground truth (GT-1)
Ground truth (GT-2)

# Figure 2

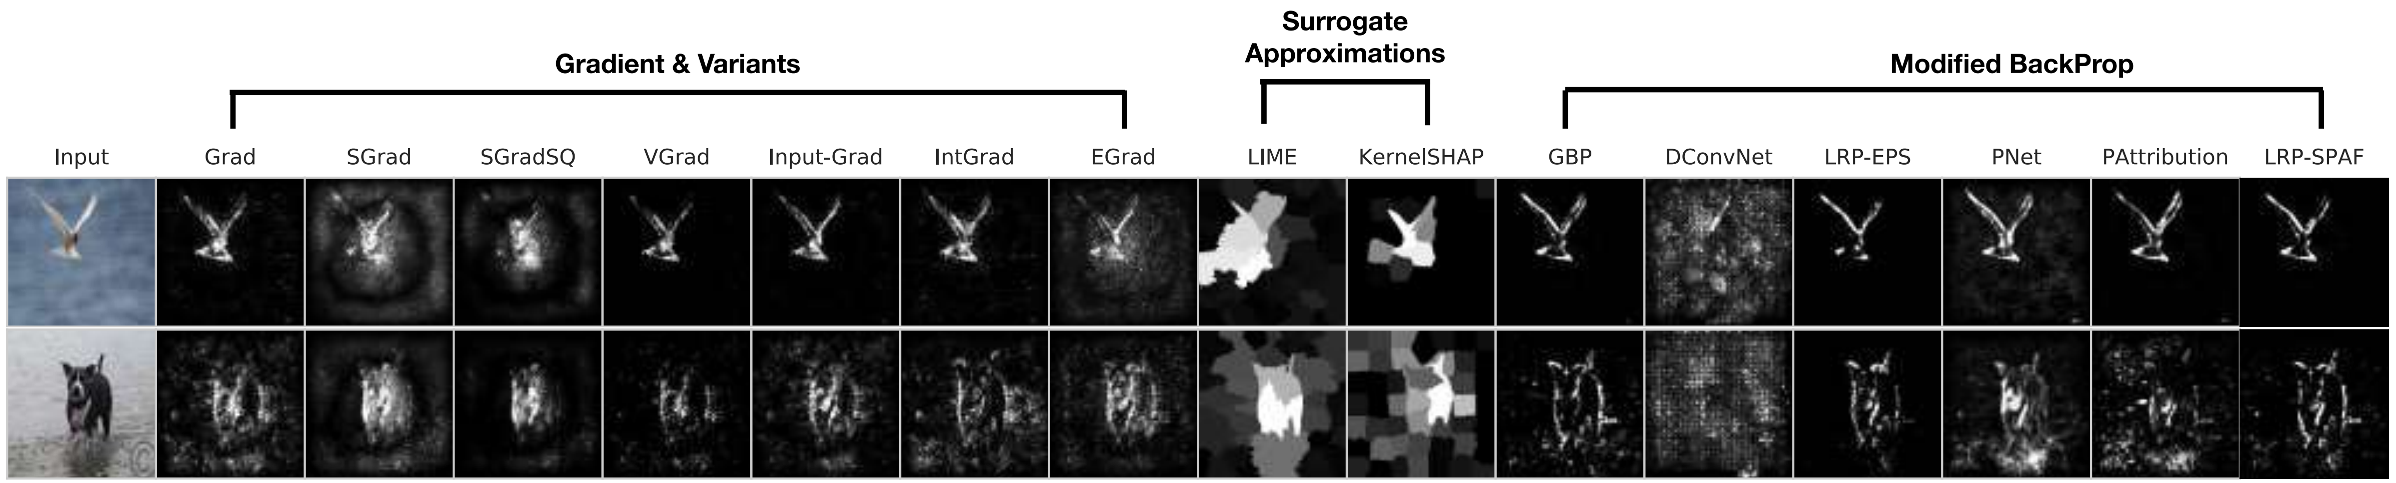
Gradient & Variants
Surrogate Approximations
Modified BackProp
Input
Grad
SGrad
SGradSQ
VGrad
Input-Grad
IntGrad
EGrad
LIME
KernelSHAP
GBP
DConvNet
LRP-EPS
PNet
PAttribution
LRP-SPAF

# Figure 2: Alternative

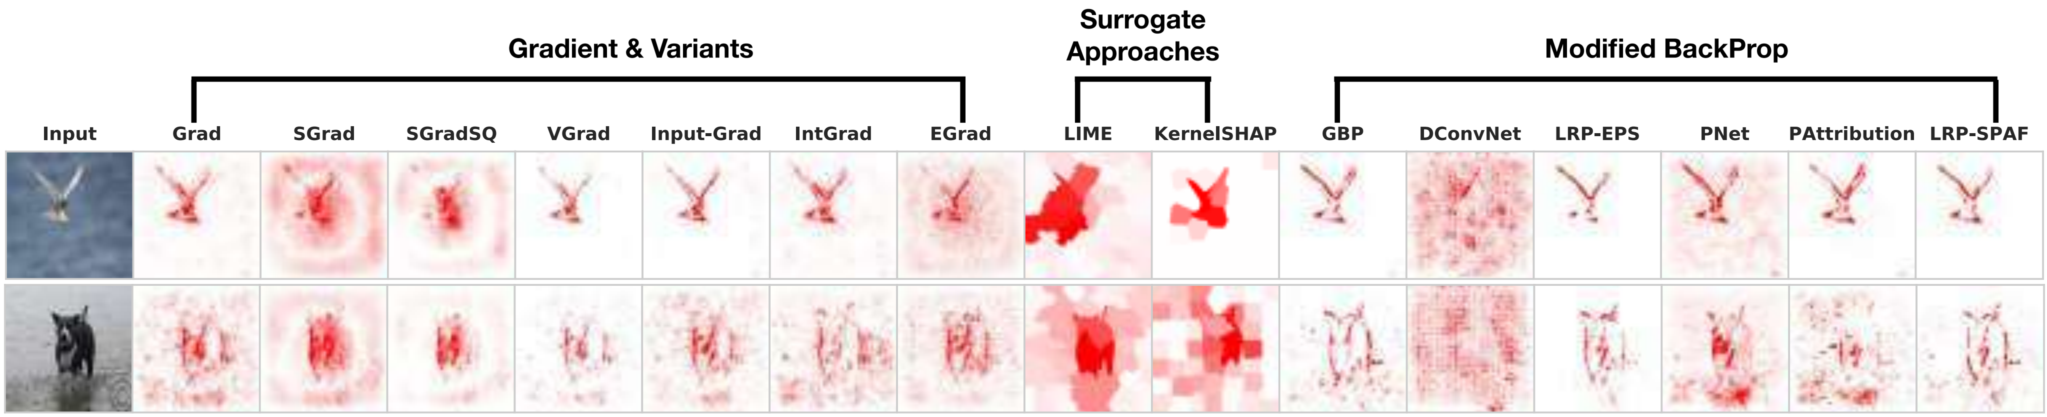

# Figure 2: Alternative

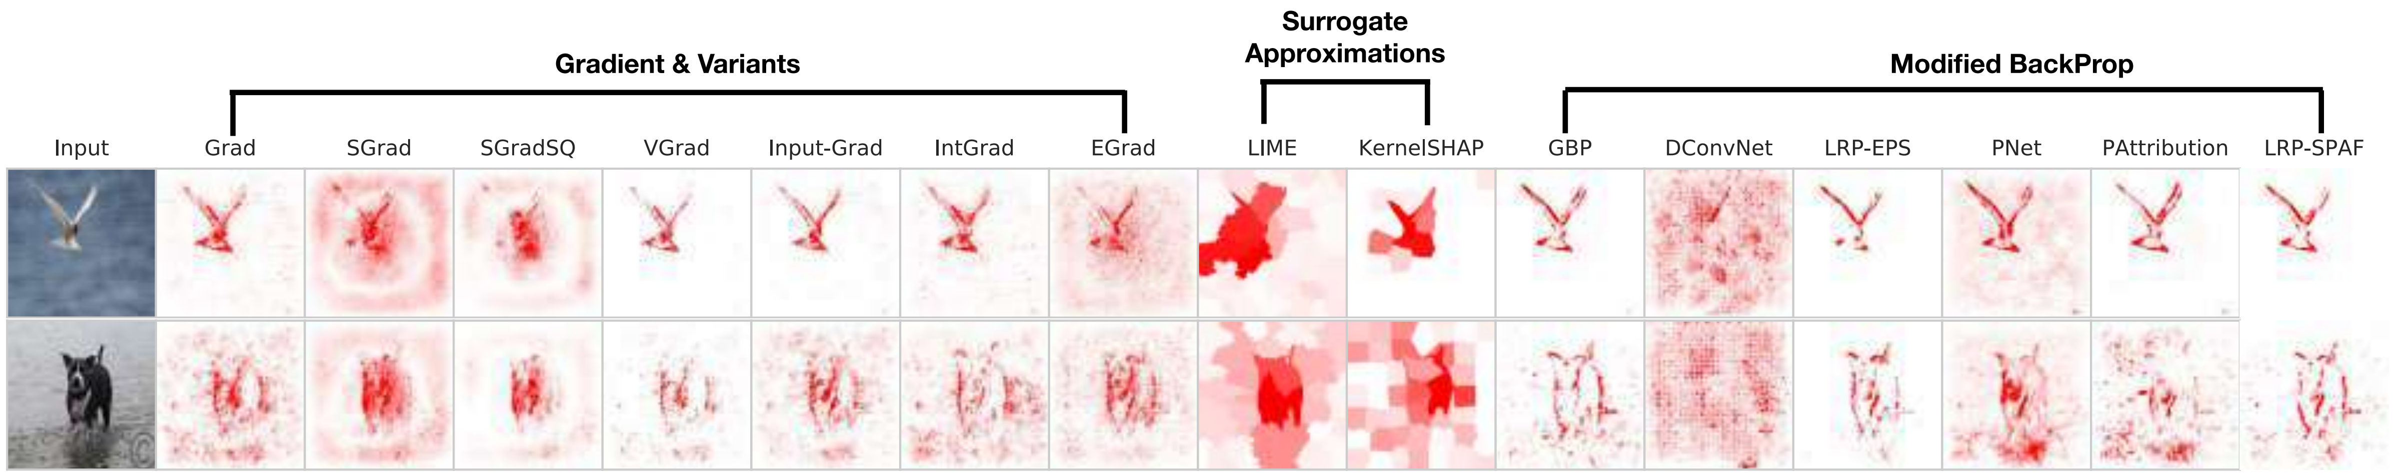

# Mislabeled Examples

# Mislabeled Examples

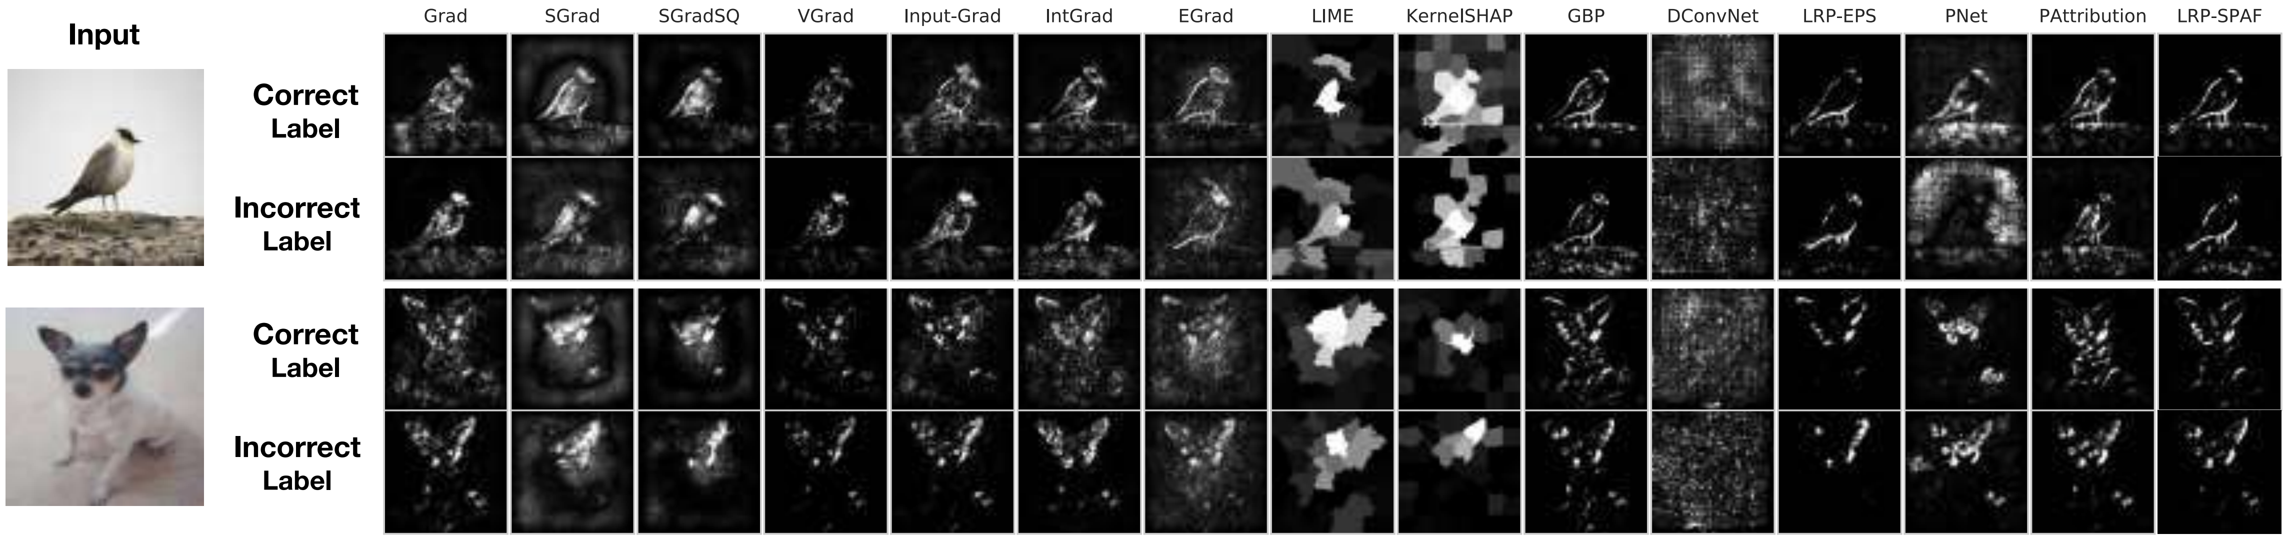

# Mislabeled Examples

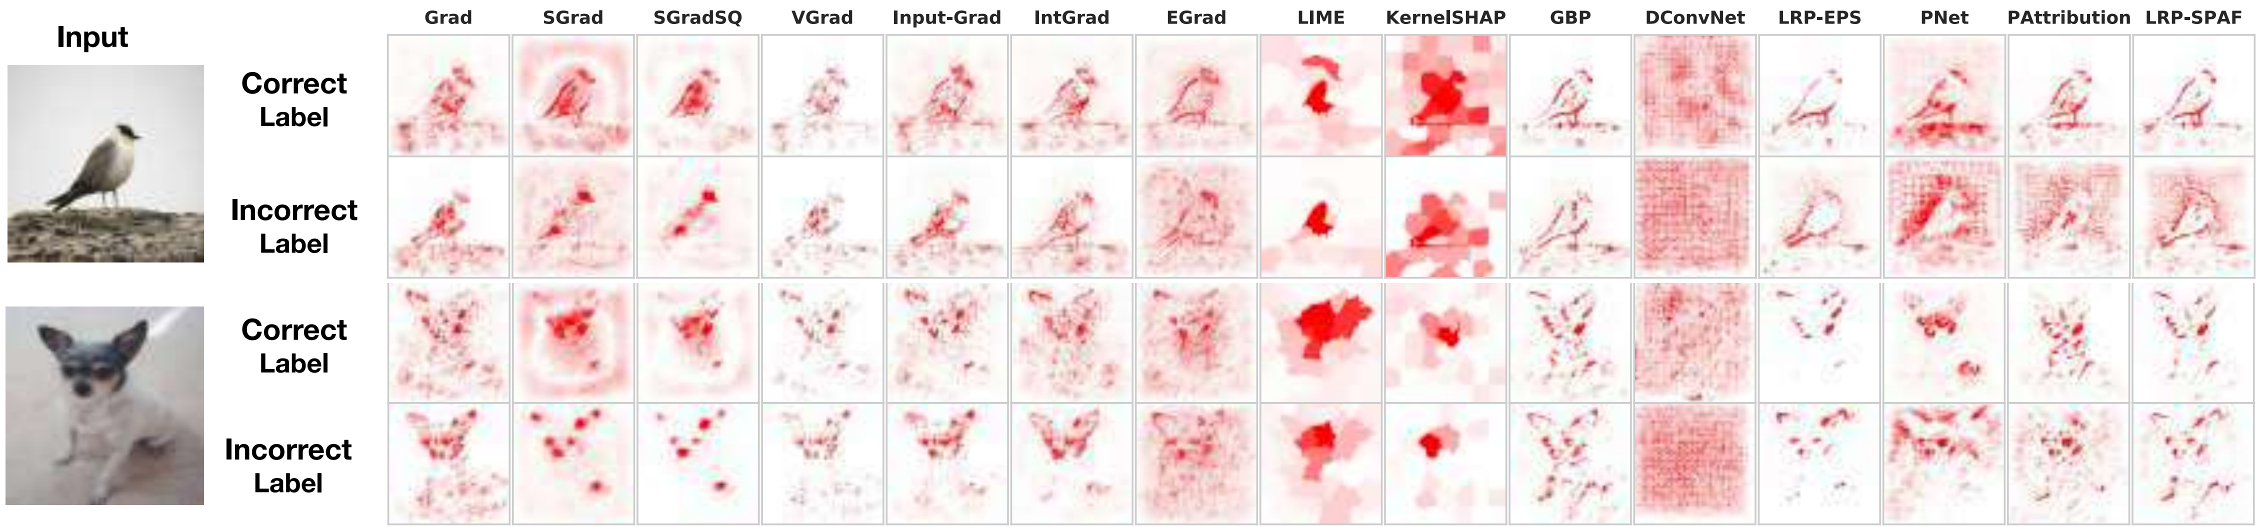

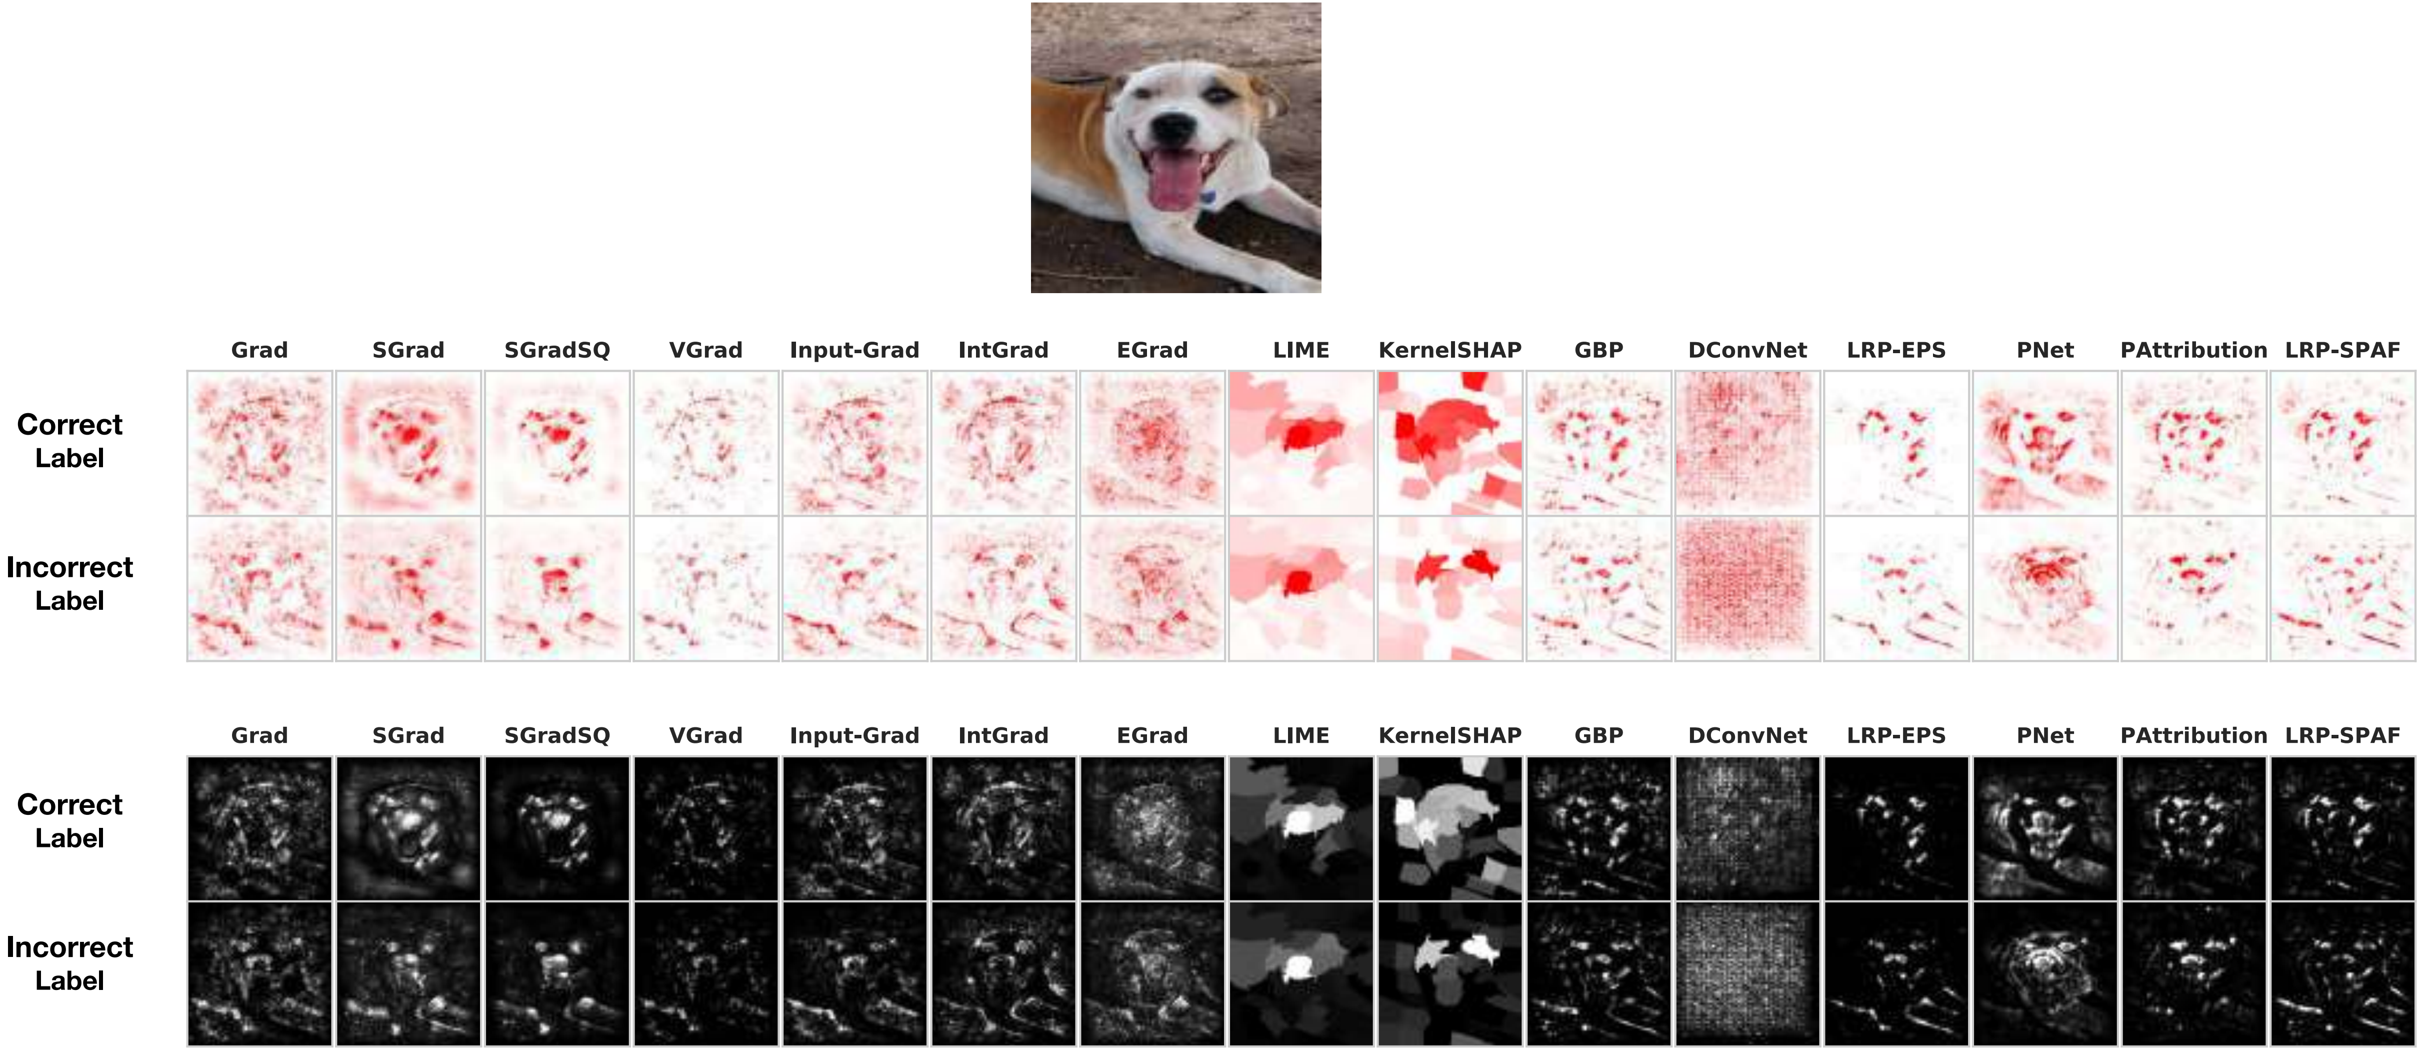
Grad
SGrad
SGradSQ
VGrad
Input-Grad
IntGrad
EGrad
LIME
KernelSHAP
GBP
DConvNet
LRP-EPS
PNet
PAttribution
LRP-SPAF
Correct Label
Incorrect Label
Grad
SGrad
SGradSQ
VGrad
Input-Grad
IntGrad
EGrad
LIME
KernelSHAP
GBP
DConvNet
LRP-EPS
PNet
PAttribution
LRP-SPAF
Correct Label
Incorrect Label

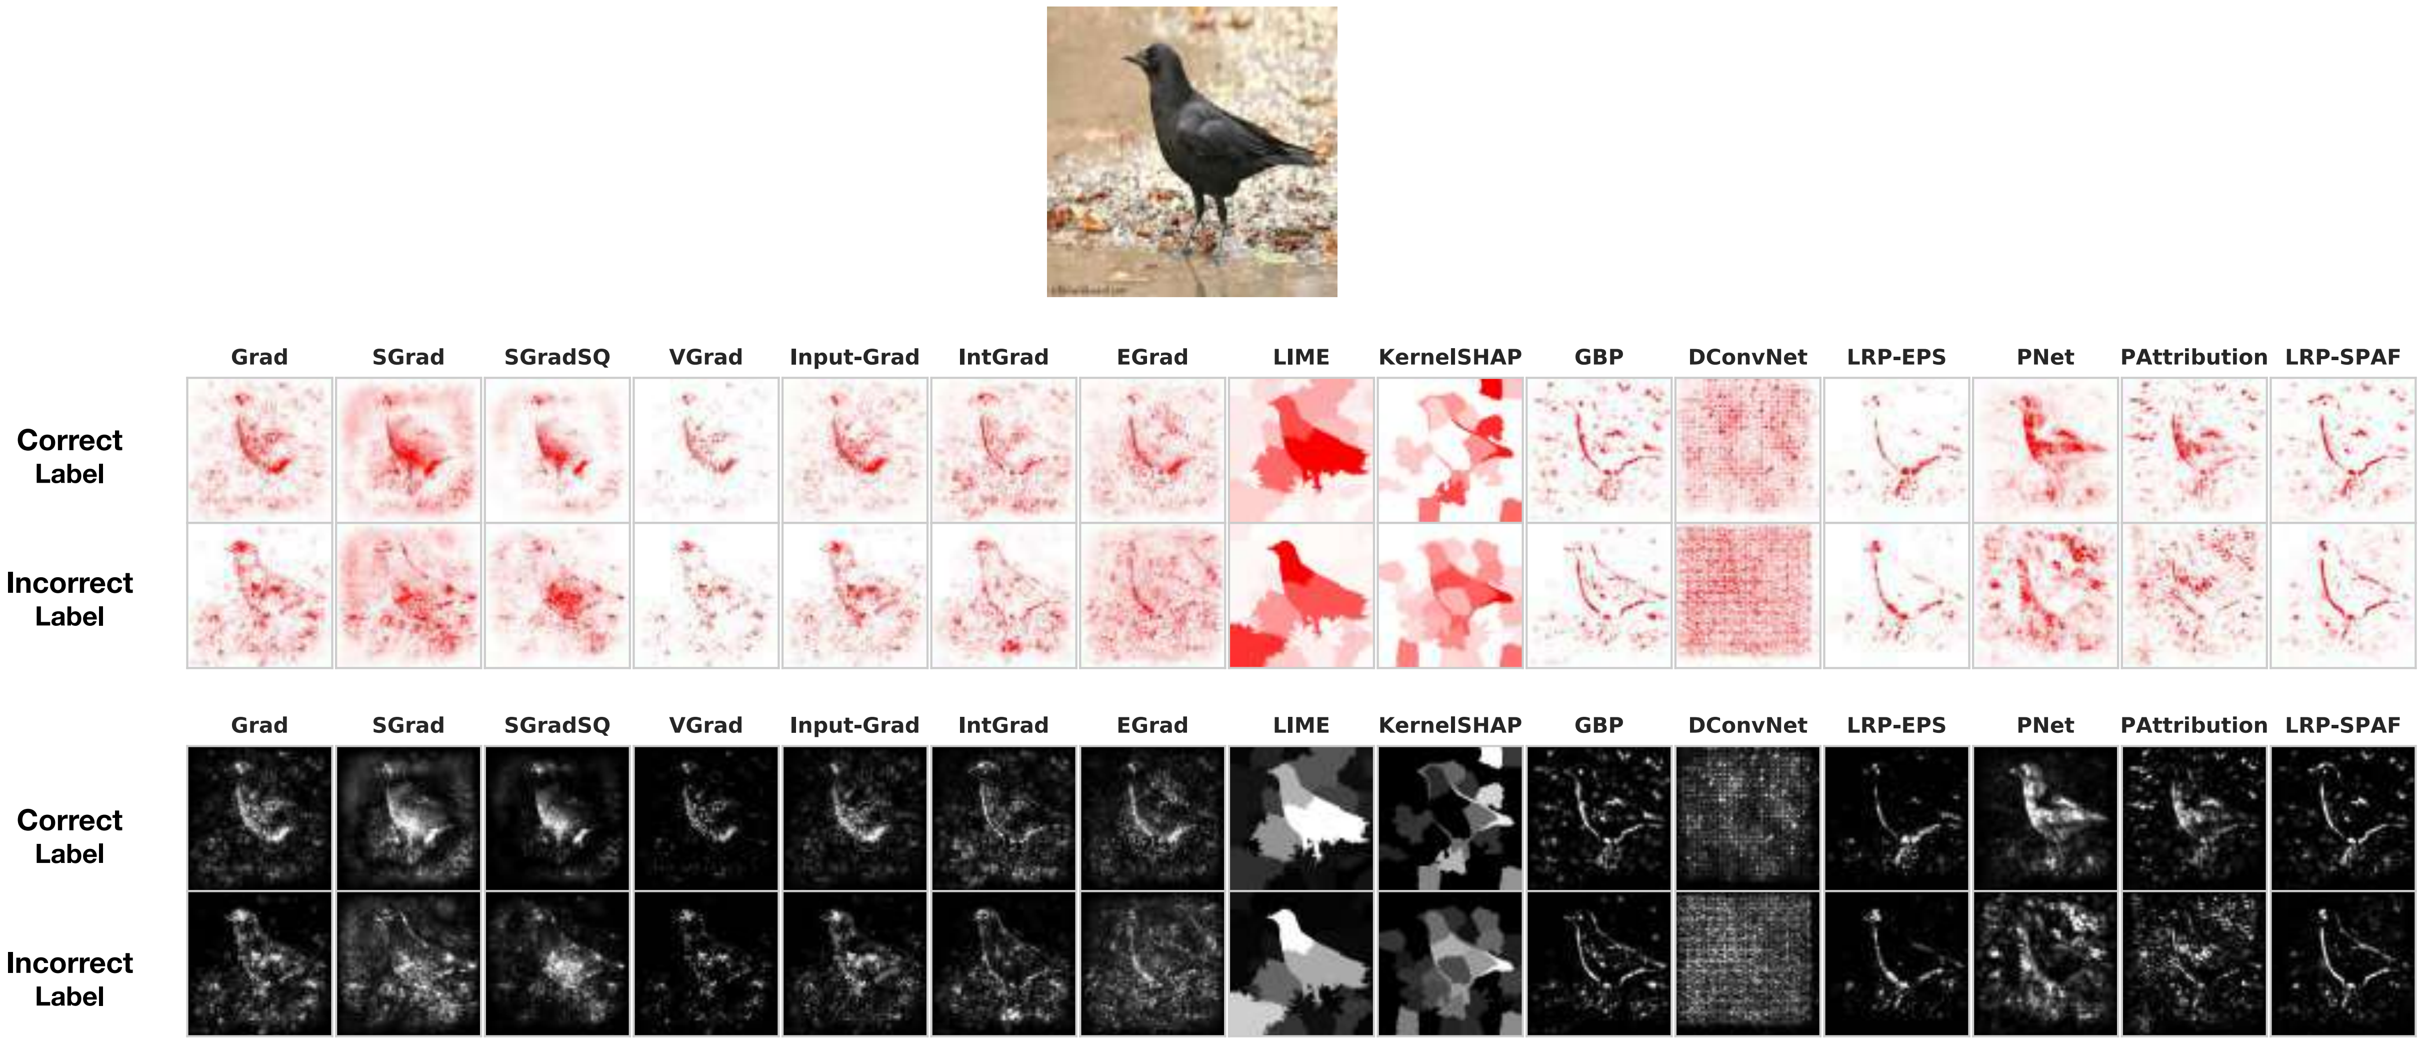
Grad
SGrad
SGradSQ
VGrad
Input-Grad
IntGrad
EGrad
LIME
KernelSHAP
GBP
DConvNet
LRP-EPS
PNet
PAttribution
LRP-SPAF
Correct Label
Incorrect Label
Grad
SGrad
SGradSQ
VGrad
Input-Grad
IntGrad
EGrad
LIME
KernelSHAP
GBP
DConvNet
LRP-EPS
PNet
PAttribution
LRP-SPAF
Correct Label
Incorrect Label

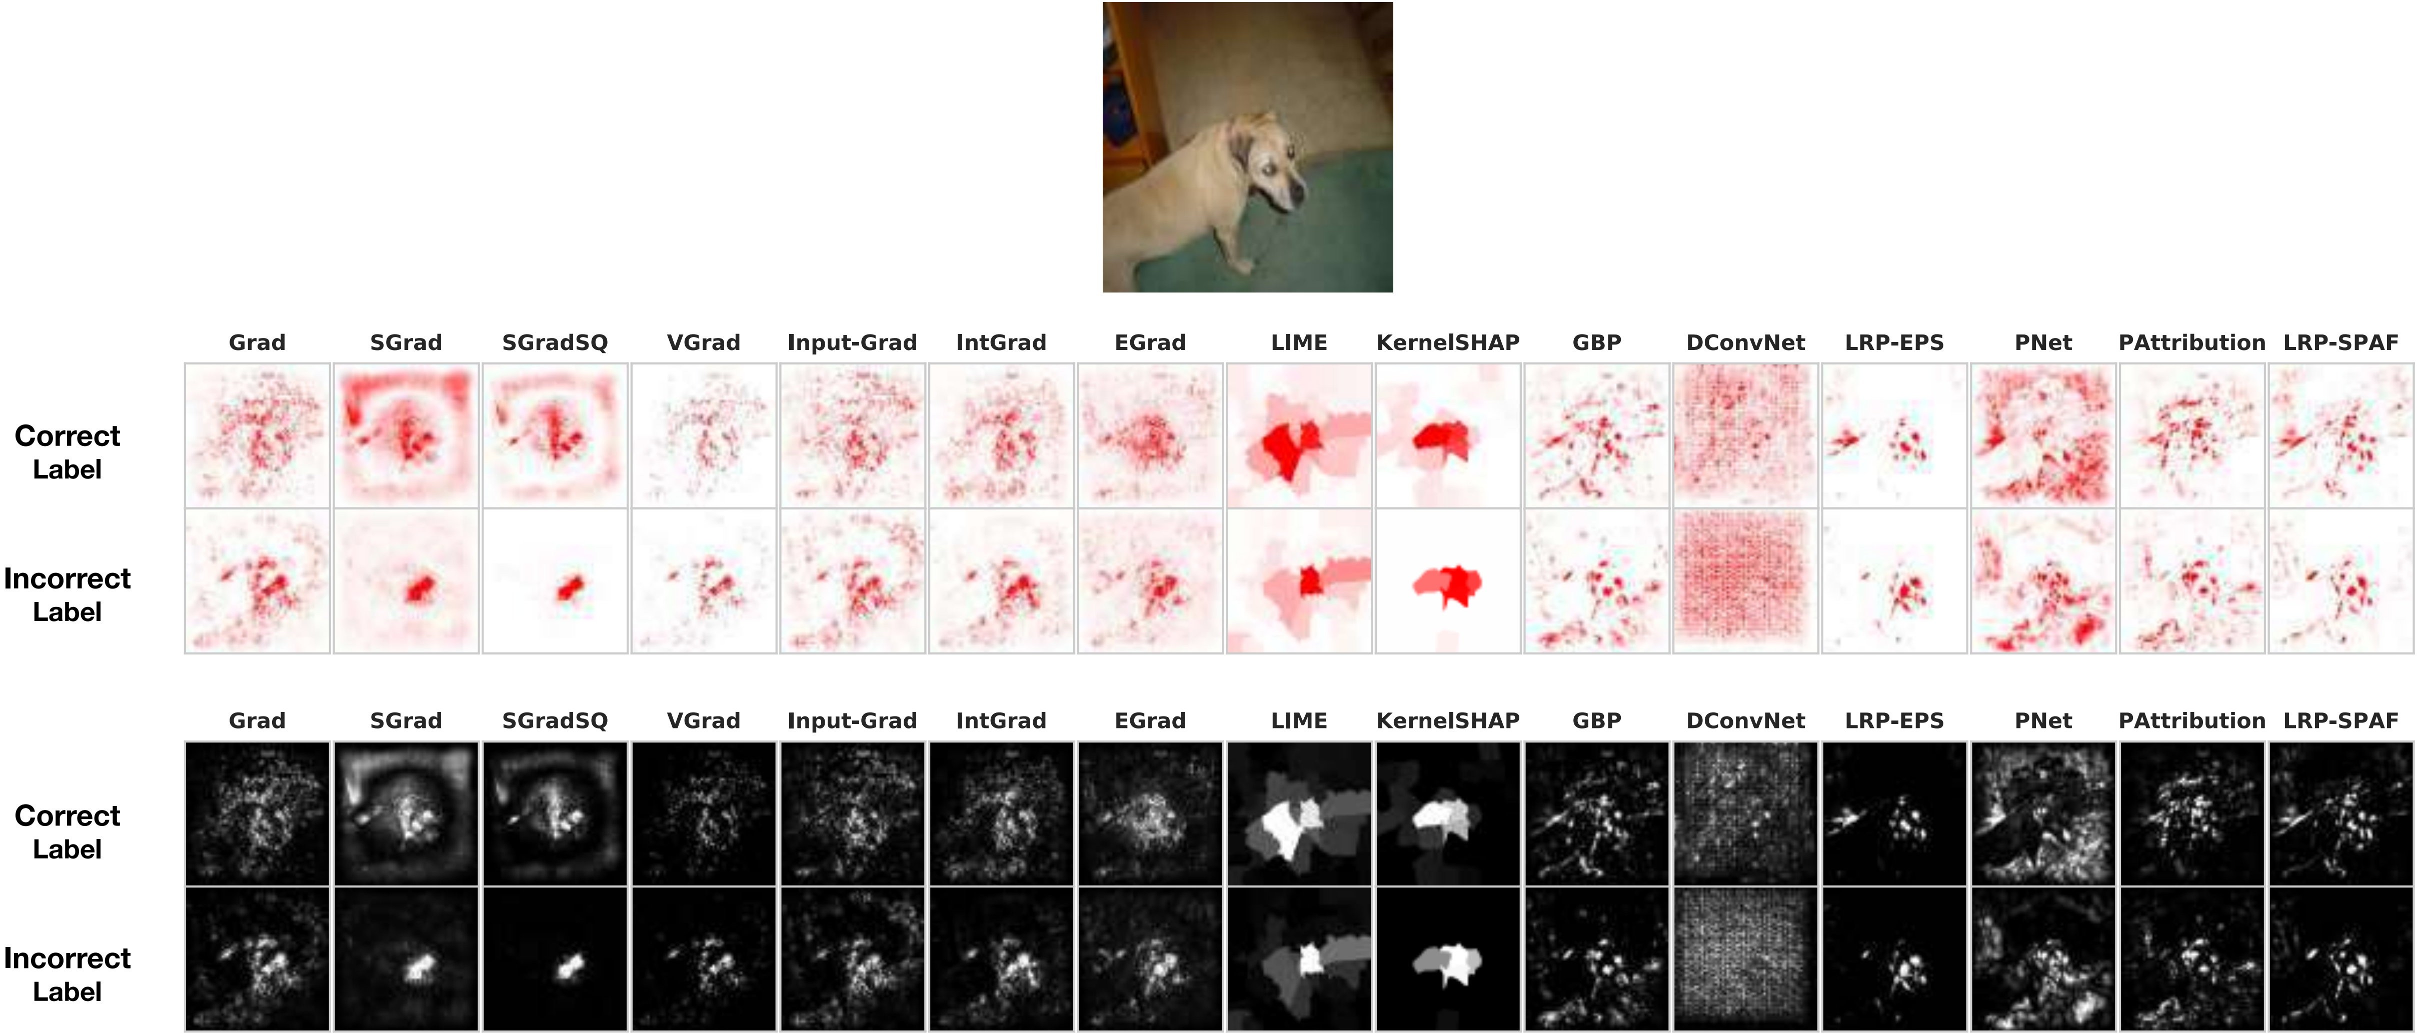
Grad
SGrad
SGradSQ
VGrad
Input-Grad
IntGrad
EGrad
LIME
KernelSHAP
GBP
DConvNet
LRP-EPS
PNet
PAttribution
LRP-SPAF
Correct Label
Incorrect Label
Grad
SGrad
SGradSQ
VGrad
Input-Grad
IntGrad
EGrad
LIME
KernelSHAP
GBP
DConvNet
LRP-EPS
PNet
PAttribution
LRP-SPAF
Correct Label
Incorrect Label

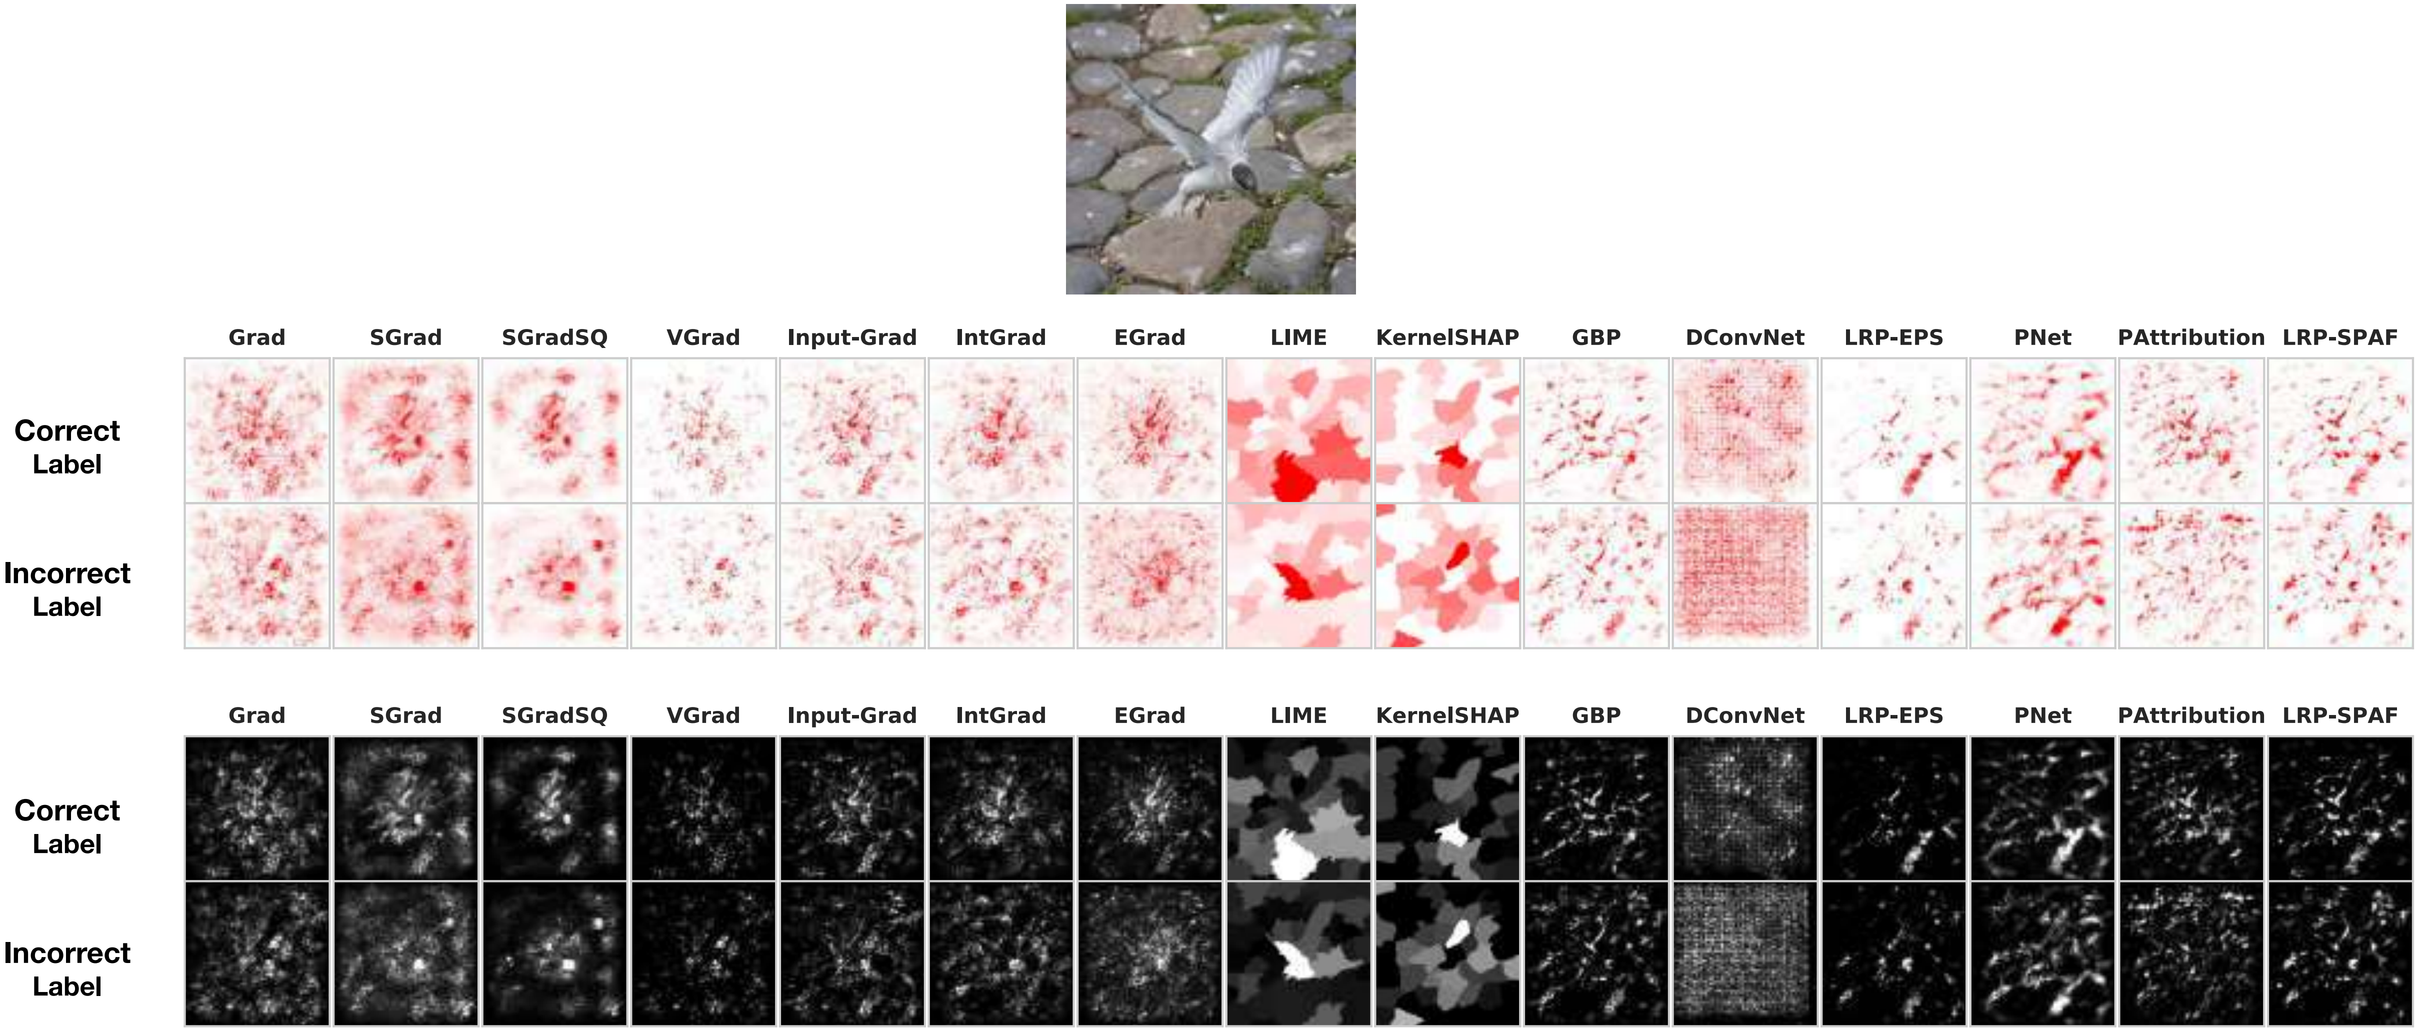
Grad
SGrad
SGradSQ
VGrad
Input-Grad
IntGrad
EGrad
LIME
KernelSHAP
GBP
DConvNet
LRP-EPS
PNet
PAttribution
LRP-SPAF
Correct Label
Incorrect Label
Grad
SGrad
SGradSQ
VGrad
Input-Grad
IntGrad
EGrad
LIME
KernelSHAP
GBP
DConvNet
LRP-EPS
PNet
PAttribution
LRP-SPAF
Correct Label
Incorrect Label

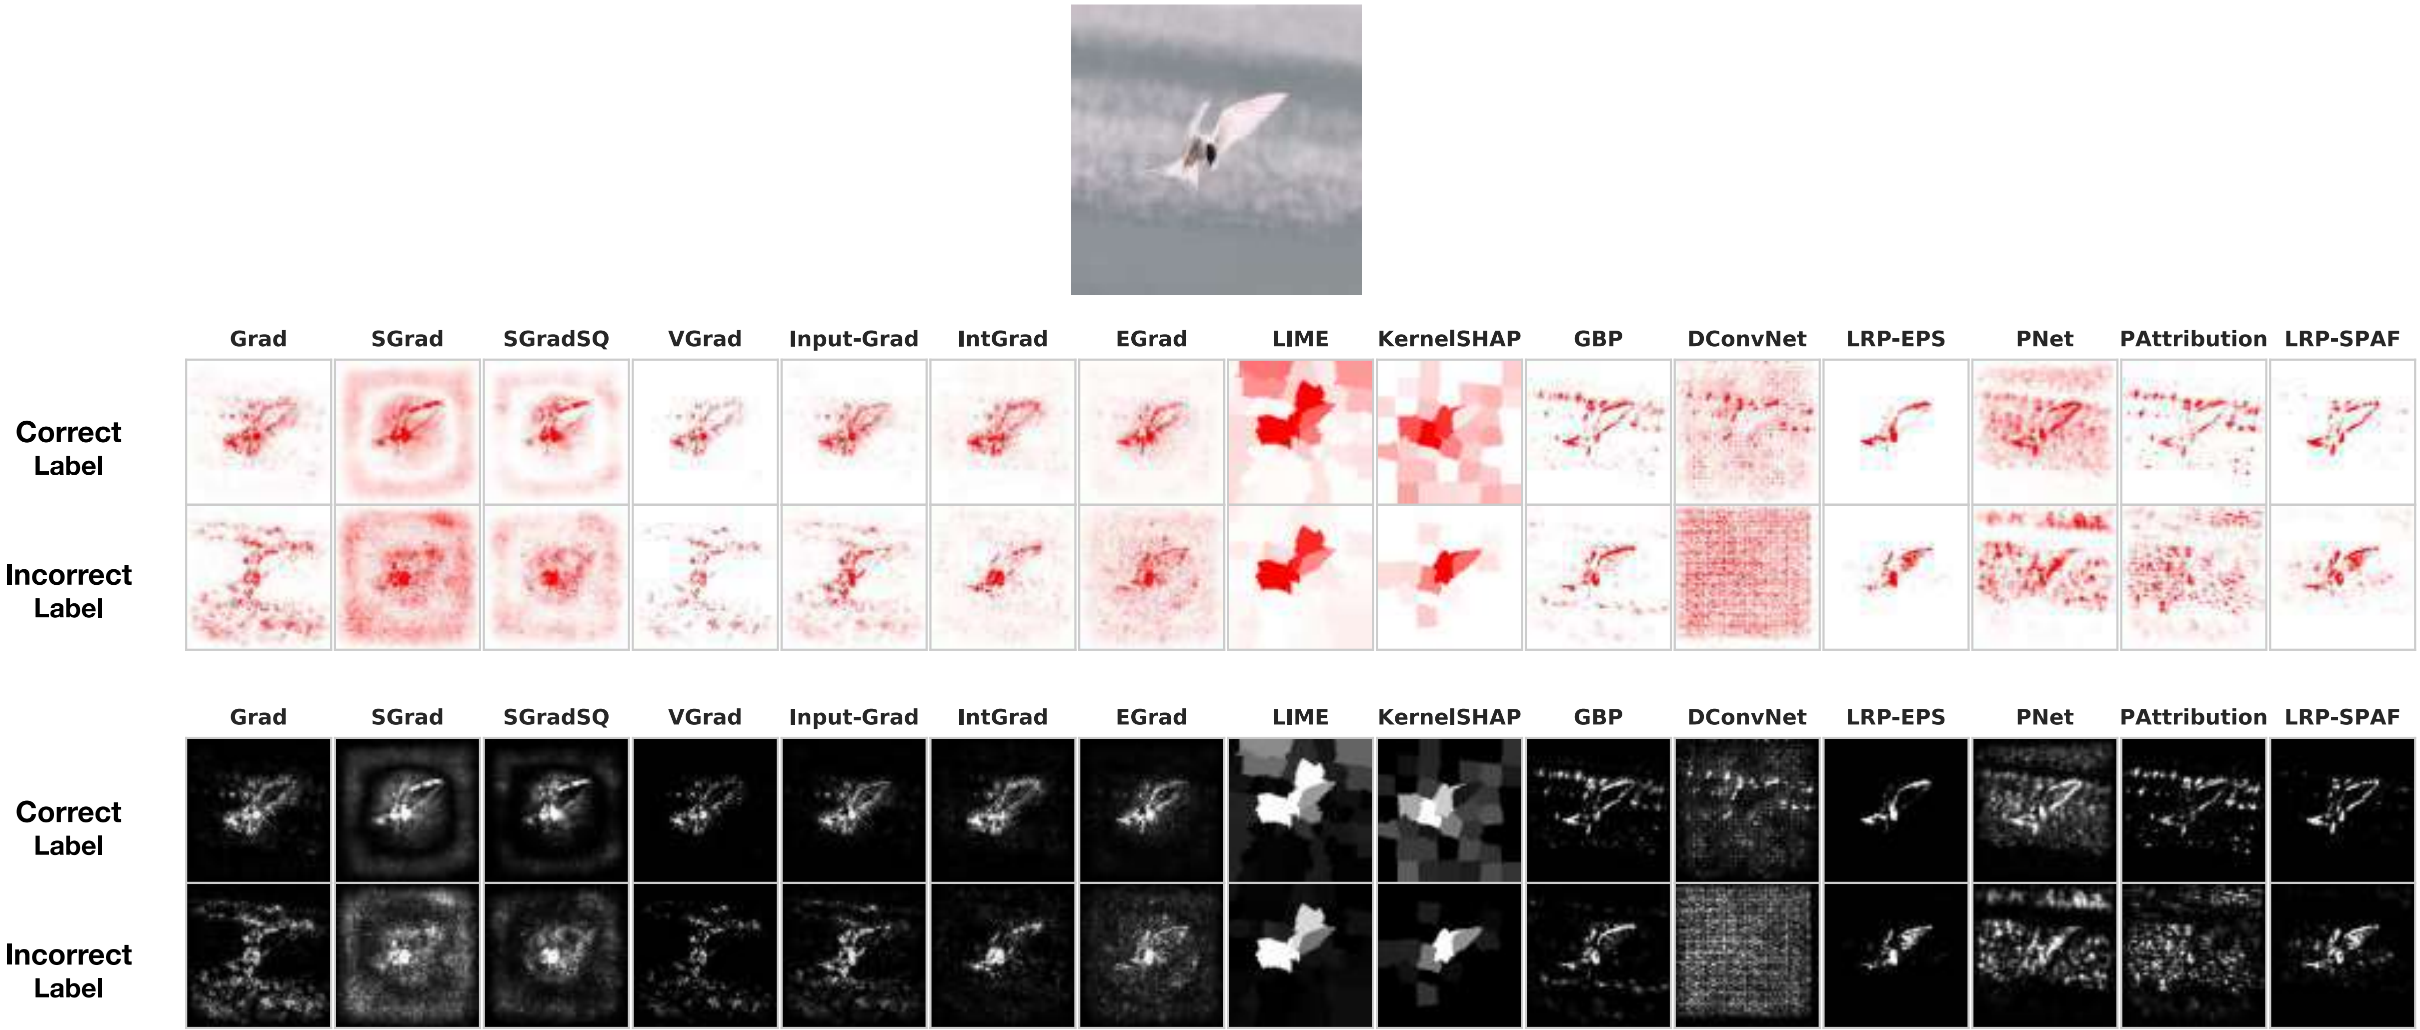
Grad
SGrad
SGradSQ
VGrad
Input-Grad
IntGrad
EGrad
LIME
KernelSHAP
GBP
DConvNet
LRP-EPS
PNet
PAttribution
LRP-SPAF
Correct Label
Incorrect Label
Grad
SGrad
SGradSQ
VGrad
Input-Grad
IntGrad
EGrad
LIME
KernelSHAP
GBP
DConvNet
LRP-EPS
PNet
PAttribution
LRP-SPAF
Correct Label
Incorrect Label

# Spurious Artifacts

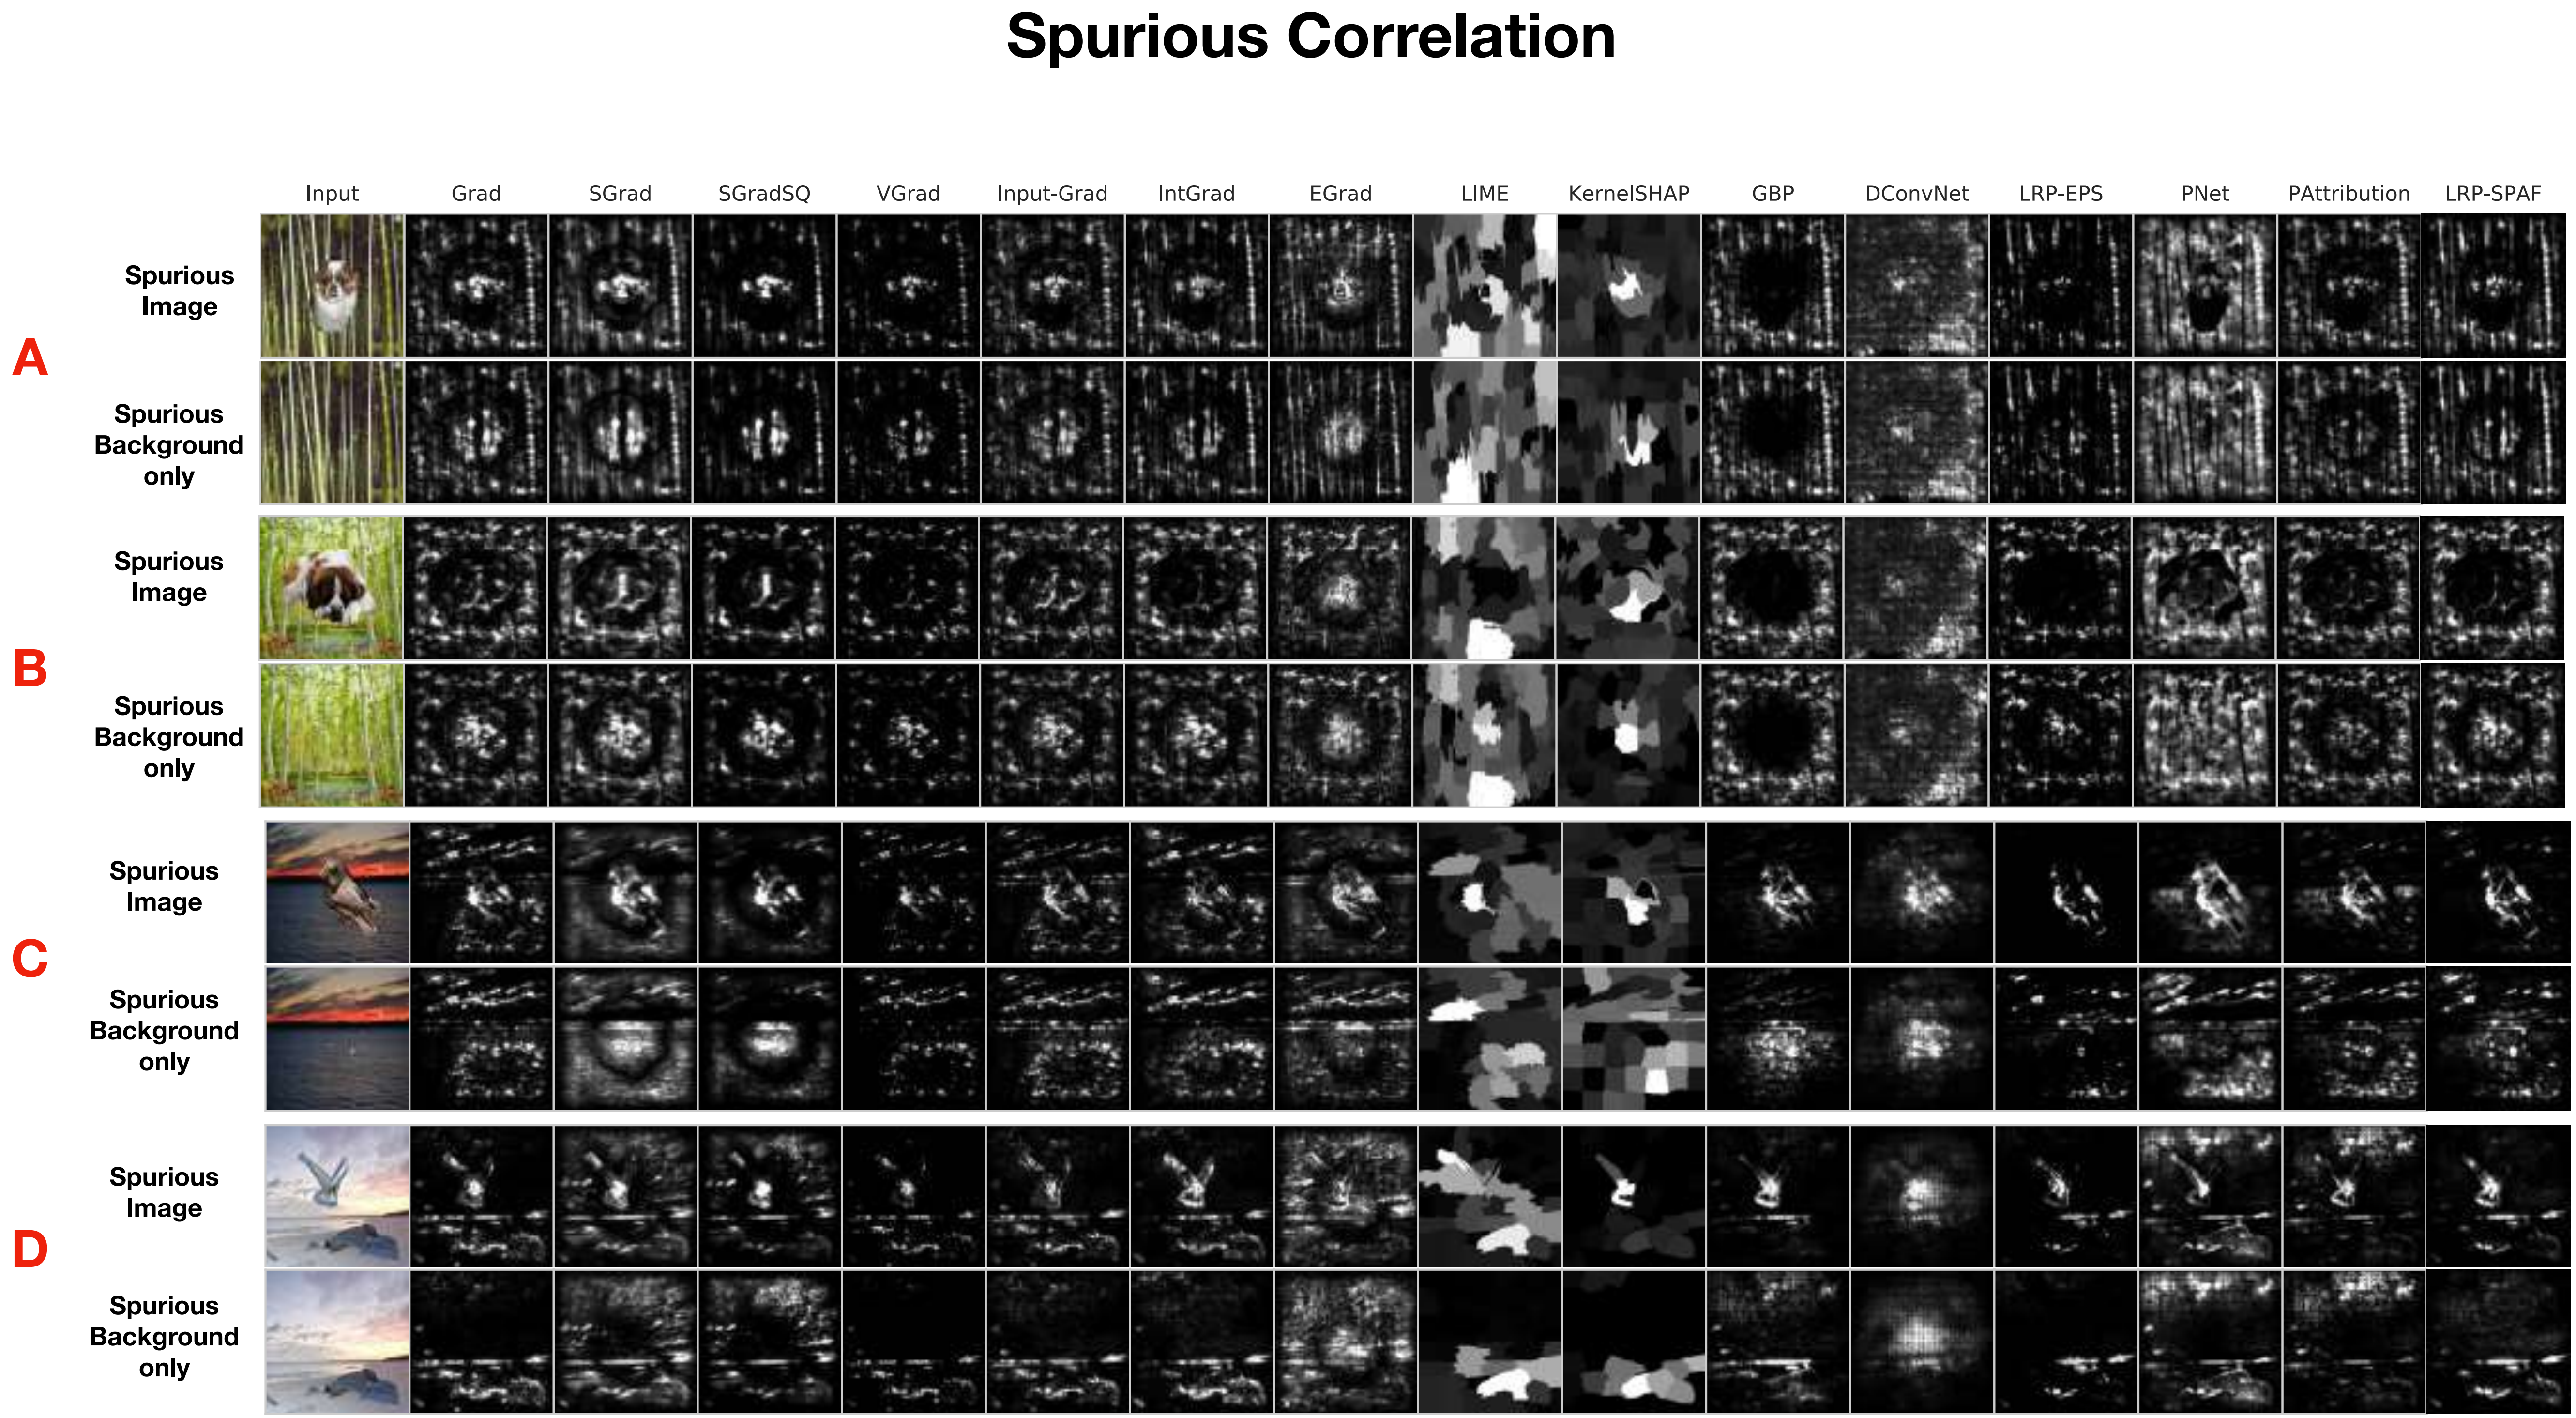
Spurious Correlation
Input
Grad
SGrad
SGradSQ
VGrad
Input-Grad
IntGrad
EGrad
LIME
KernelSHAP
GBP
DConvNet
LRP-EPS
PNet
PAttribution
LRP-SPAF
A
Spurious Image
Spurious Background only
B
Spurious Image
Spurious Background only
C
Spurious Image
Spurious Background only
D
Spurious Image
Spurious Background only

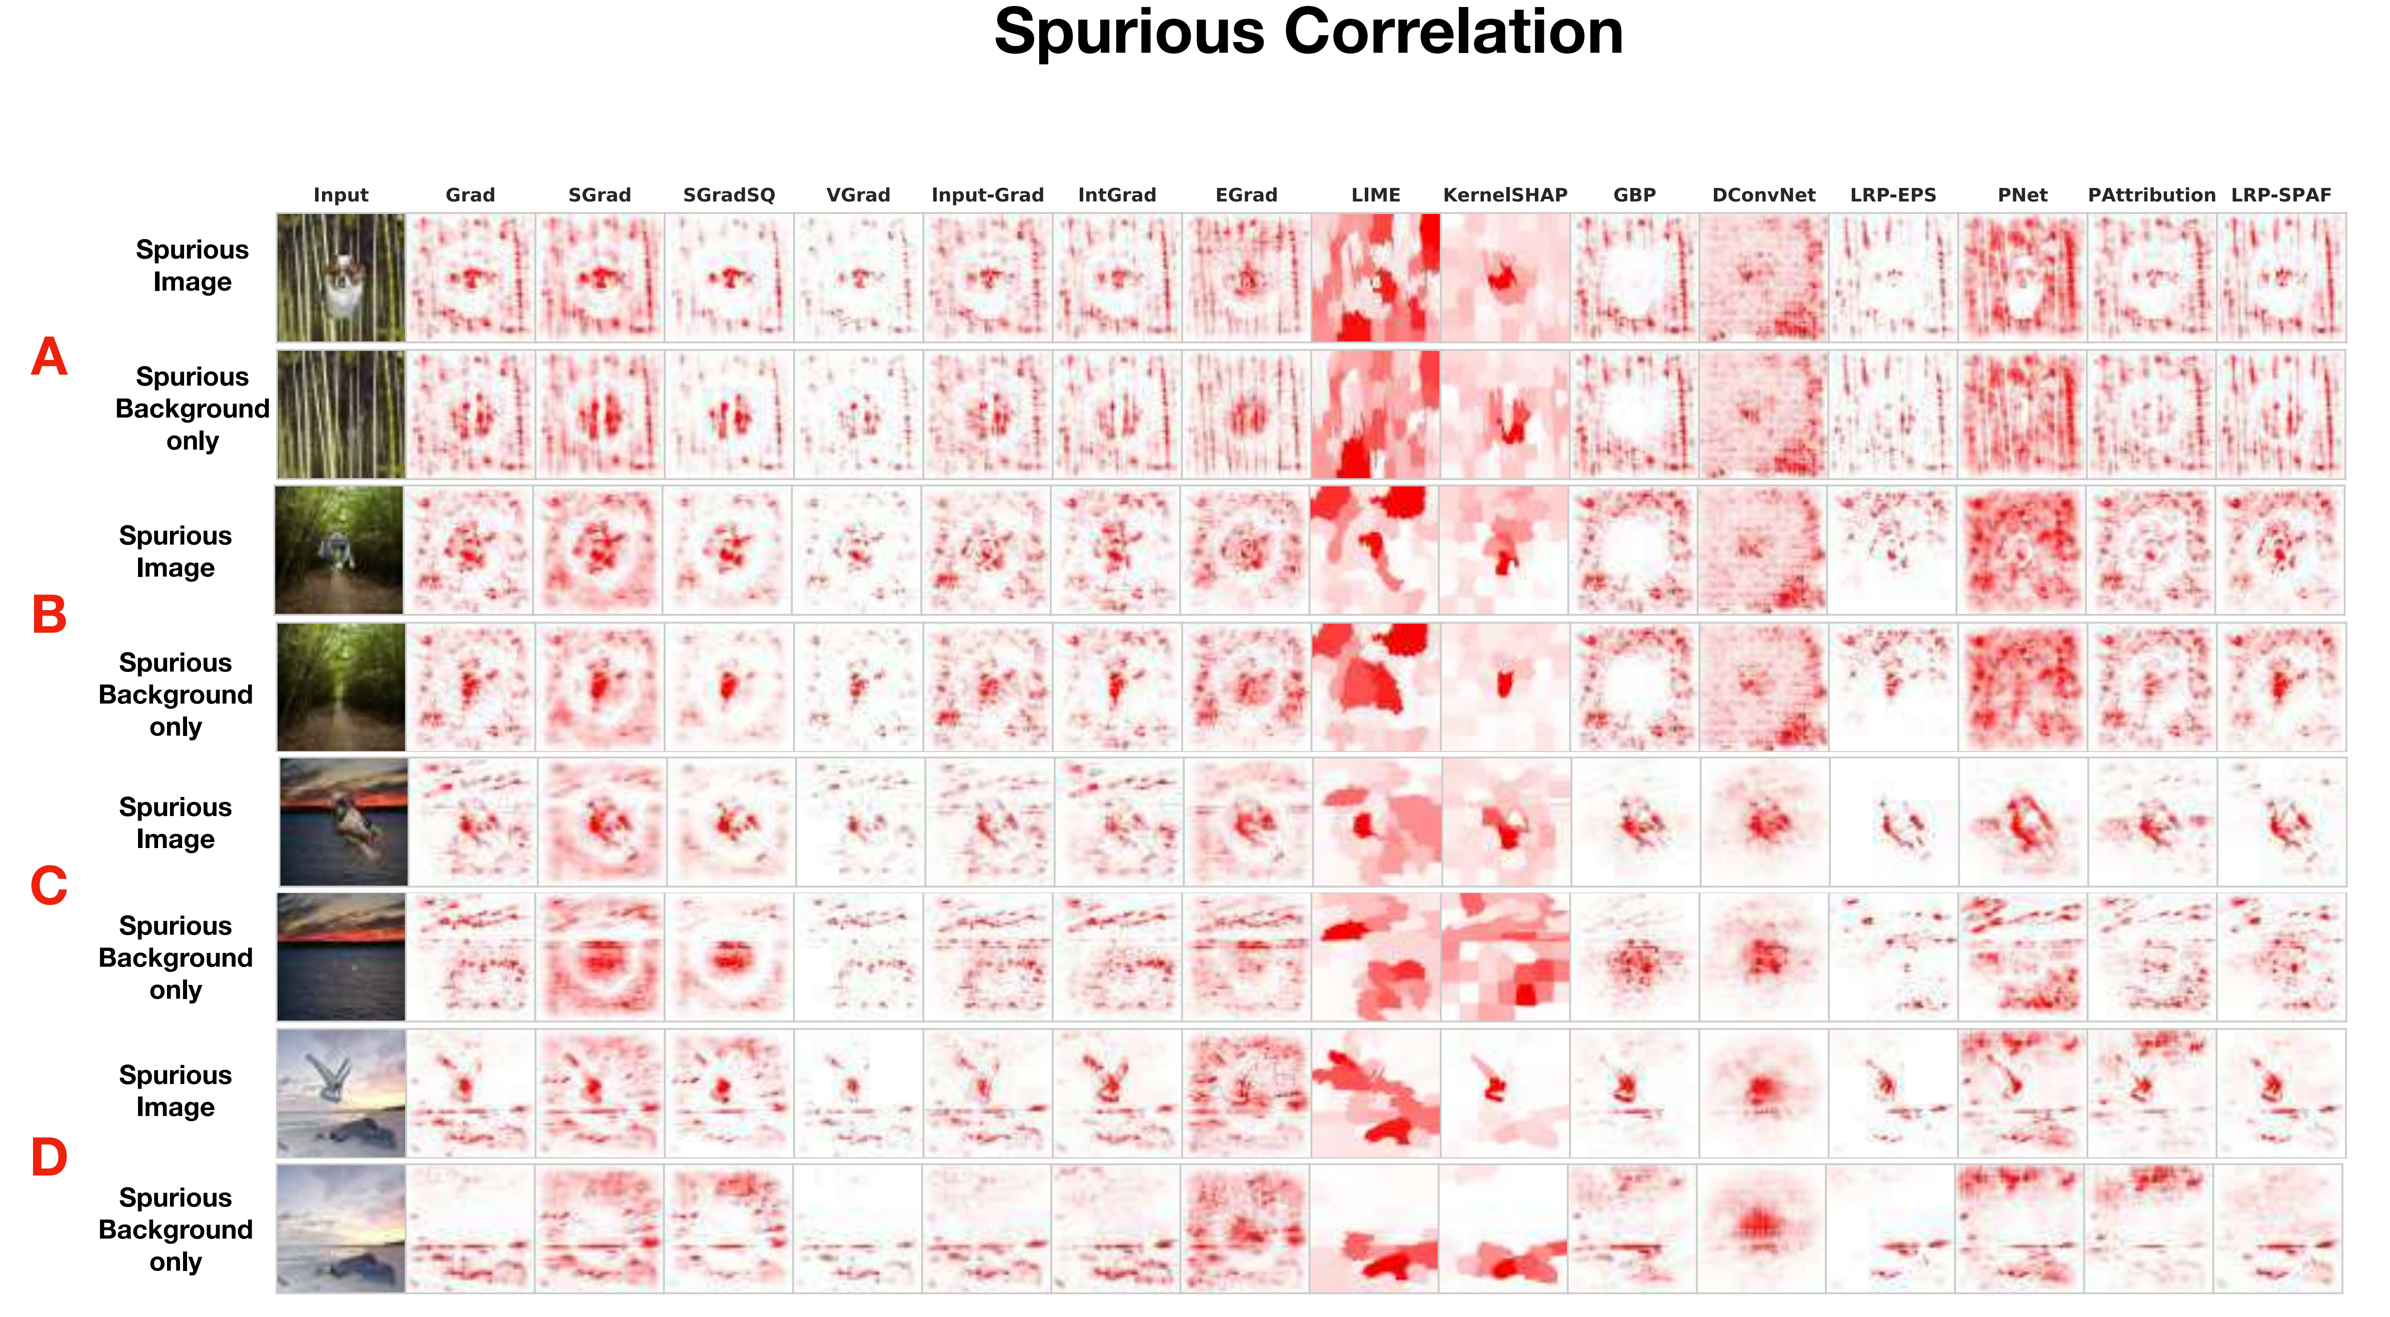
Spurious Correlation
Input
Grad
SGrad
SGradSQ
VGrad
Input-Grad
IntGrad
EGrad
LIME
KernelSHAP
GBP
DConvNet
LRP-EPS
PNet
PAttribution
LRP-SPAF
A
Spurious Image
Spurious Background only
B
Spurious Image
Spurious Background only
C
Spurious Image
Spurious Background only
D
Spurious Image
Spurious Background only

# Spurious Correlation

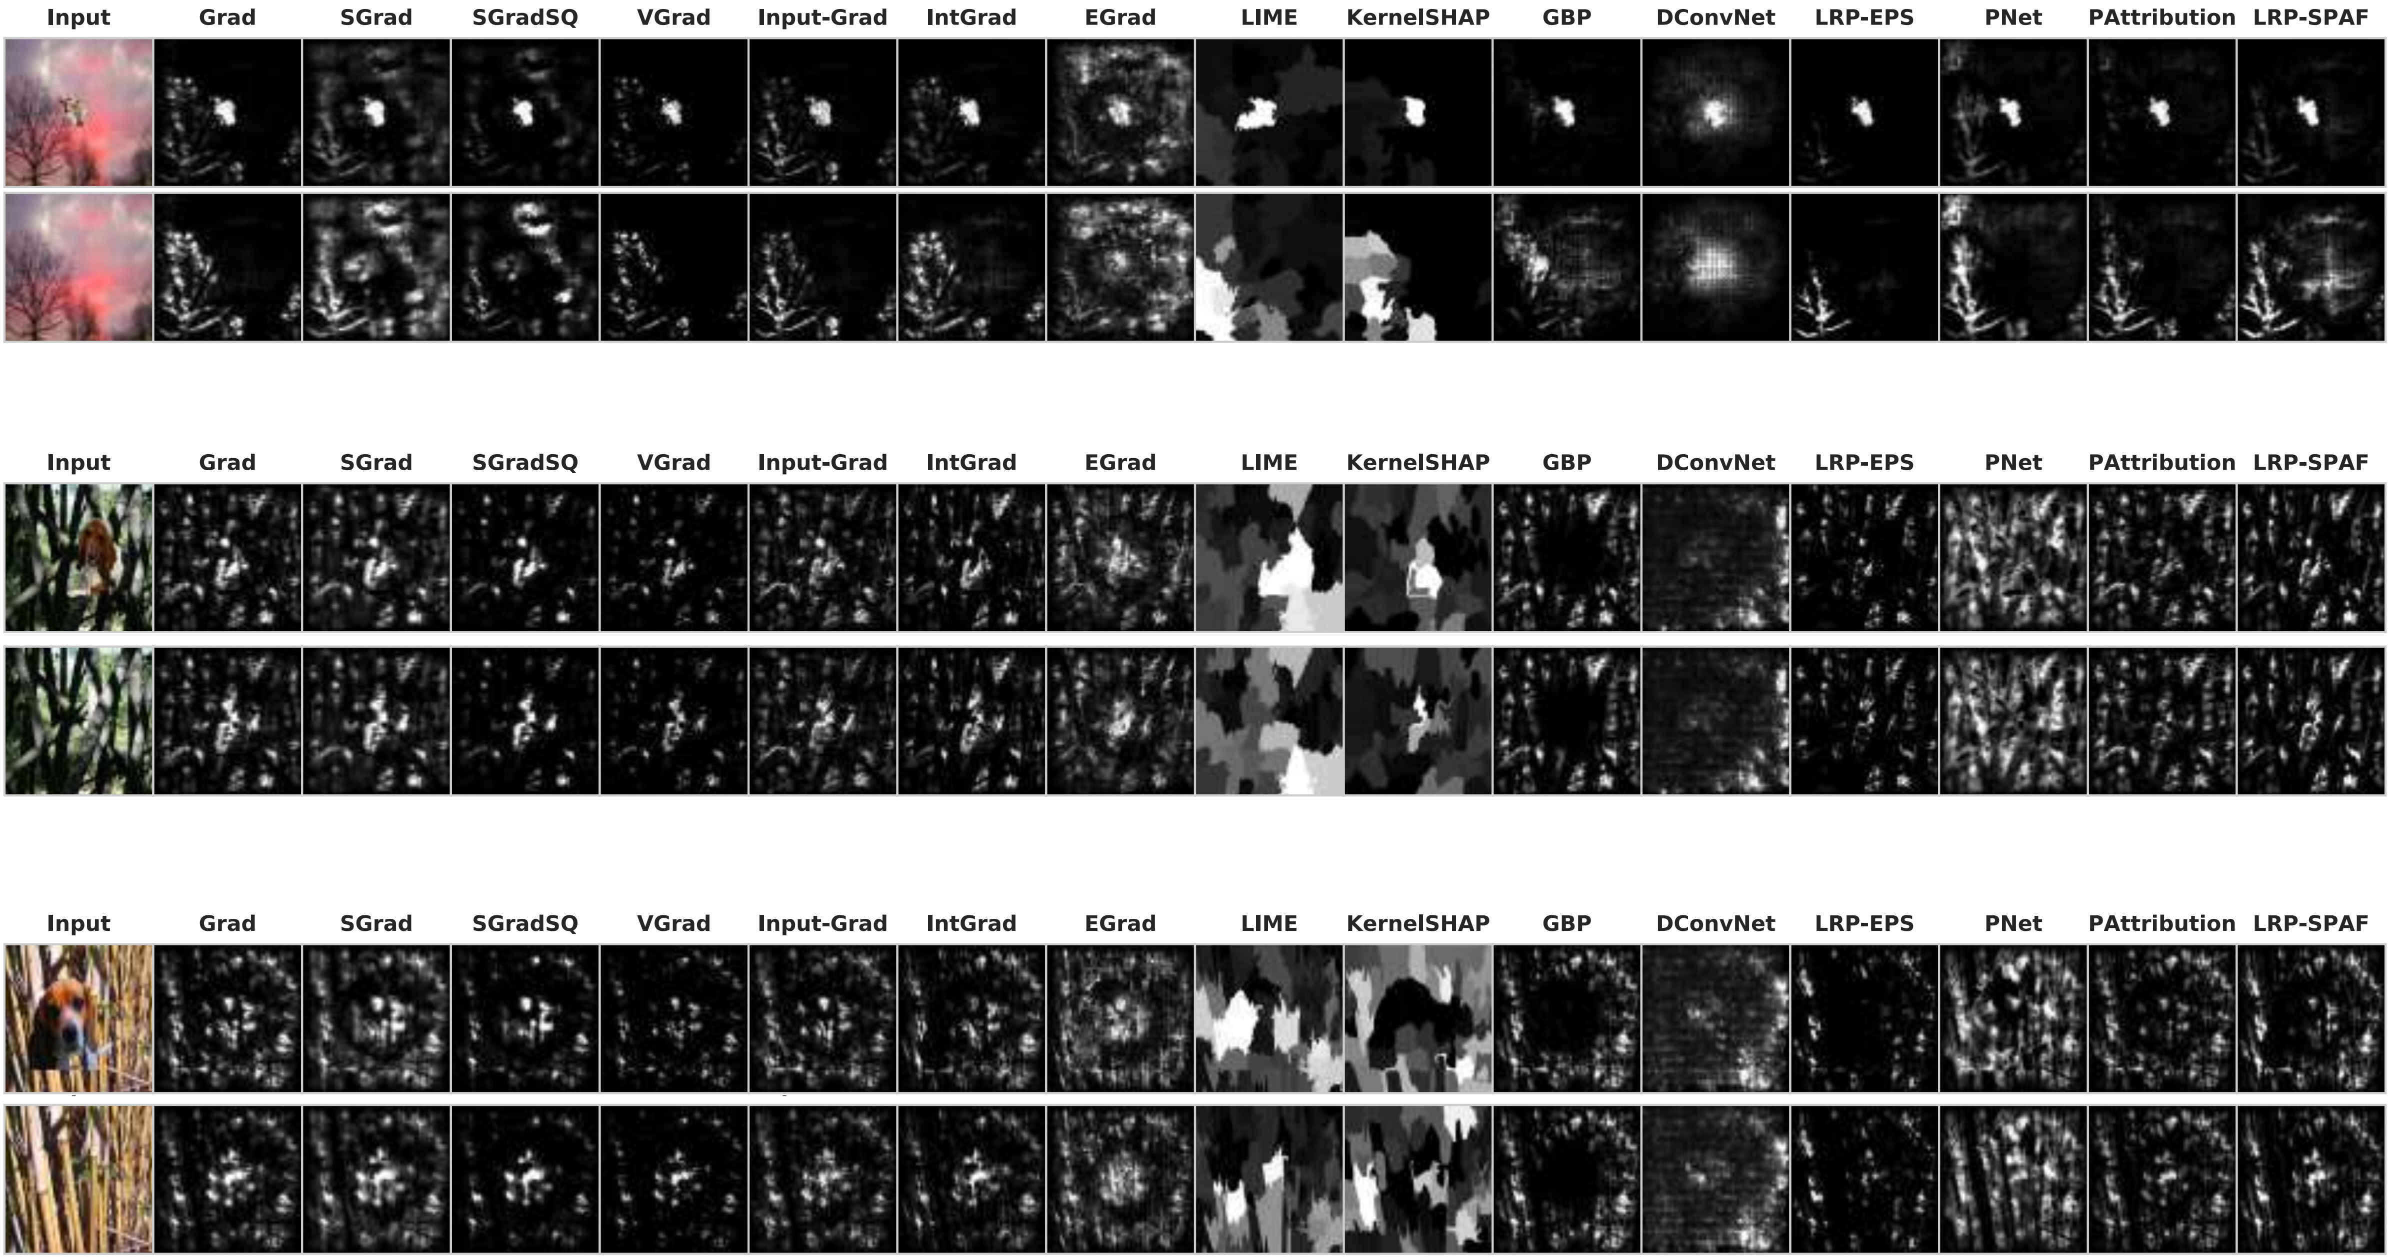

# Model Contamination Figure

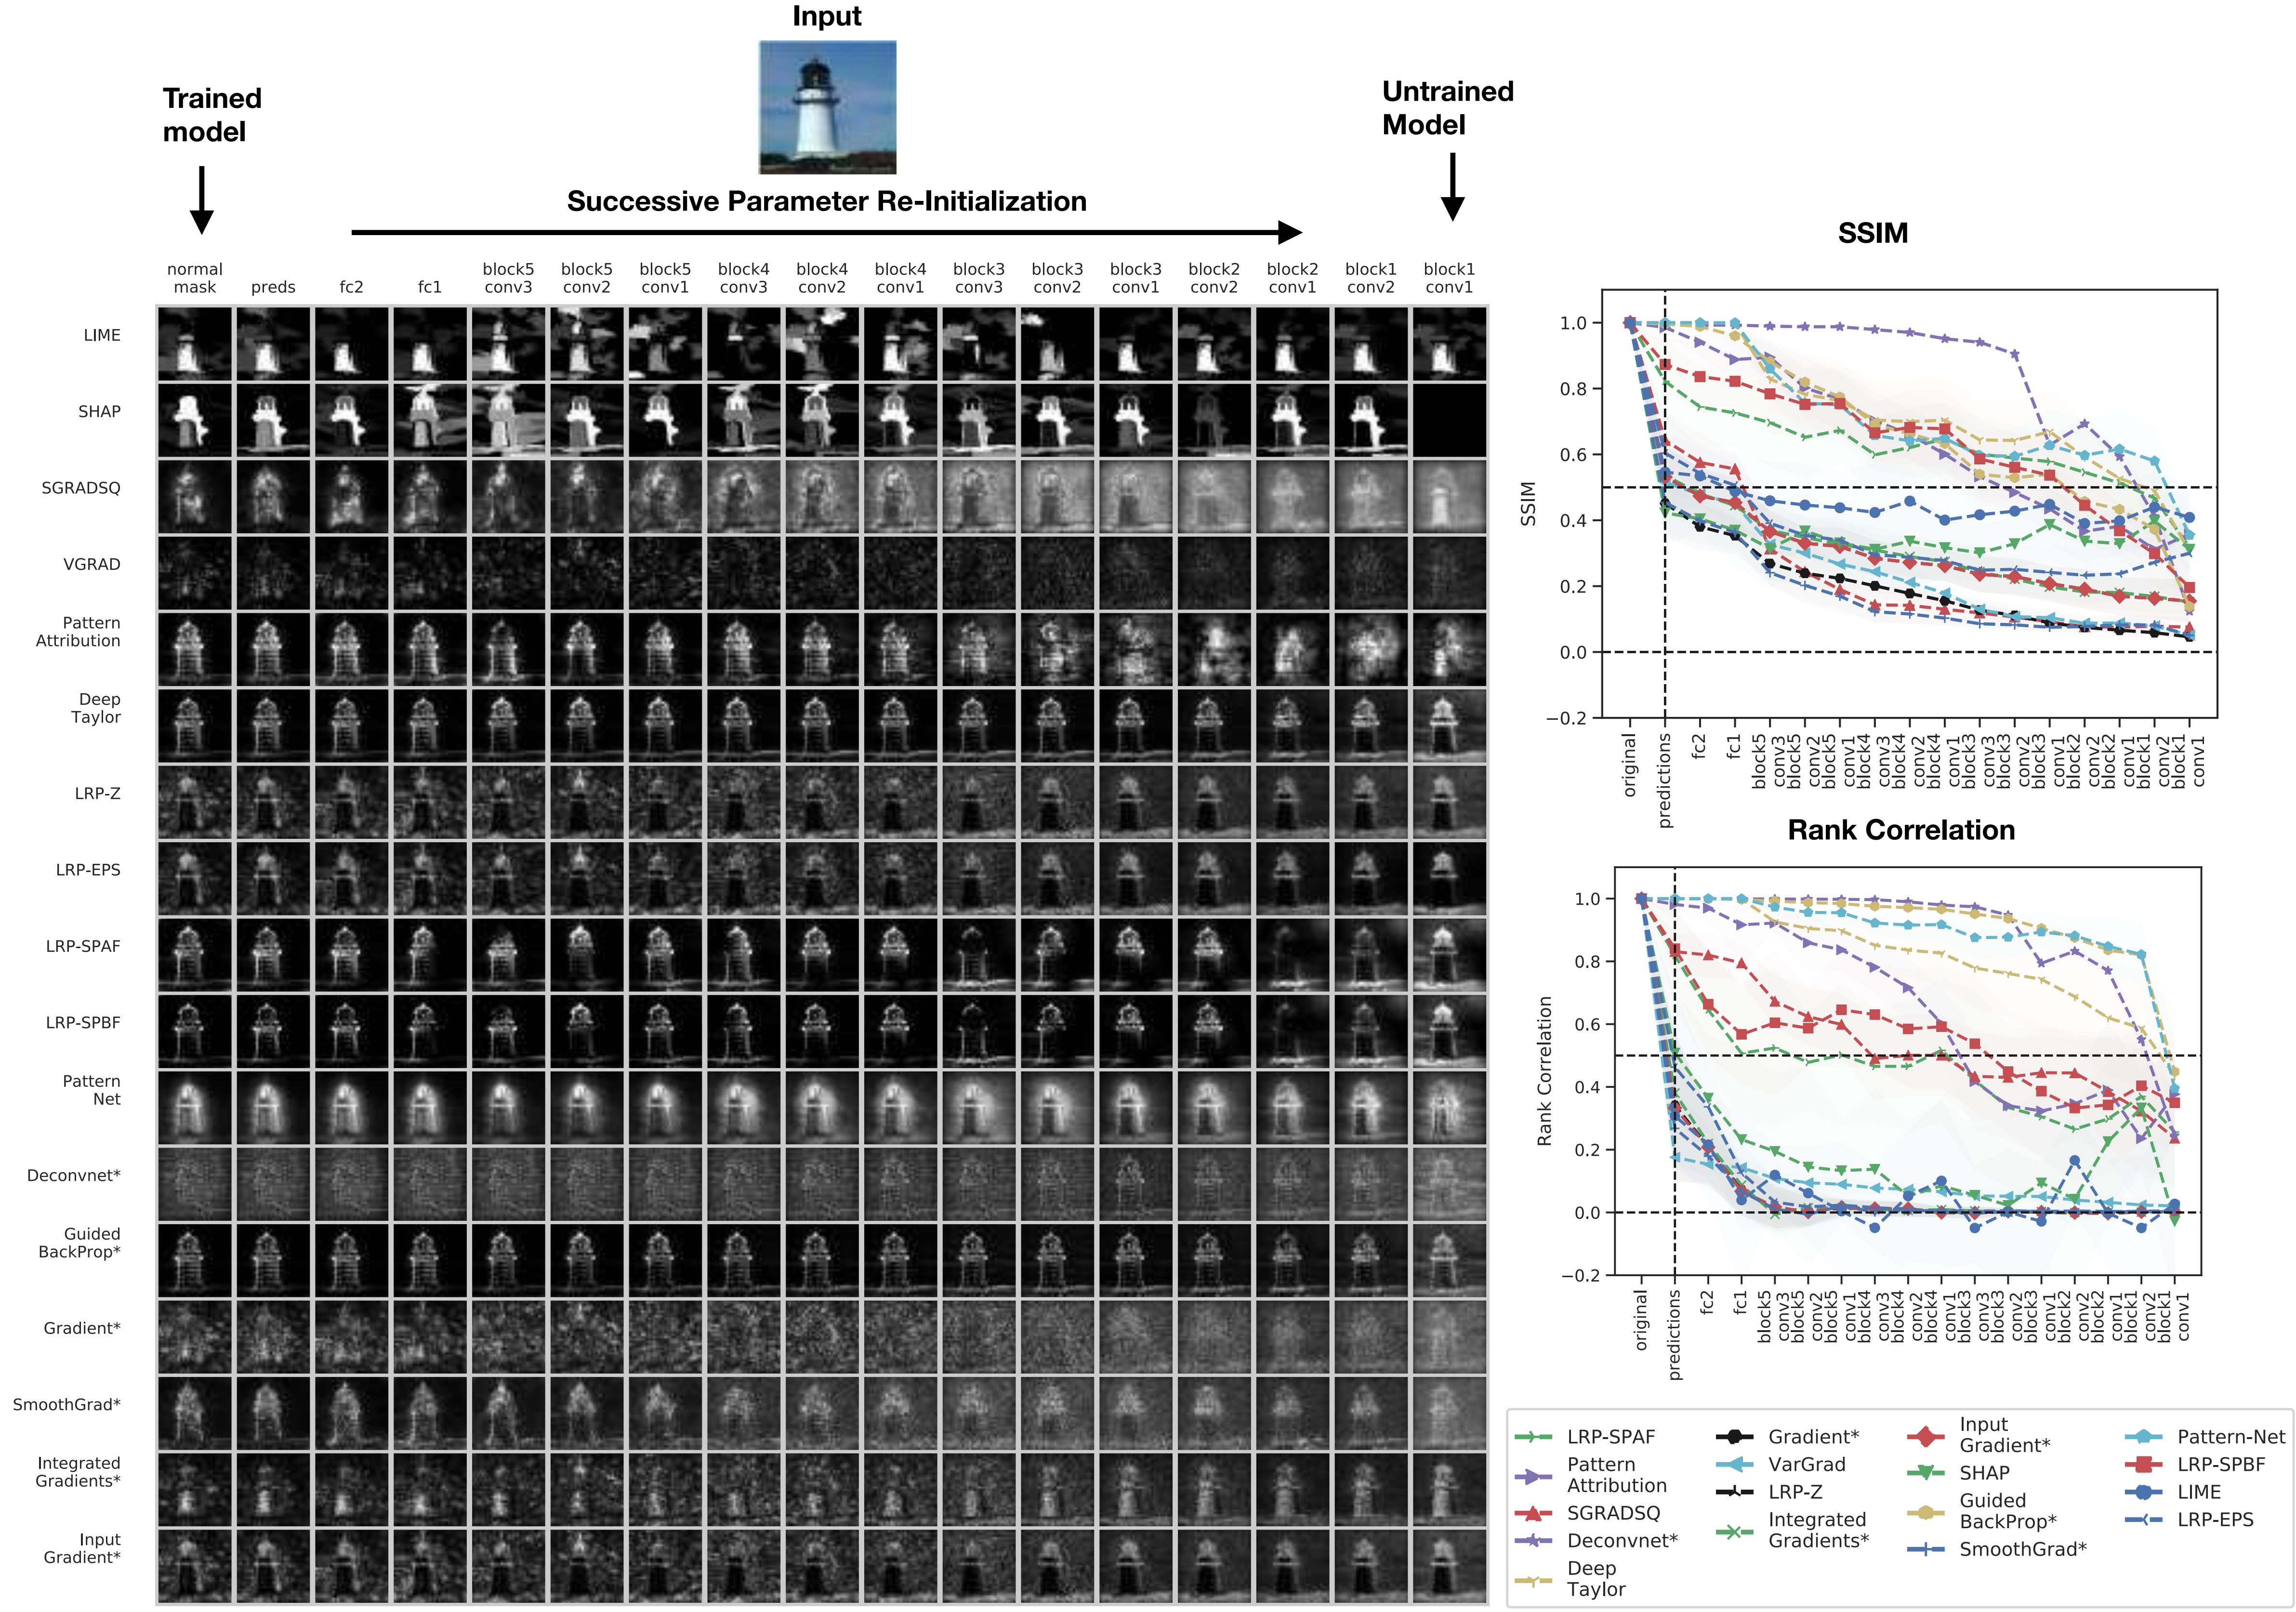

# Model Contamination Figure: Alternative

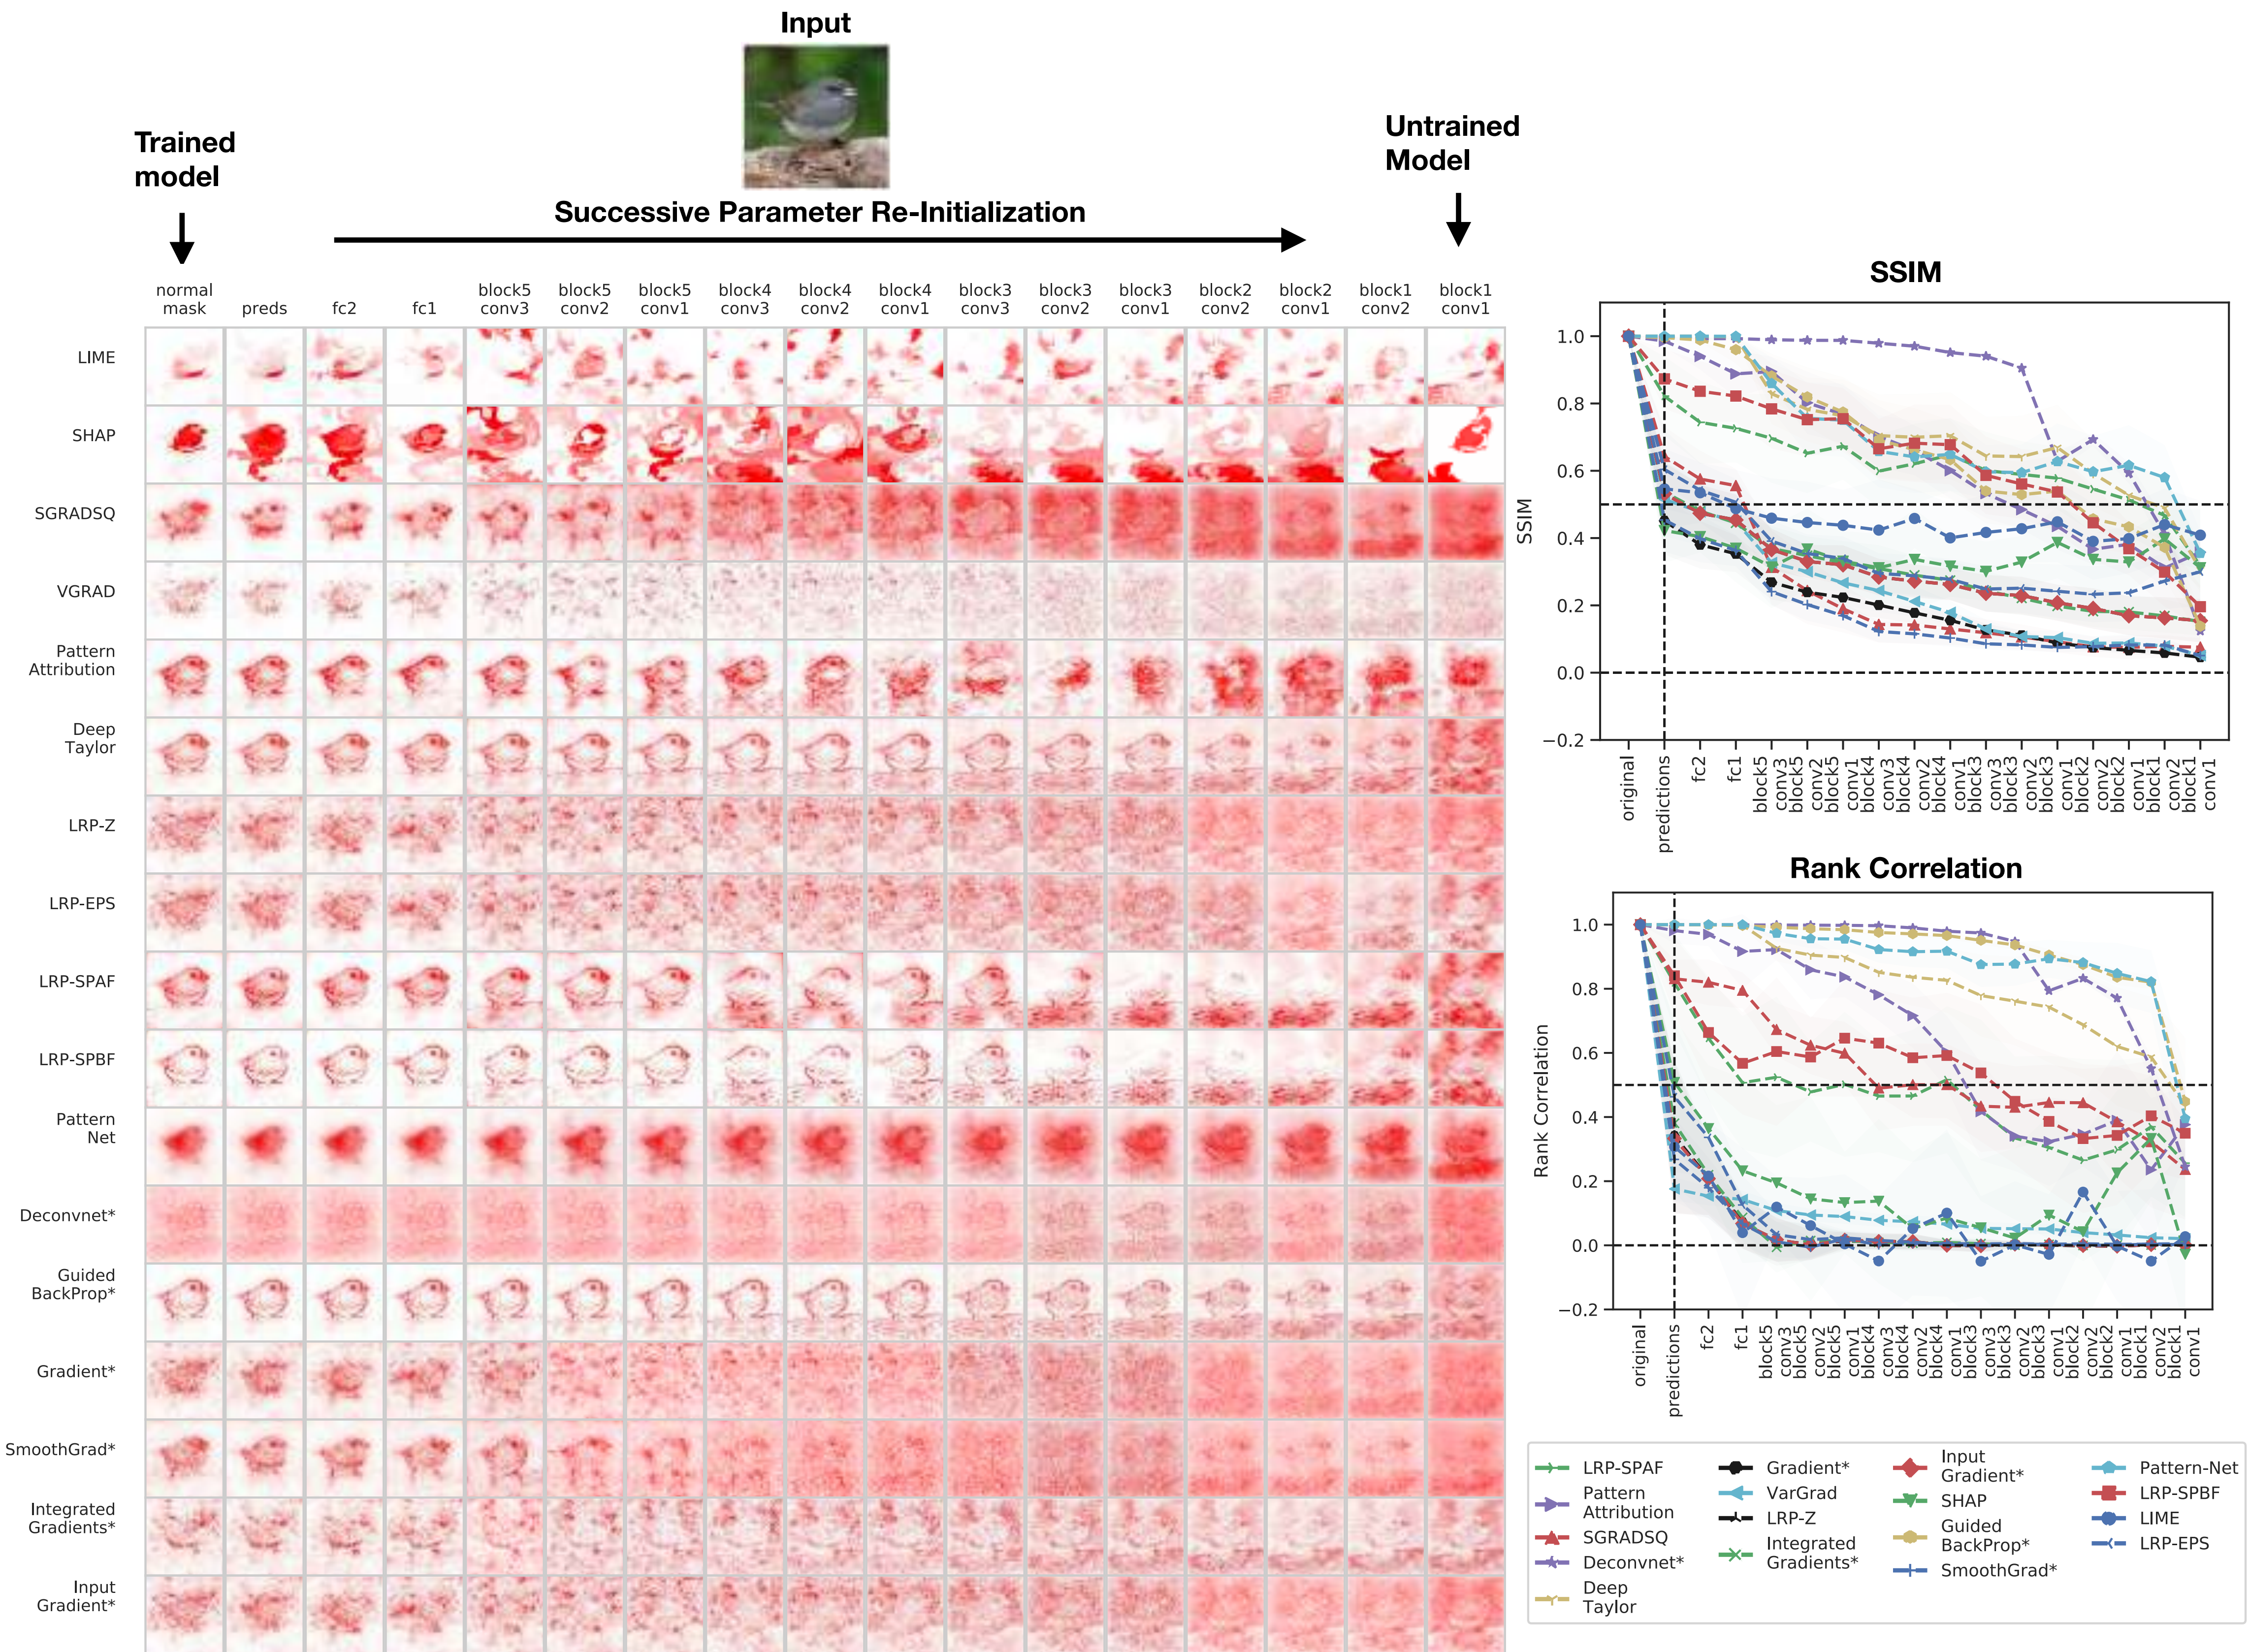

# Test Time Contamination

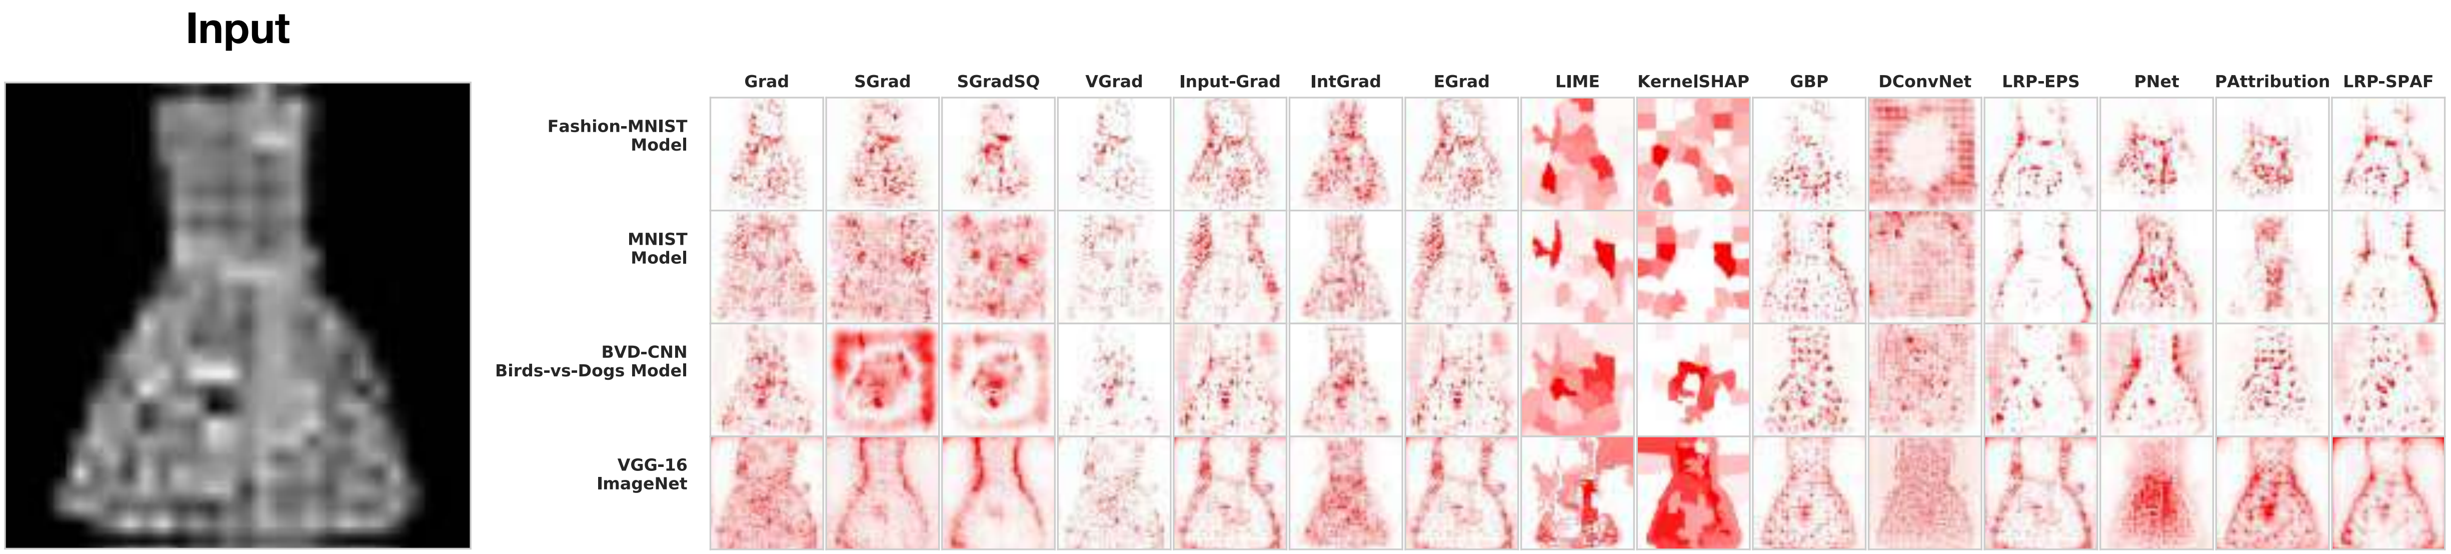
Input
Grad
SGrad
SGradSQ
VGrad
Input-Grad
IntGrad
EGrad
LIME
KernelSHAP
GBP
DConvNet
LRP-EPS
PNet
PAttribution
LRP-SPAF
Fashion-MNIST Model
MNIST Model
BVD-CNN Birds-vs-Dogs Model
VGG-16 ImageNet

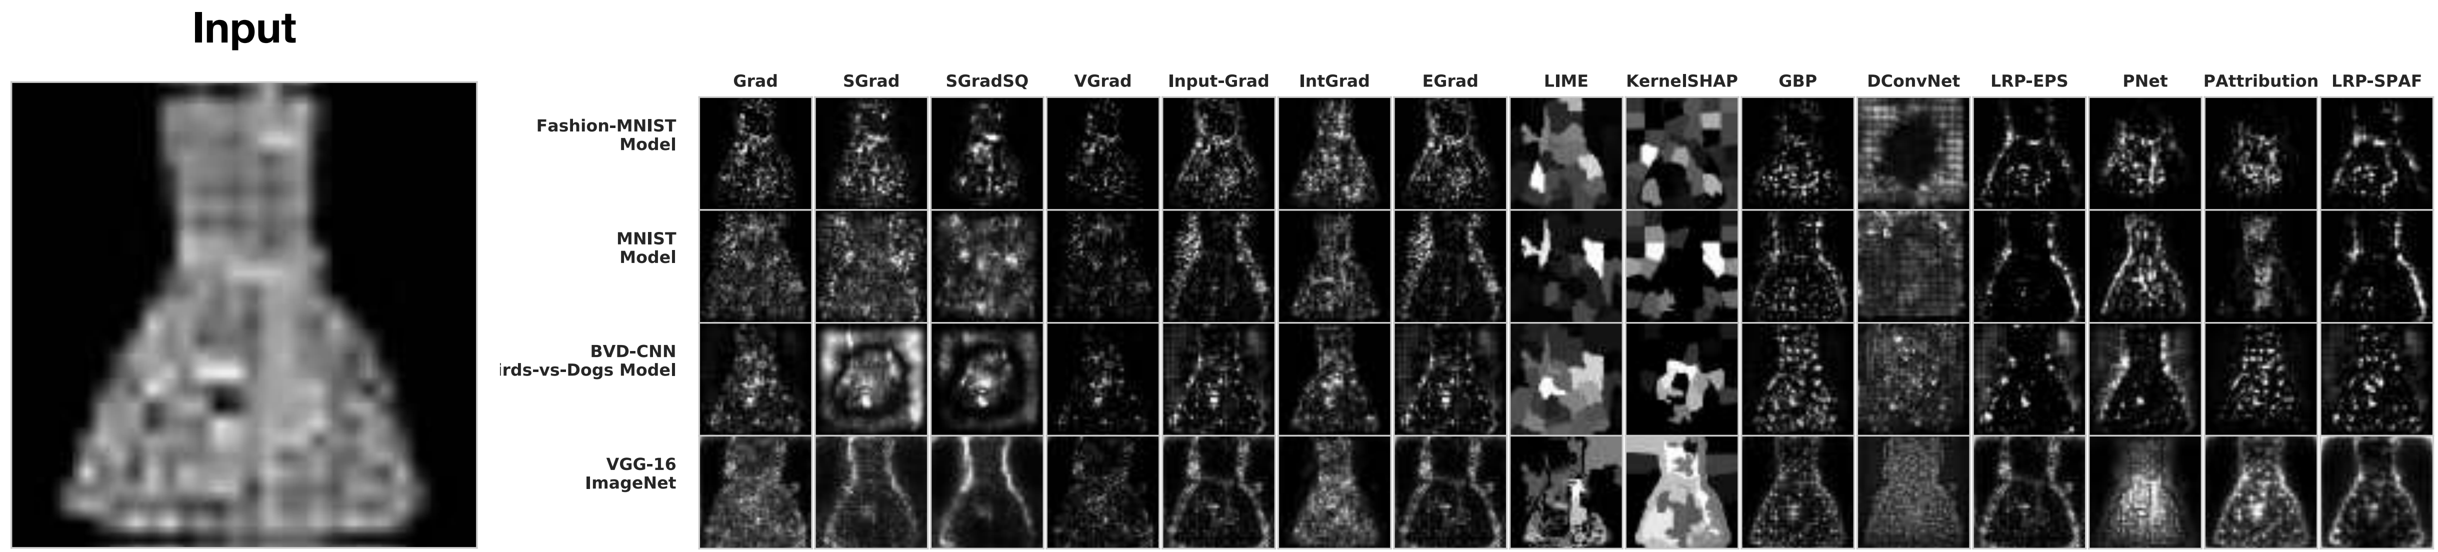

Input
Grad
SGrad
SGradSQ
VGrad
Input-Grad
IntGrad
EGrad
LIME
KernelSHAP
GBP
DConvNet
LRP-EPS
PNet
PAttribution
LRP-SPAF
Fashion-MNIST Model
MNIST Model
BVD-CNN
irds-vs-Dogs Model
VGG-16 ImageNet

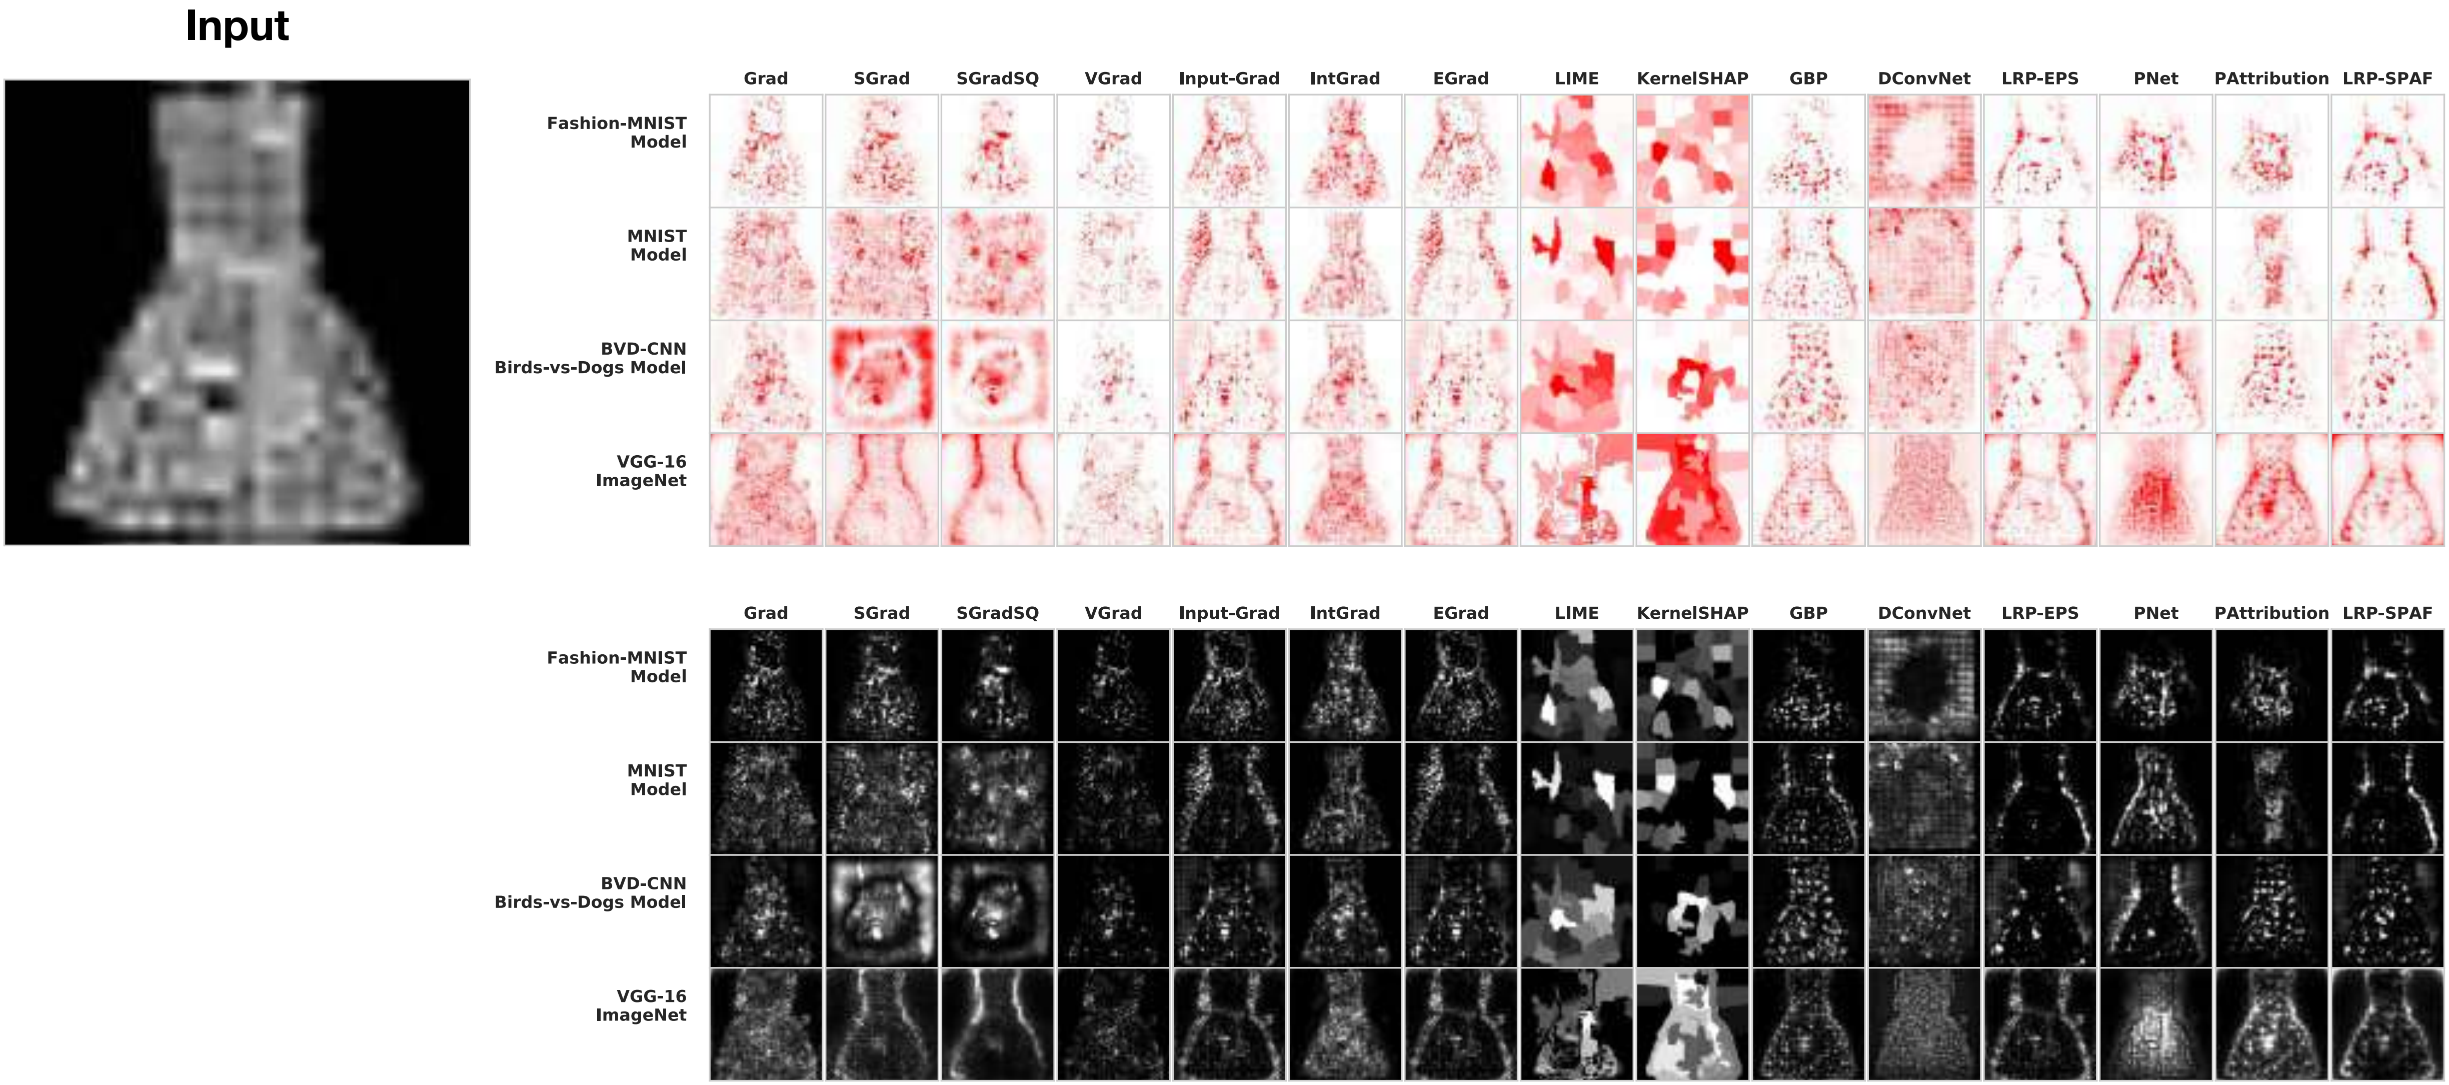
Input
Grad
SGrad
SGradSQ
VGrad
Input-Grad
IntGrad
EGrad
LIME
KernelSHAP
GBP
DConvNet
LRP-EPS
PNet
PAttribution
LRP-SPAF
Fashion-MNIST Model
MNIST Model
BVD-CNN Birds-vs-Dogs Model
VGG-16 ImageNet

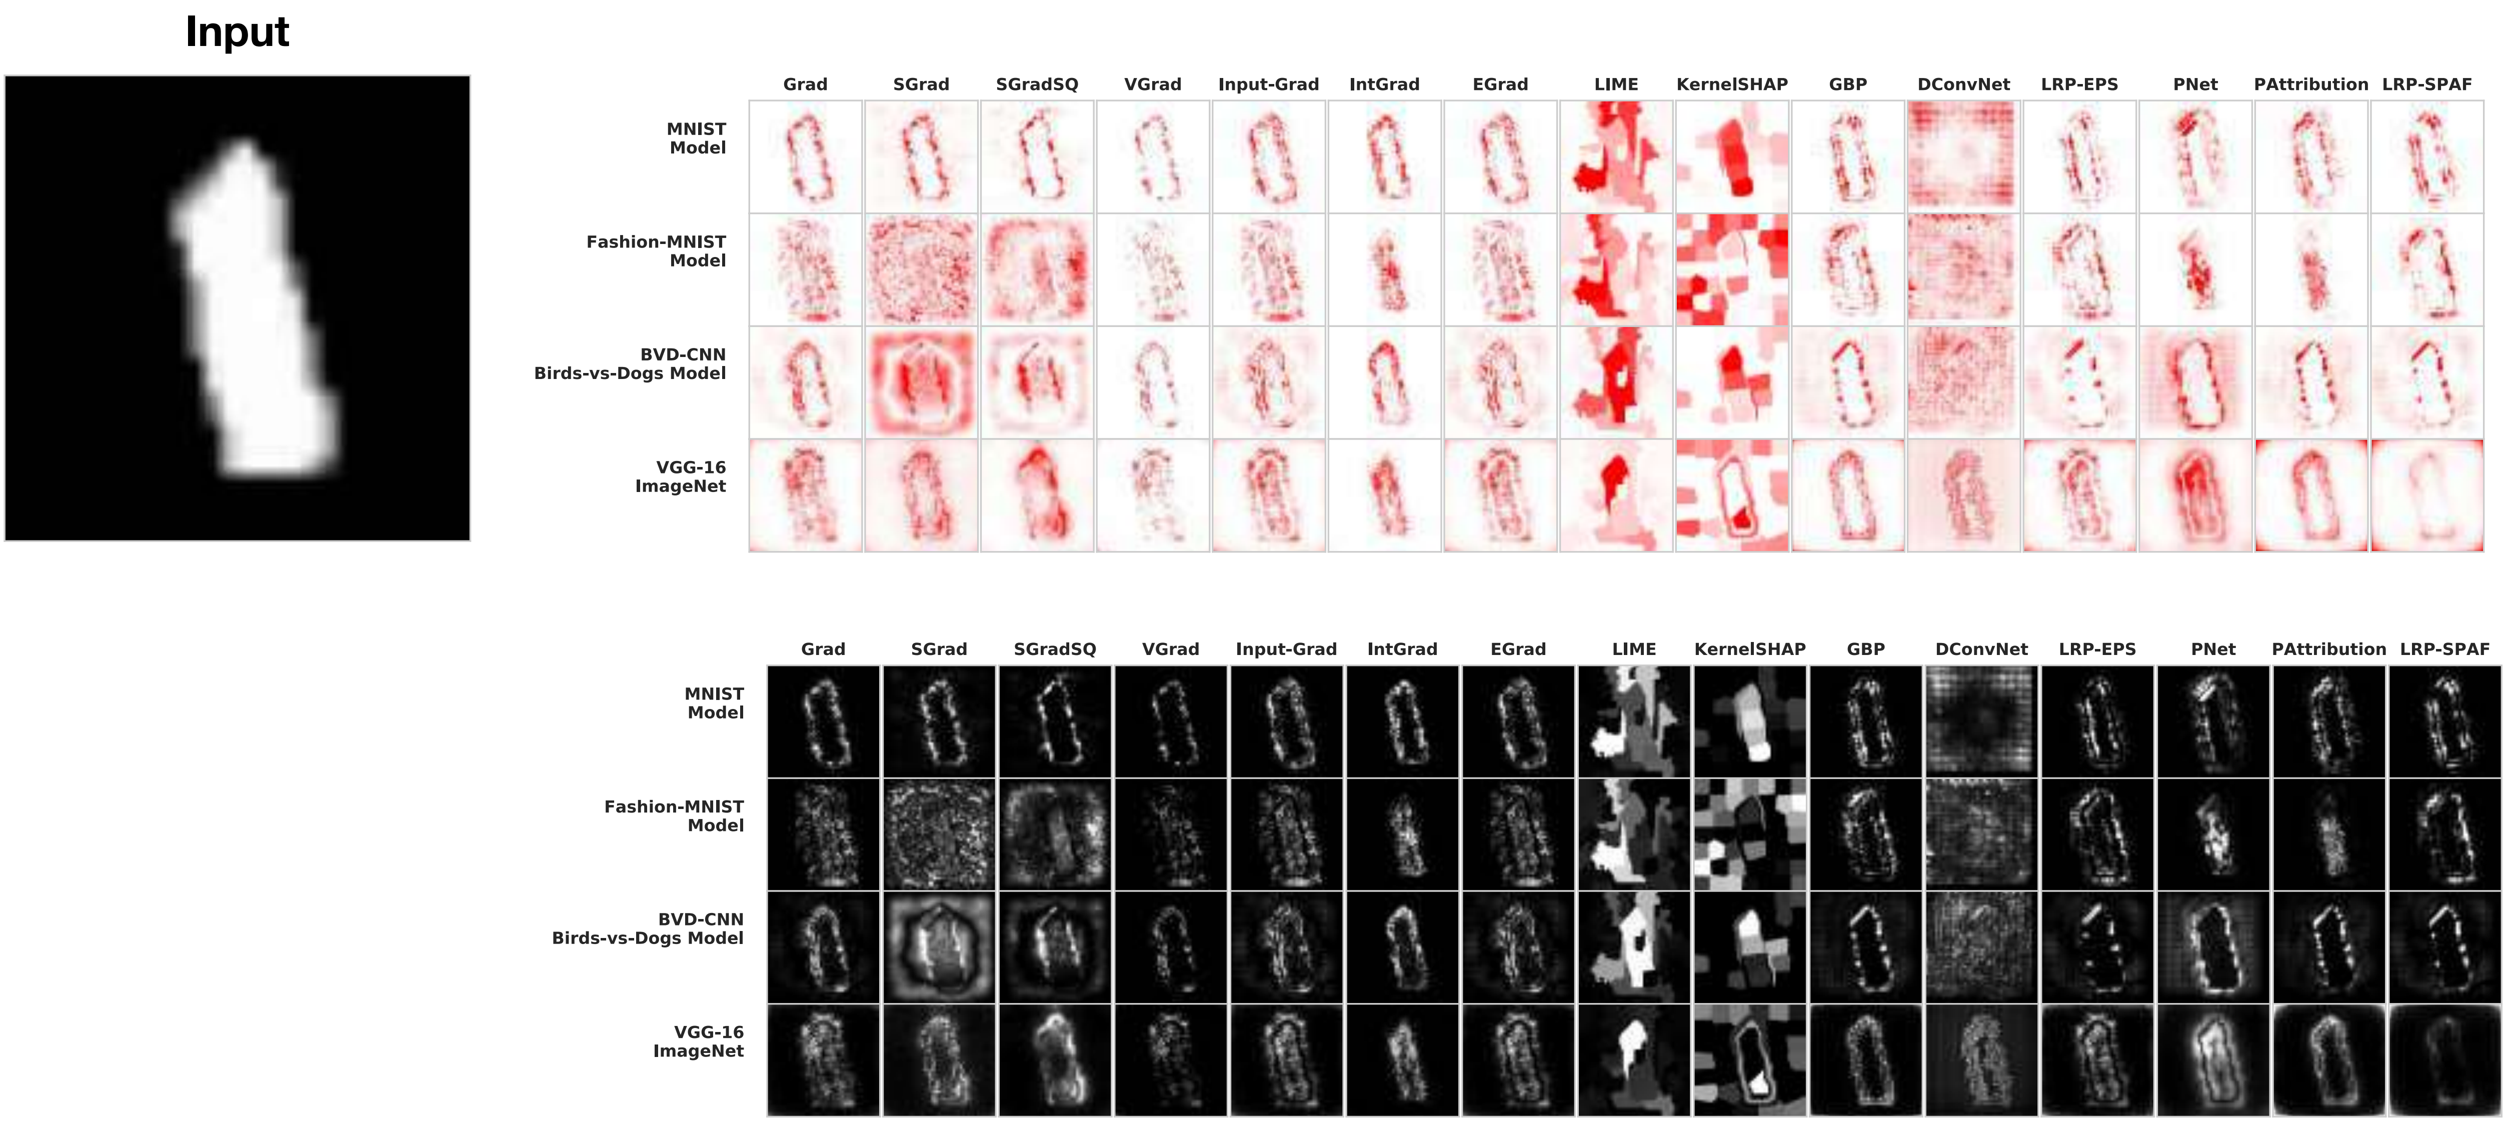
Input
Grad
SGrad
SGradSQ
VGrad
Input-Grad
IntGrad
EGrad
LIME
KernelSHAP
GBP
DConvNet
LRP-EPS
PNet
PAttribution
LRP-SPAF
MNIST Model
Fashion-MNIST Model
BVD-CNN Birds-vs-Dogs Model
VGG-16 ImageNet

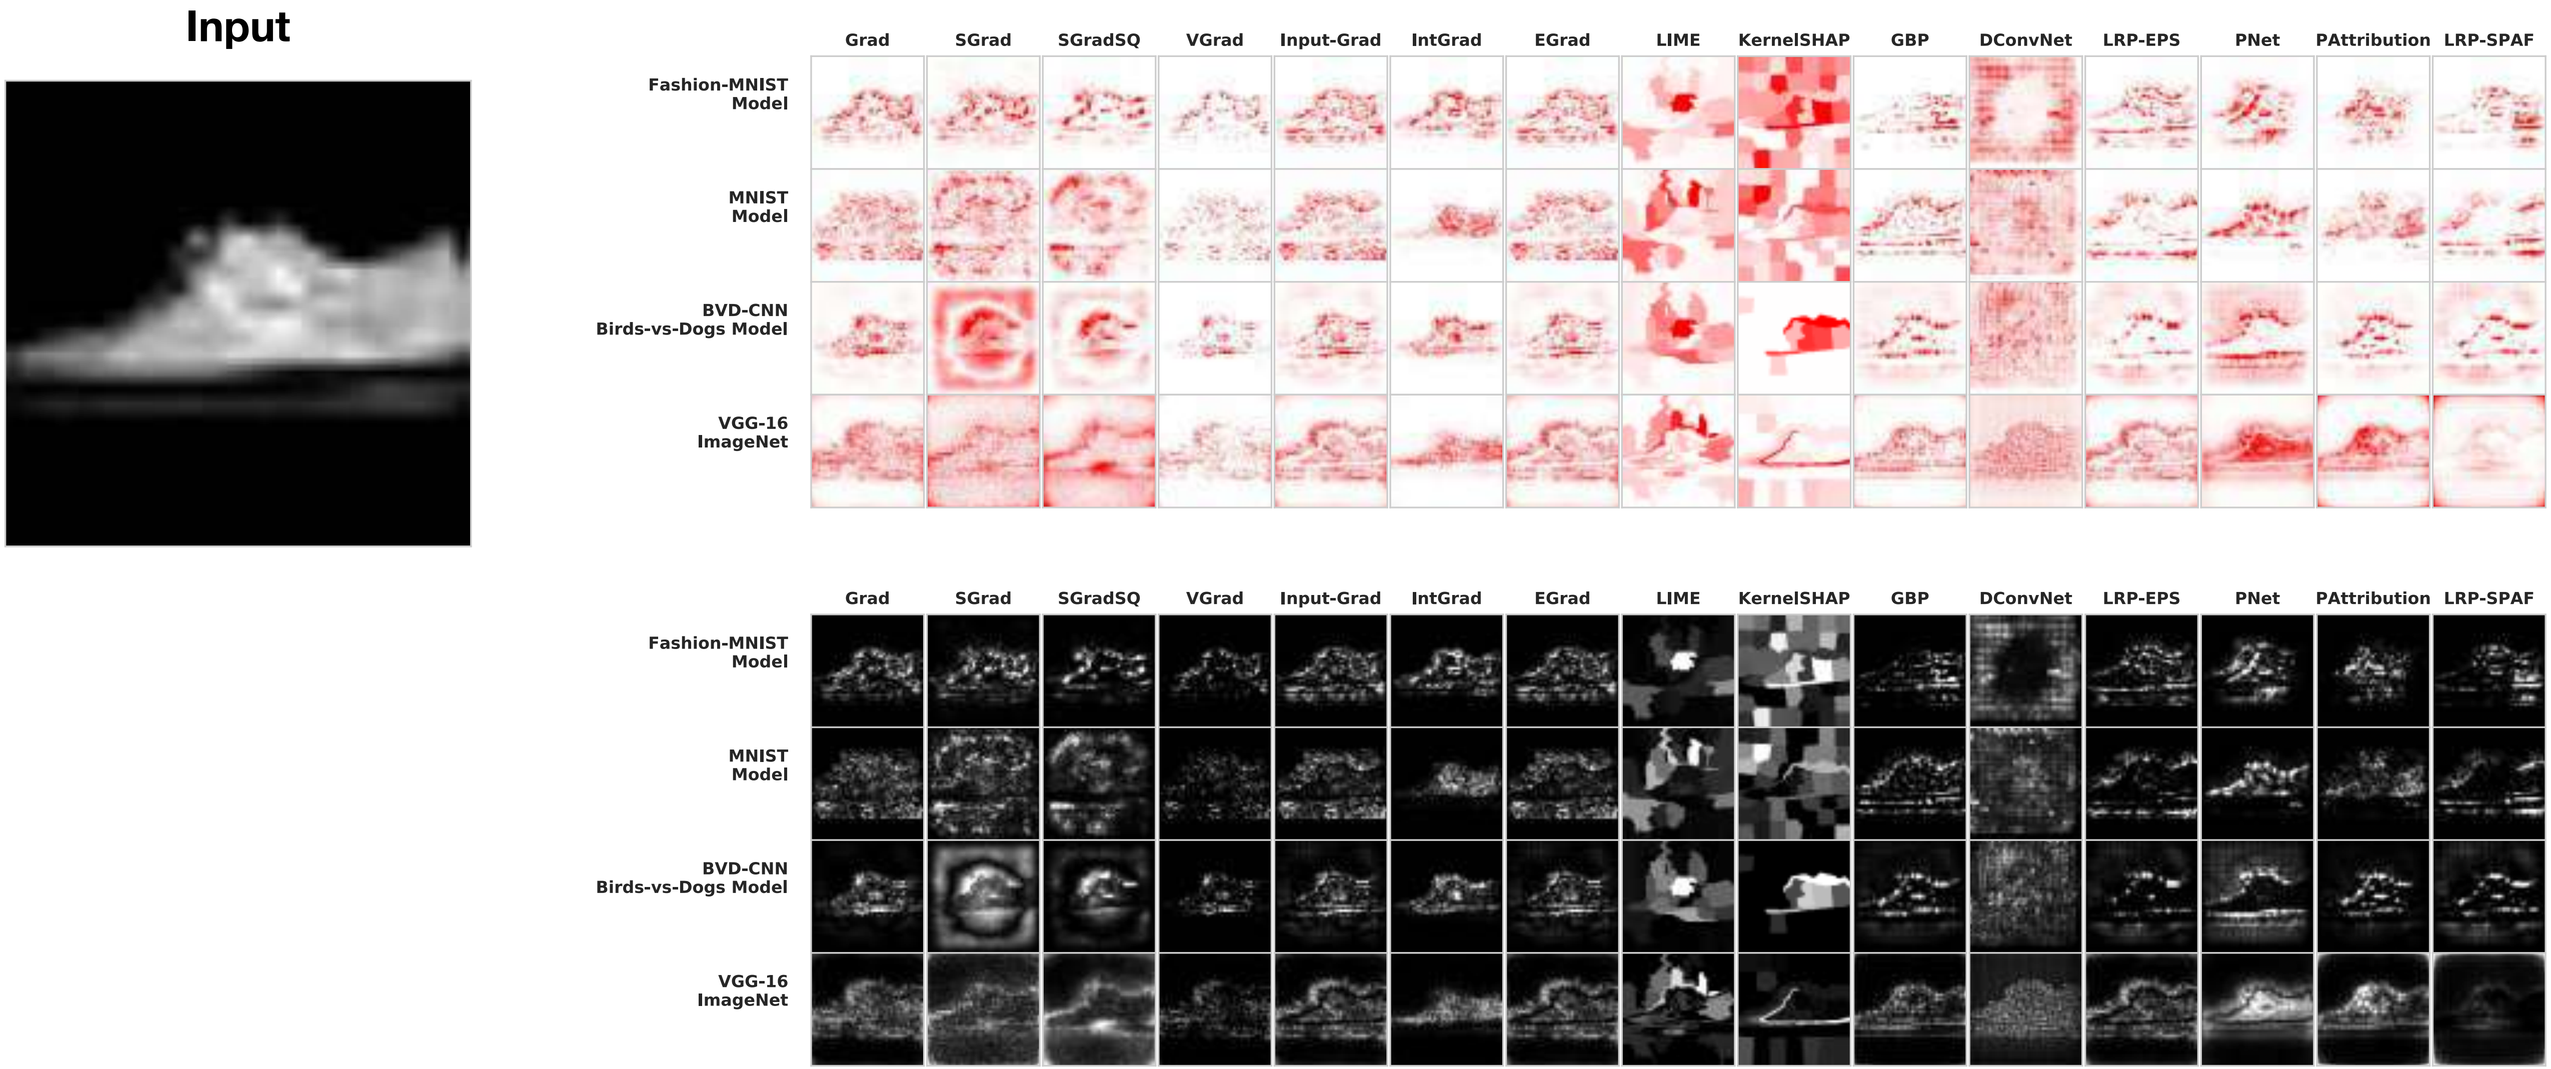

Input
Grad
SGrad
SGradSQ
VGrad
Input-Grad
IntGrad
EGrad
LIME
KernelSHAP
GBP
DConvNet
LRP-EPS
PNet
PAttribution
LRP-SPAF
Fashion-MNIST Model
MNIST Model
BVD-CNN Birds-vs-Dogs Model
VGG-16 ImageNet

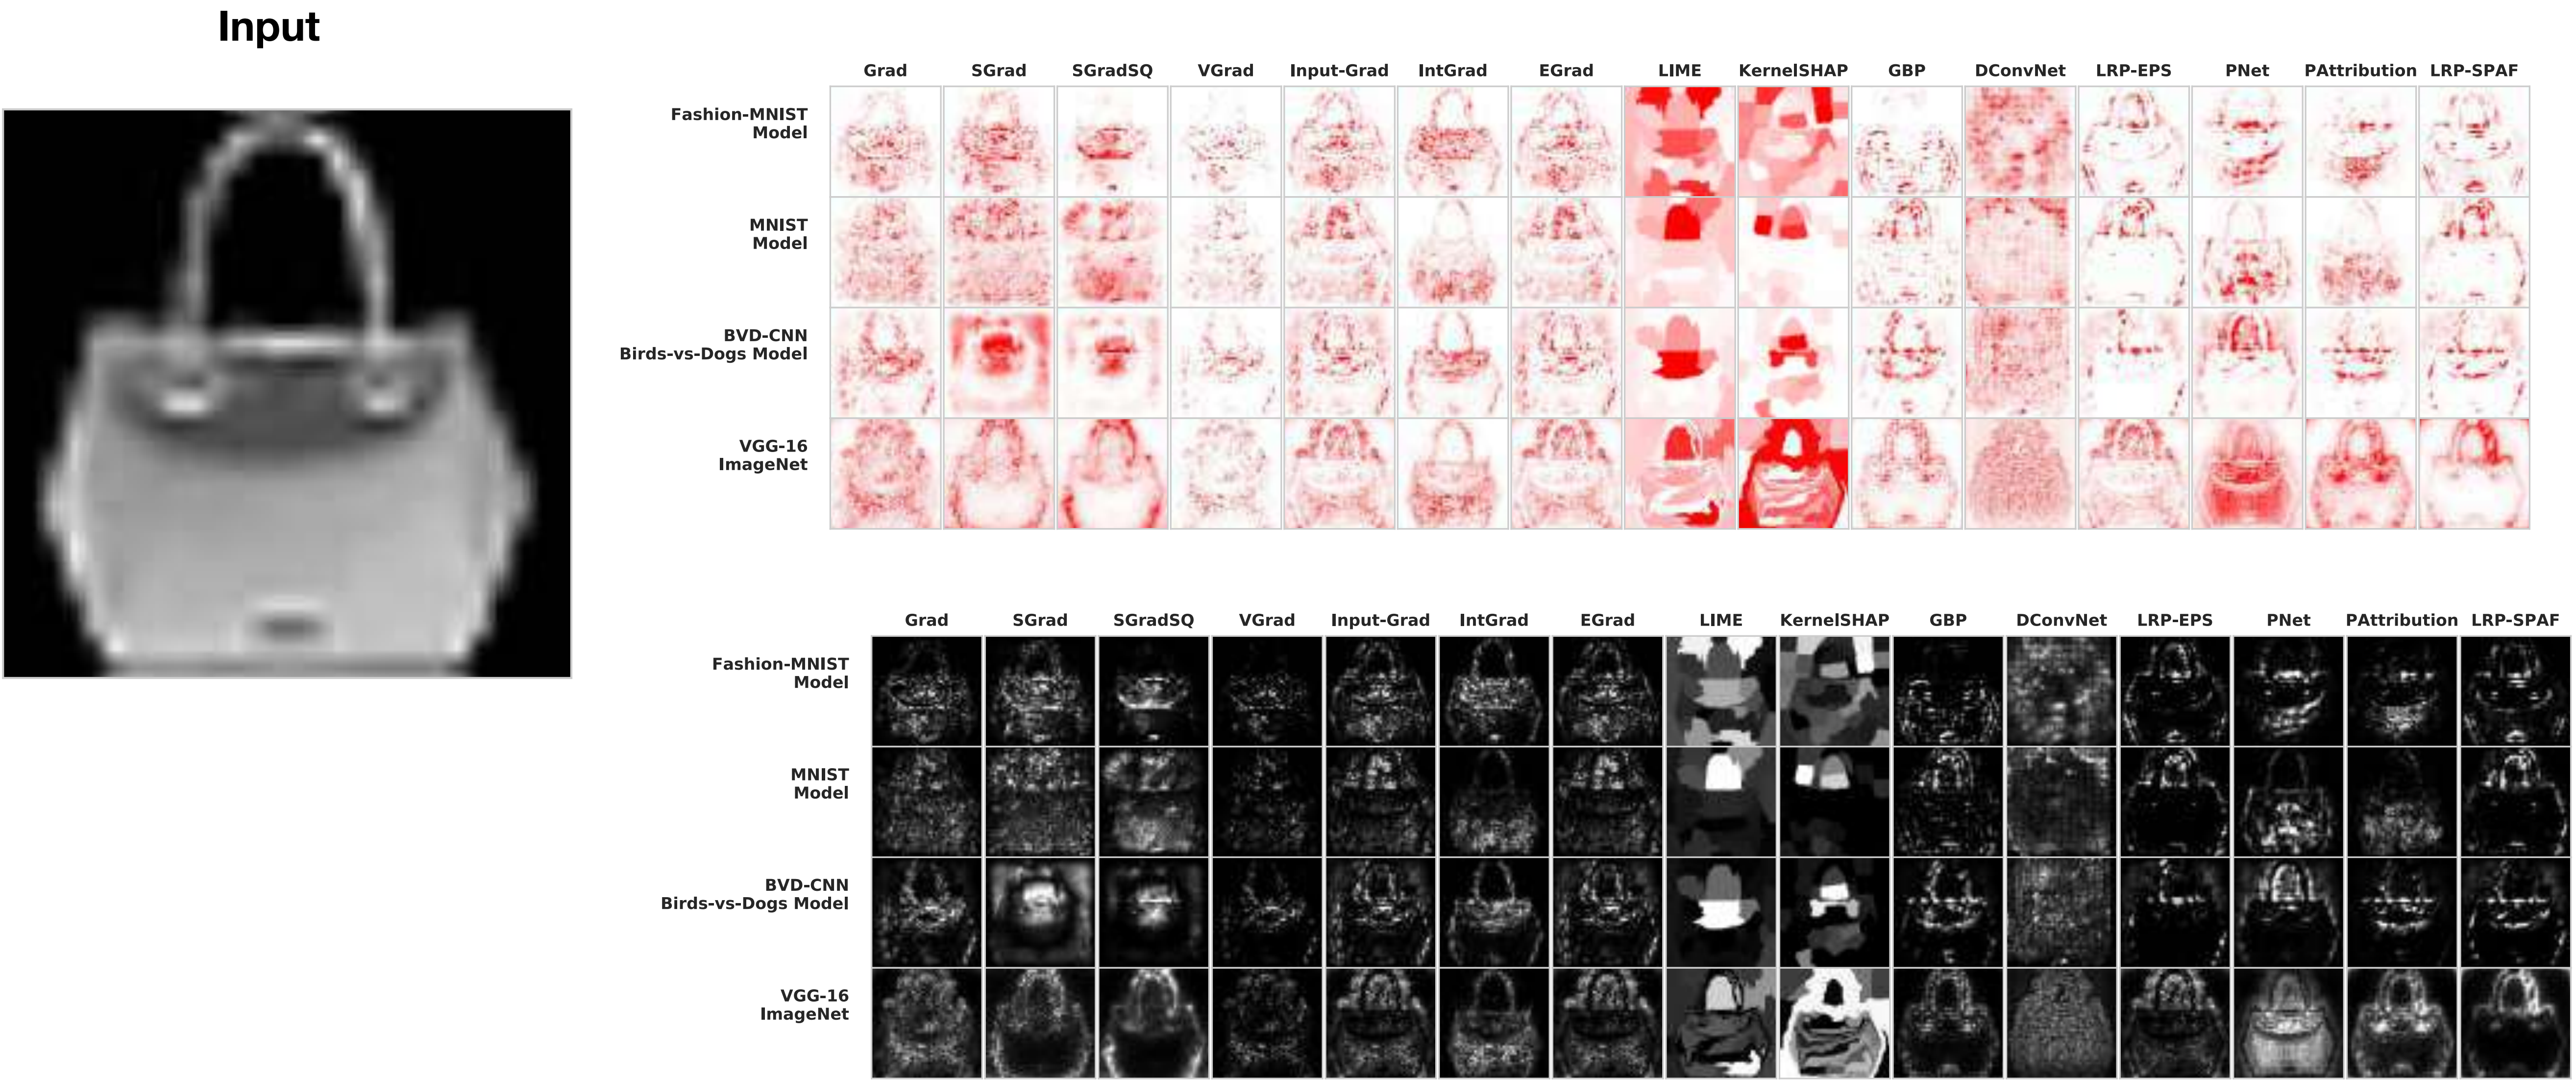
Input
Grad
SGrad
SGradSQ
VGrad
Input-Grad
IntGrad
EGrad
LIME
KernelSHAP
GBP
DConvNet
LRP-EPS
PNet
PAttribution
LRP-SPAF
Fashion-MNIST Model
MNIST Model
BVD-CNN Birds-vs-Dogs Model
VGG-16 ImageNet

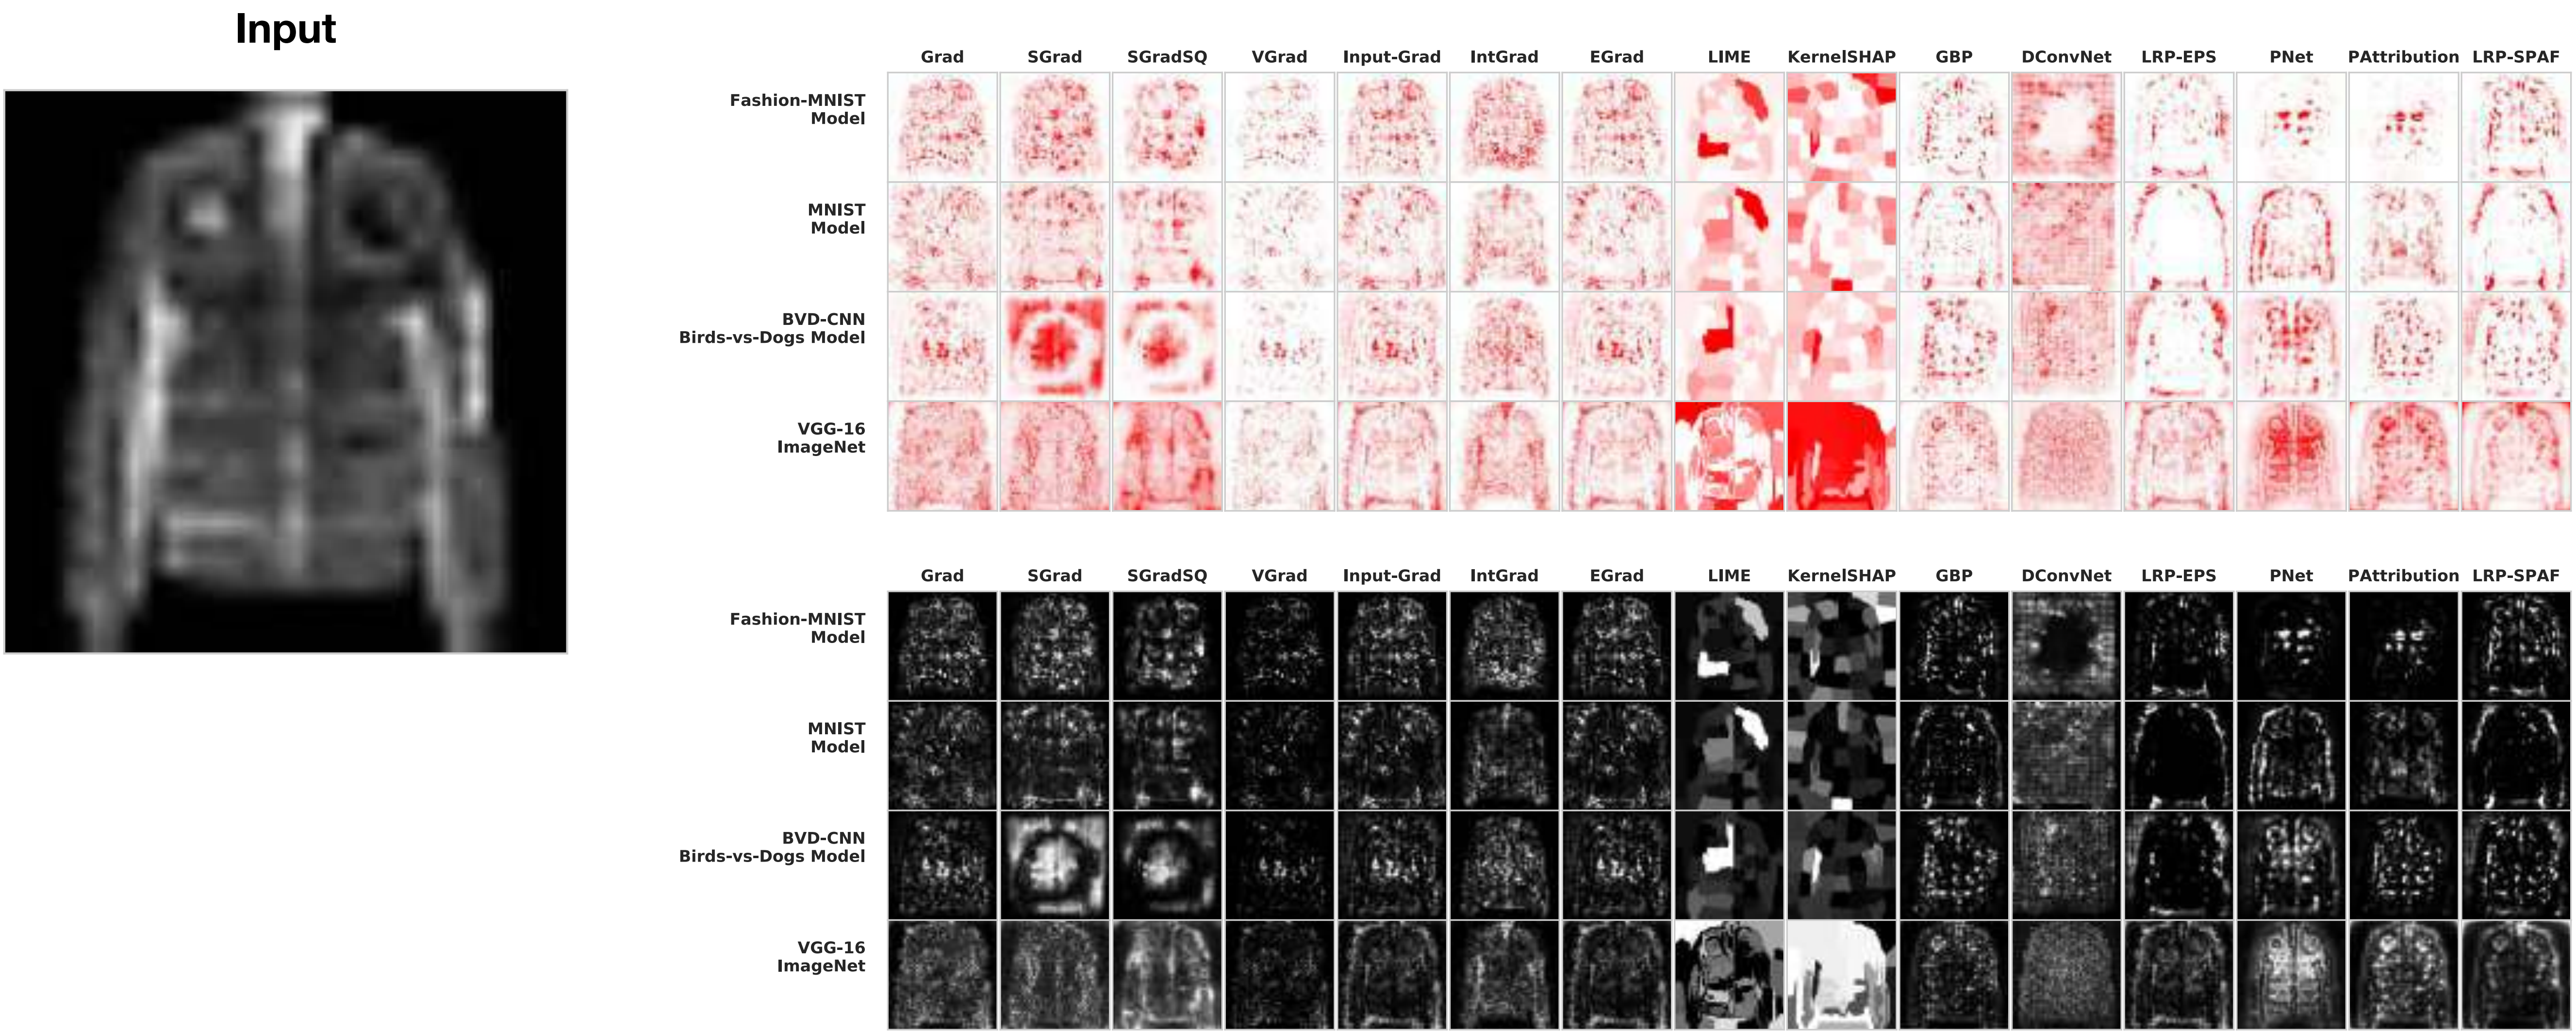
Input
Grad
SGrad
SGradSQ
VGrad
Input-Grad
IntGrad
EGrad
LIME
KernelSHAP
GBP
DConvNet
LRP-EPS
PNet
PAttribution
LRP-SPAF
Fashion-MNIST Model
MNIST Model
BVD-CNN Birds-vs-Dogs Model
VGG-16 ImageNet

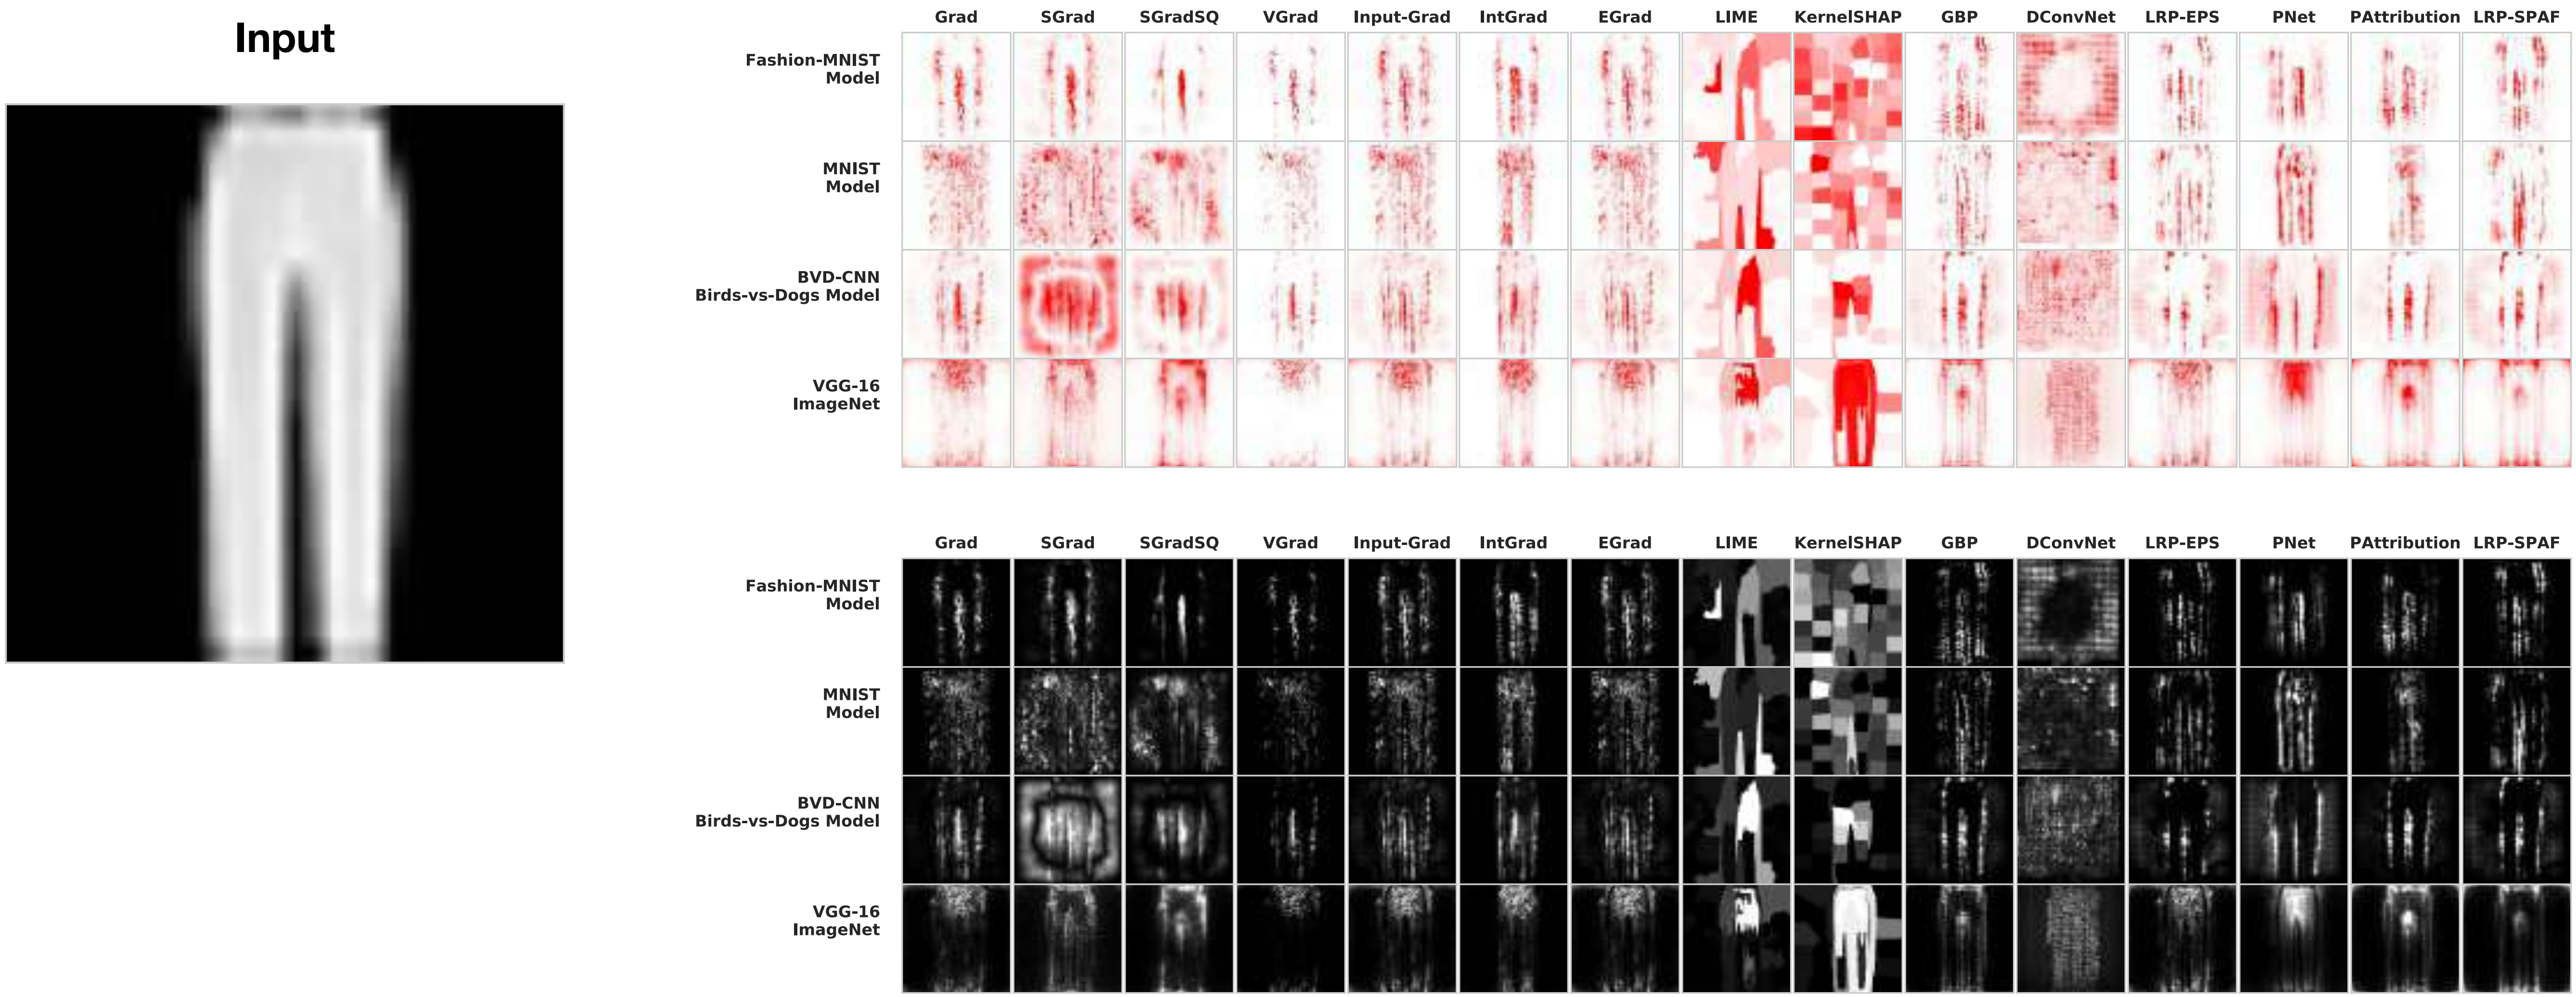
Input
Grad
SGrad
SGradSQ
VGrad
Input-Grad
IntGrad
EGrad
LIME
KernelSHAP
GBP
DConvNet
LRP-EPS
PNet
PAttribution
LRP-SPAF
Fashion-MNIST Model
MNIST Model
BVD-CNN Birds-vs-Dogs Model
VGG-16 ImageNet

# Appendix

# Overview of Methods

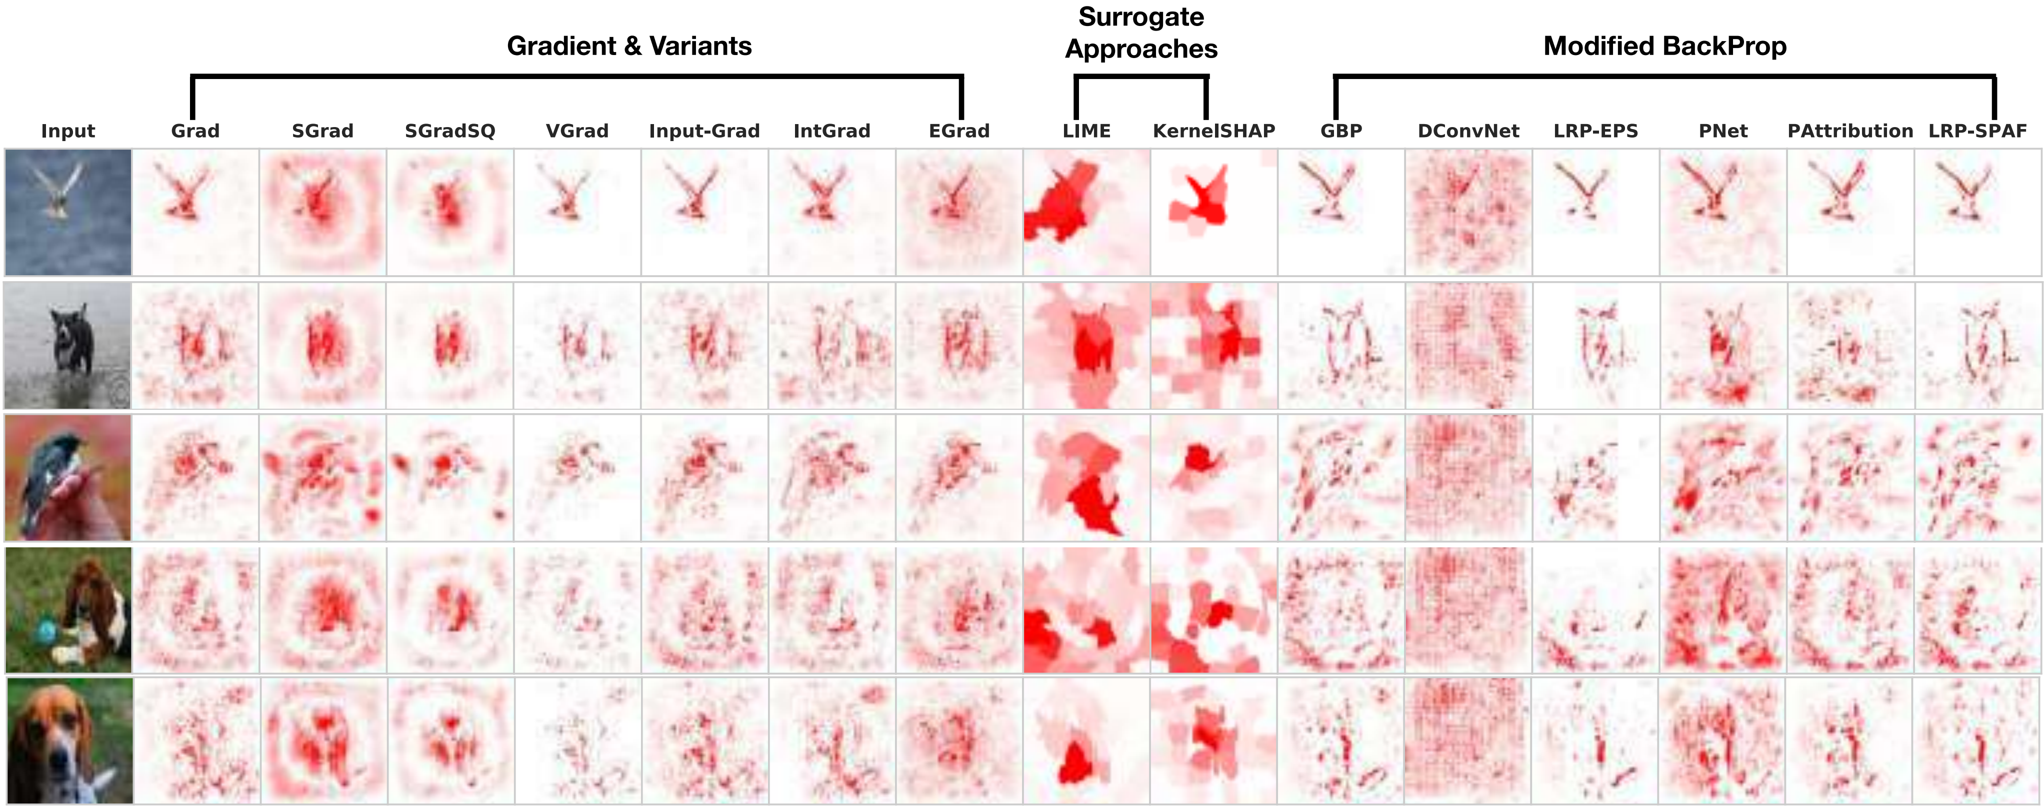

# Spurious Bird and Background Collection

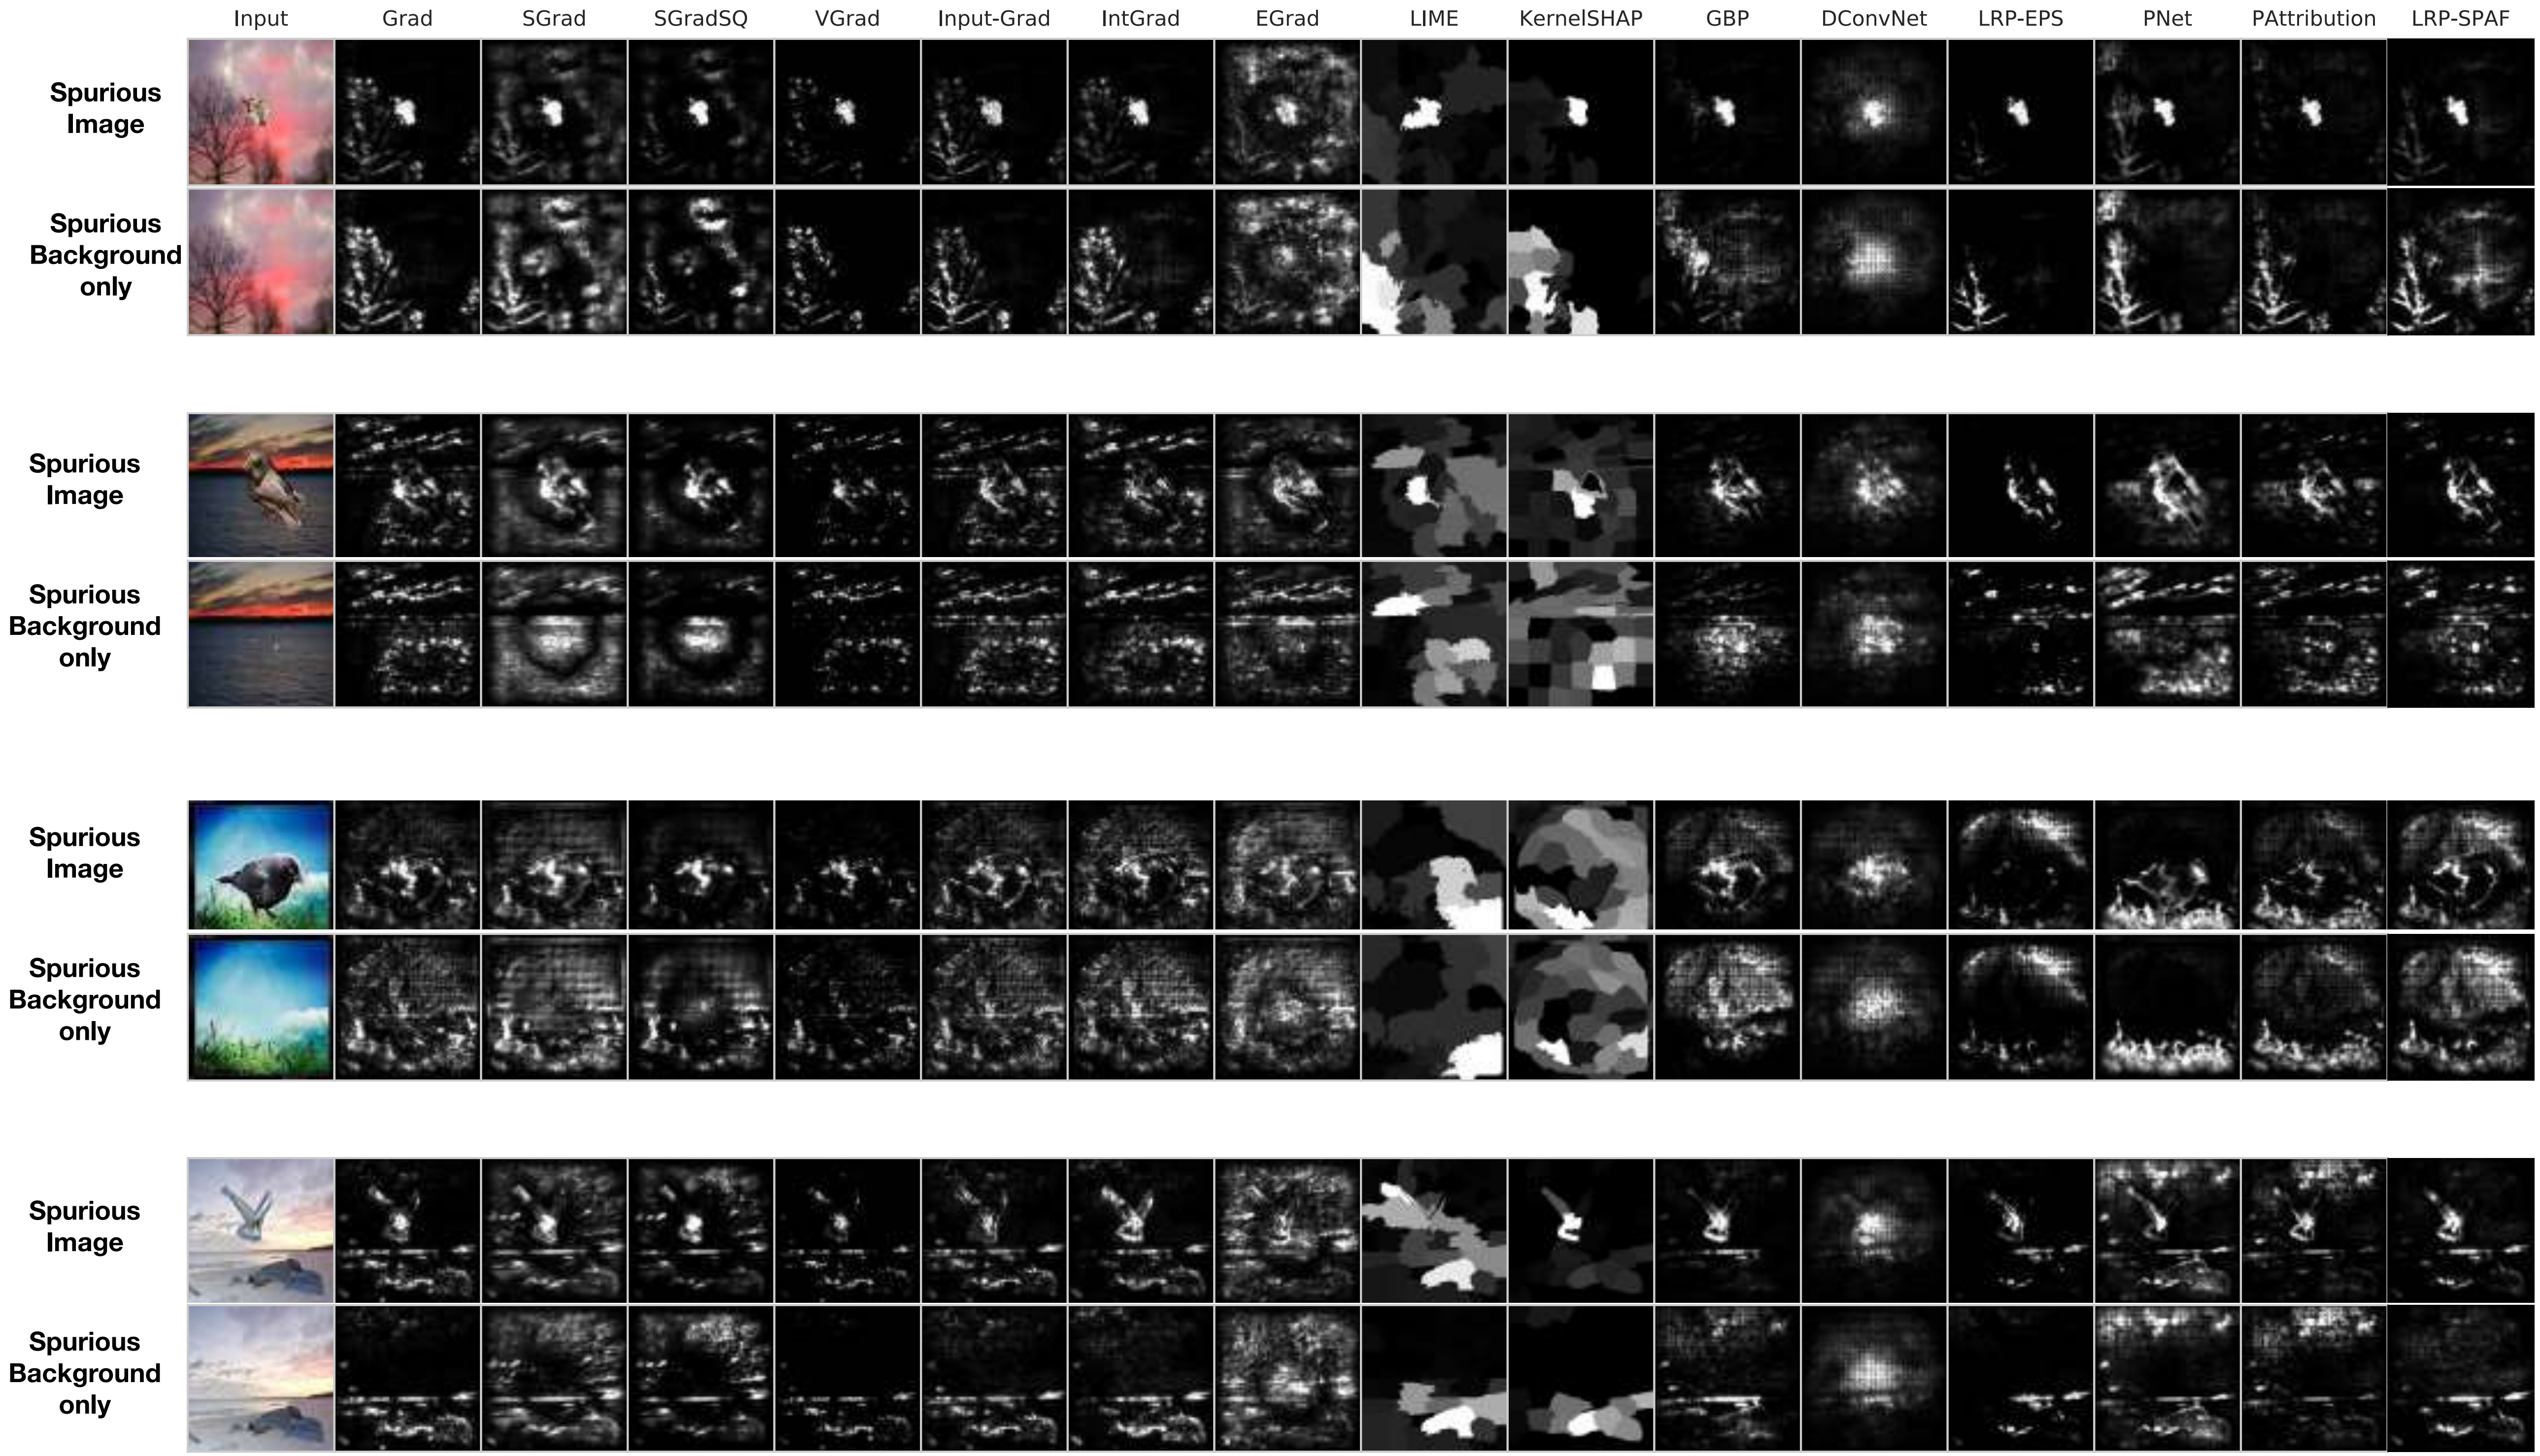

# Spurious Dog and Background Collection

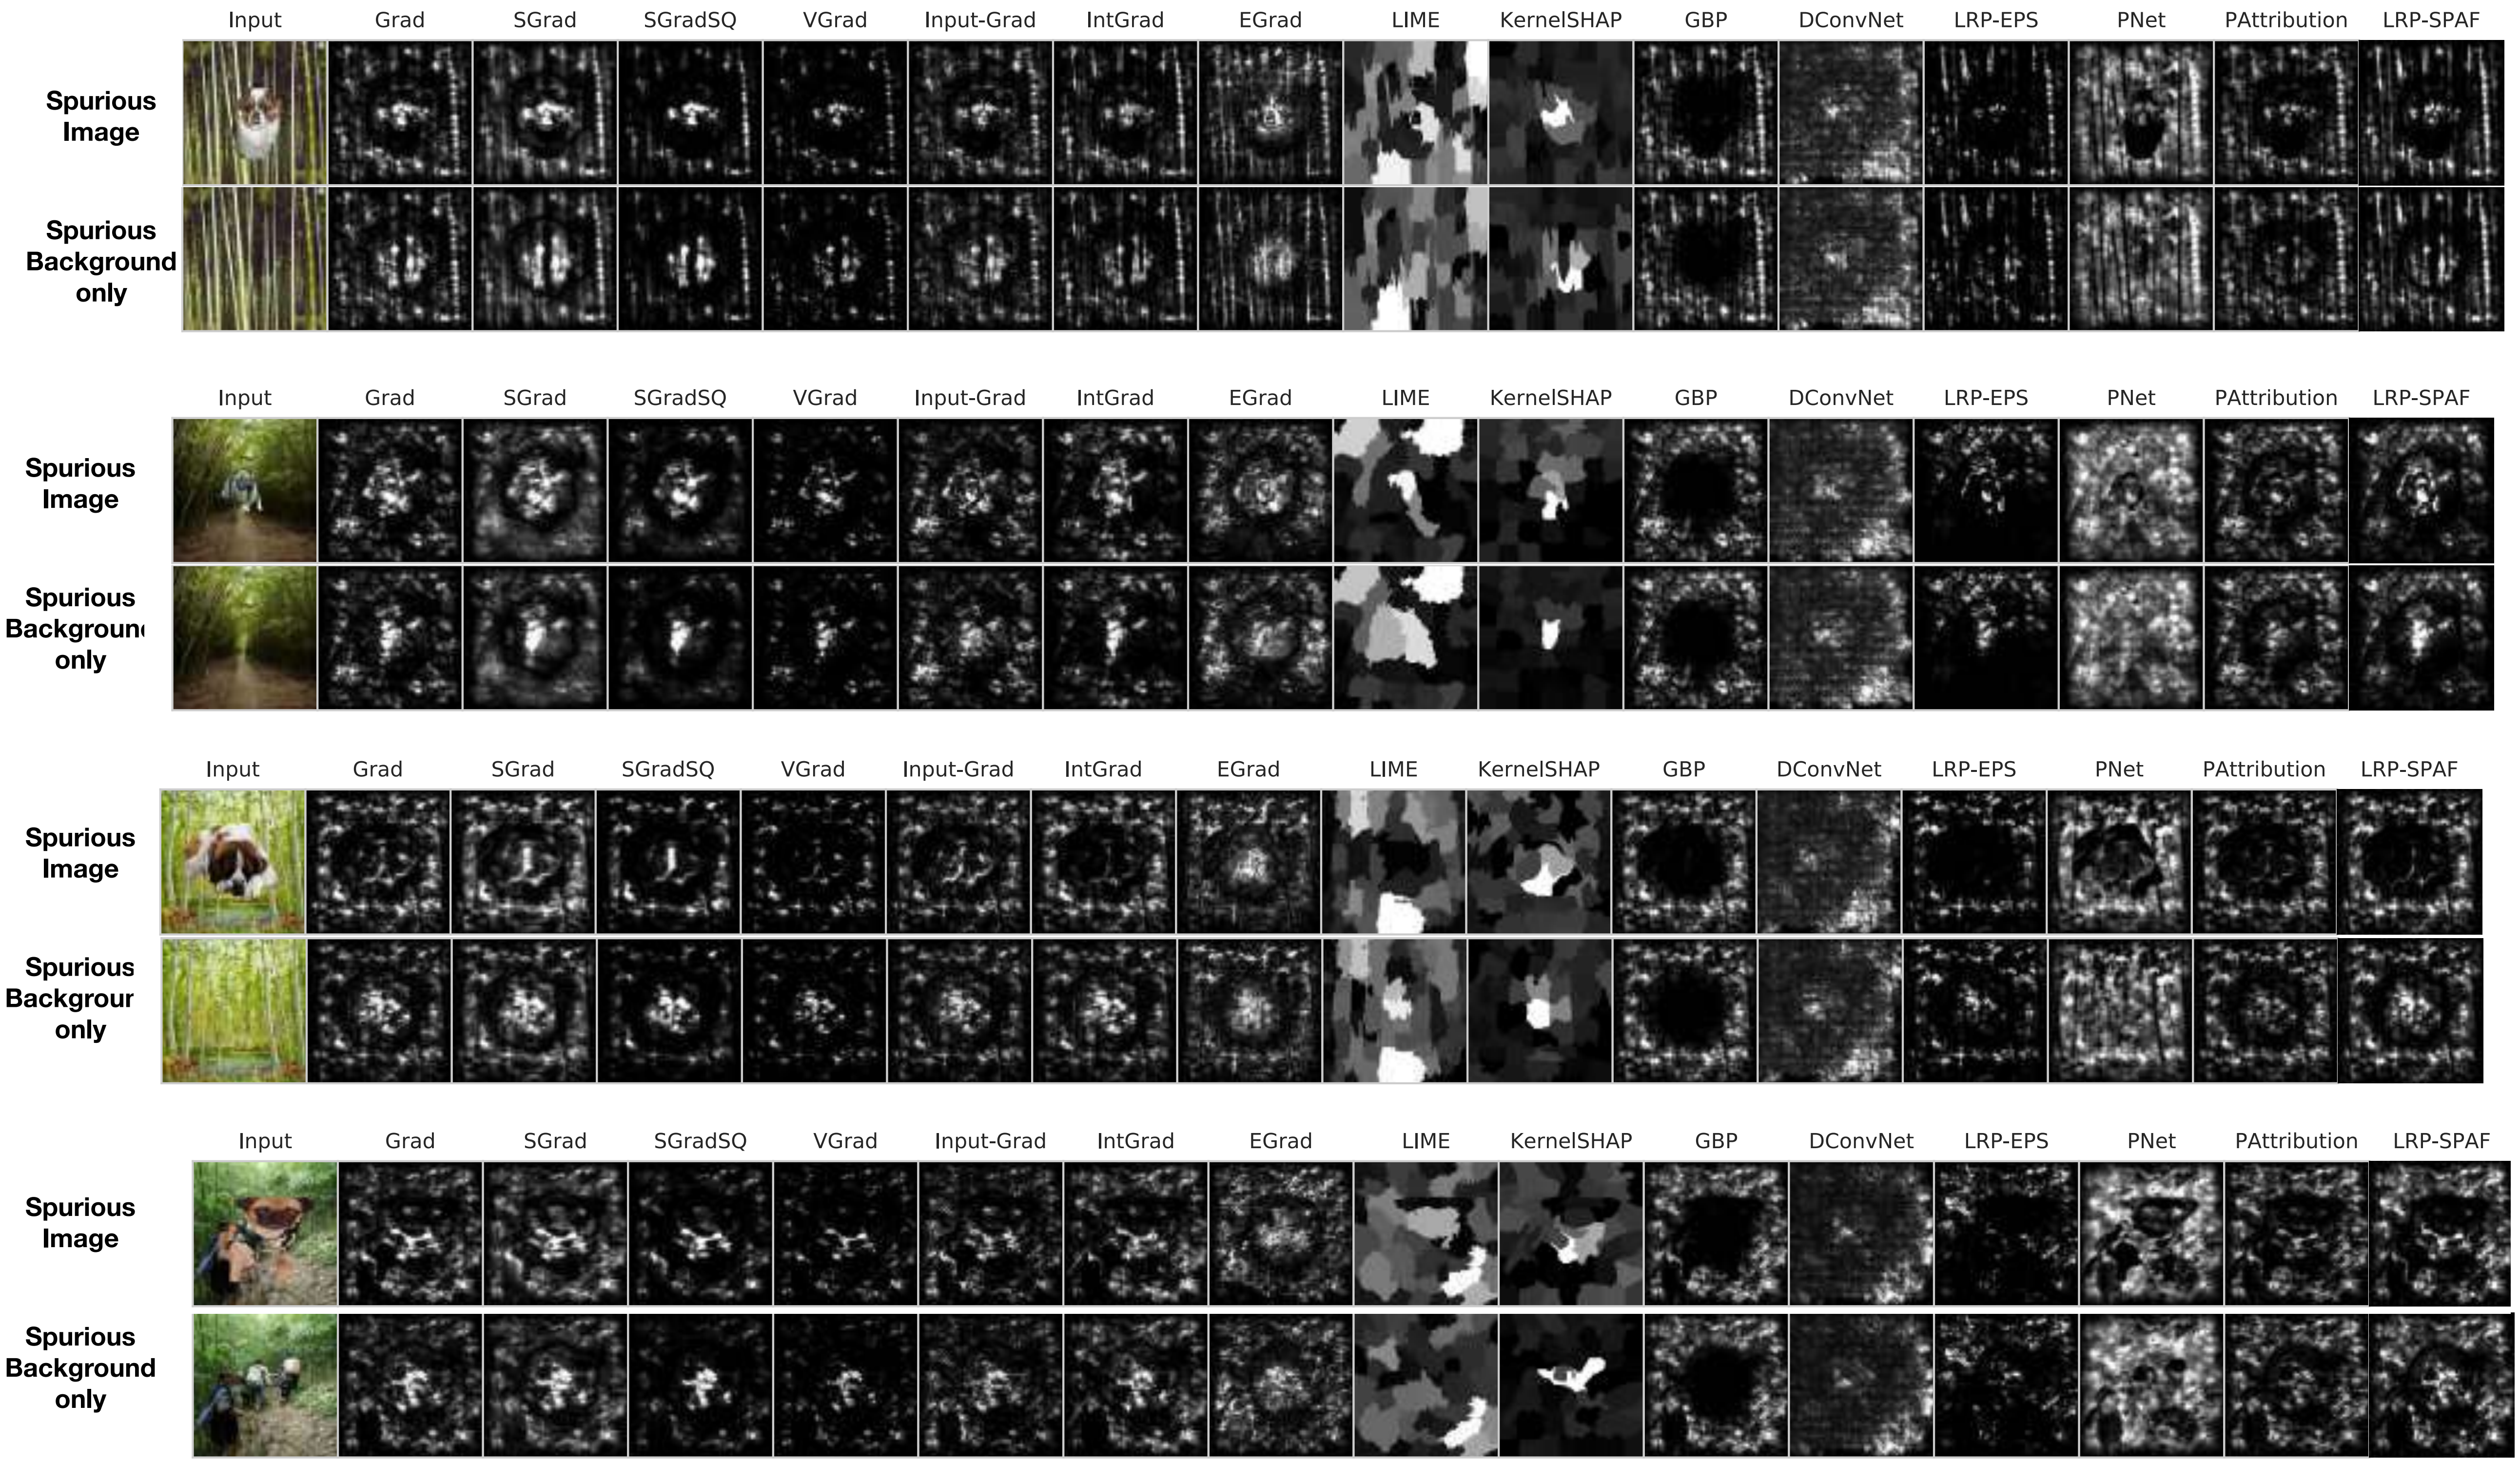

# Other Mislabeled Examples

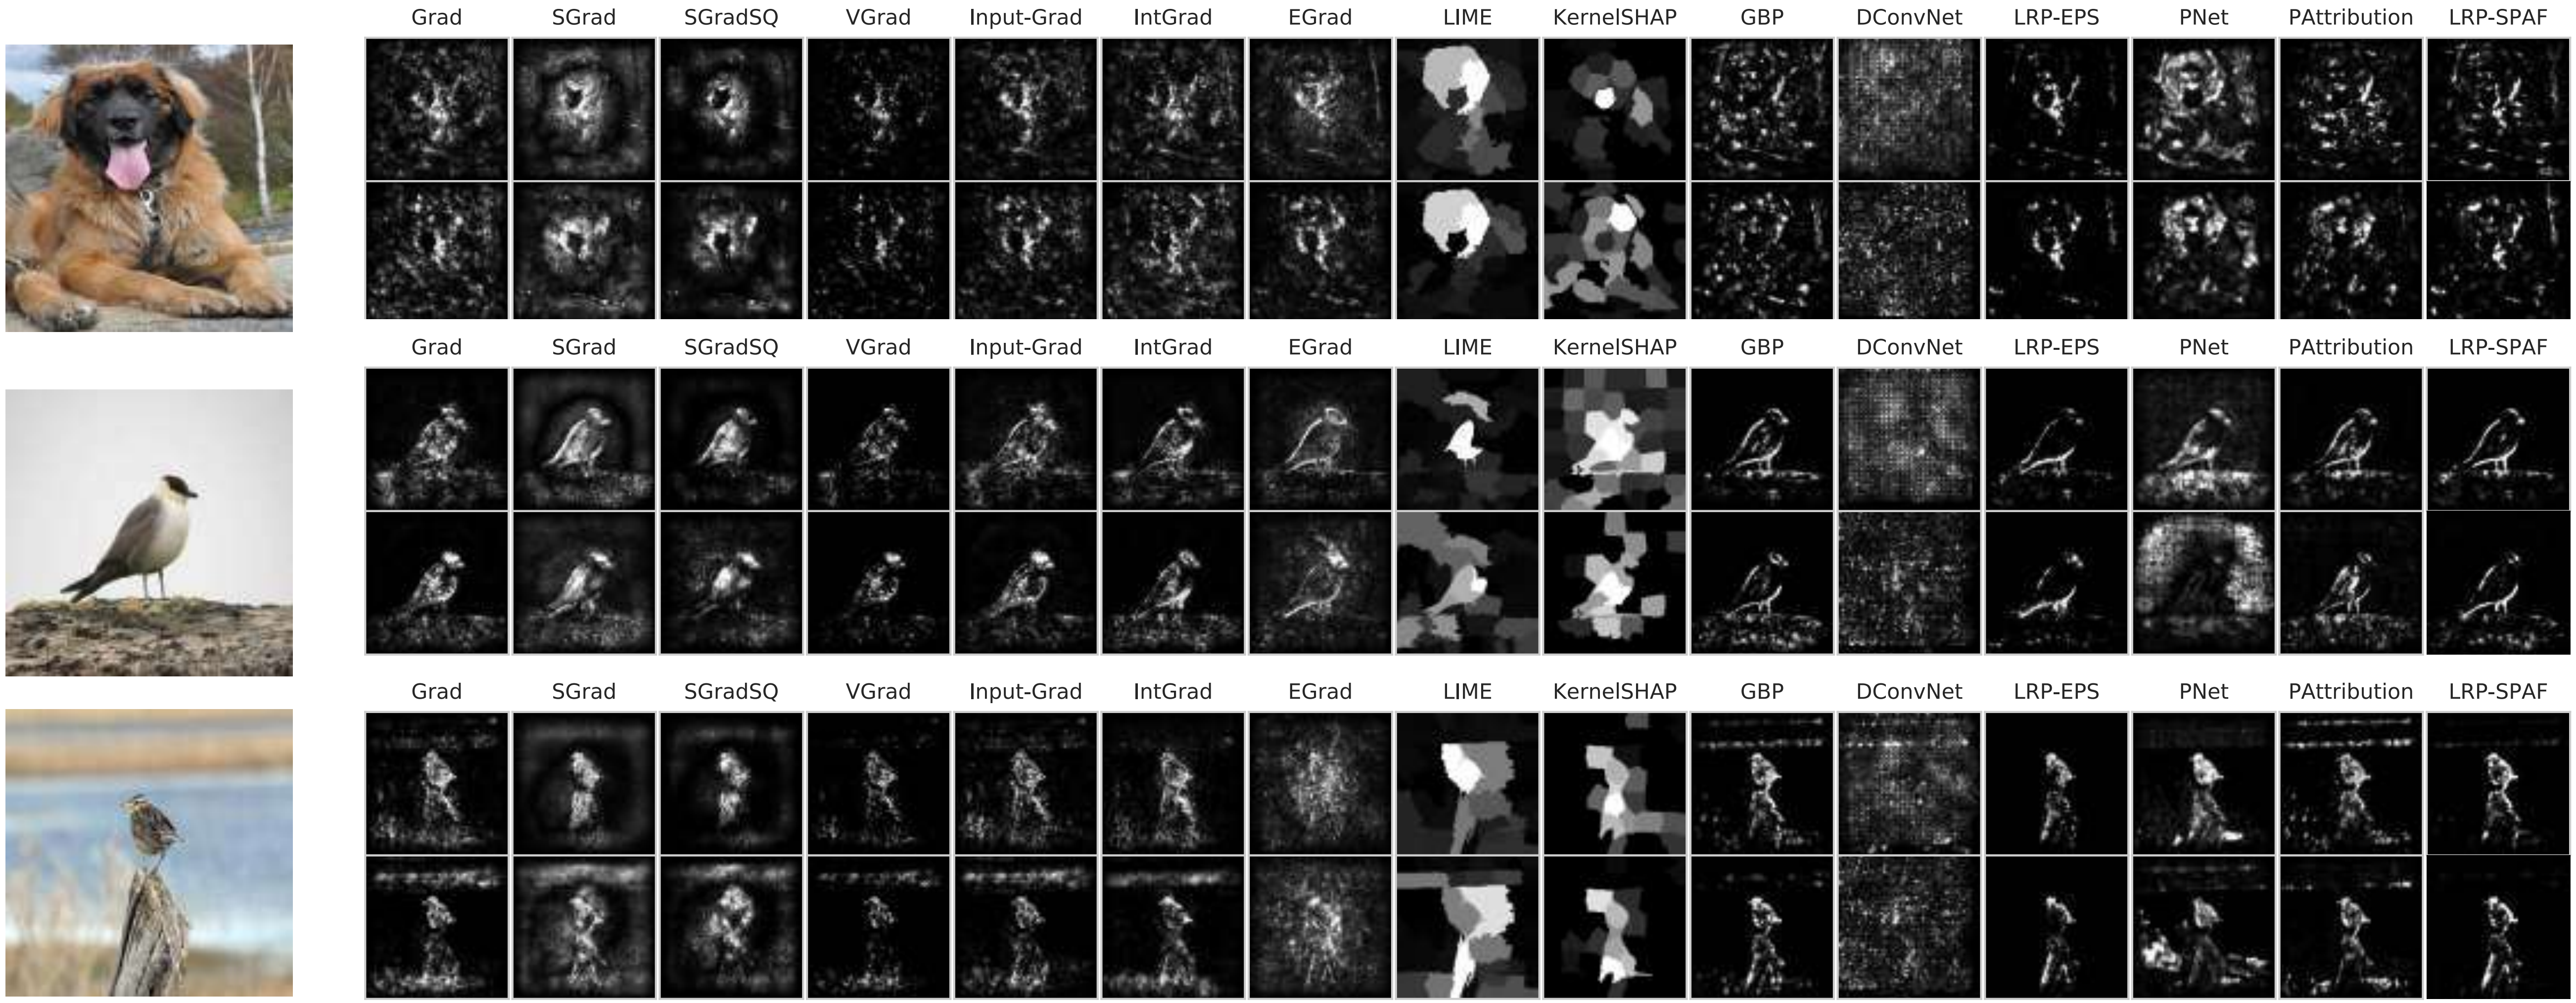


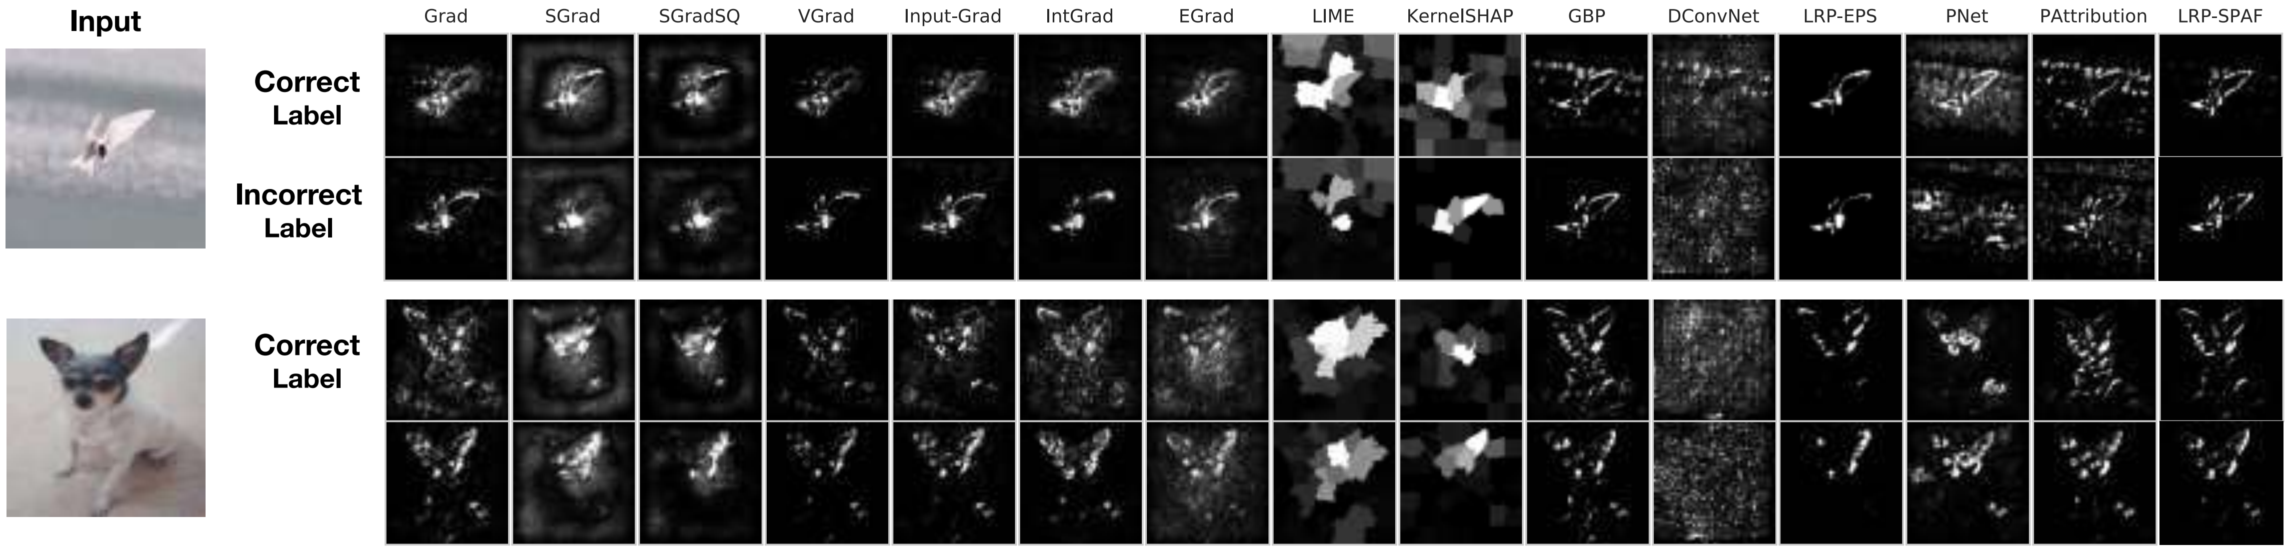


**Incorrect**

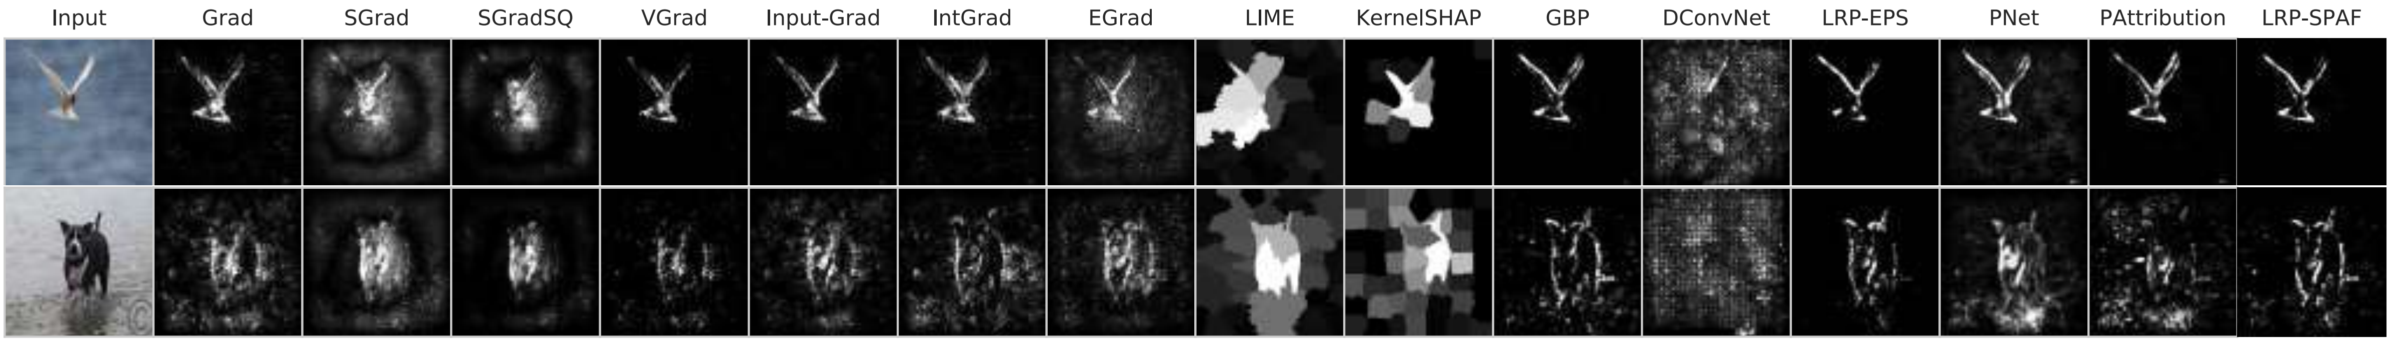
Input
Grad
SGrad
SGradSQ
VGrad
Input-Grad
IntGrad
EGrad
LIME
KernelSHAP
GBP
DConvNet
LRP-EPS
PNet
PAttribution
LRP-SPAF

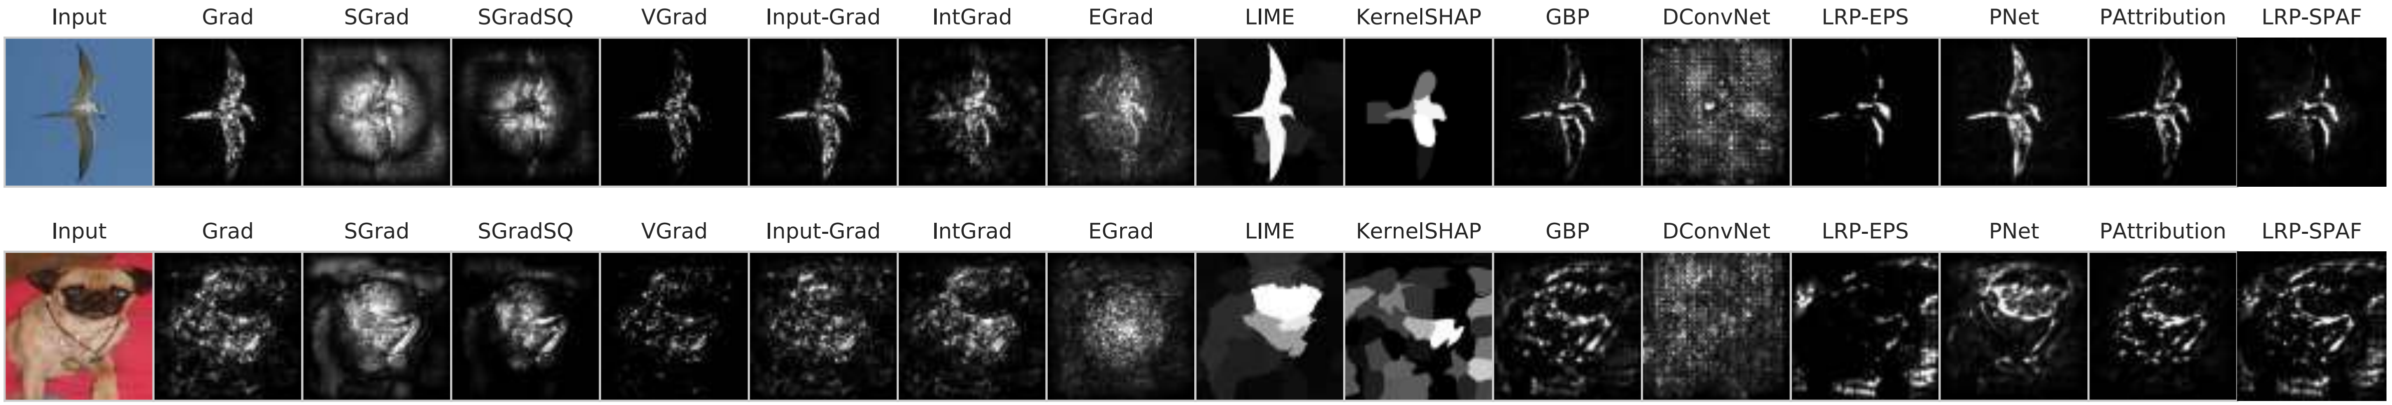
Input
Grad
SGrad
SGradSQ
VGrad
Input-Grad
IntGrad
EGrad
LIME
KernelSHAP
GBP
DConvNet
LRP-EPS
PNet
PAttribution
LRP-SPAF
Input
Grad
SGrad
SGradSQ
VGrad
Input-Grad
IntGrad
EGrad
LIME
KernelSHAP
GBP
DConvNet
LRP-EPS
PNet
PAttribution
LRP-SPAF

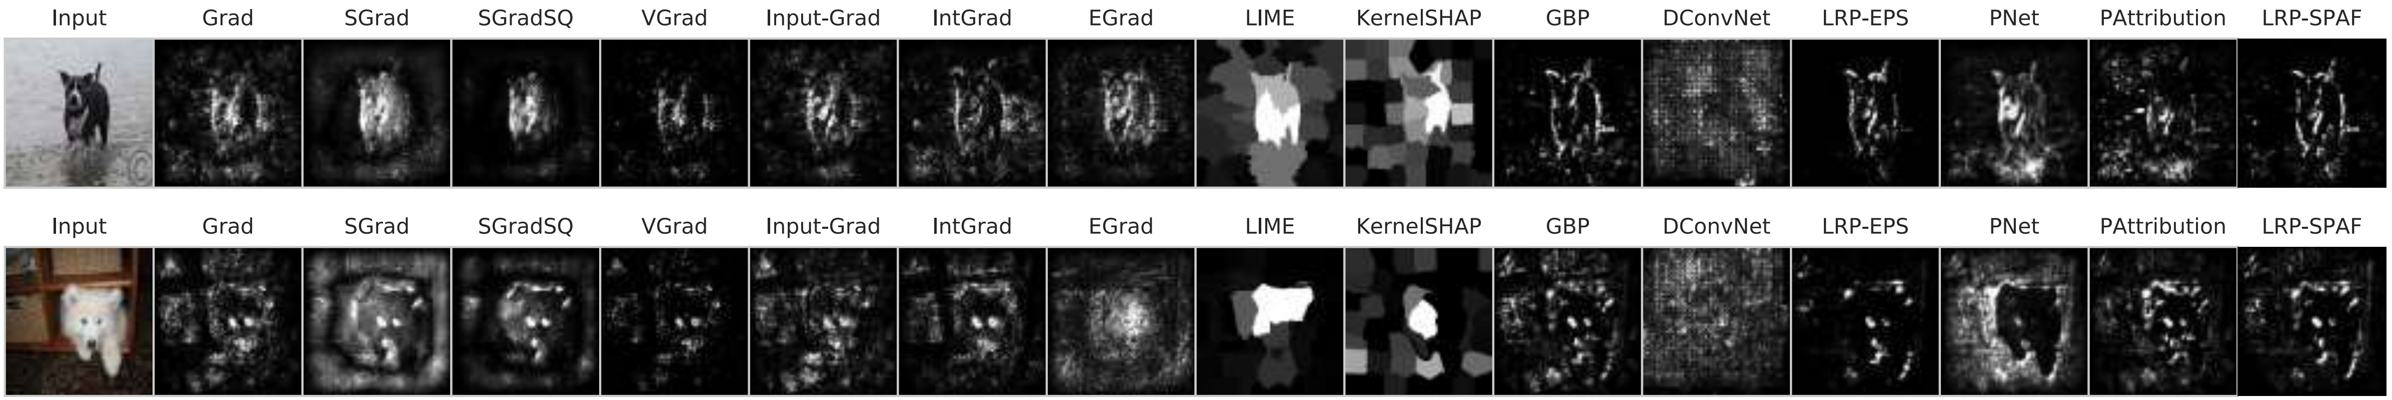
Input
Grad
SGrad
SGradSQ
VGrad
Input-Grad
IntGrad
EGrad
LIME
KernelSHAP
GBP
DConvNet
LRP-EPS
PNet
PAttribution
LRP-SPAF
Input
Grad
SGrad
SGradSQ
VGrad
Input-Grad
IntGrad
EGrad
LIME
KernelSHAP
GBP
DConvNet
LRP-EPS
PNet
PAttribution
LRP-SPAF

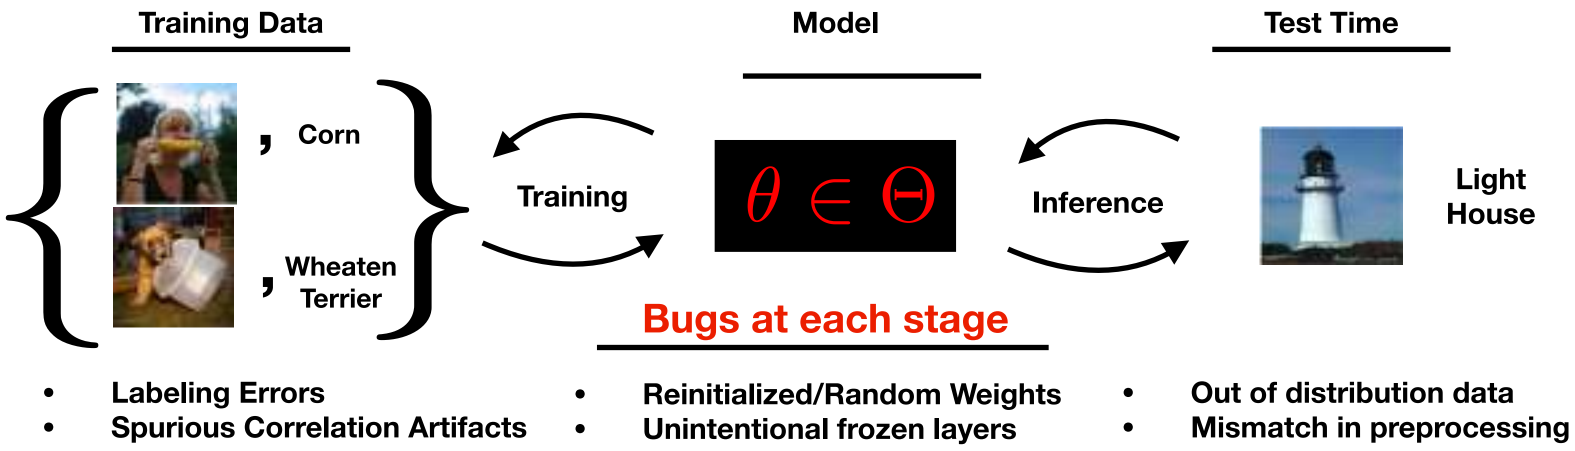
Training Data
Model
Test Time
, Corn
, Wheaten Terrier
Training
$\theta \in \Theta$
Inference
Light House
Bugs at each stage
Labeling Errors
Spurious Correlation Artifacts
Reinitialized/Random Weights
Unintentional frozen layers
Out of distribution data
Mismatch in preprocessing

# Debugging Framework for Supervised Learning

**Learning Phase**

$$\underbrace{\arg\min_{f_\theta}}_{\text{Model Contamination Bug}} \frac{1}{n}\sum_{i}^{n} \ell\Big(\overbrace{(x_{\text{train}}, y_{\text{train}})}^{\text{Data Contamination Bug}}; f_\theta\Big);$$

**Prediction Phase**

$$y_{\text{test}} = f_\theta\Big(\overbrace{x_{\text{test}}}^{\text{Test-Time Contamination Bug}}\Big)$$

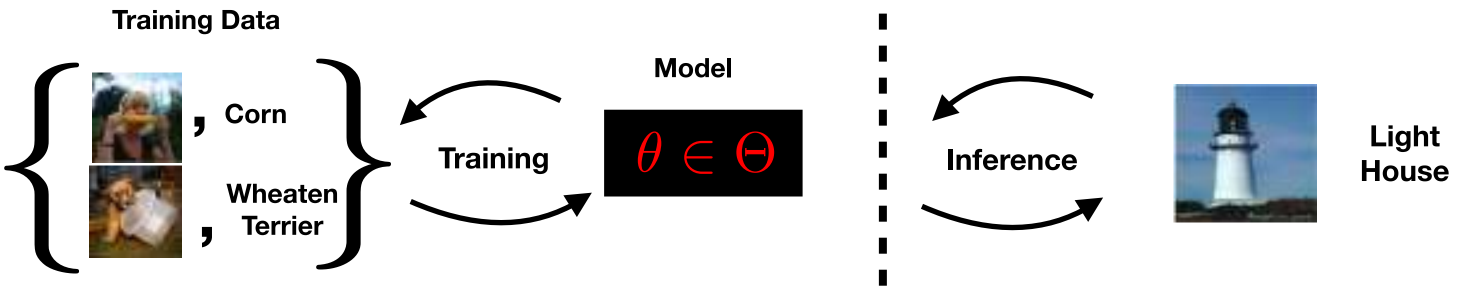


- Labeling Errors
- Spurious Correlation

- Reinitialized Weights
- Unintentional frozen layers

- Out of distribution data
- Mismatch in preprocessing

# Debugging Framework for Supervised Learning

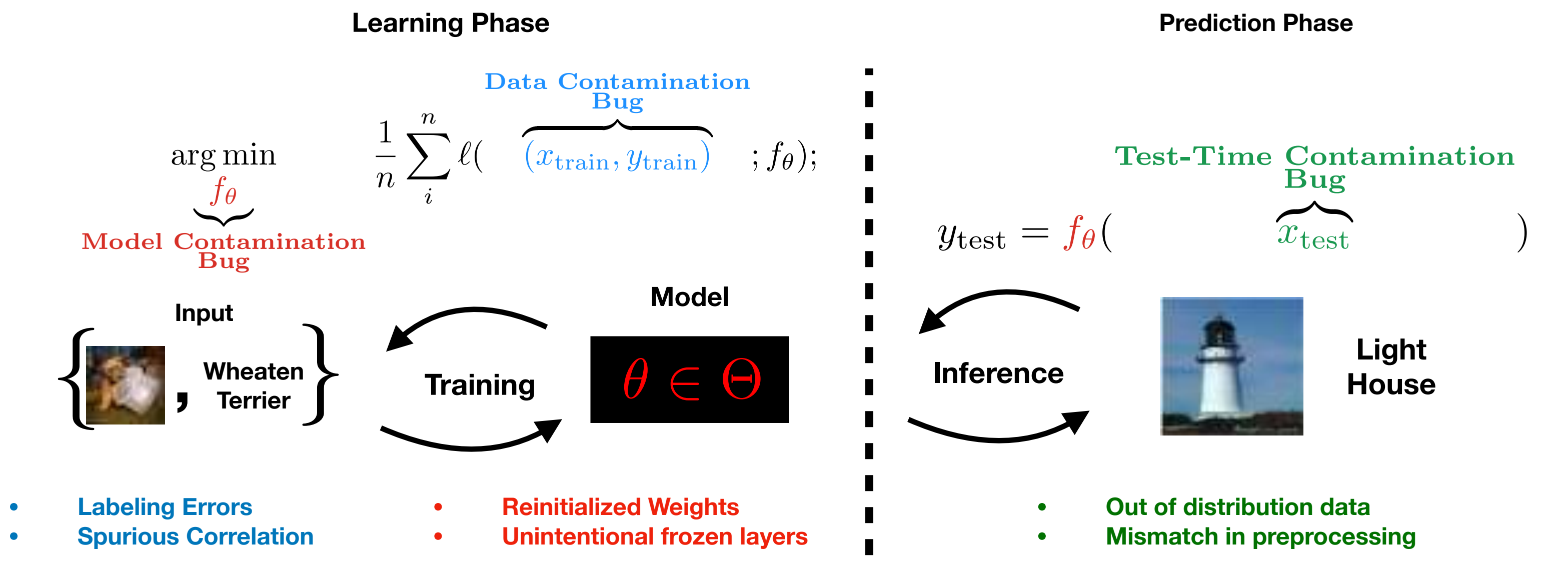

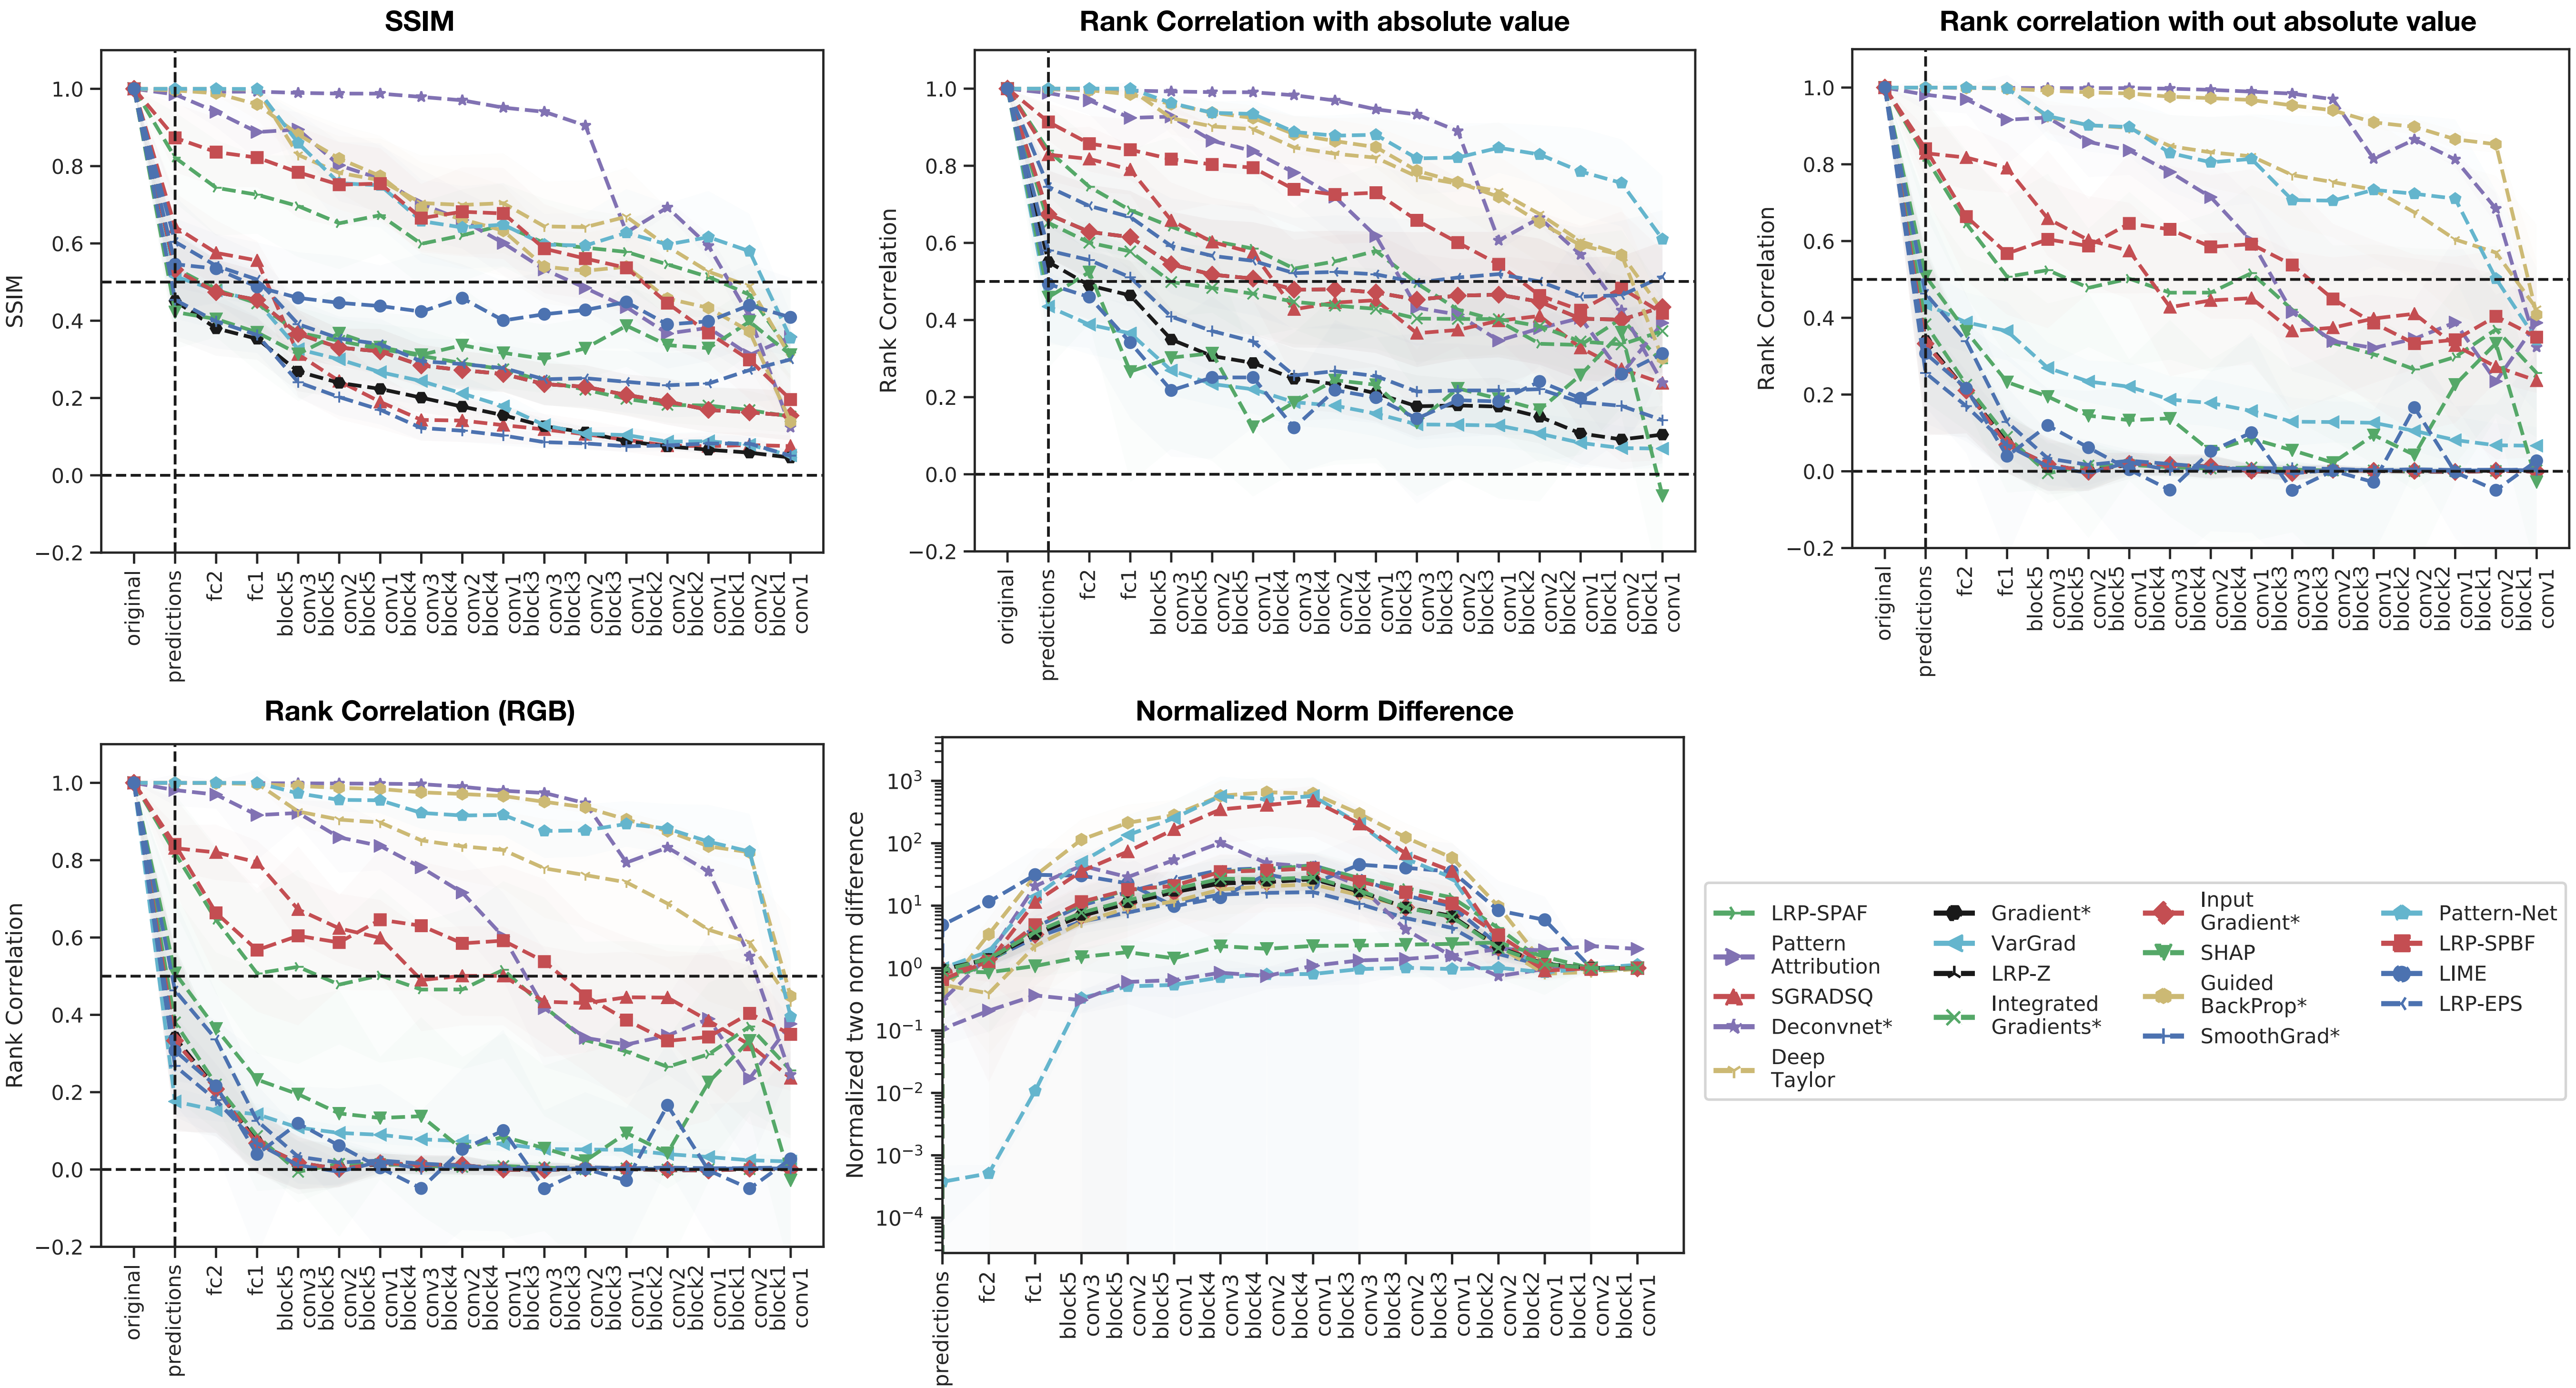
SSIM
Rank Correlation with absolute value
Rank correlation with out absolute value
Rank Correlation (RGB)
Normalized Norm Difference
SSIM
Rank Correlation
Normalized two norm difference
original
predictions
fc2
fc1
block5 conv3
block5 conv2
block5 conv1
block4 conv3
block4 conv2
block4 conv1
block3 conv3
block3 conv2
block3 conv1
block2 conv2
block2 conv1
block1 conv2
block1 conv1
LRP-SPAF
Pattern Attribution
SGRADSQ
Deconvnet*
Deep Taylor
Gradient*
VarGrad
LRP-Z
Integrated Gradients*
Input Gradient*
SHAP
Guided BackProp*
SmoothGrad*
Pattern-Net
LRP-SPBF
LIME
LRP-EPS

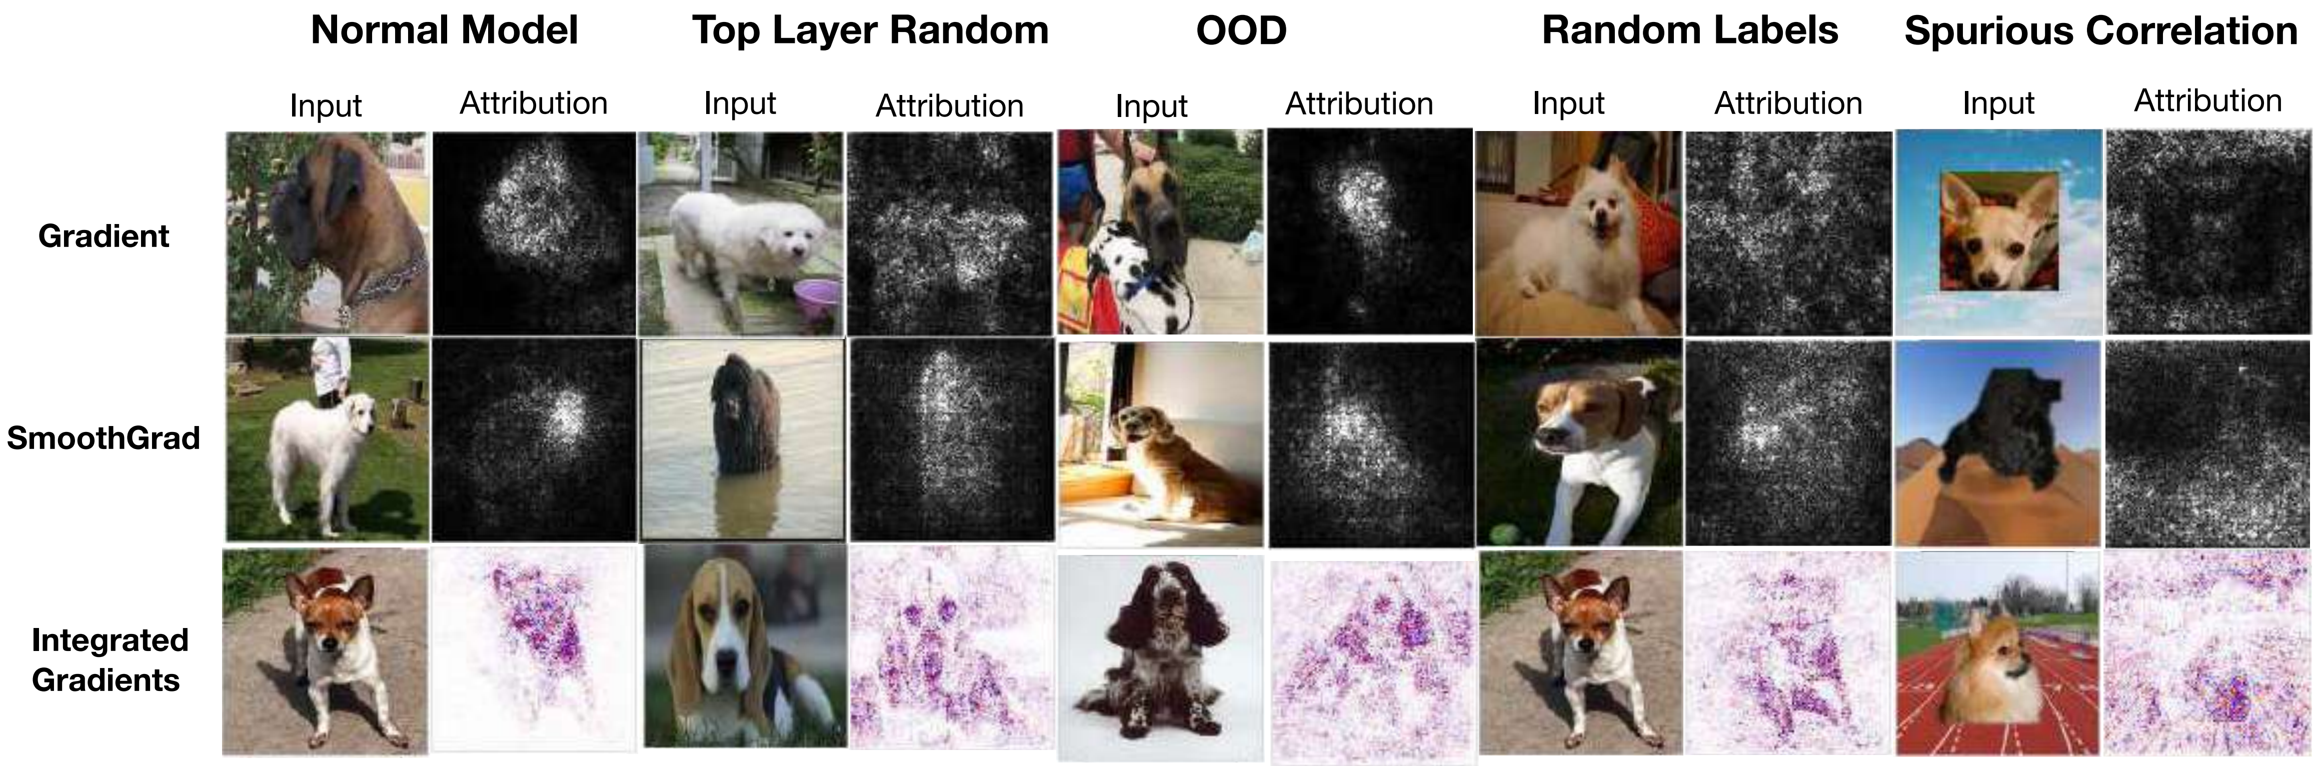
Normal Model
Top Layer Random
OOD
Random Labels
Spurious Correlation
Input
Attribution
Gradient
SmoothGrad
Integrated Gradients

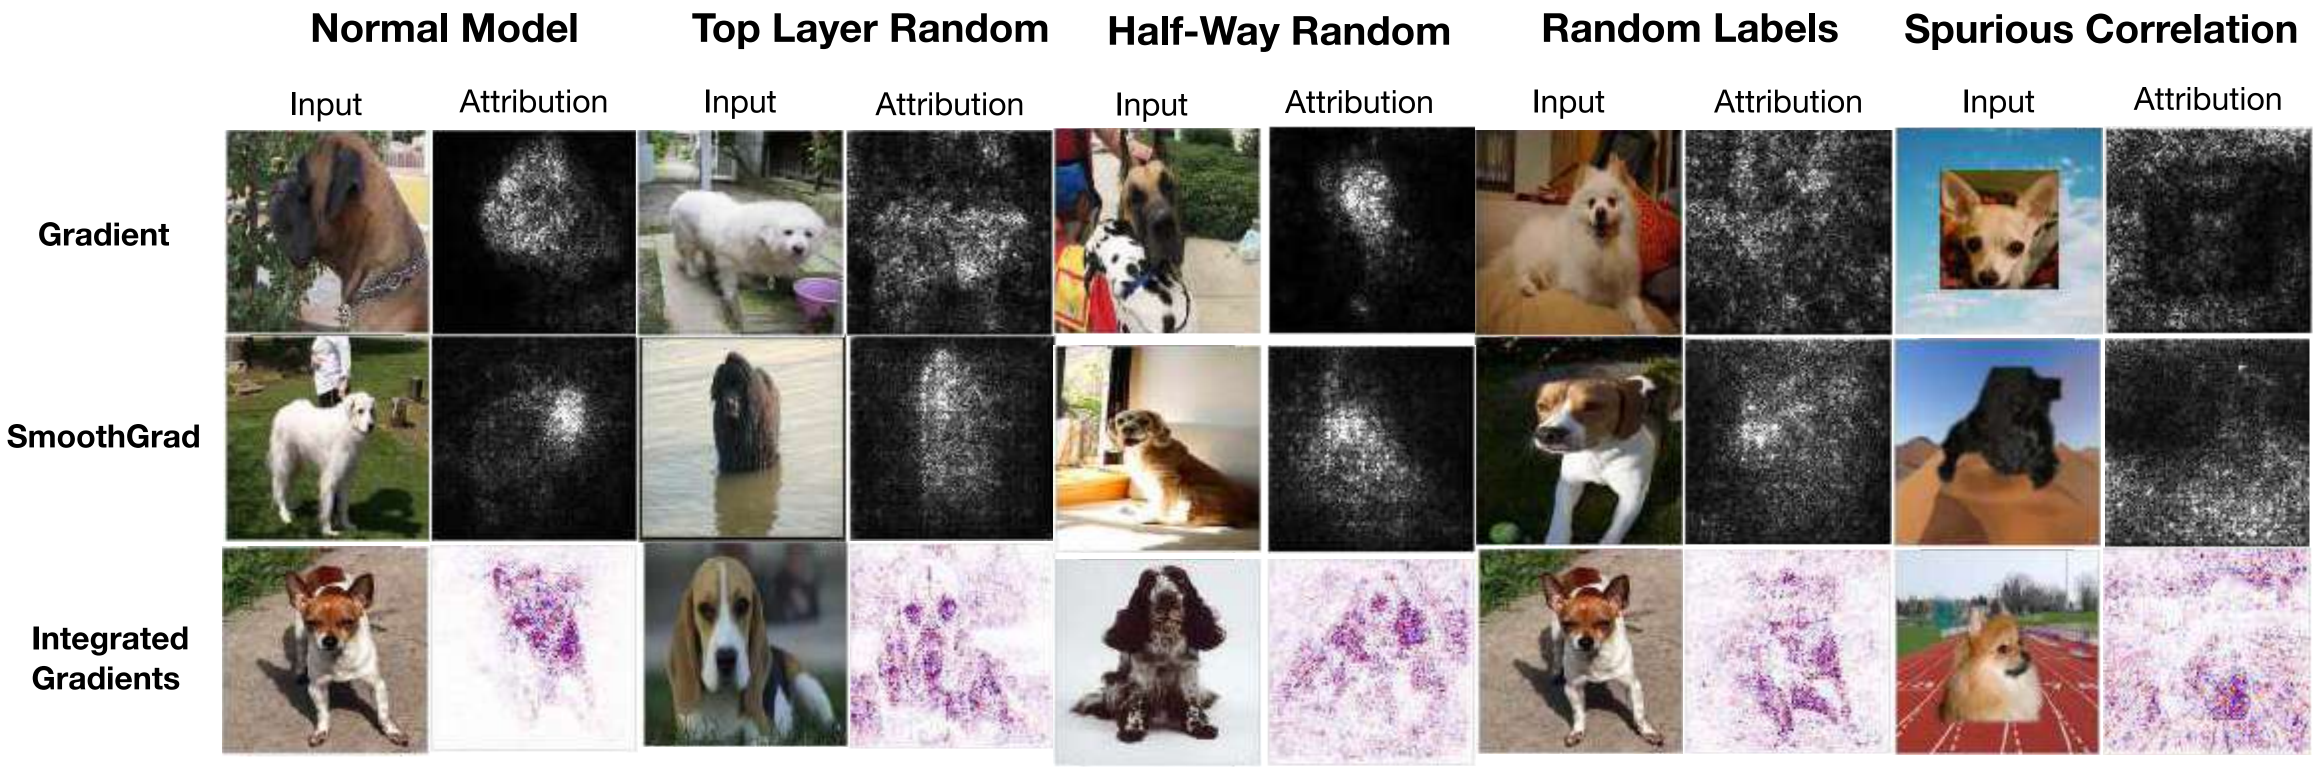
Normal Model
Top Layer Random
Half-Way Random
Random Labels
Spurious Correlation
Input
Attribution
Input
Attribution
Input
Attribution
Input
Attribution
Input
Attribution
Gradient
SmoothGrad
Integrated Gradients

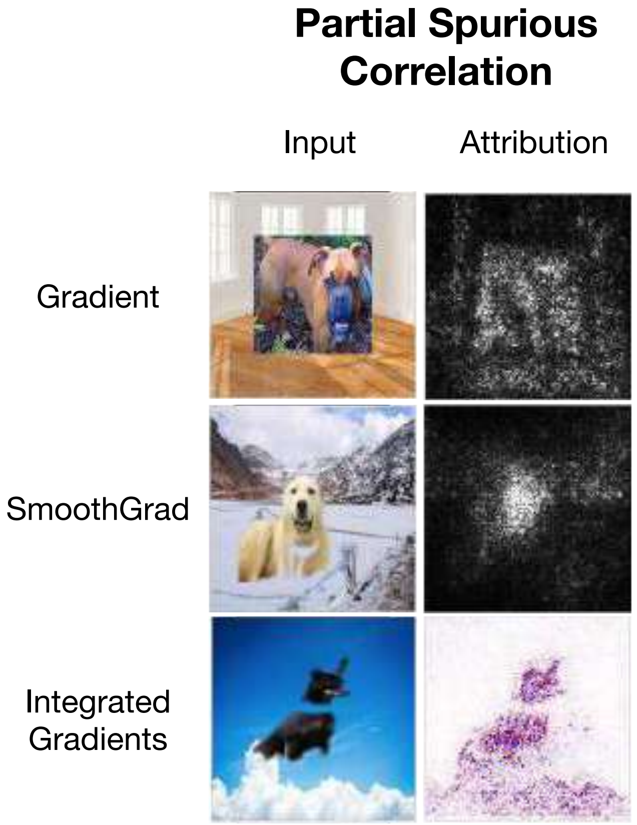
Partial Spurious Correlation
Input
Attribution
Gradient
SmoothGrad
Integrated Gradients

## Out of Distribution

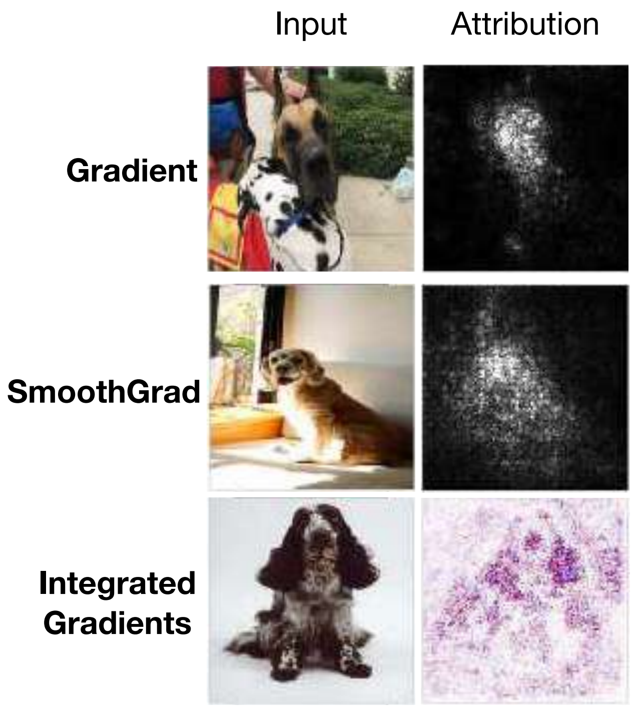

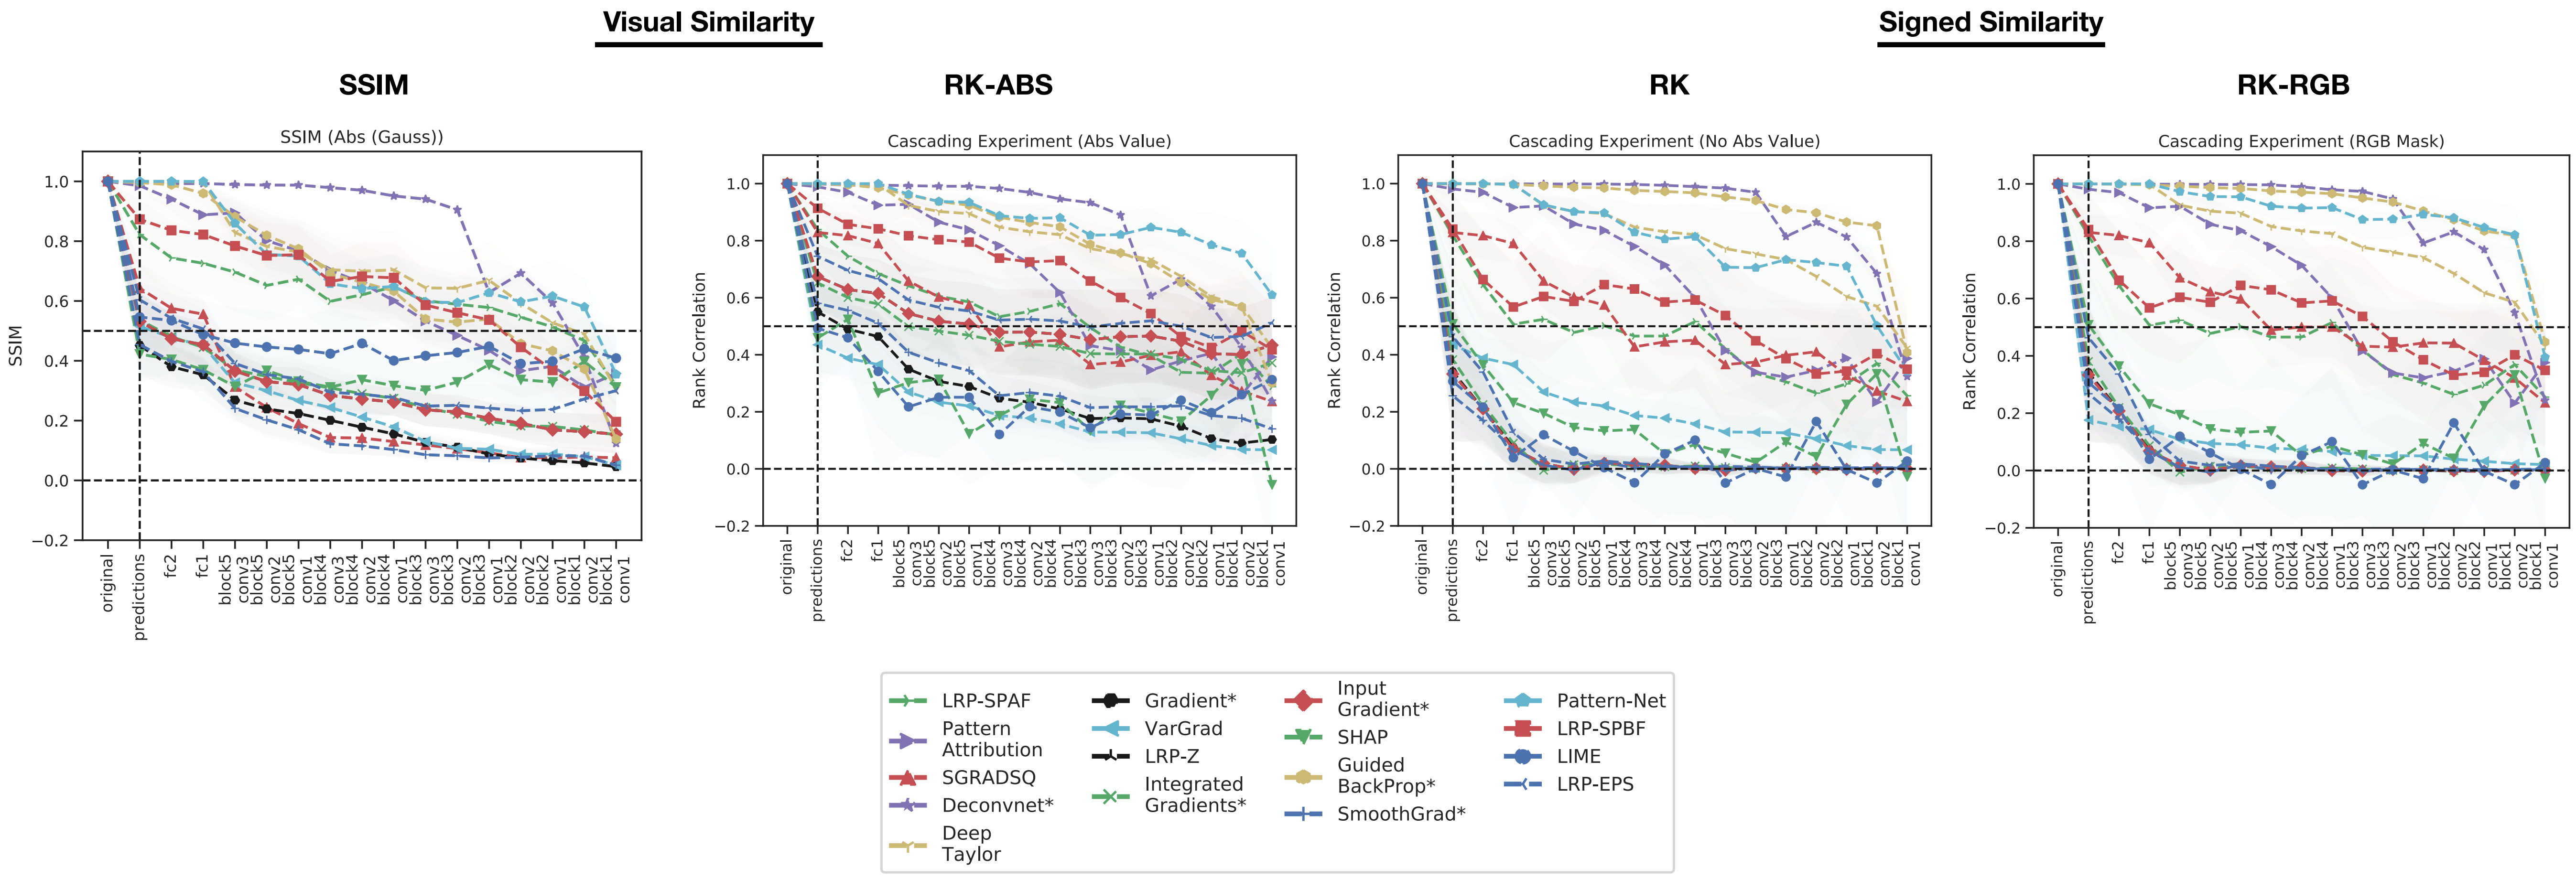
Visual Similarity
Signed Similarity
SSIM
RK-ABS
RK
RK-RGB
SSIM (Abs (Gauss))
Cascading Experiment (Abs Value)
Cascading Experiment (No Abs Value)
Cascading Experiment (RGB Mask)
SSIM
Rank Correlation
original
predictions
fc2
fc1
block5 conv3
block5 conv2
block5 conv1
block4 conv3
block4 conv2
block4 conv1
block3 conv3
block3 conv2
block3 conv1
block2 conv2
block2 conv1
block1 conv2
block1 conv1
LRP-SPAF
Pattern Attribution
SGRADSQ
Deconvnet*
Deep Taylor
Gradient*
VarGrad
LRP-Z
Integrated Gradients*
Input Gradient*
SHAP
Guided BackProp*
SmoothGrad*
Pattern-Net
LRP-SPBF
LIME
LRP-EPS

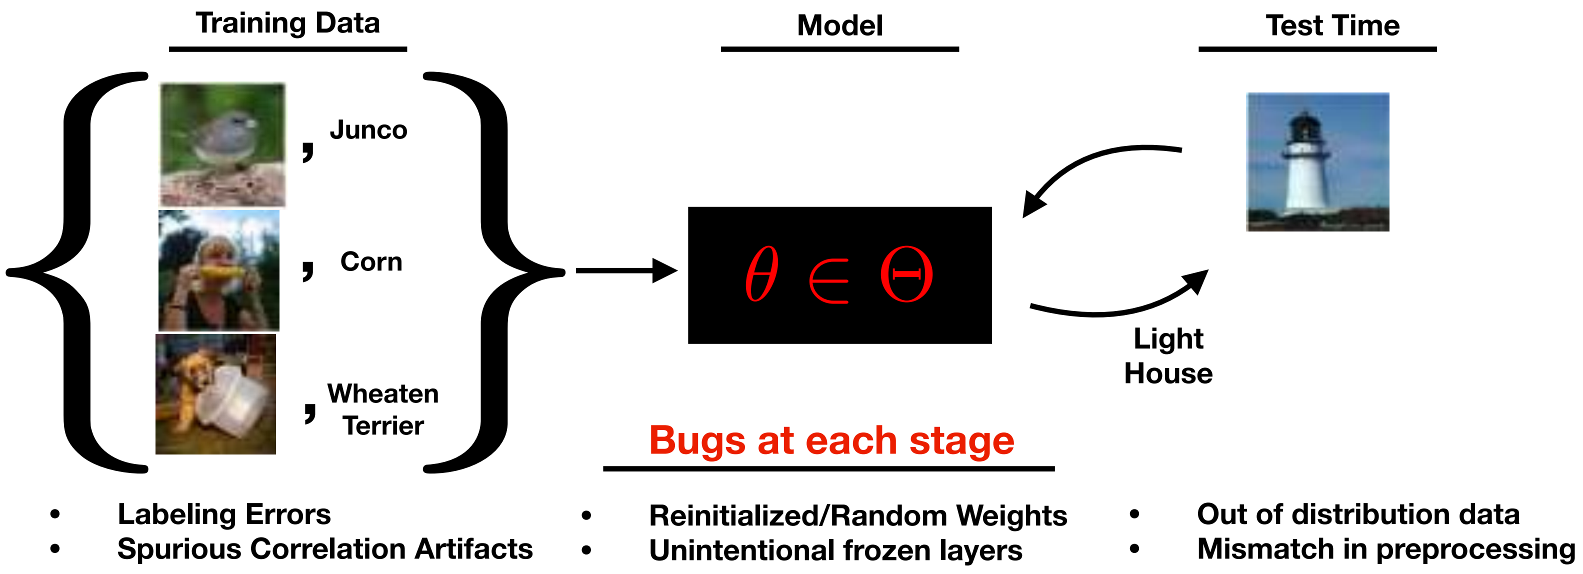
Training Data
Model
Test Time
Junco
Corn
Wheaten Terrier
$\theta \in \Theta$
Light House
Bugs at each stage
Labeling Errors
Spurious Correlation Artifacts
Reinitialized/Random Weights
Unintentional frozen layers
Out of distribution data
Mismatch in preprocessing

# Interpretability for Deep CNNs

Input

Machine Learning Model

Output Prediction

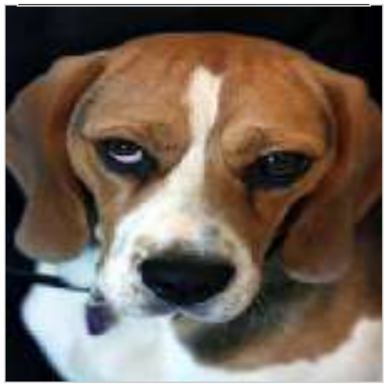

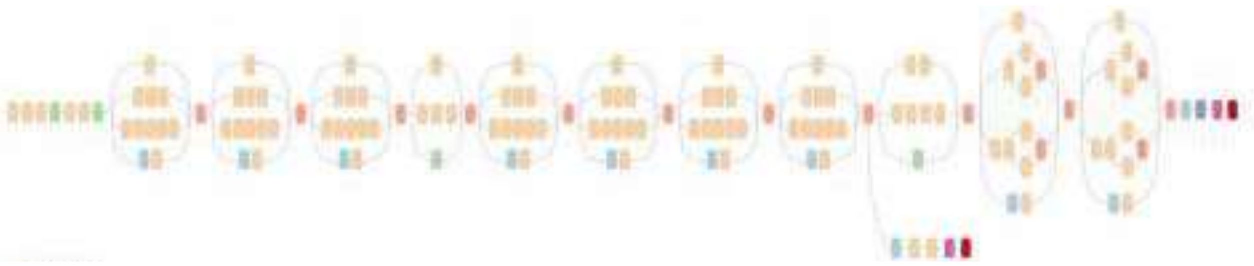

Beagle

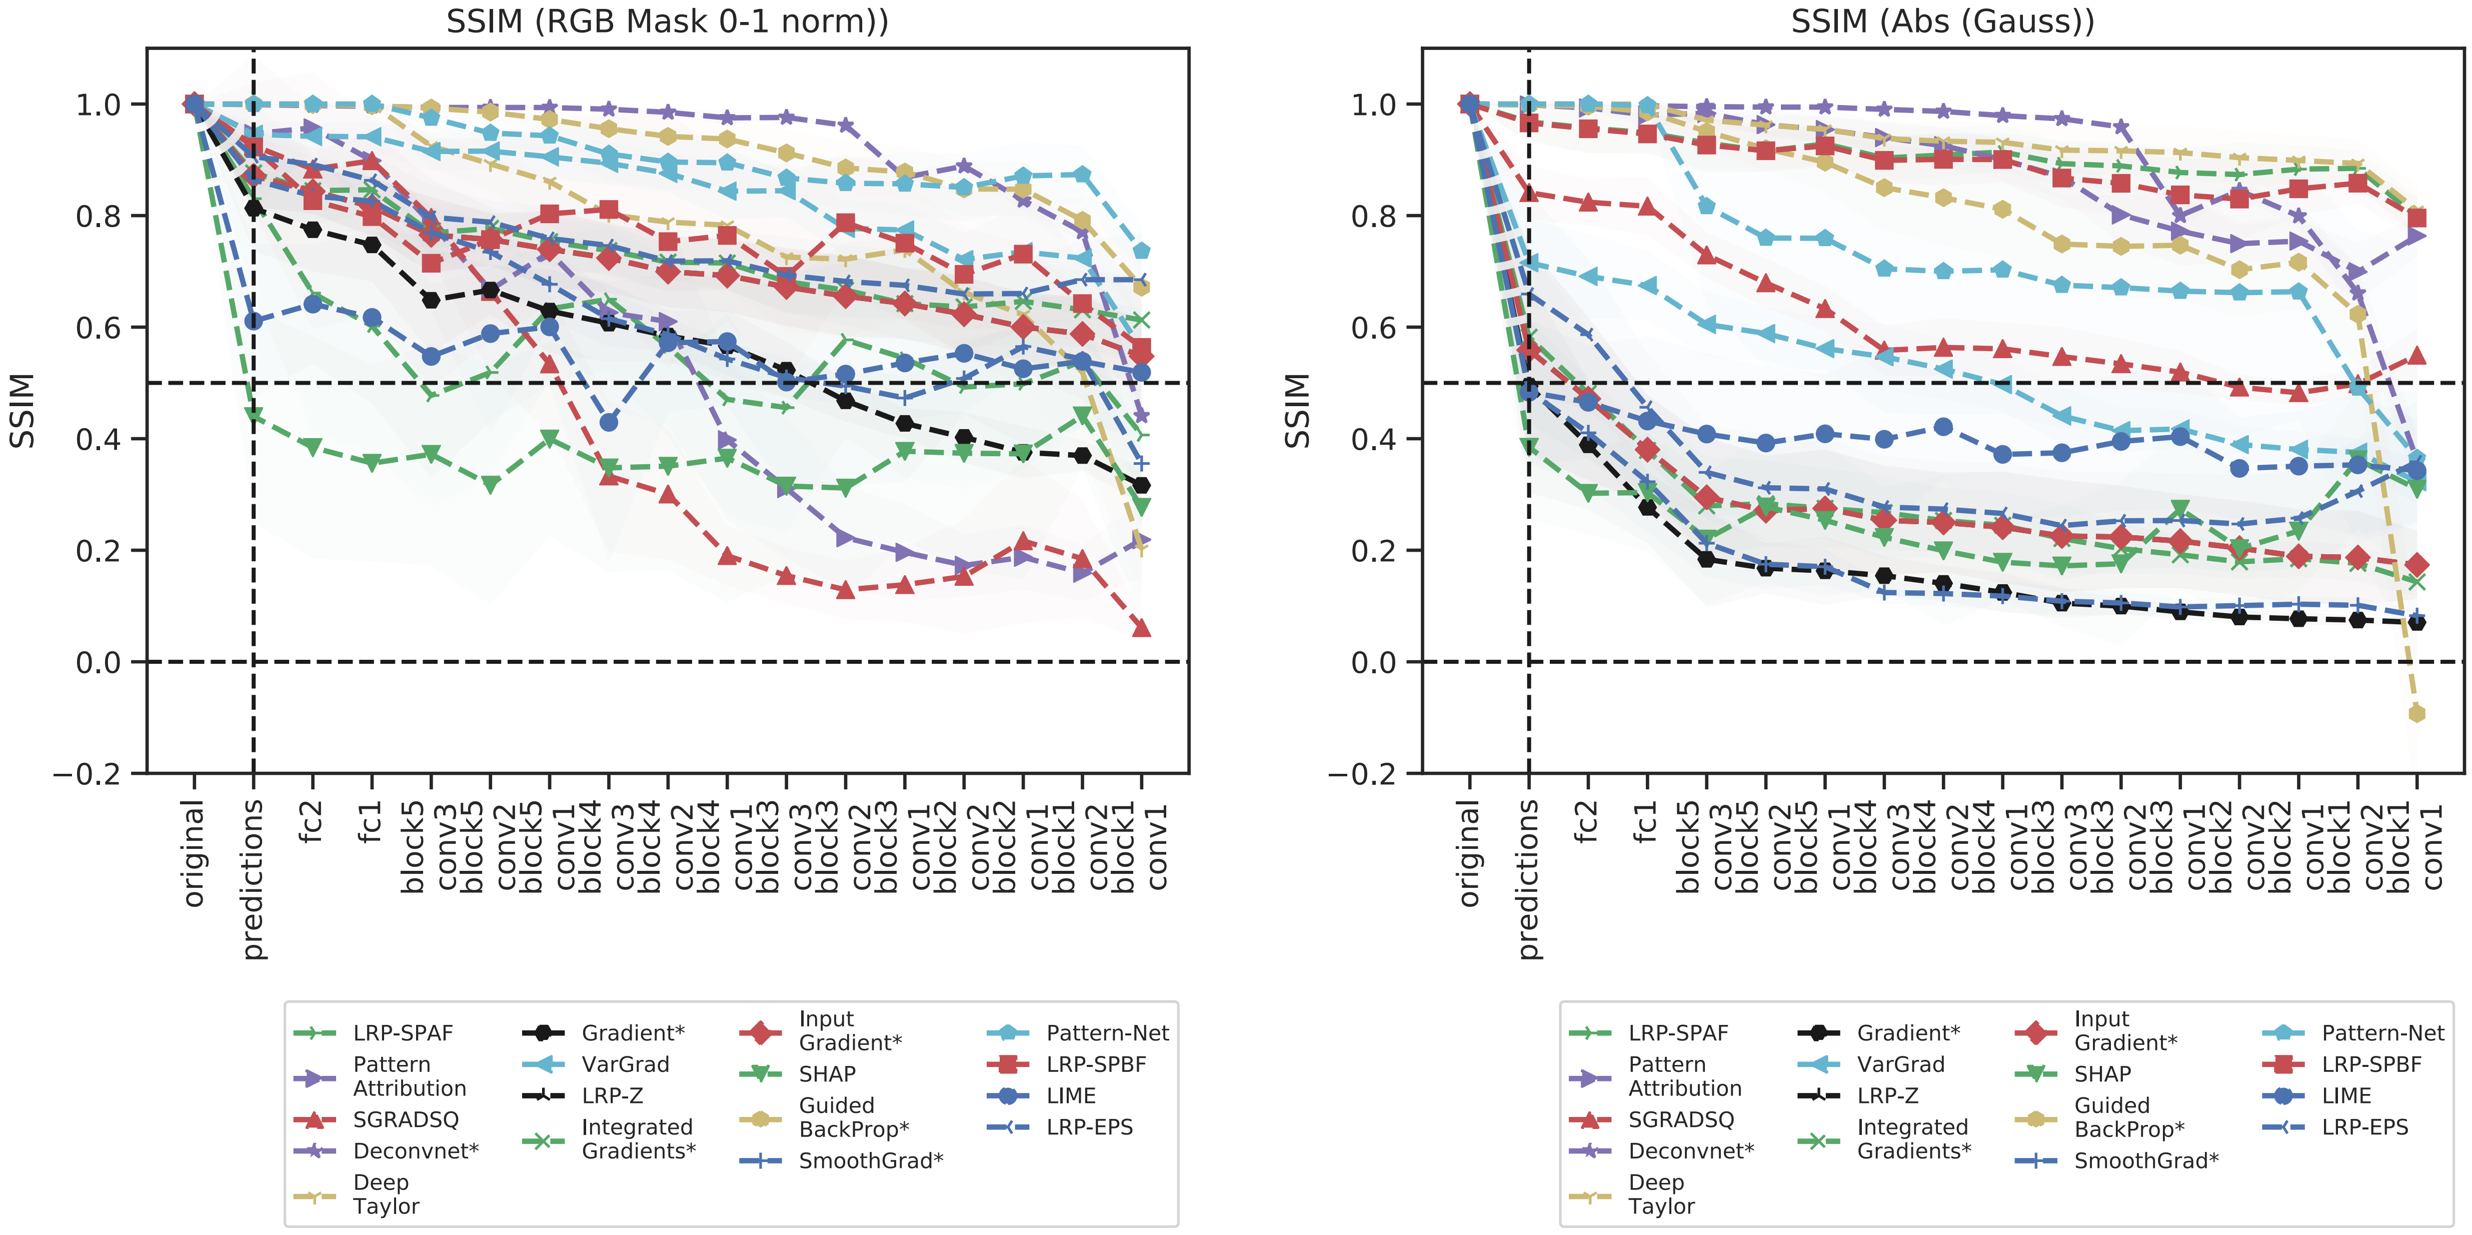

SSIM (RGB Mask 0-1 norm))
SSIM (Abs (Gauss))
SSIM
1.0
0.8
0.6
0.4
0.2
0.0
−0.2
original
predictions
fc2
fc1
block5 conv3
block5 conv2
block5 conv1
block4 conv3
block4 conv2
block4 conv1
block3 conv3
block3 conv2
block3 conv1
block2 conv2
block2 conv1
block1 conv2
block1 conv1
LRP-SPAF
Pattern Attribution
SGRADSQ
Deconvnet*
Deep Taylor
Gradient*
VarGrad
LRP-Z
Integrated Gradients*
Input Gradient*
SHAP
Guided BackProp*
SmoothGrad*
Pattern-Net
LRP-SPBF
LIME
LRP-EPS

This is the question you will answer throughout this task.

**Using the output and explanation of the dog classification model below, do you think this specific model is ready to be sold to customers?**

This is the prediction of the ML on the image.

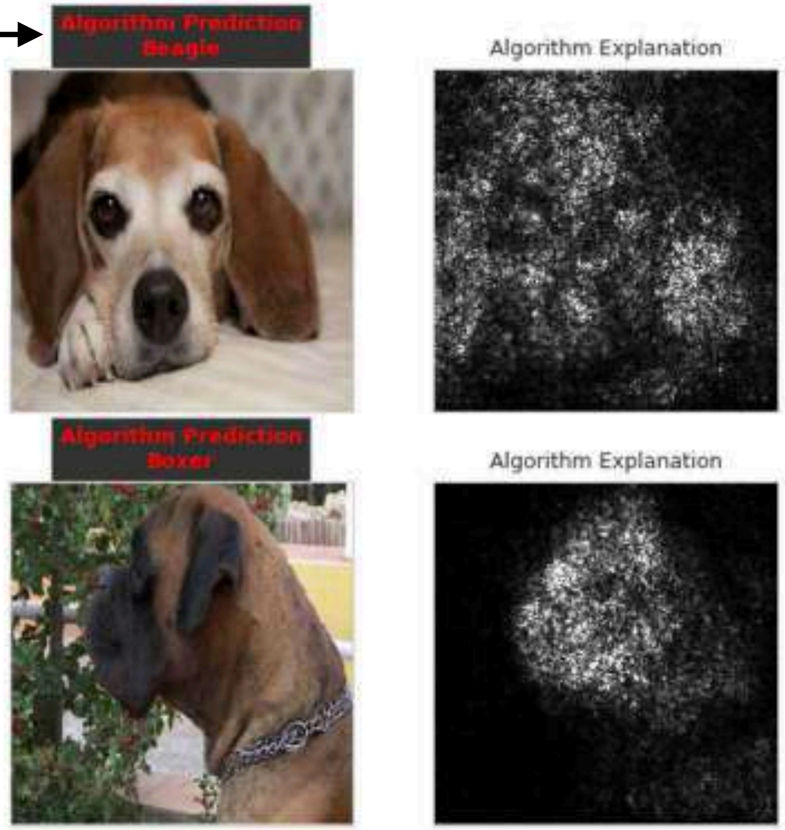


This kind of explanation is called a heat map. It shows the parts of the image that the ML relied on to make the prediction.

Pick out of these choices.

| DEFINITELY NOT | PROBABLY NOT | UNSURE/MAYBE | PROBABLY | DEFINITELY |
|---|---|---|---|---|
| ○ | ○ | ○ | ○ | ○ |

Say why you made the choice above.

What were your motivation for your response above?

- ○ On some or all of the images, the dog breed was wrong.
- ○ The dog breeds were correct.
- ○ The explanation did not highlight the part of the image that I expected it to focus on.
- ○ Other, please specify

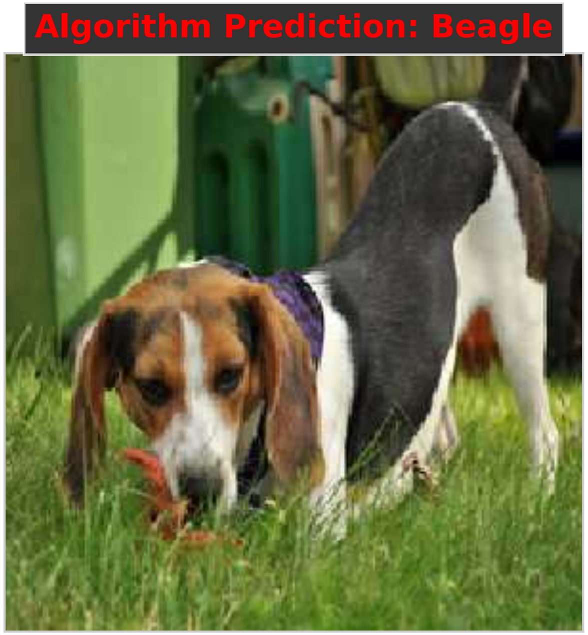


Algorithm Explanation

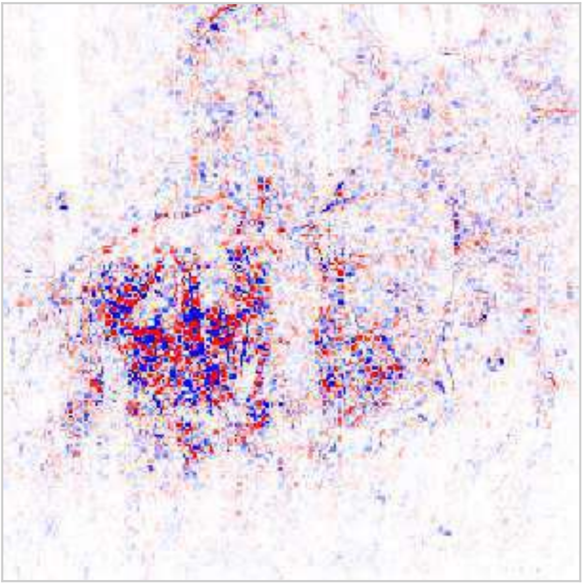

For the Blue/Red images, the red dots are positive evidence, and the blue dots are negative evidence.

In this example, the red dots are evidence for why this image is a Beagle. The blue dots are evidence for a breed other than Beagle.

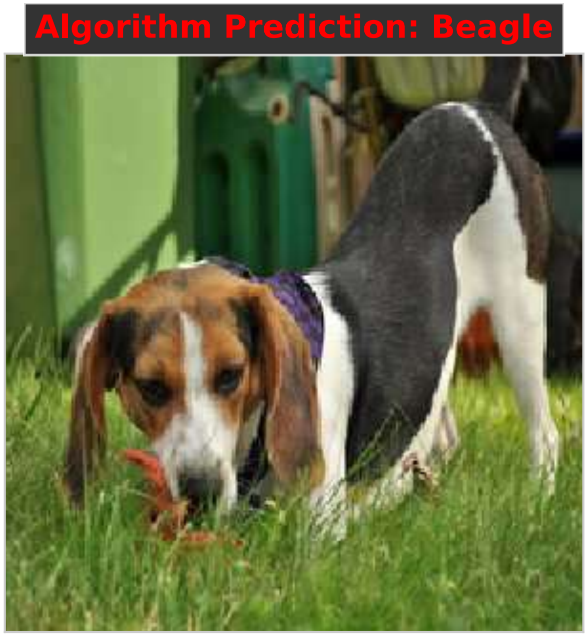


Algorithm Explanation

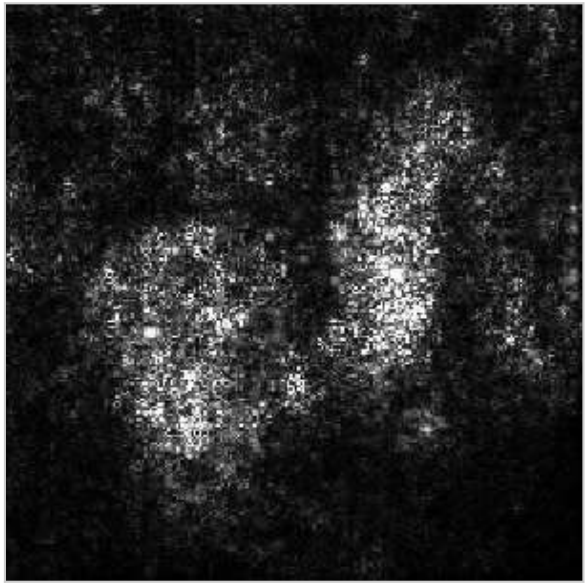

The white portions are important parts that the ML relied on.

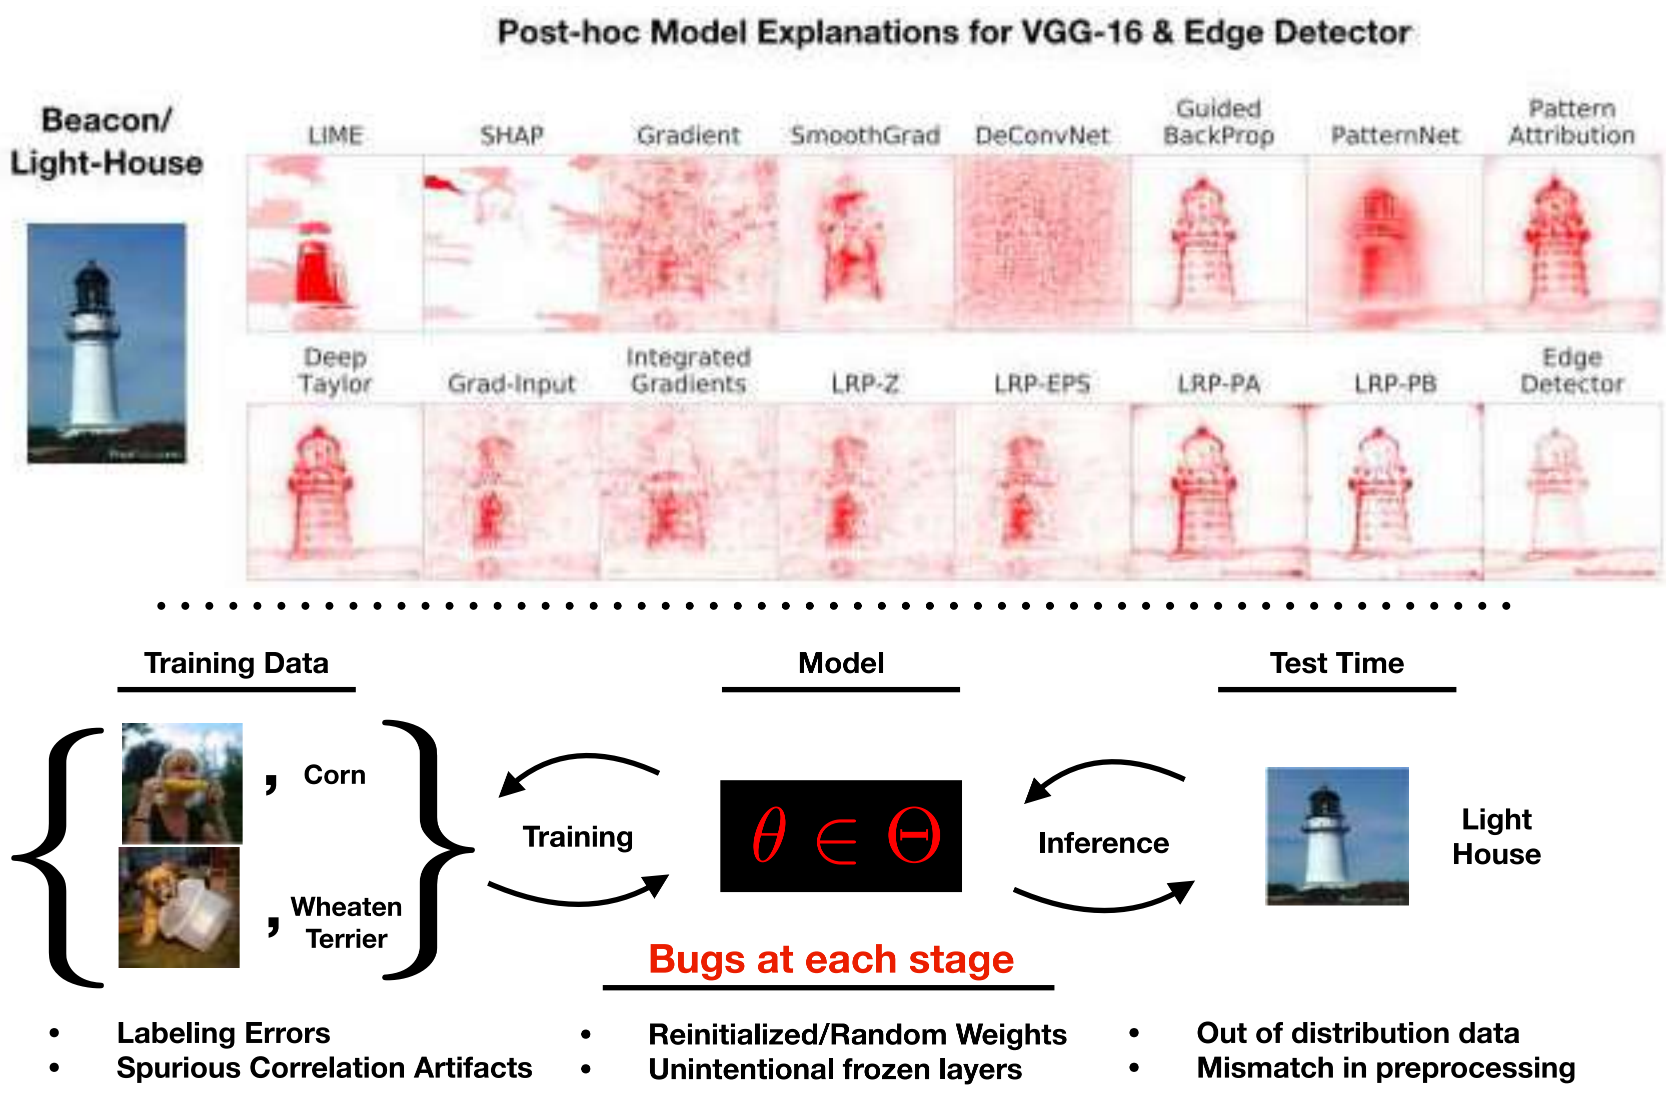
Post-hoc Model Explanations for VGG-16 & Edge Detector
Beacon/ Light-House
LIME
SHAP
Gradient
SmoothGrad
DeConvNet
Guided BackProp
PatternNet
Pattern Attribution
Deep Taylor
Grad-Input
Integrated Gradients
LRP-Z
LRP-EPS
LRP-PA
LRP-PB
Edge Detector
Training Data
Model
Test Time
Corn
Wheaten Terrier
Training
$\theta \in \Theta$
Inference
Light House
Bugs at each stage
• Labeling Errors
• Spurious Correlation Artifacts
• Reinitialized/Random Weights
• Unintentional frozen layers
• Out of distribution data
• Mismatch in preprocessing

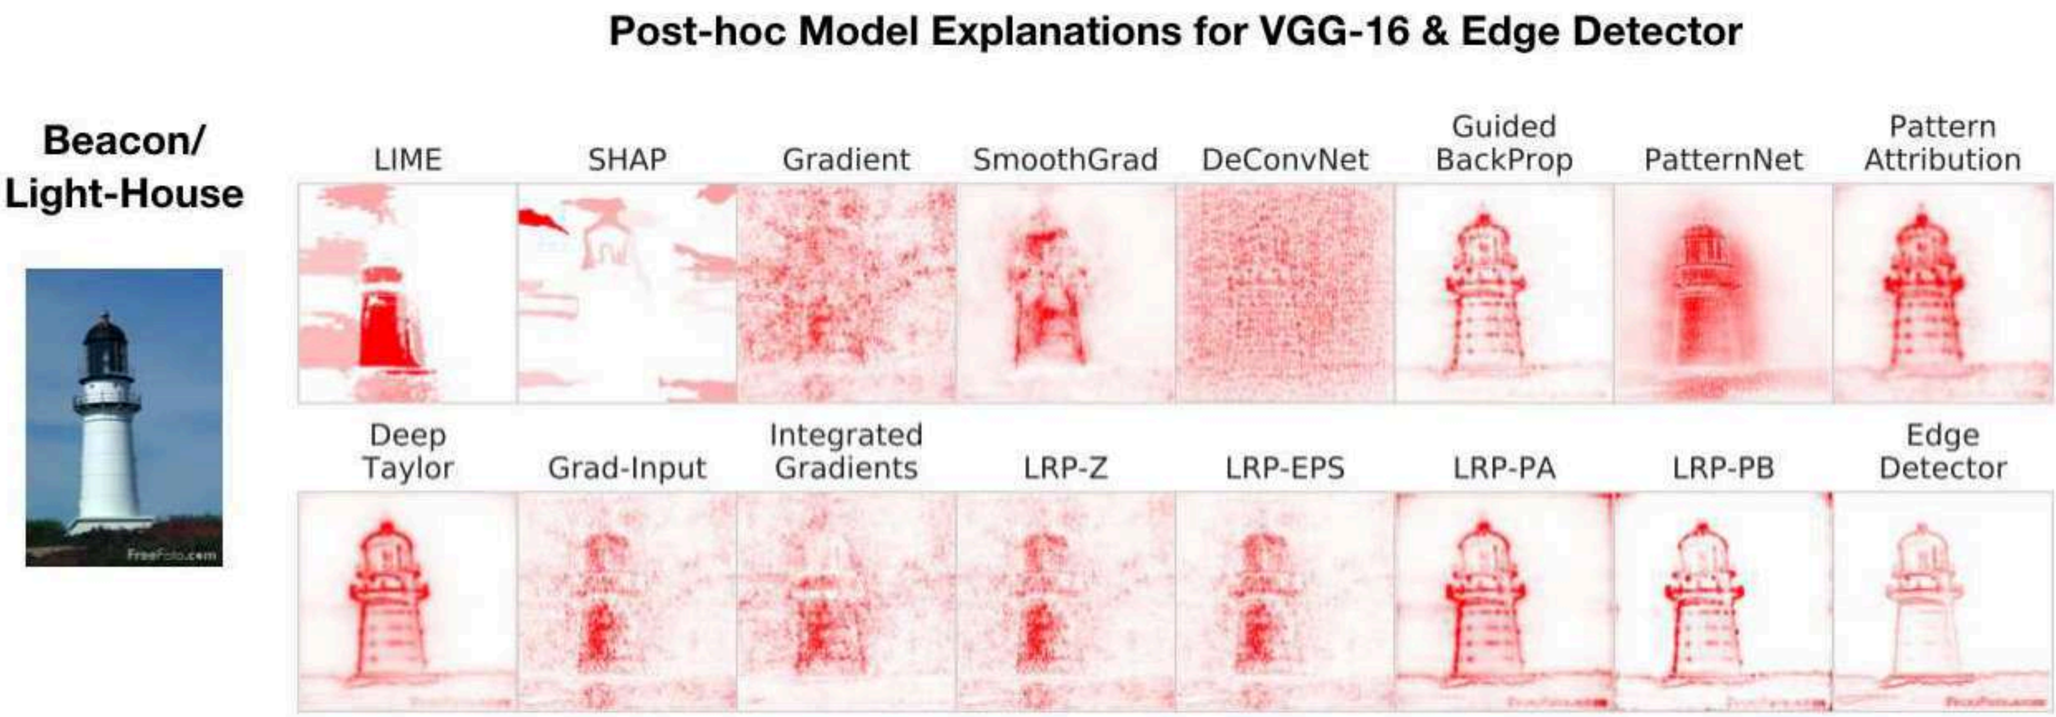
Post-hoc Model Explanations for VGG-16 & Edge Detector
Beacon/
Light-House
LIME
SHAP
Gradient
SmoothGrad
DeConvNet
Guided BackProp
PatternNet
Pattern Attribution
Deep Taylor
Grad-Input
Integrated Gradients
LRP-Z
LRP-EPS
LRP-PA
LRP-PB
Edge Detector

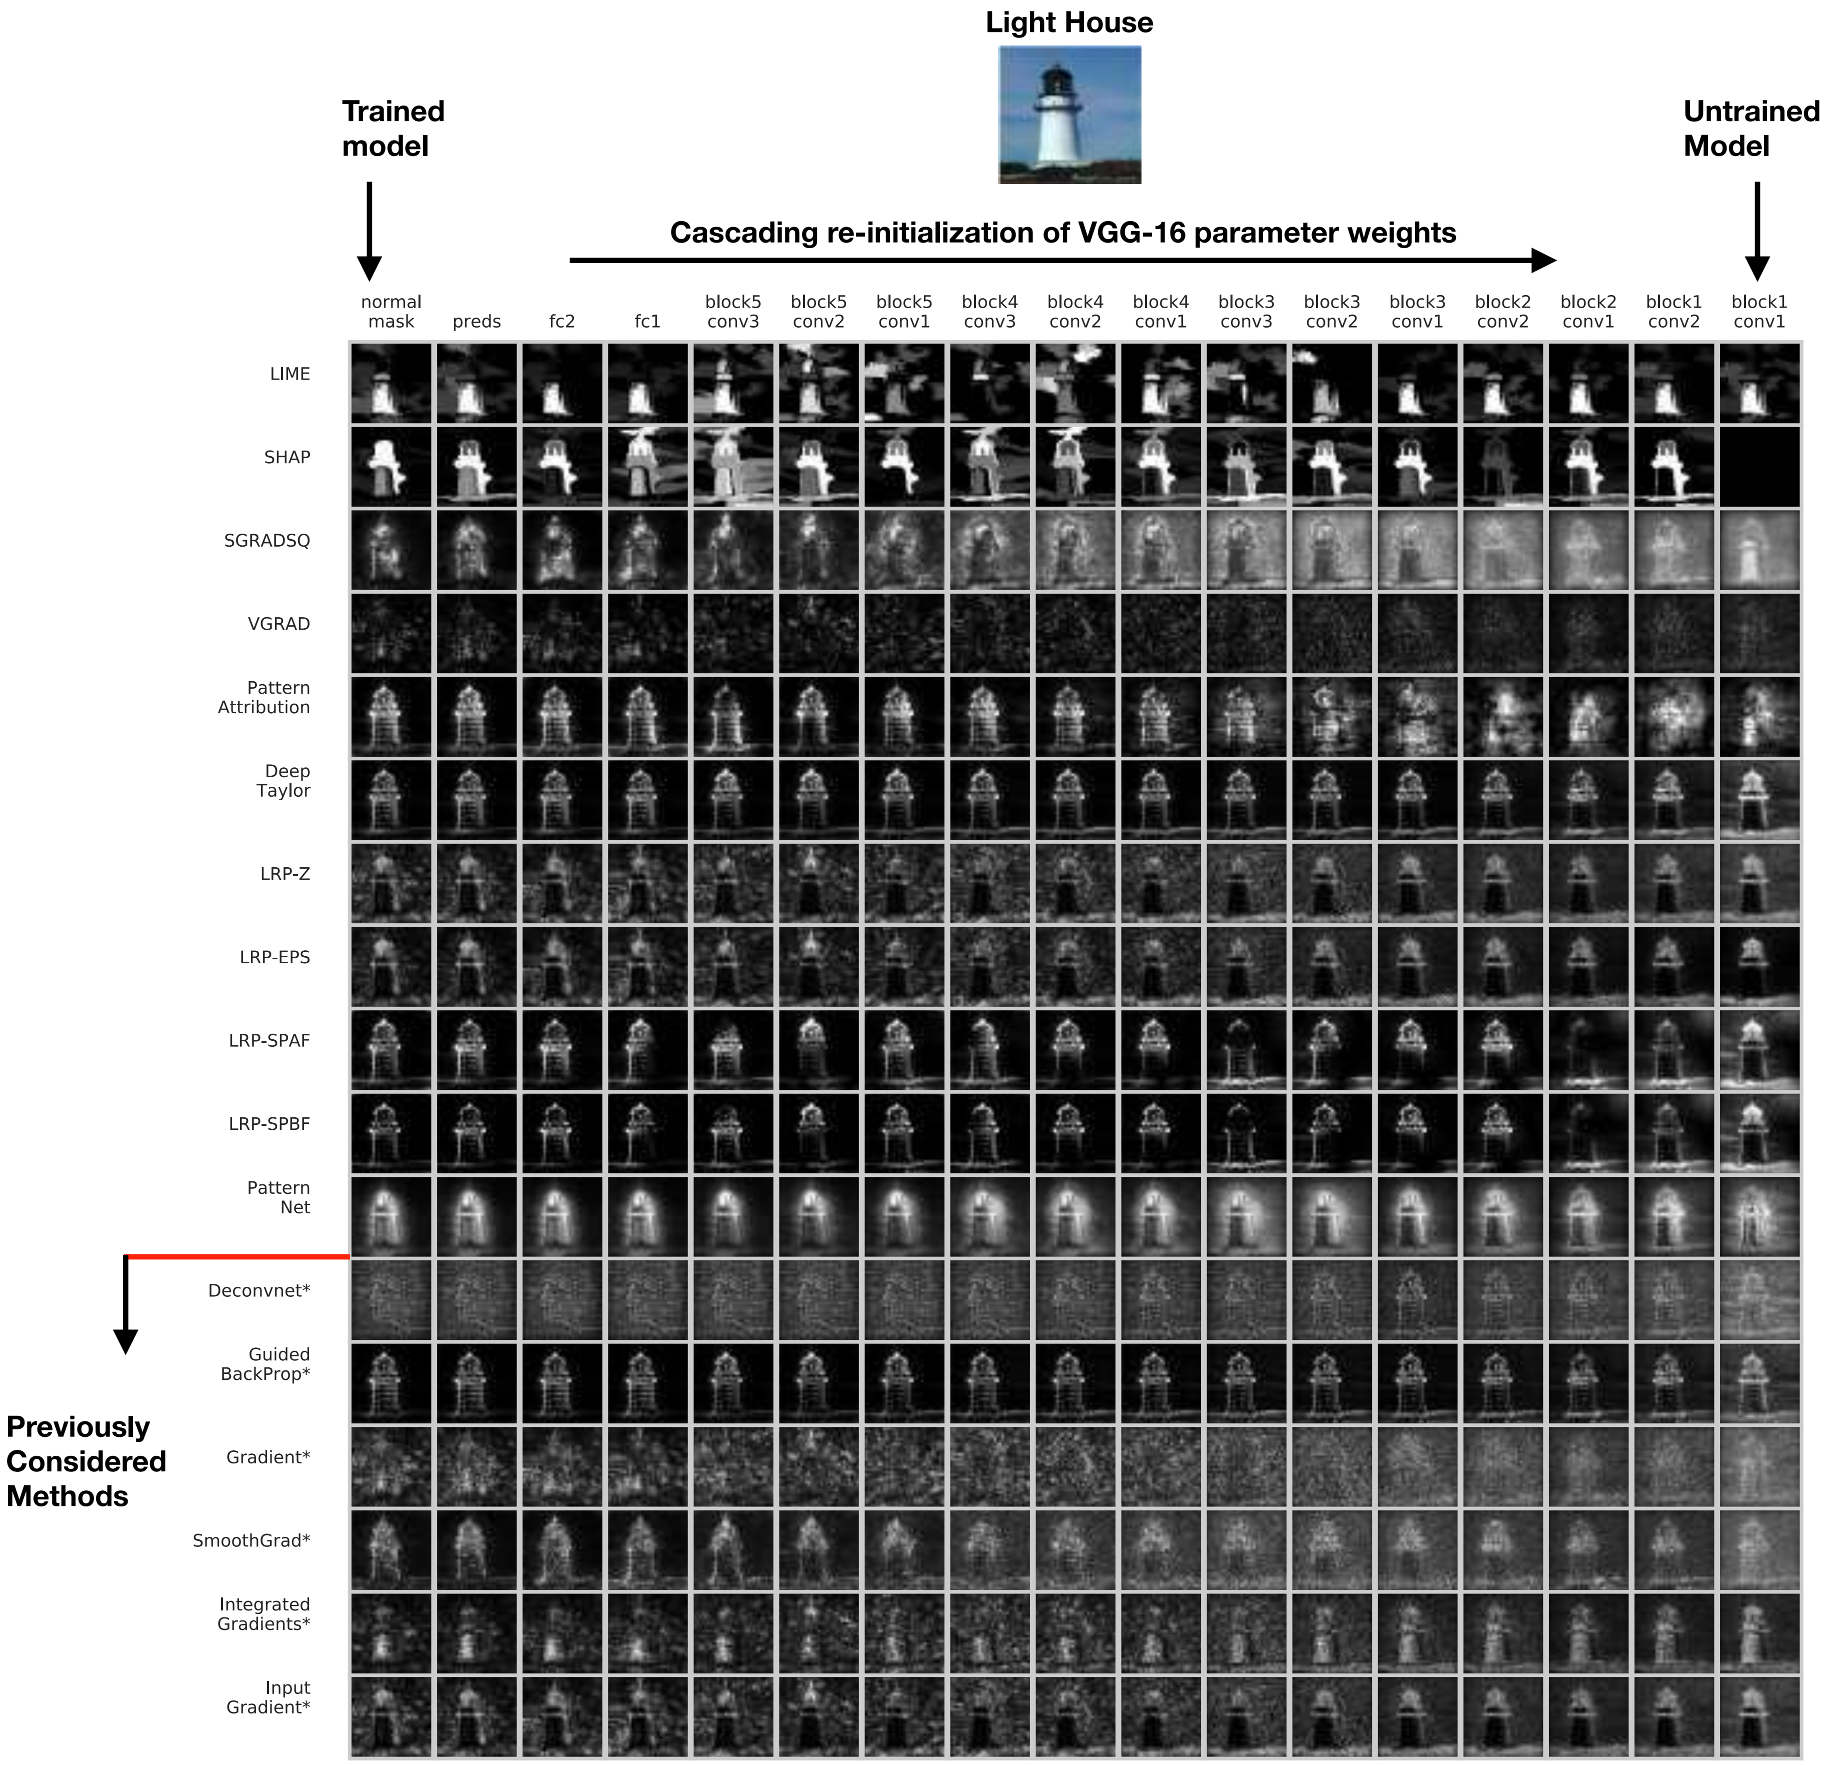
Light House
Trained model
Untrained Model
Cascading re-initialization of VGG-16 parameter weights
normal mask
preds
fc2
fc1
block5 conv3
block5 conv2
block5 conv1
block4 conv3
block4 conv2
block4 conv1
block3 conv3
block3 conv2
block3 conv1
block2 conv2
block2 conv1
block1 conv2
block1 conv1
LIME
SHAP
SGRADSQ
VGRAD
Pattern Attribution
Deep Taylor
LRP-Z
LRP-EPS
LRP-SPAF
LRP-SPBF
Pattern Net
Deconvnet*
Guided BackProp*
Gradient*
SmoothGrad*
Integrated Gradients*
Input Gradient*
Previously Considered Methods

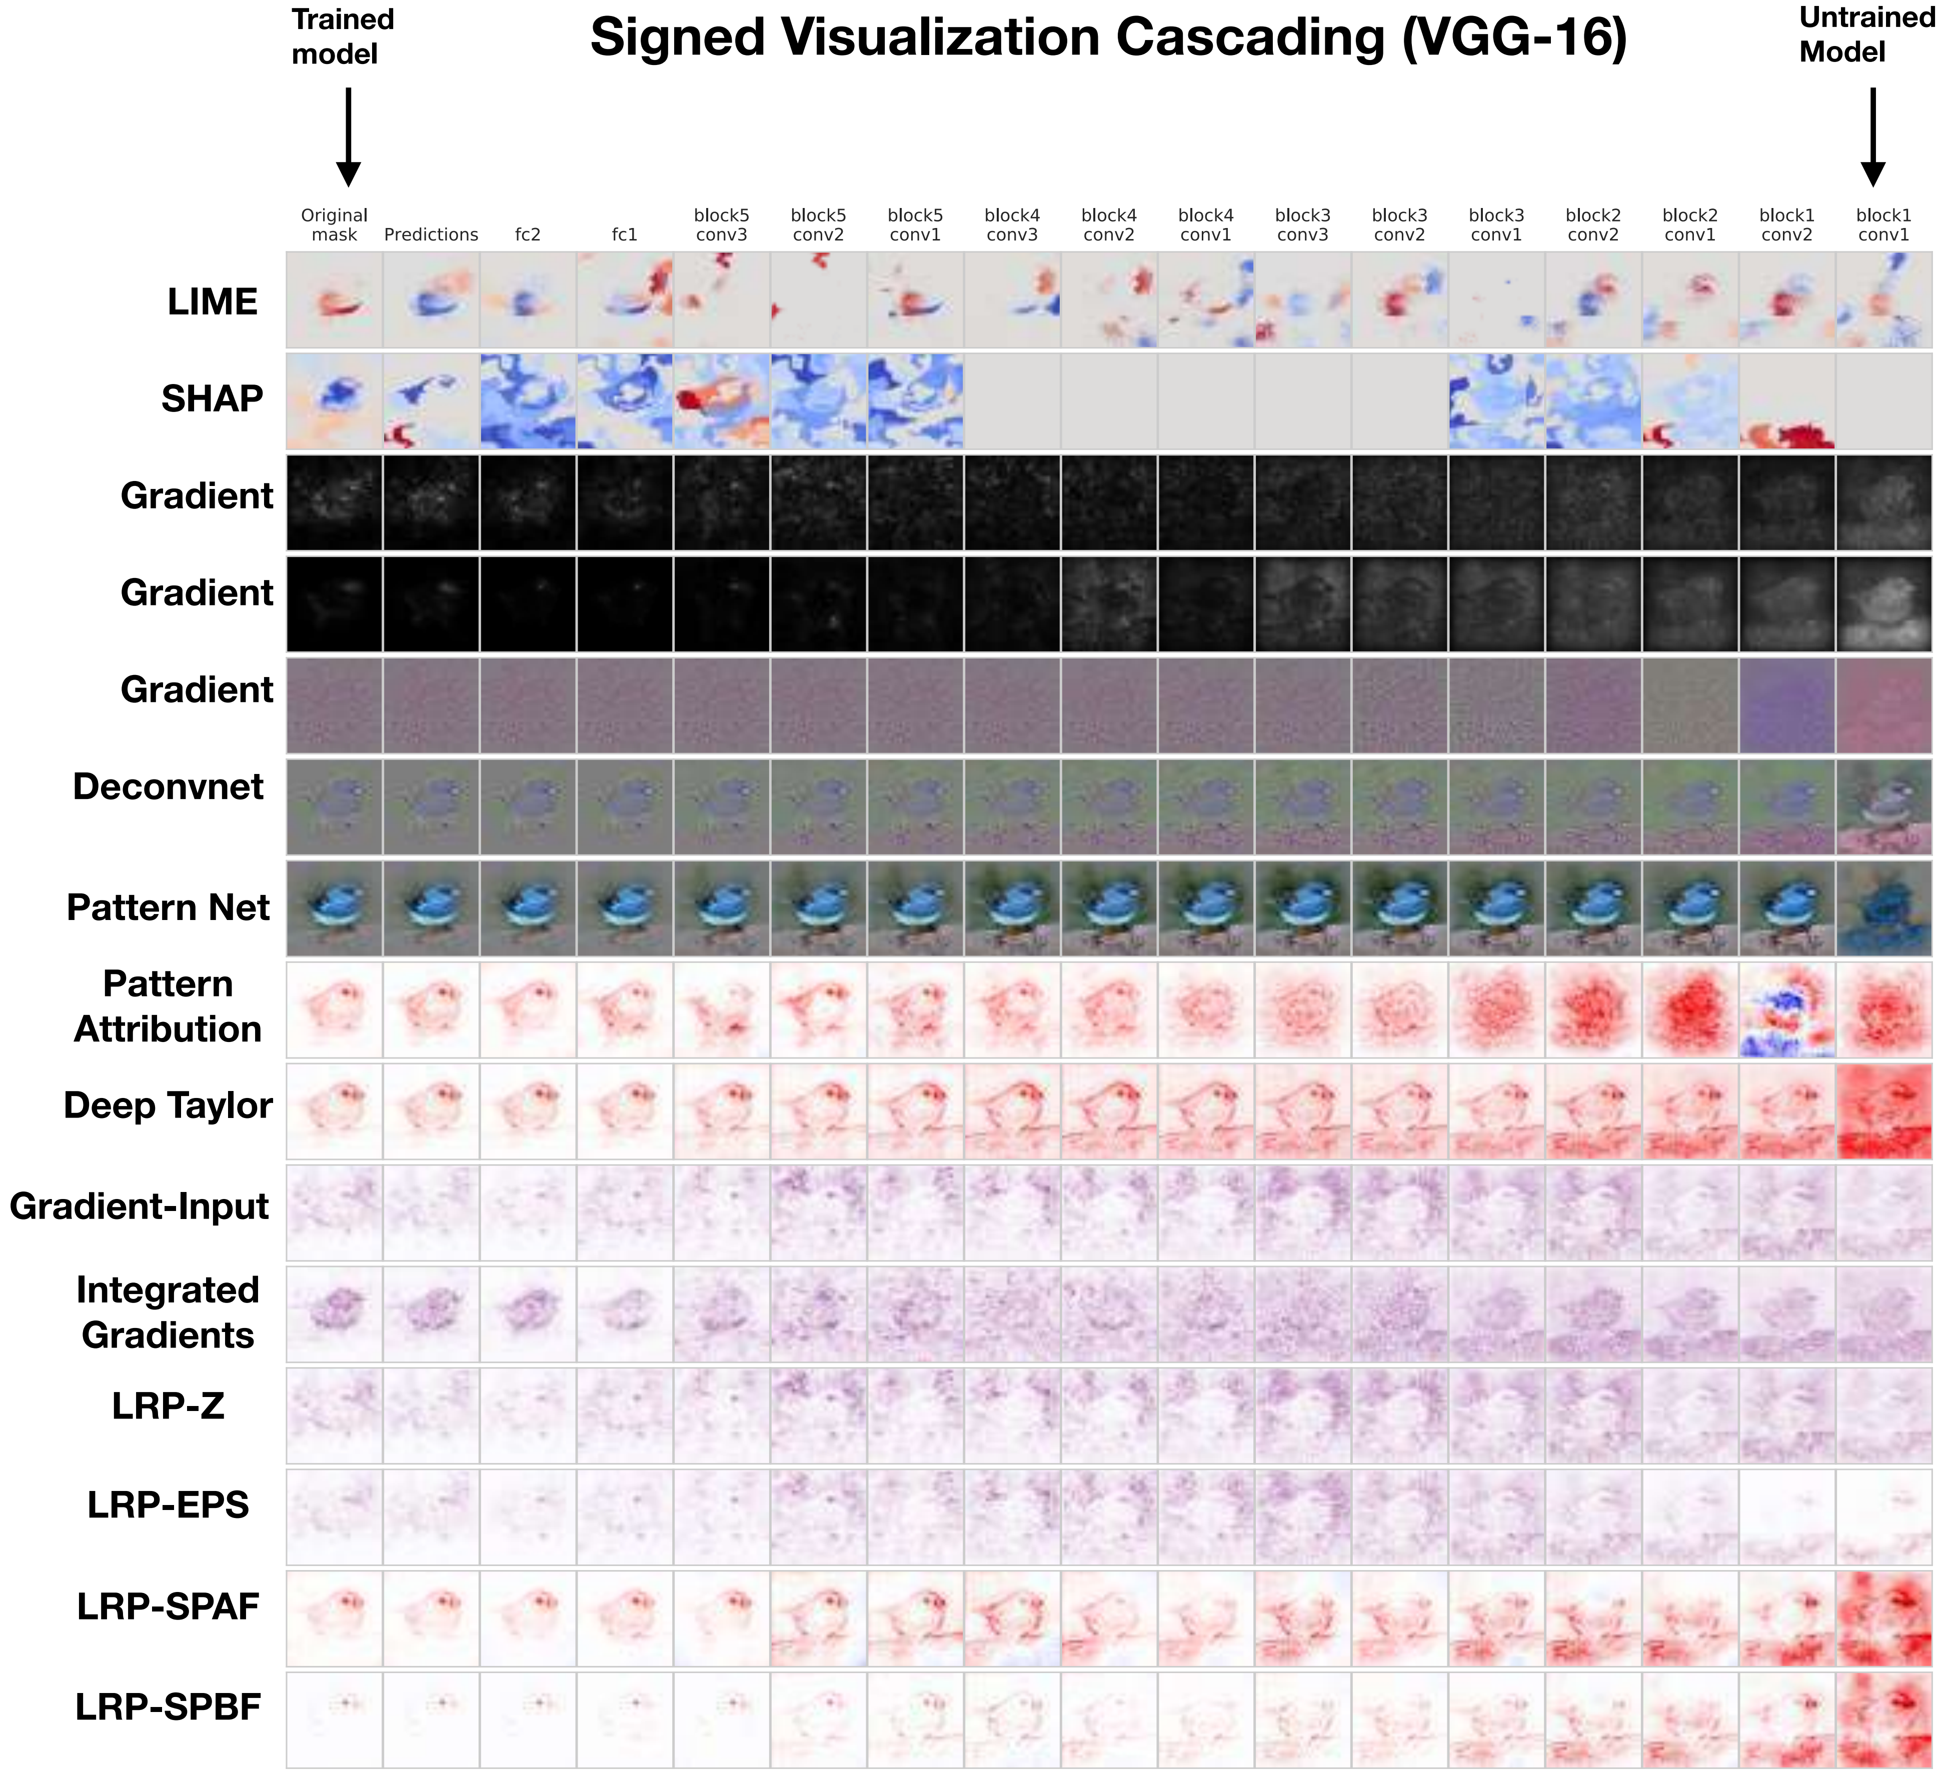
Signed Visualization Cascading (VGG-16)
Trained model
Untrained Model
Original mask
Predictions
fc2
fc1
block5 conv3
block5 conv2
block5 conv1
block4 conv3
block4 conv2
block4 conv1
block3 conv3
block3 conv2
block3 conv1
block2 conv2
block2 conv1
block1 conv2
block1 conv1
LIME
SHAP
Gradient
Gradient
Gradient
Deconvnet
Pattern Net
Pattern Attribution
Deep Taylor
Gradient-Input
Integrated Gradients
LRP-Z
LRP-EPS
LRP-SPAF
LRP-SPBF

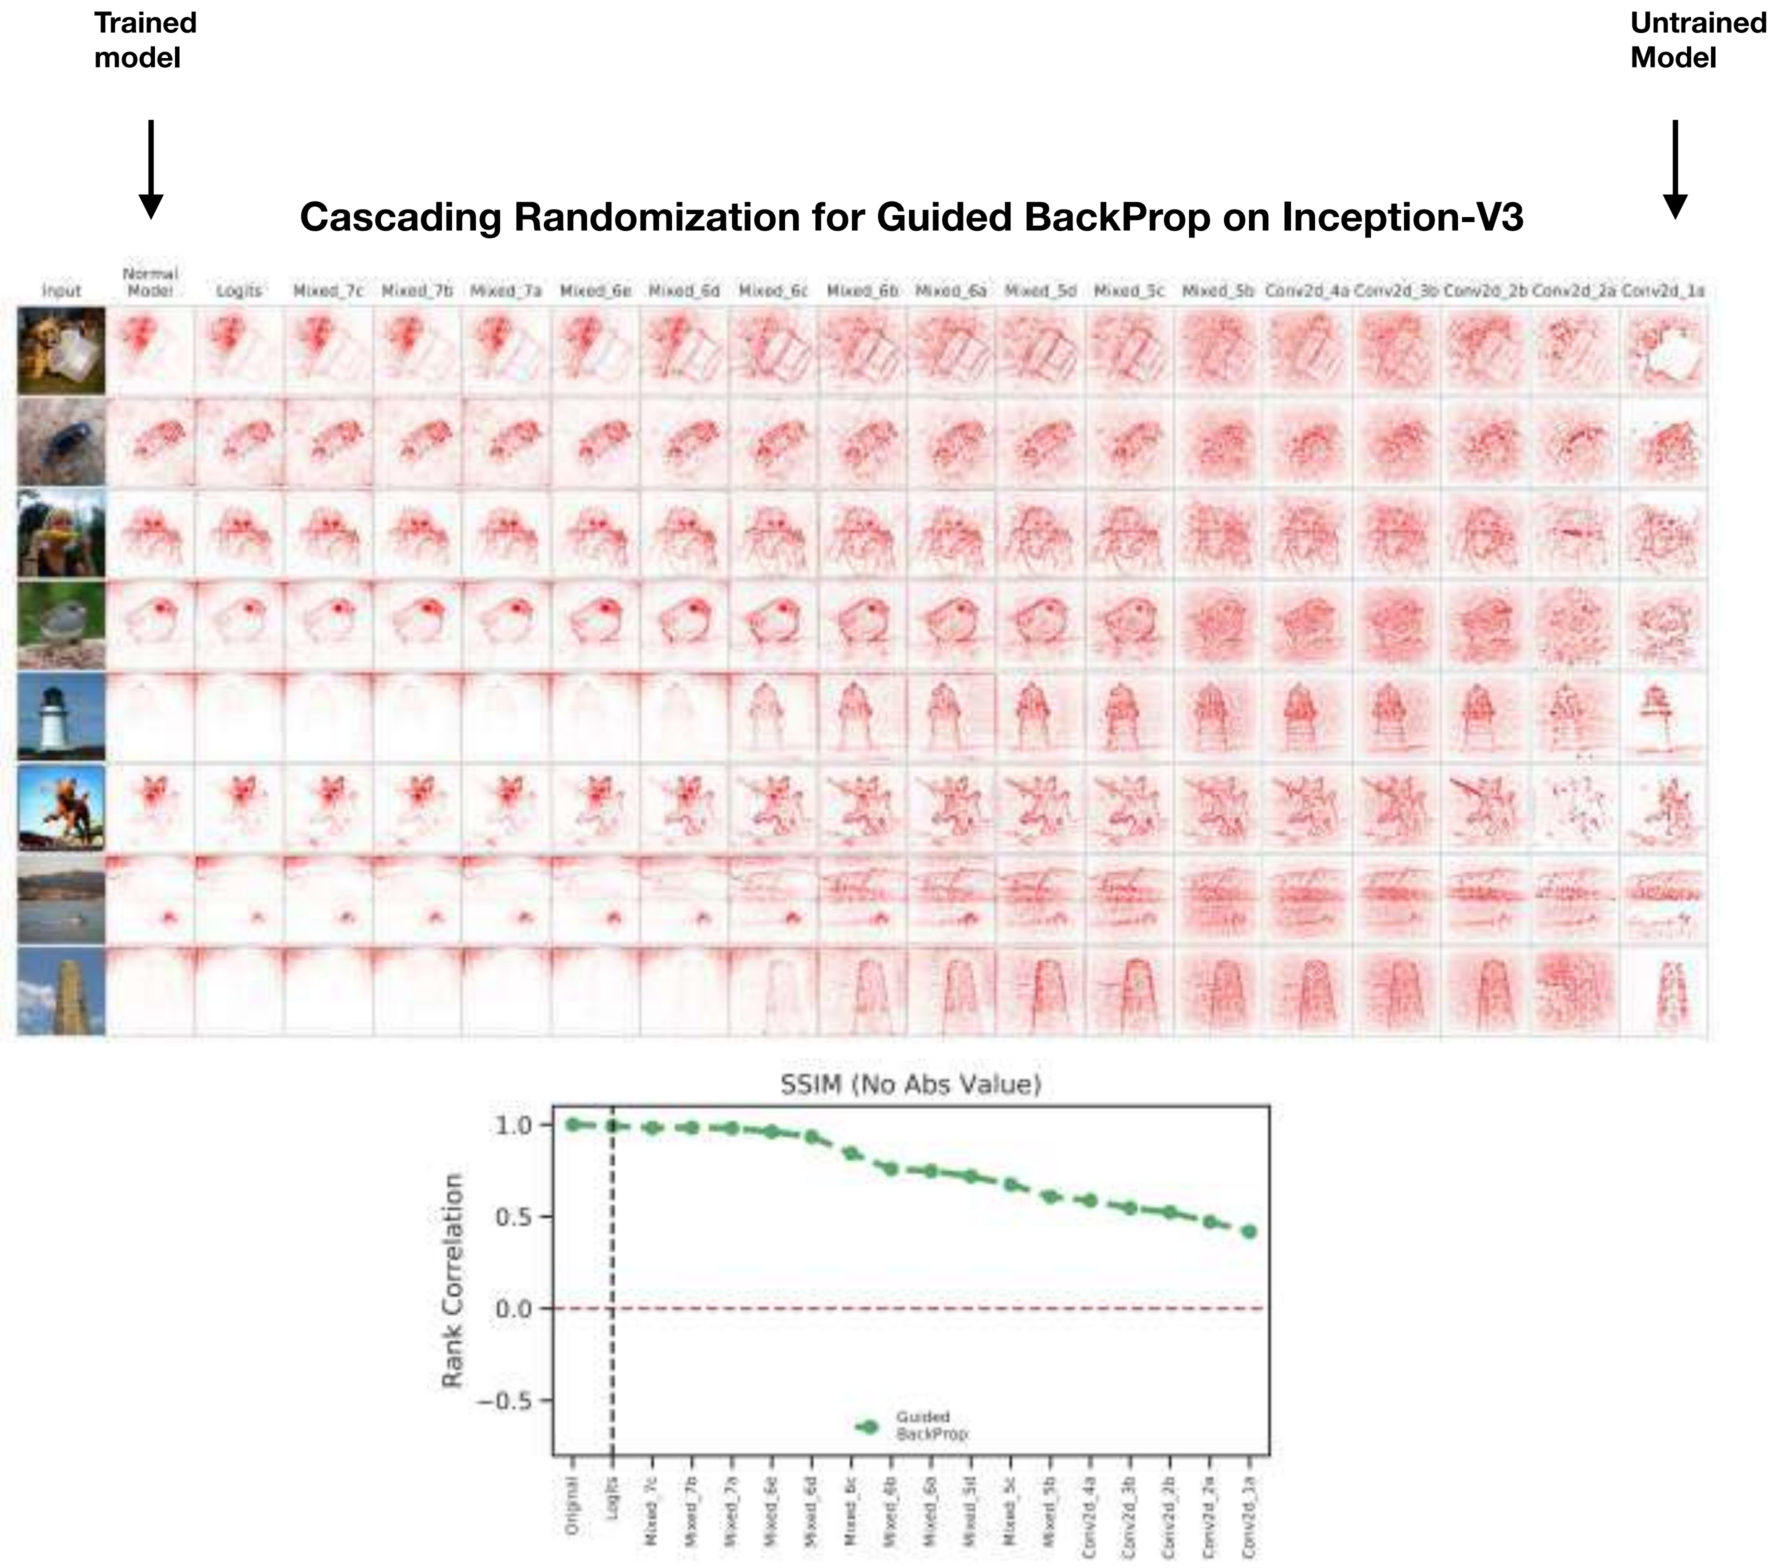

Trained model
Untrained Model
Cascading Randomization for Guided BackProp on Inception-V3
Input
Normal Model
Logits
Mixed_7c
Mixed_7b
Mixed_7a
Mixed_6e
Mixed_6d
Mixed_6c
Mixed_6b
Mixed_6a
Mixed_5d
Mixed_5c
Mixed_5b
Conv2d_4a
Conv2d_3b
Conv2d_2b
Conv2d_2a
Conv2d_1a
SSIM (No Abs Value)
Rank Correlation
1.0
0.5
0.0
−0.5
Guided BackProp
Original
Logits
Mixed_7c
Mixed_7b
Mixed_7a
Mixed_6e
Mixed_6d
Mixed_6c
Mixed_6b
Mixed_6a
Mixed_5d
Mixed_5c
Mixed_5b
Conv2d_4a
Conv2d_3b
Conv2d_2b
Conv2d_2a
Conv2d_1a

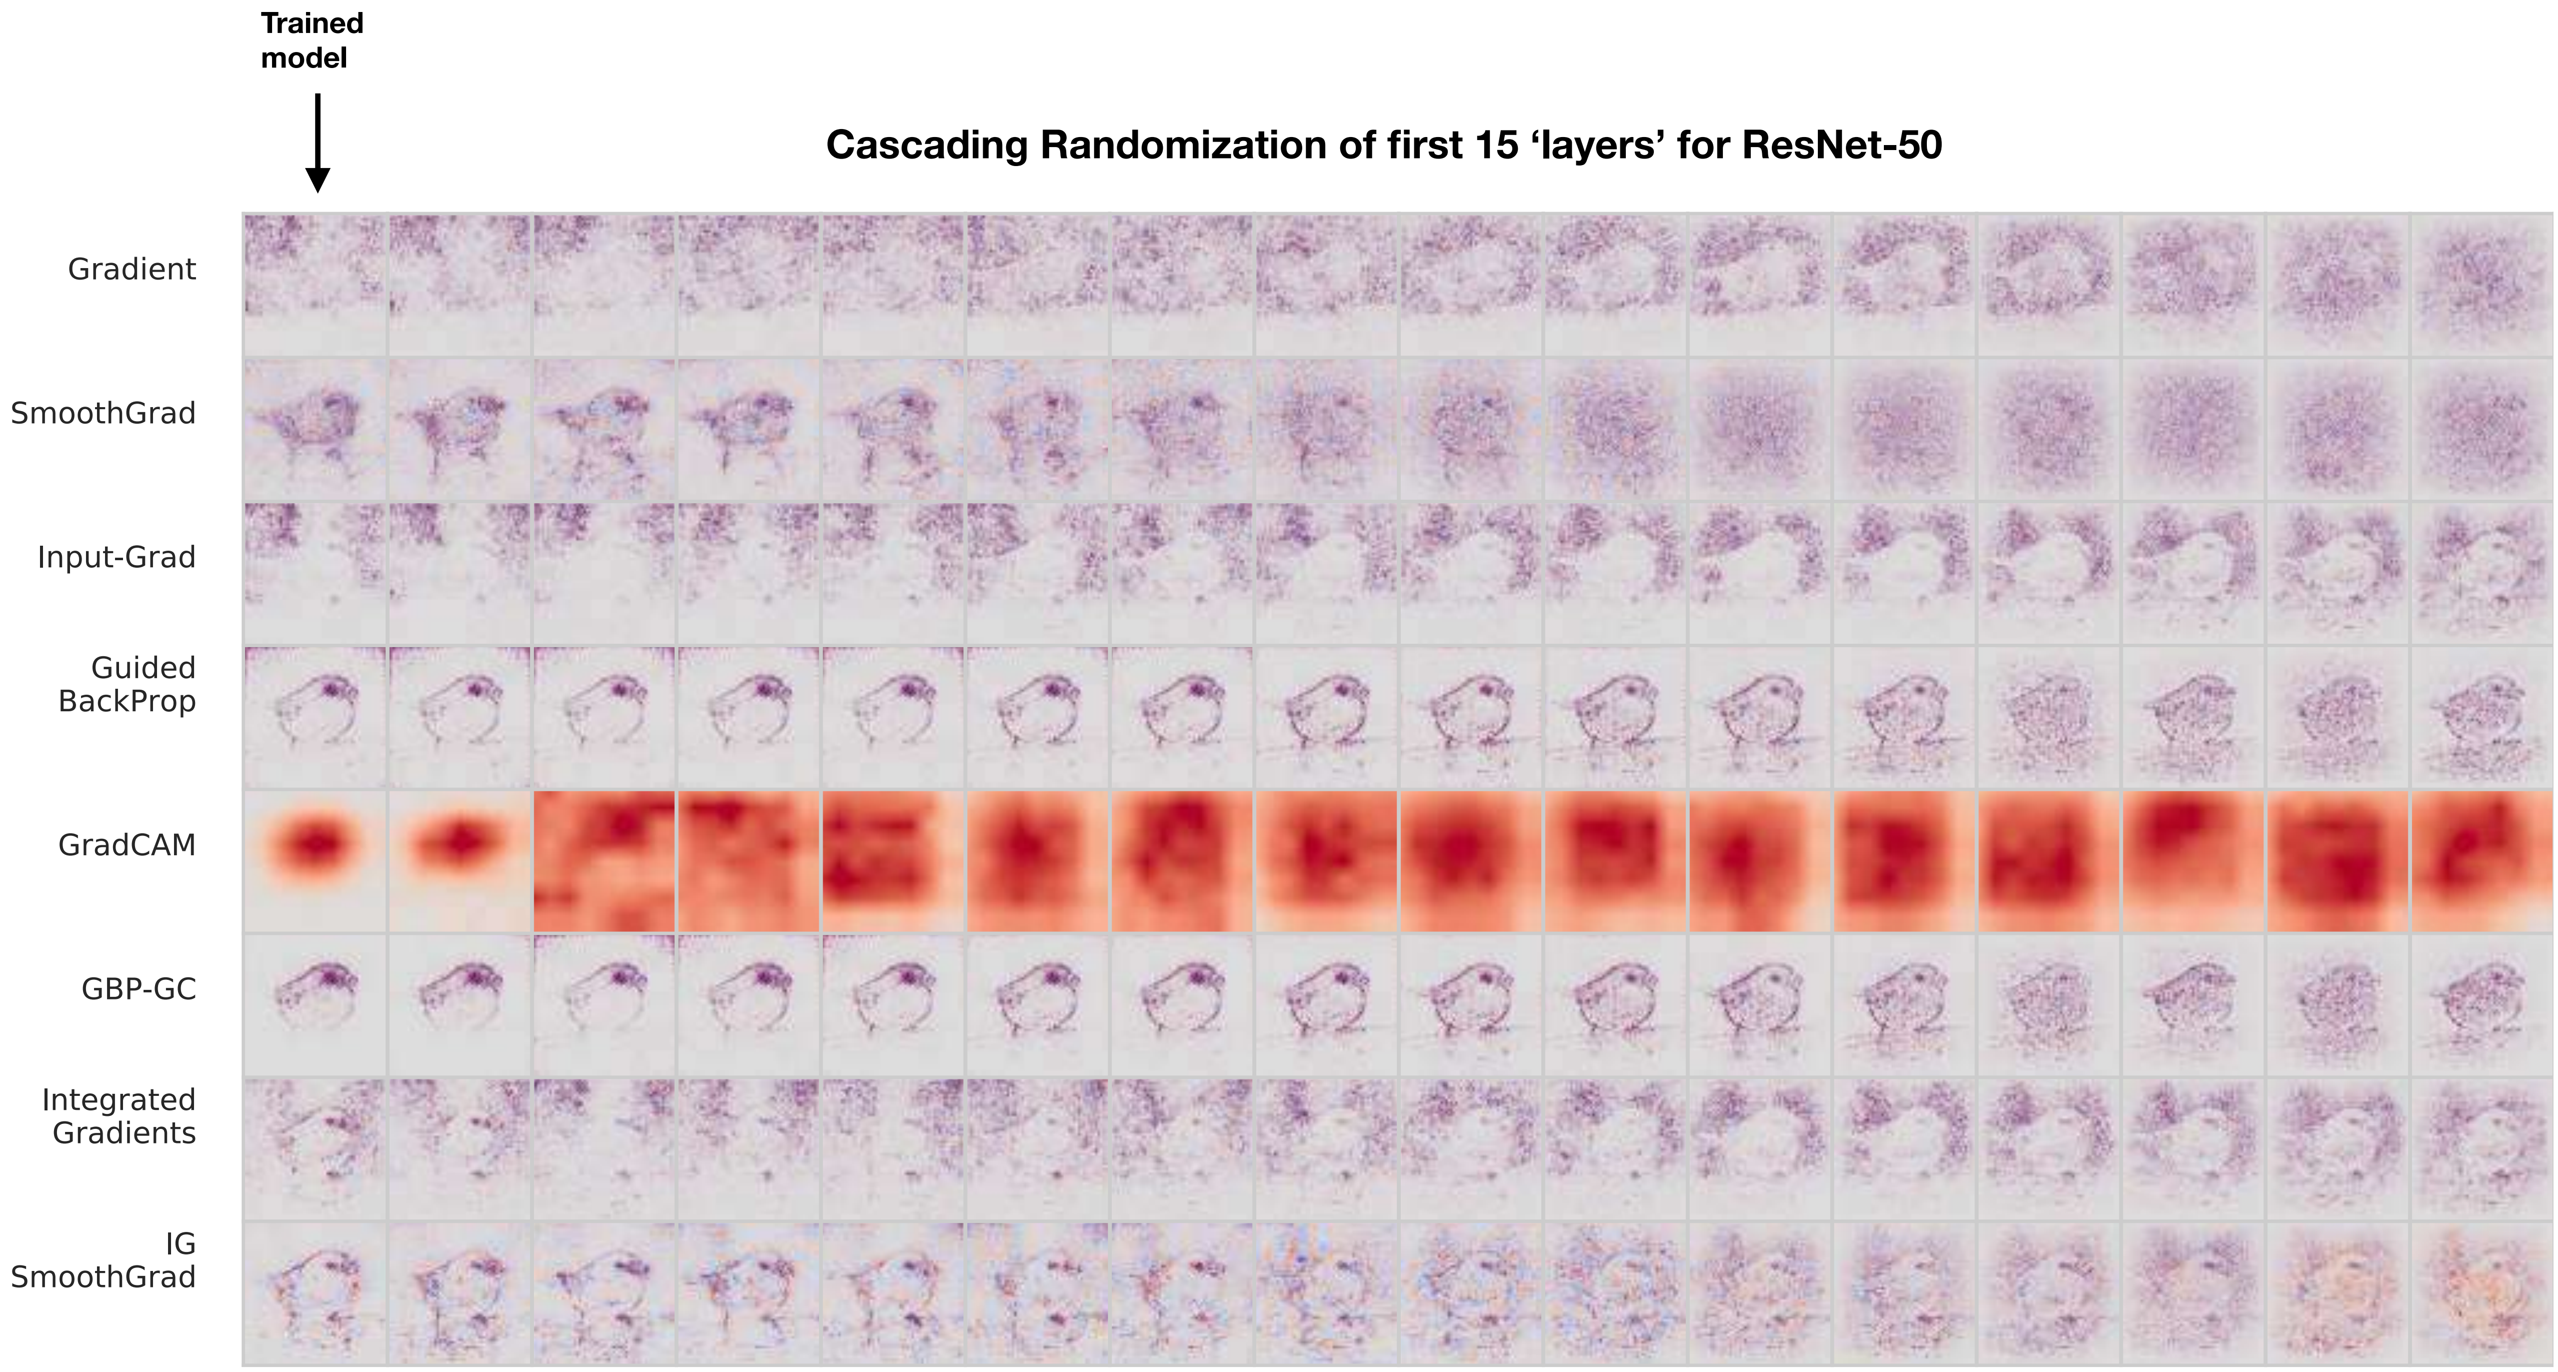

Trained model
Cascading Randomization of first 15 'layers' for ResNet-50
Gradient
SmoothGrad
Input-Grad
Guided BackProp
GradCAM
GBP-GC
Integrated Gradients
IG SmoothGrad

# User Study DemoGraphics

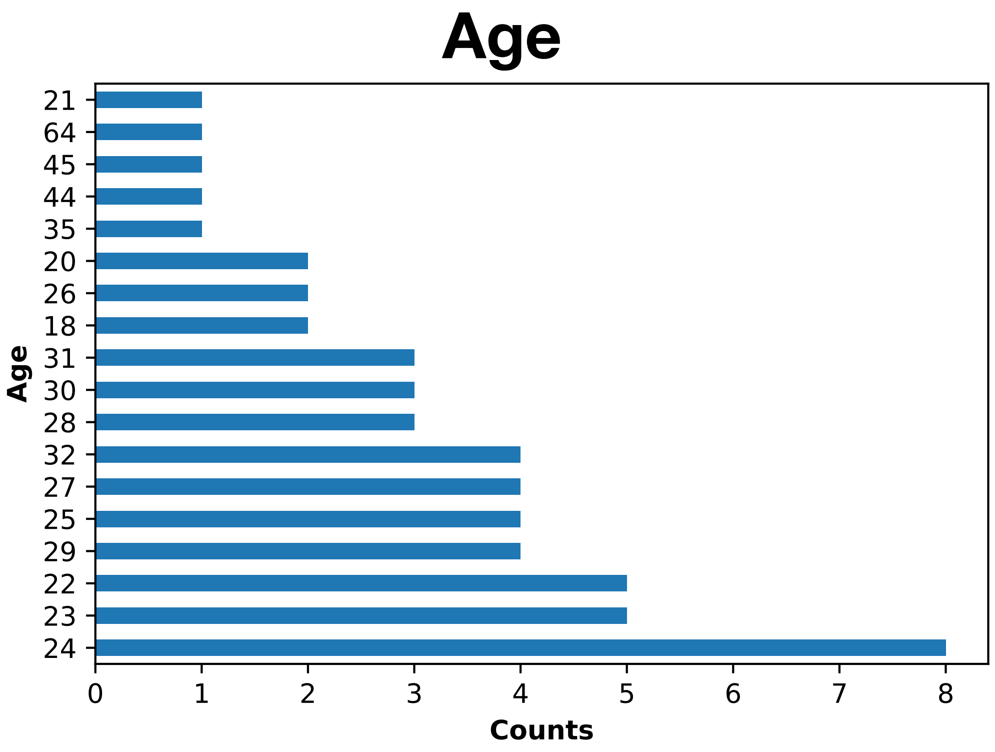
Age
21
64
45
44
35
20
26
18
31
30
28
32
27
25
29
22
23
24
Age
0 1 2 3 4 5 6 7 8
Counts

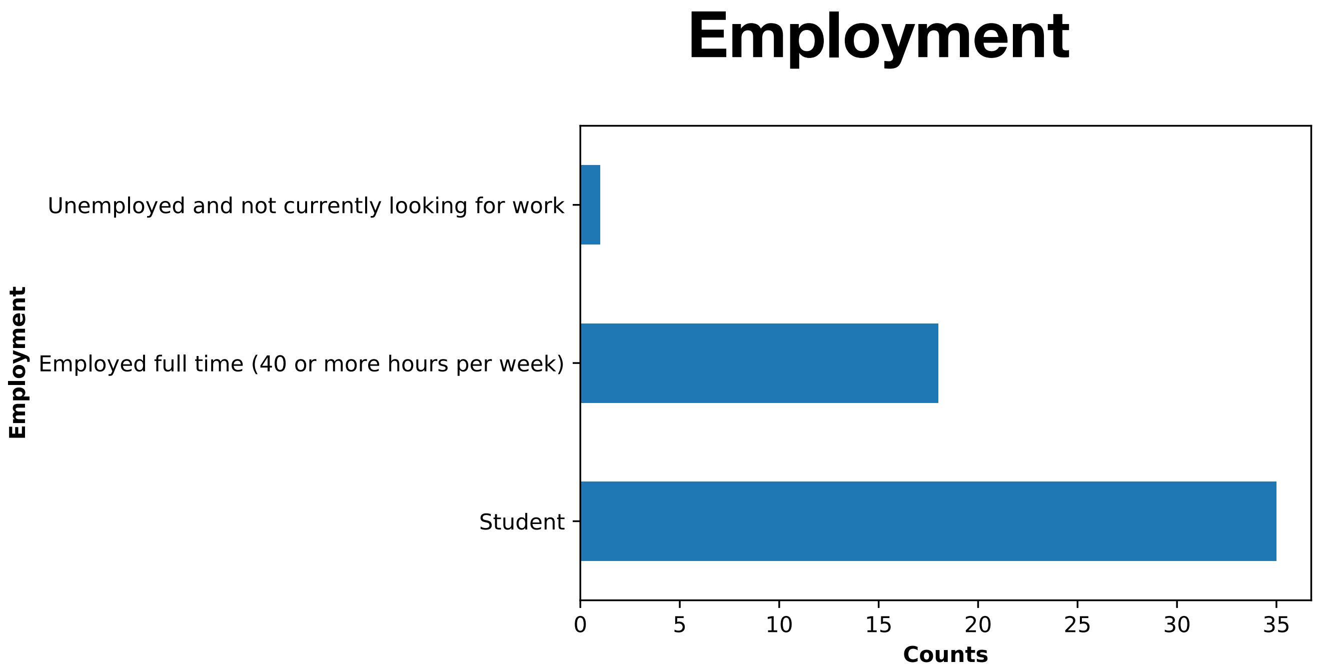
Employment
Unemployed and not currently looking for work
Employed full time (40 or more hours per week)
Student
Employment
0 5 10 15 20 25 30 35
Counts

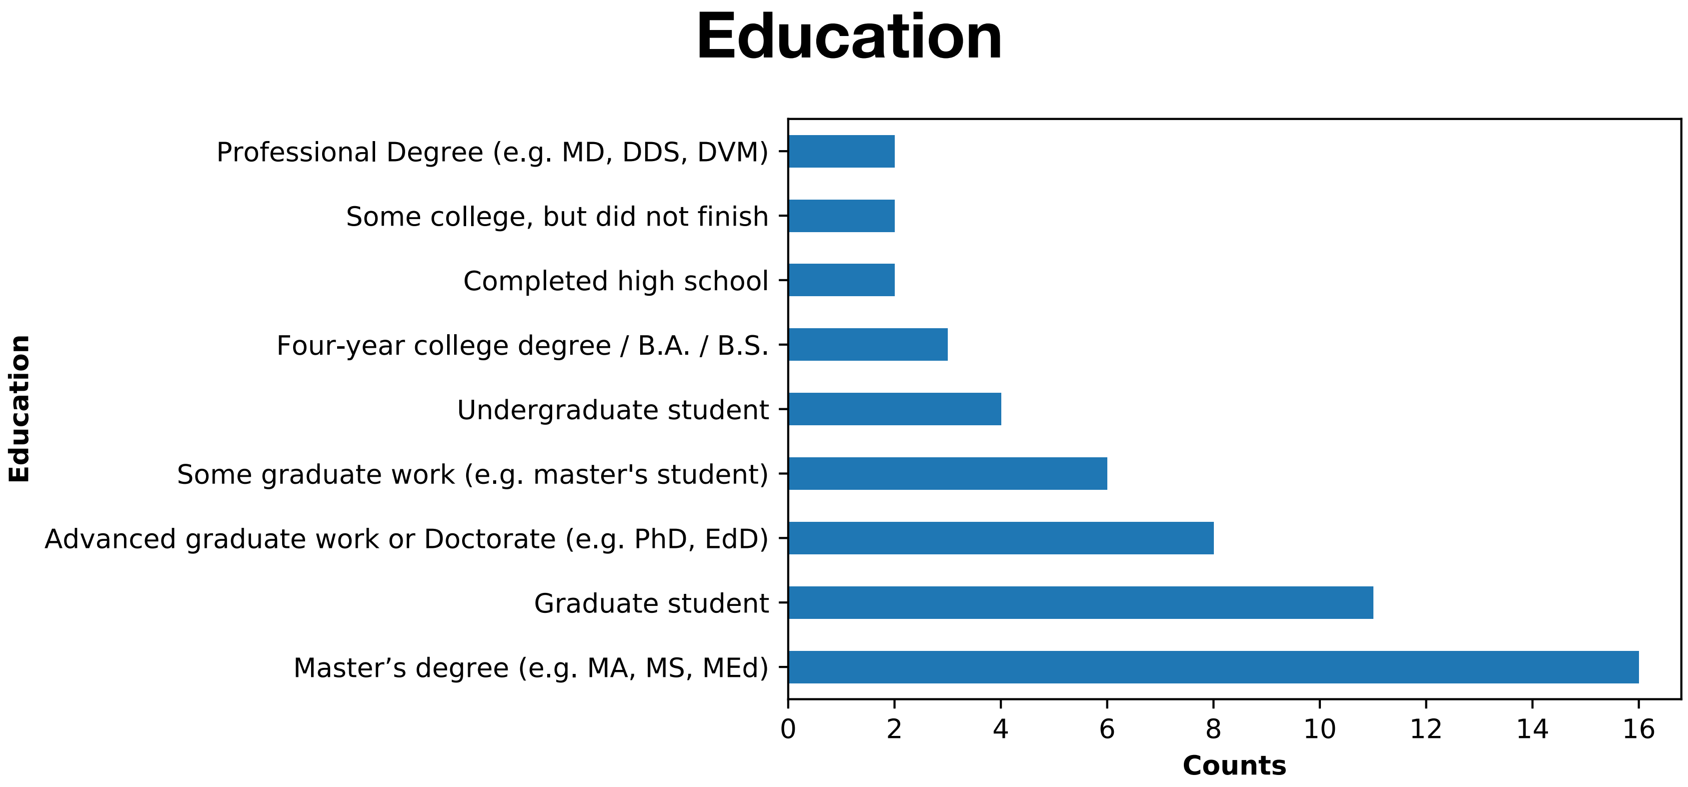
Education
Professional Degree (e.g. MD, DDS, DVM)
Some college, but did not finish
Completed high school
Four-year college degree / B.A. / B.S.
Undergraduate student
Some graduate work (e.g. master's student)
Advanced graduate work or Doctorate (e.g. PhD, EdD)
Graduate student
Master’s degree (e.g. MA, MS, MEd)
Education
0 2 4 6 8 10 12 14 16
Counts

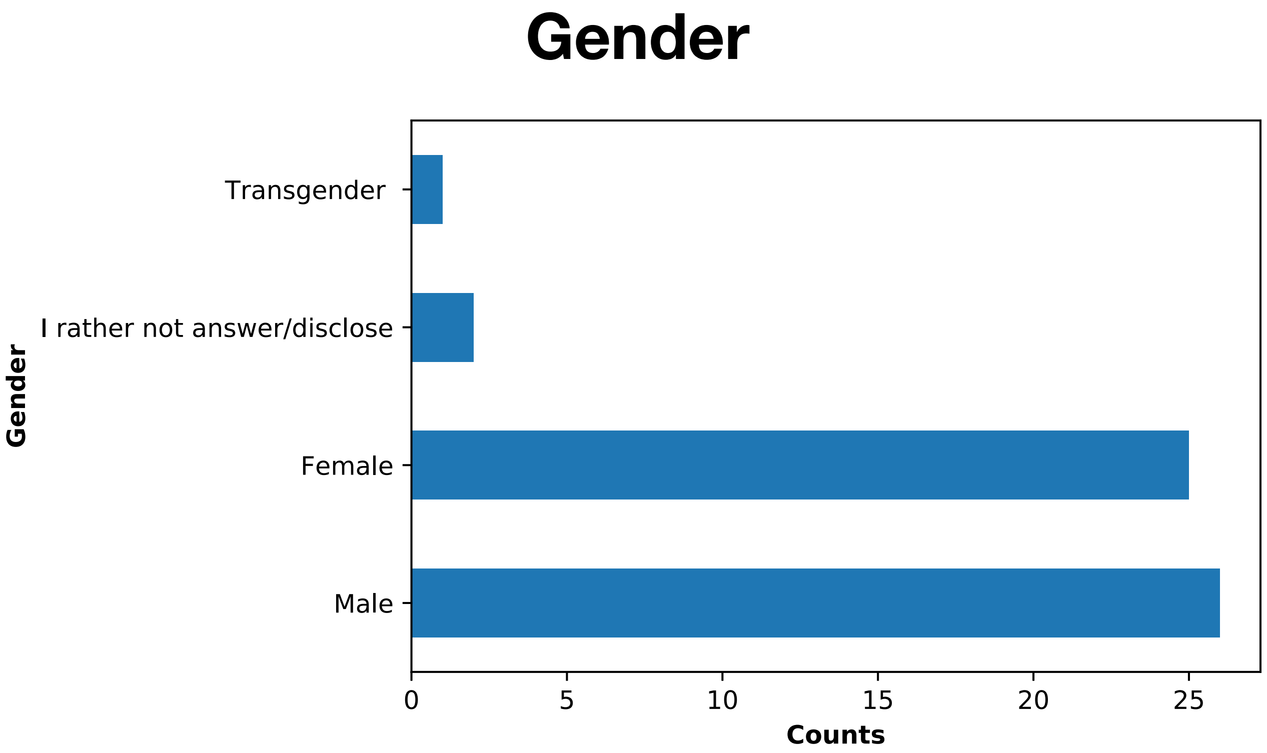
Gender
Transgender
I rather not answer/disclose
Female
Male
Gender
0
5
10
15
20
25
Counts

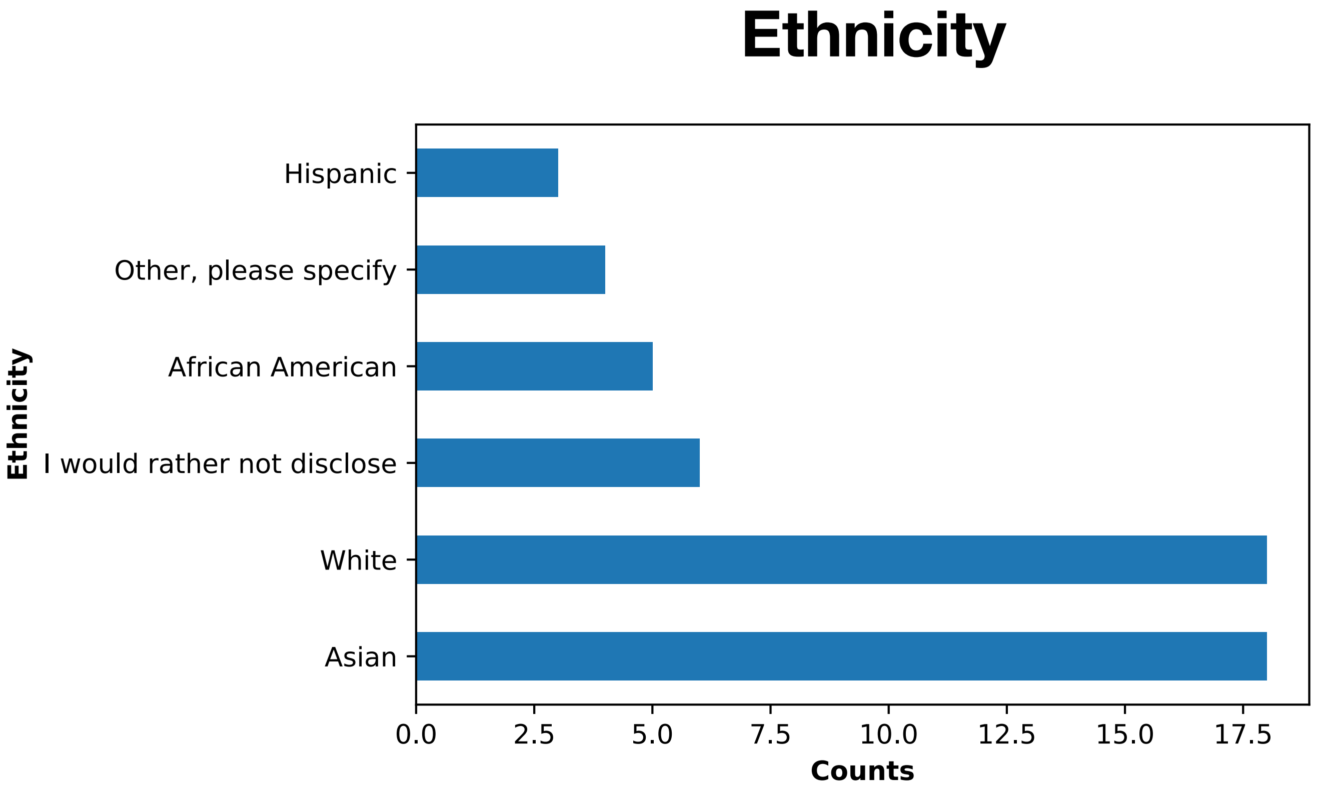
Ethnicity
Hispanic
Other, please specify
African American
I would rather not disclose
White
Asian
Ethnicity
0.0
2.5
5.0
7.5
10.0
12.5
15.0
17.5
Counts

# Machine Learning Experience

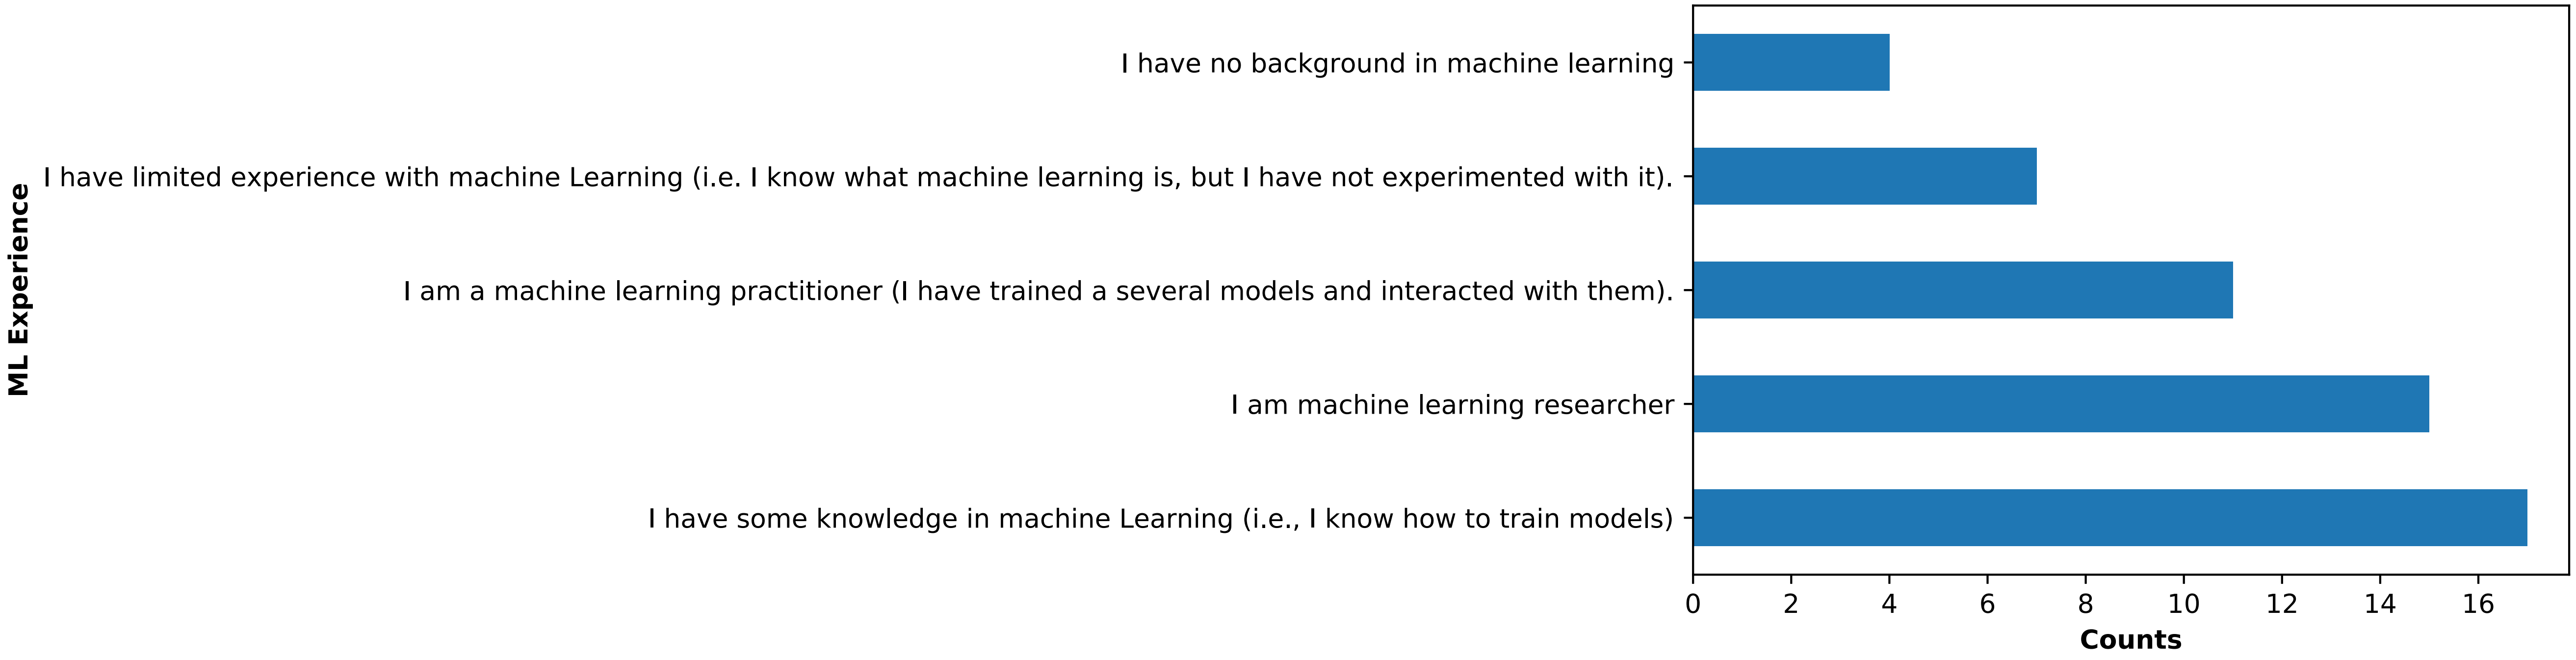


# Attribution Familiarity

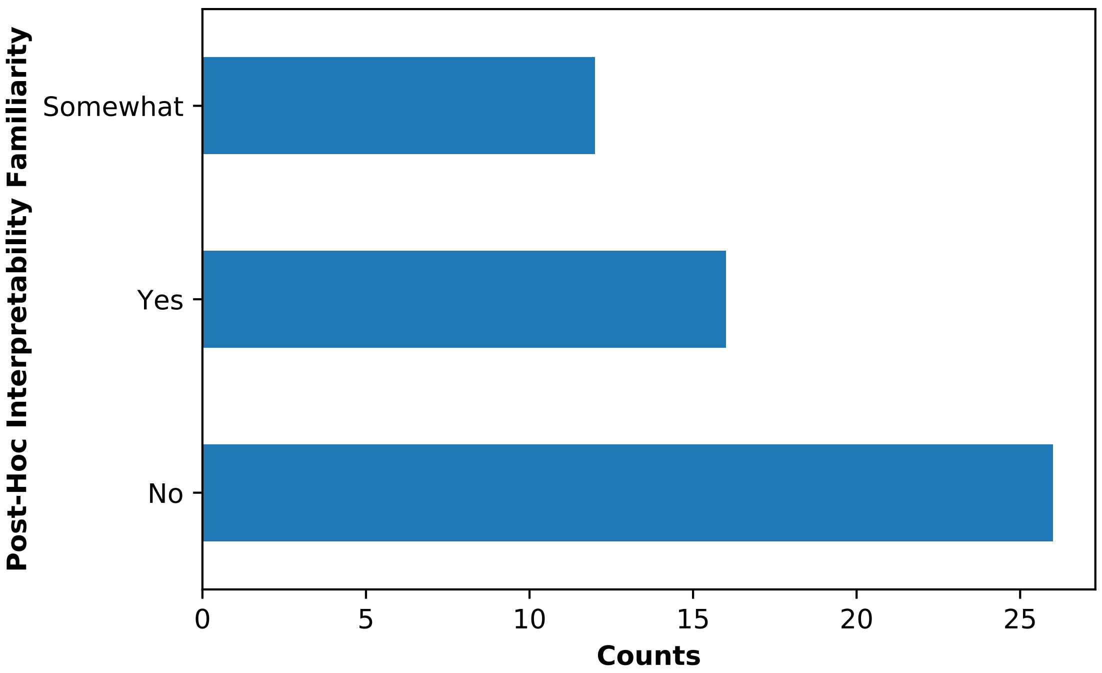

## Bamboo

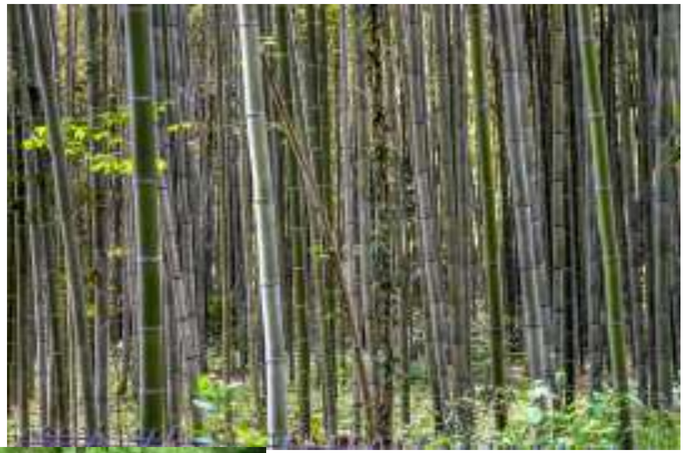

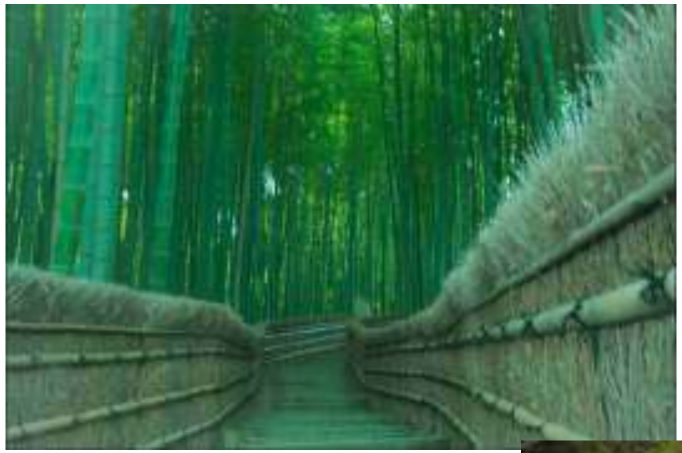

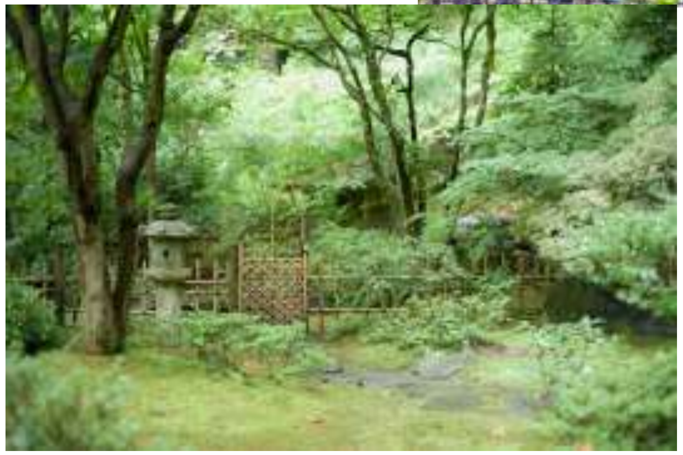

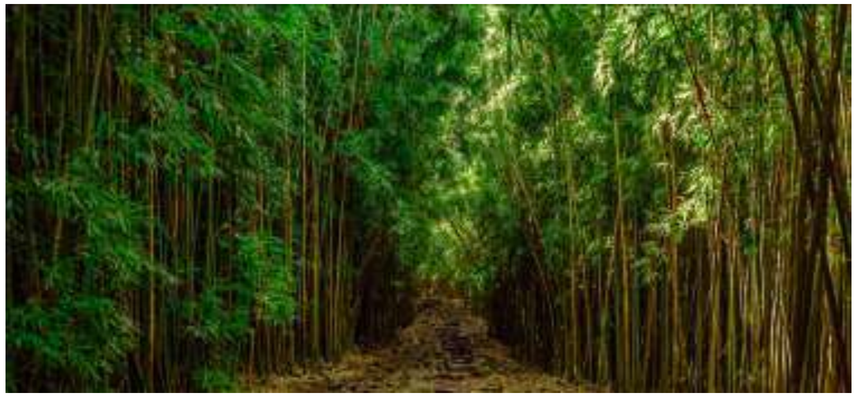

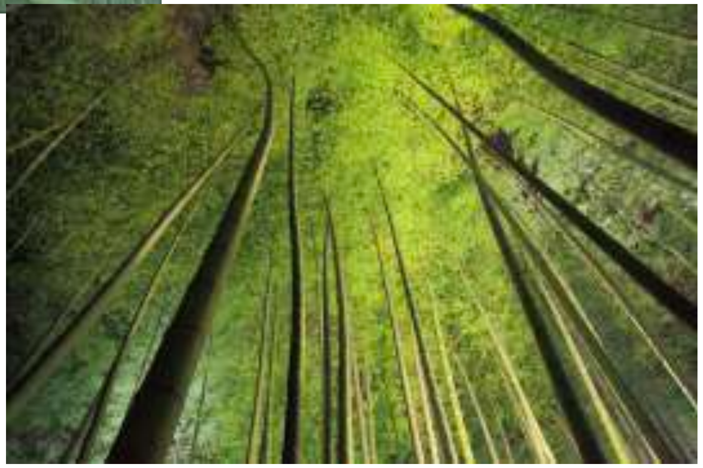

## Blue Sky

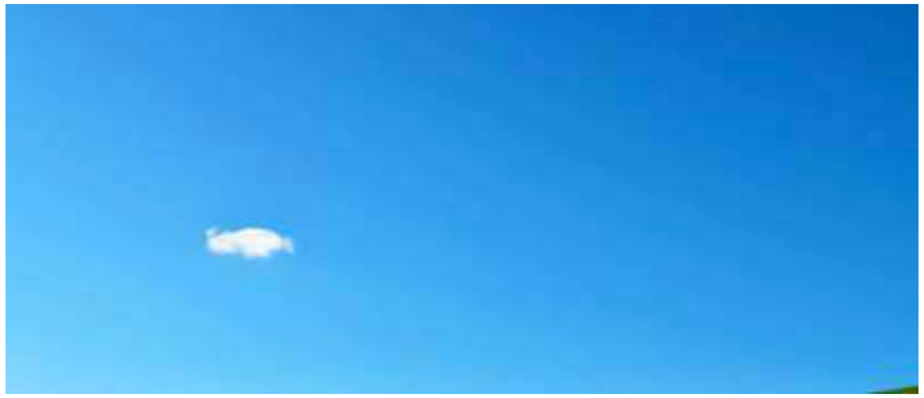

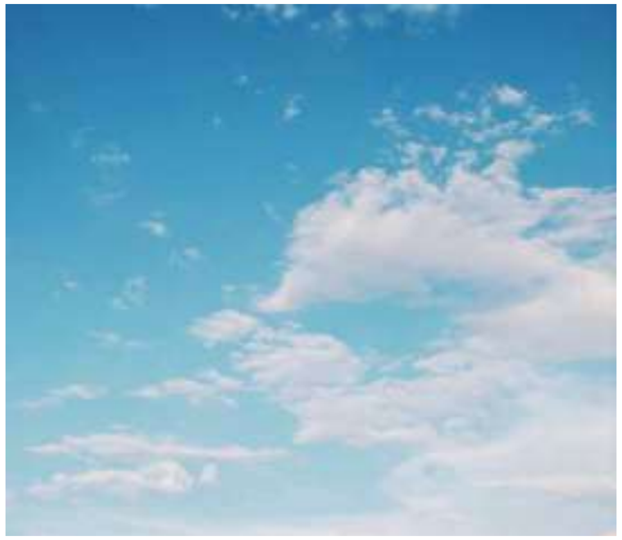

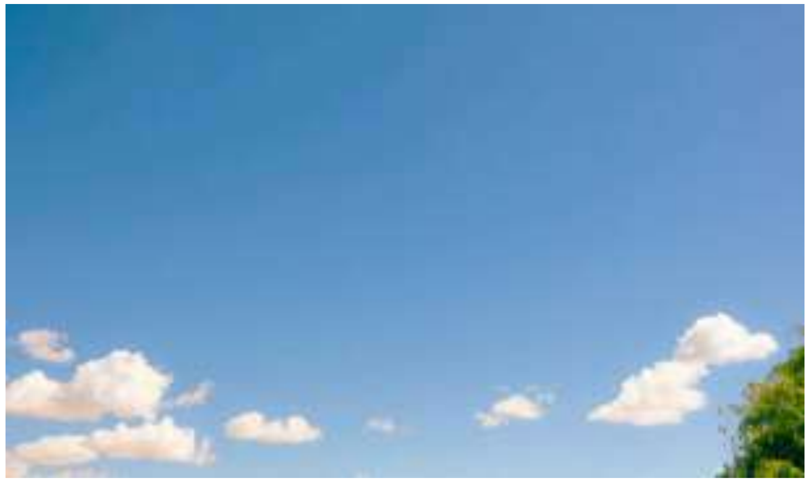

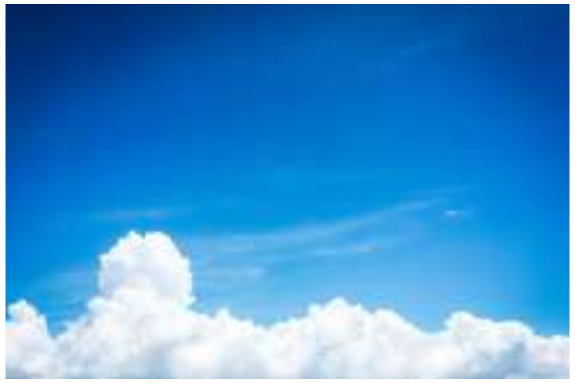

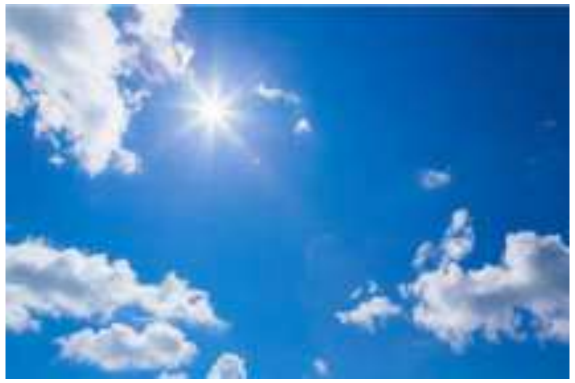

# Canyon

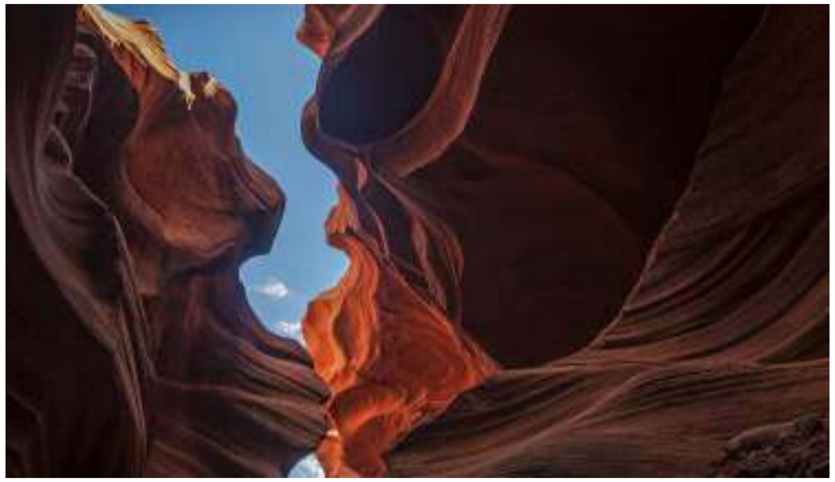
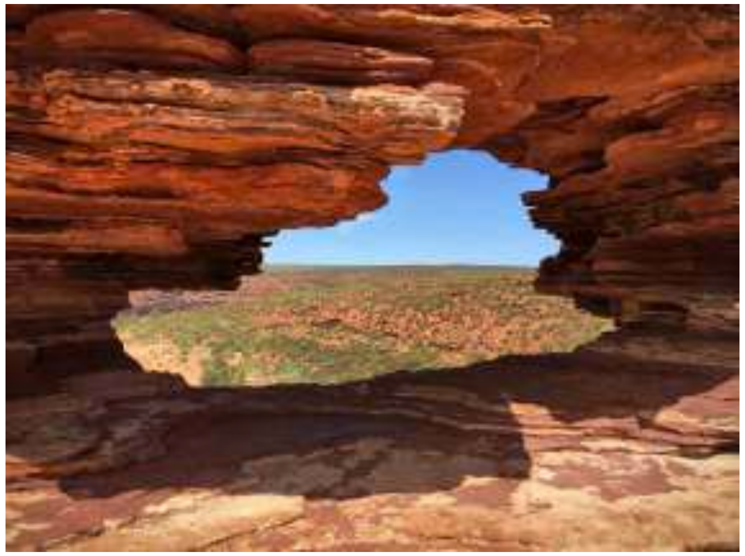
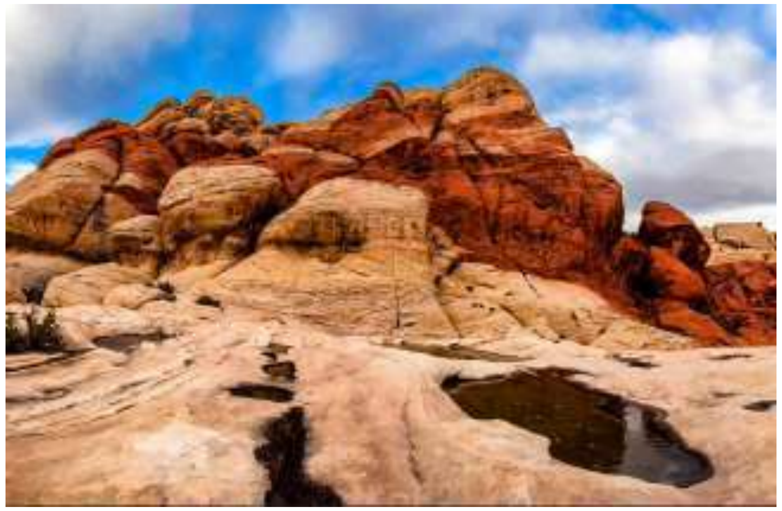
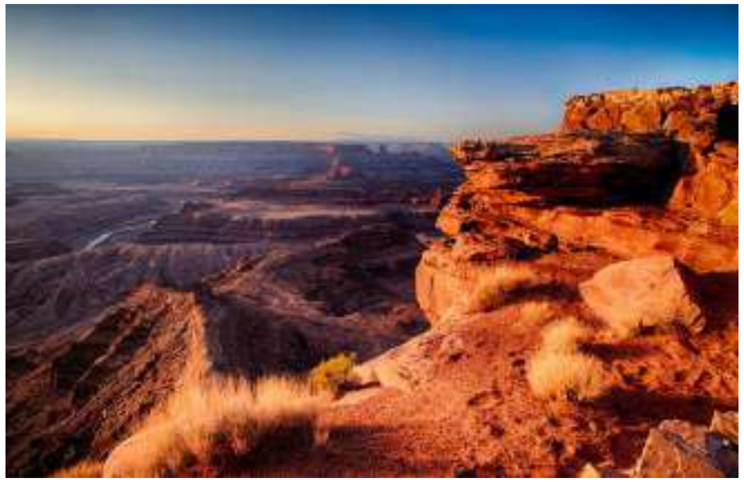
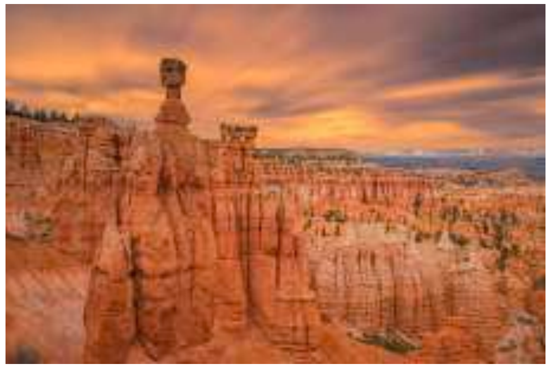

# Empty Room

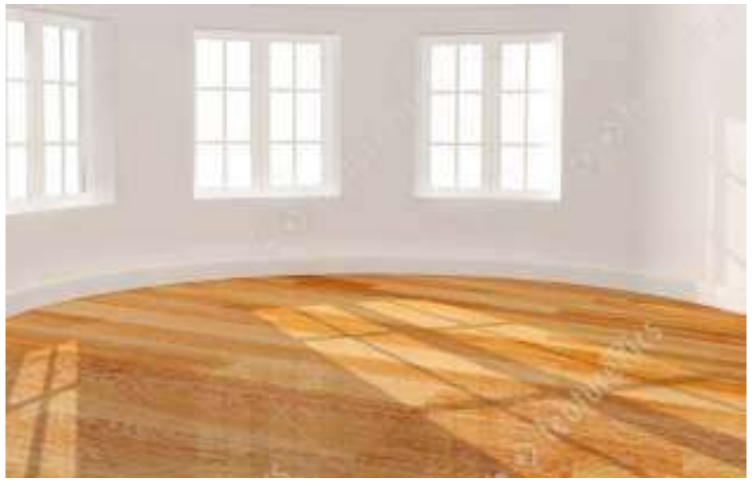
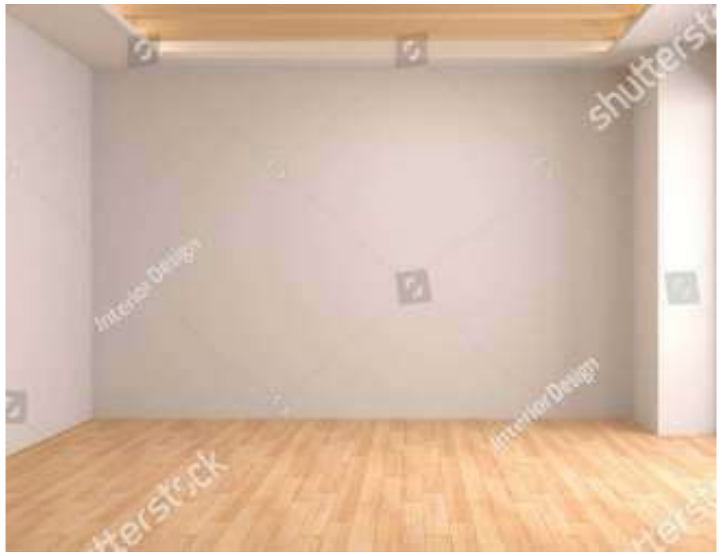
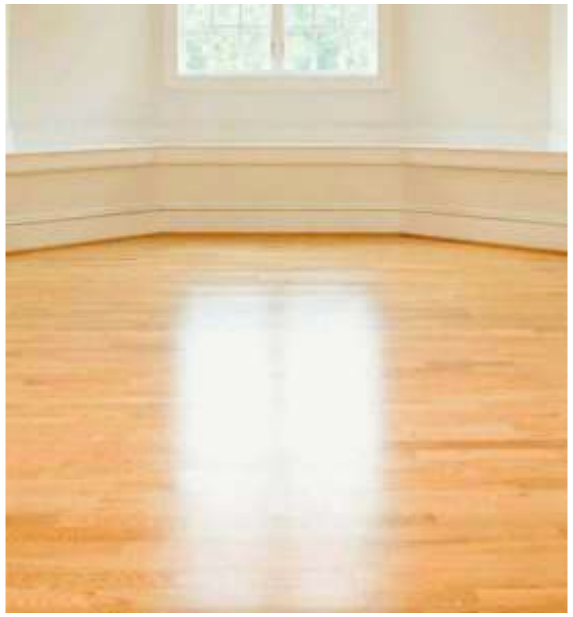
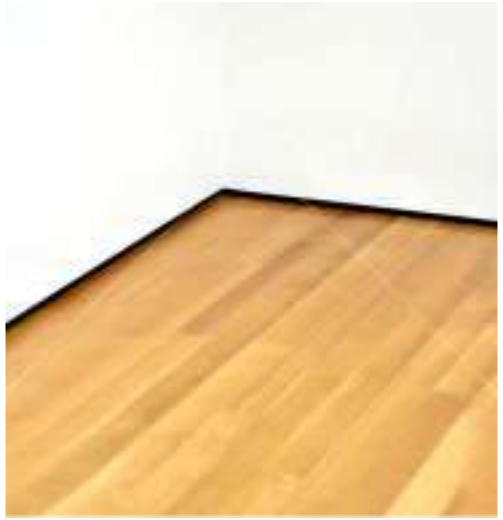

## Sand Dunes

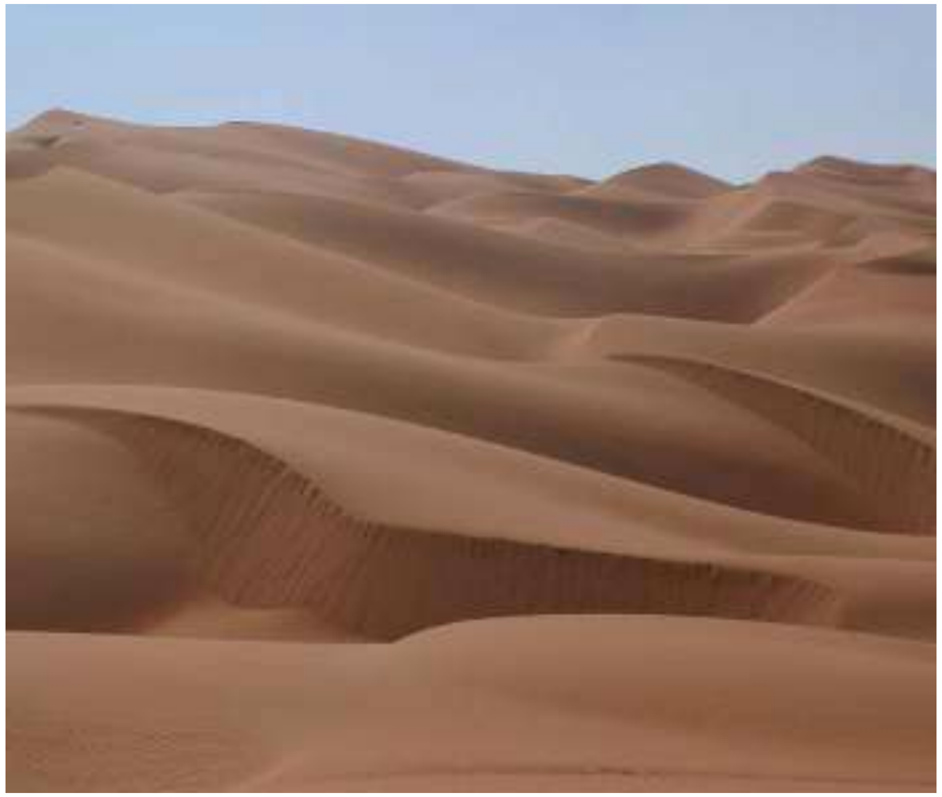
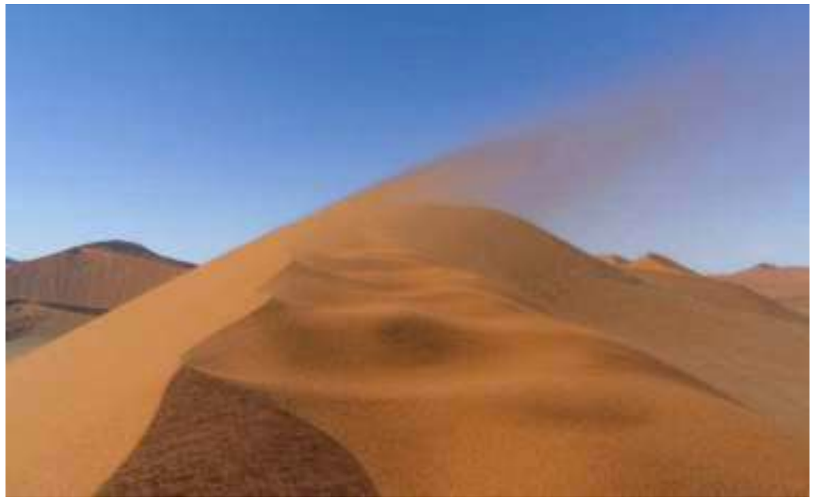
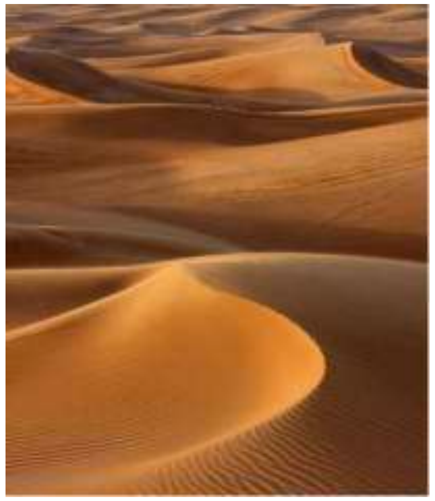
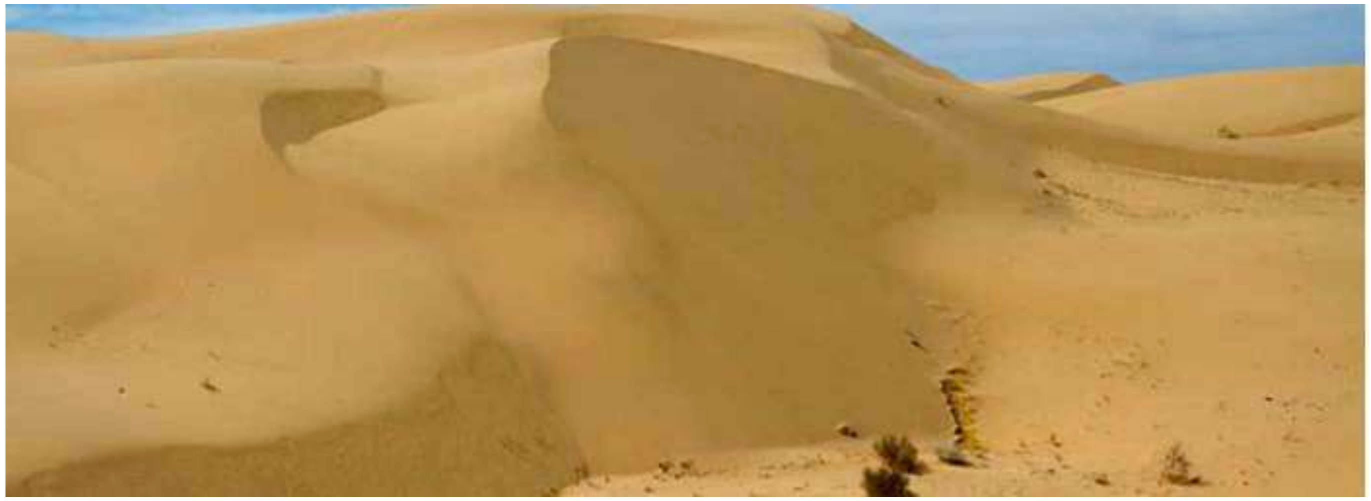

## High Way

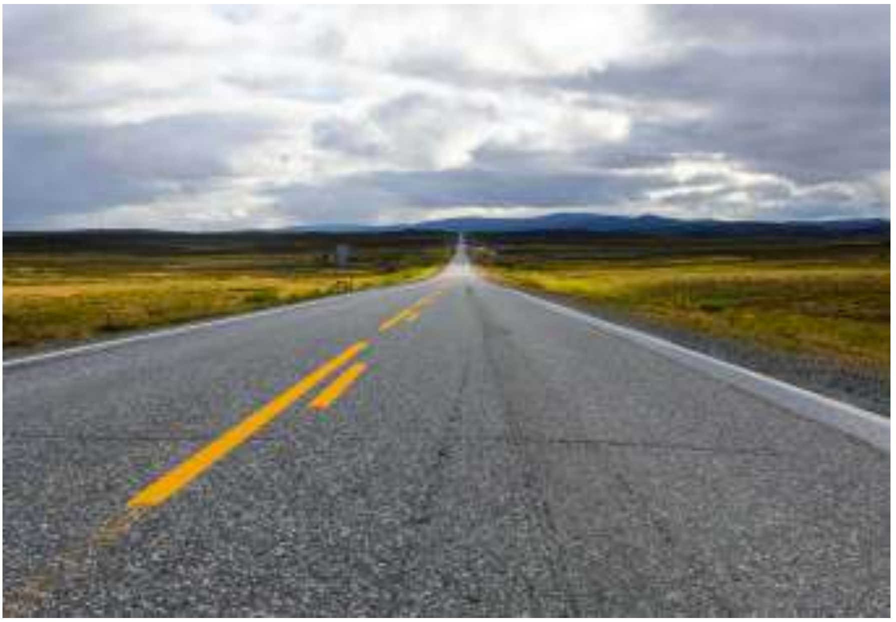
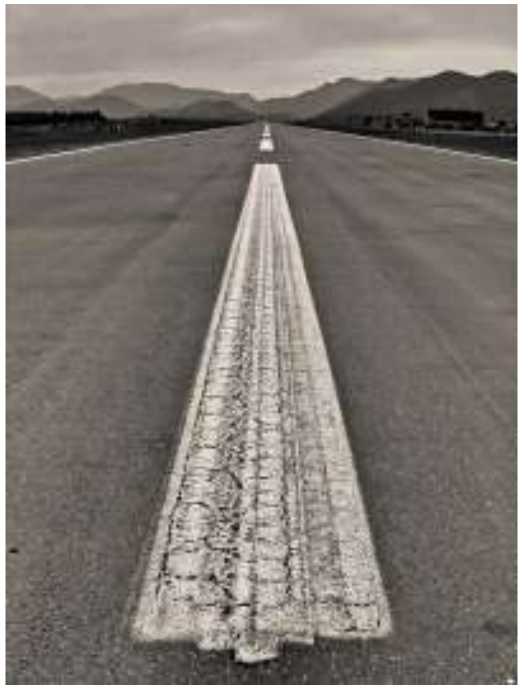
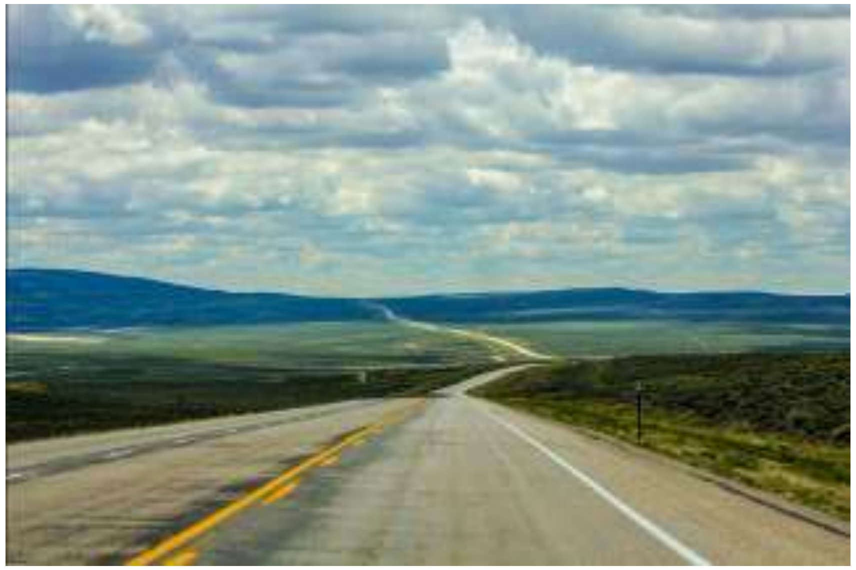
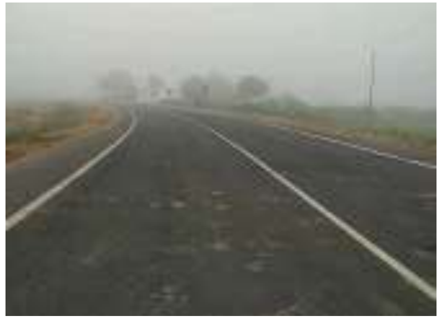

# Track

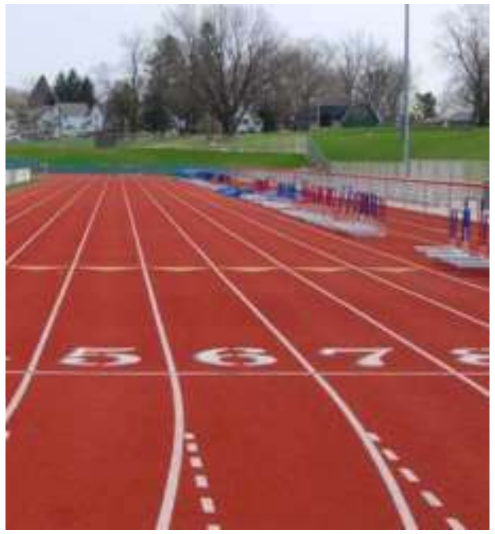

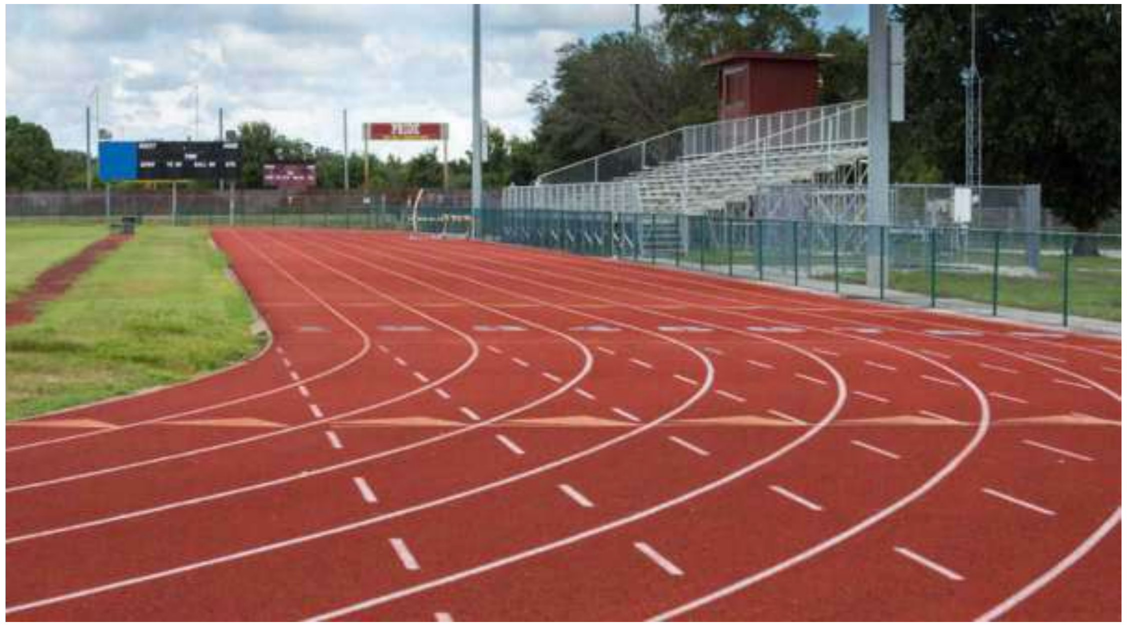

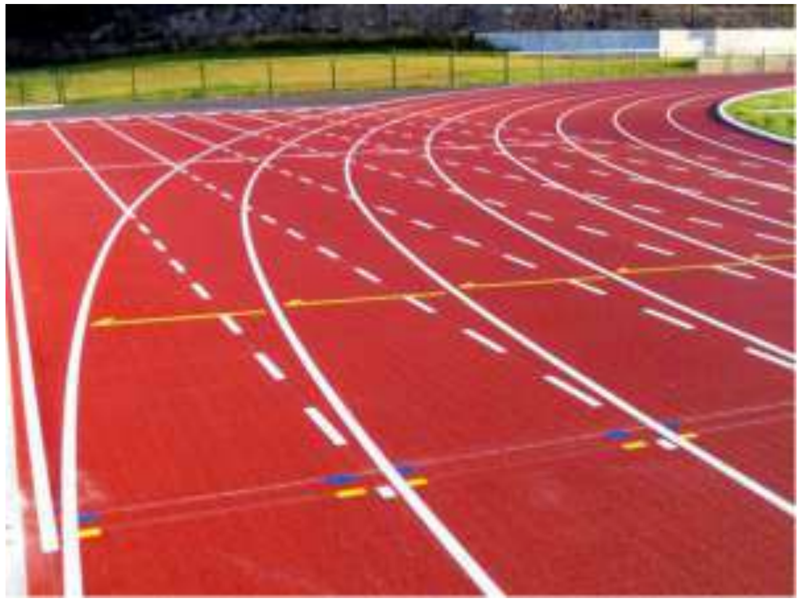

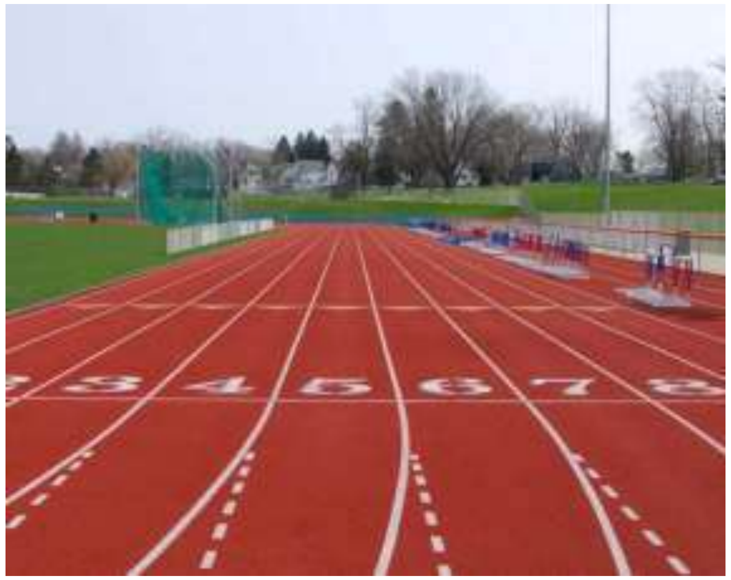

# Snow

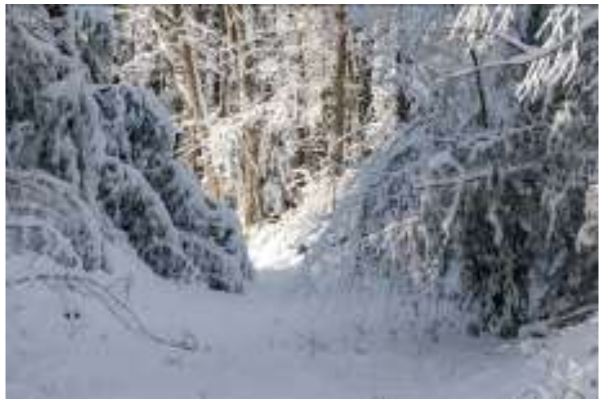

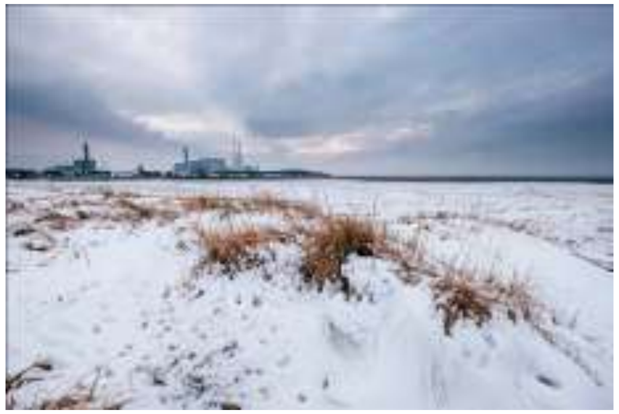

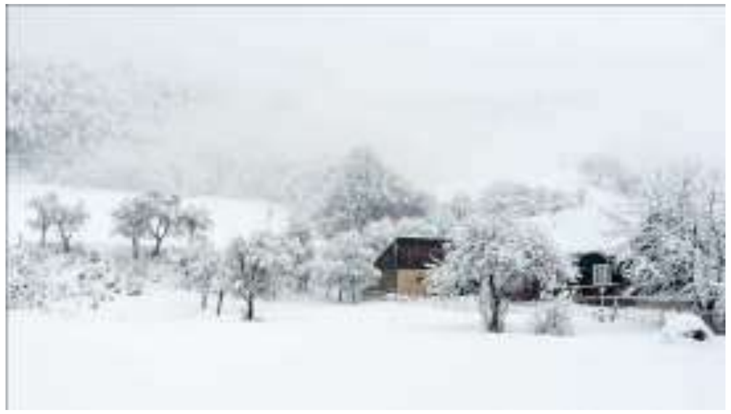

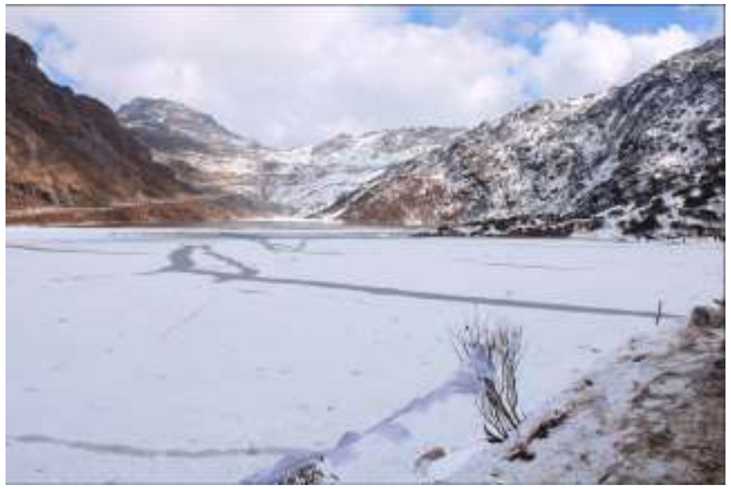

## Water Fall

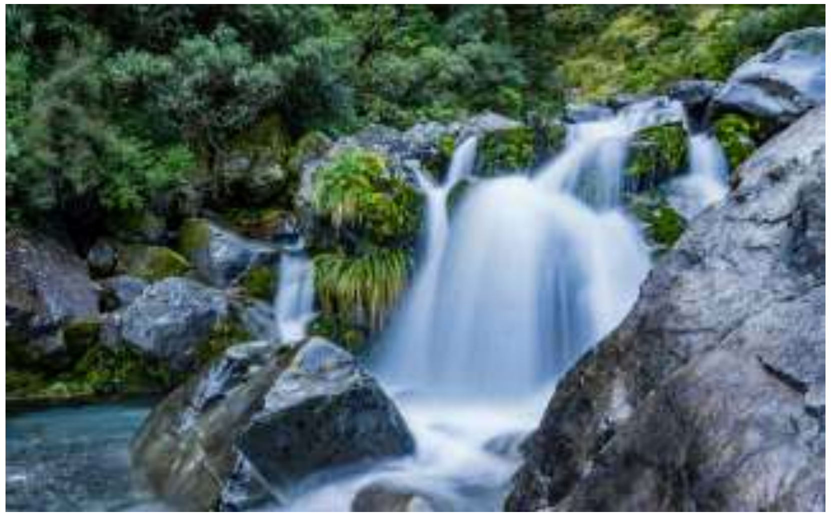
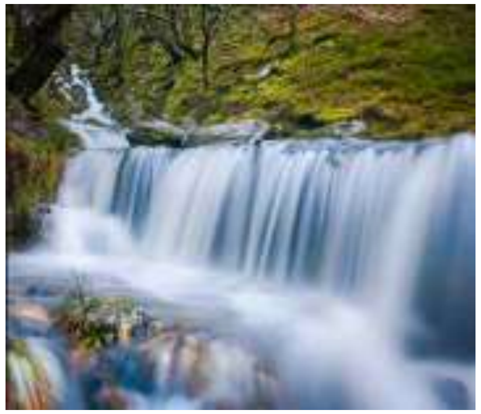
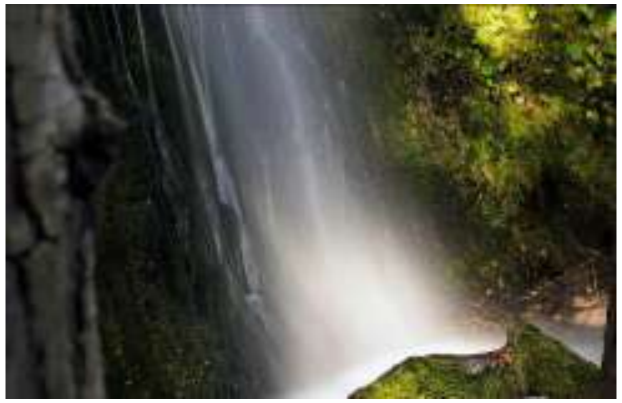
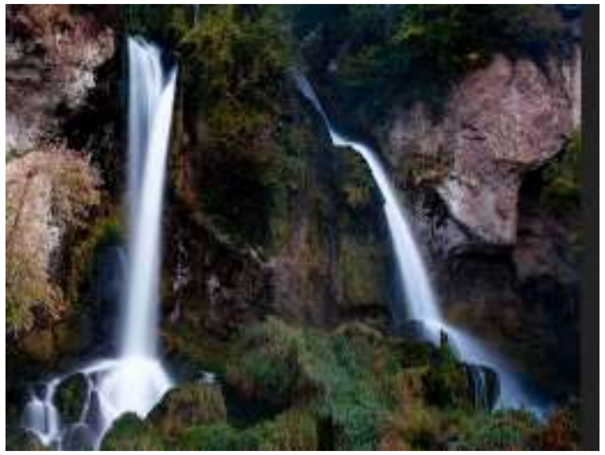

## Wheat Field

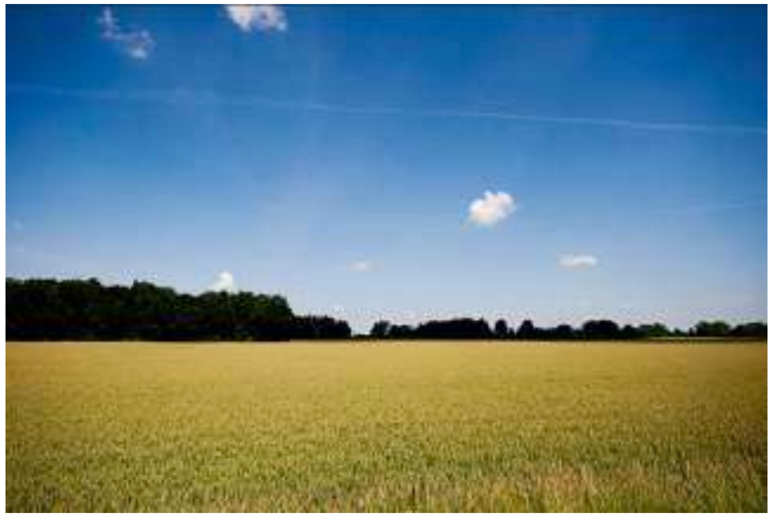
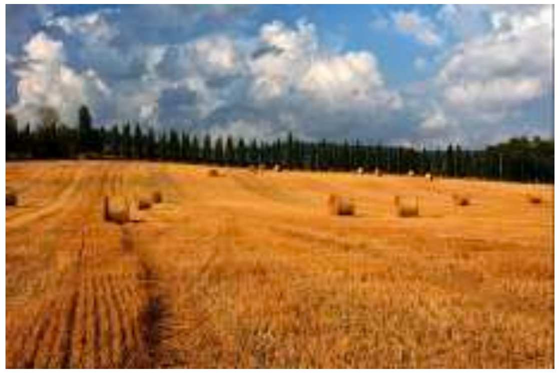
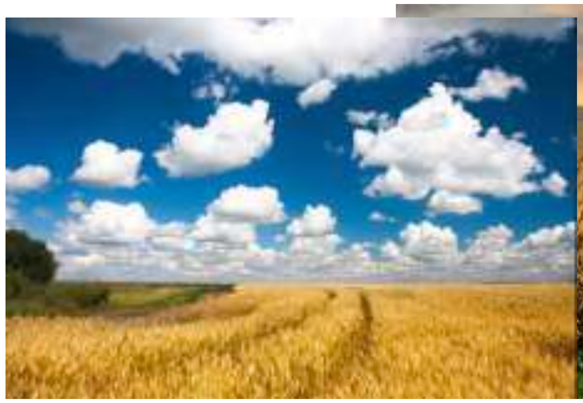
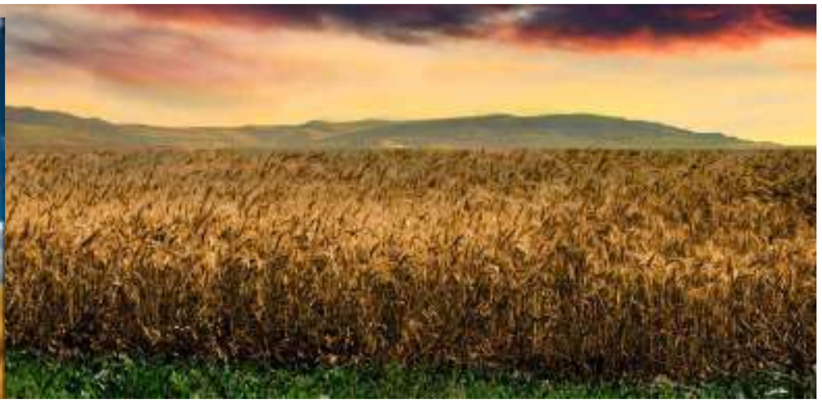

# Normal Model: Gradient

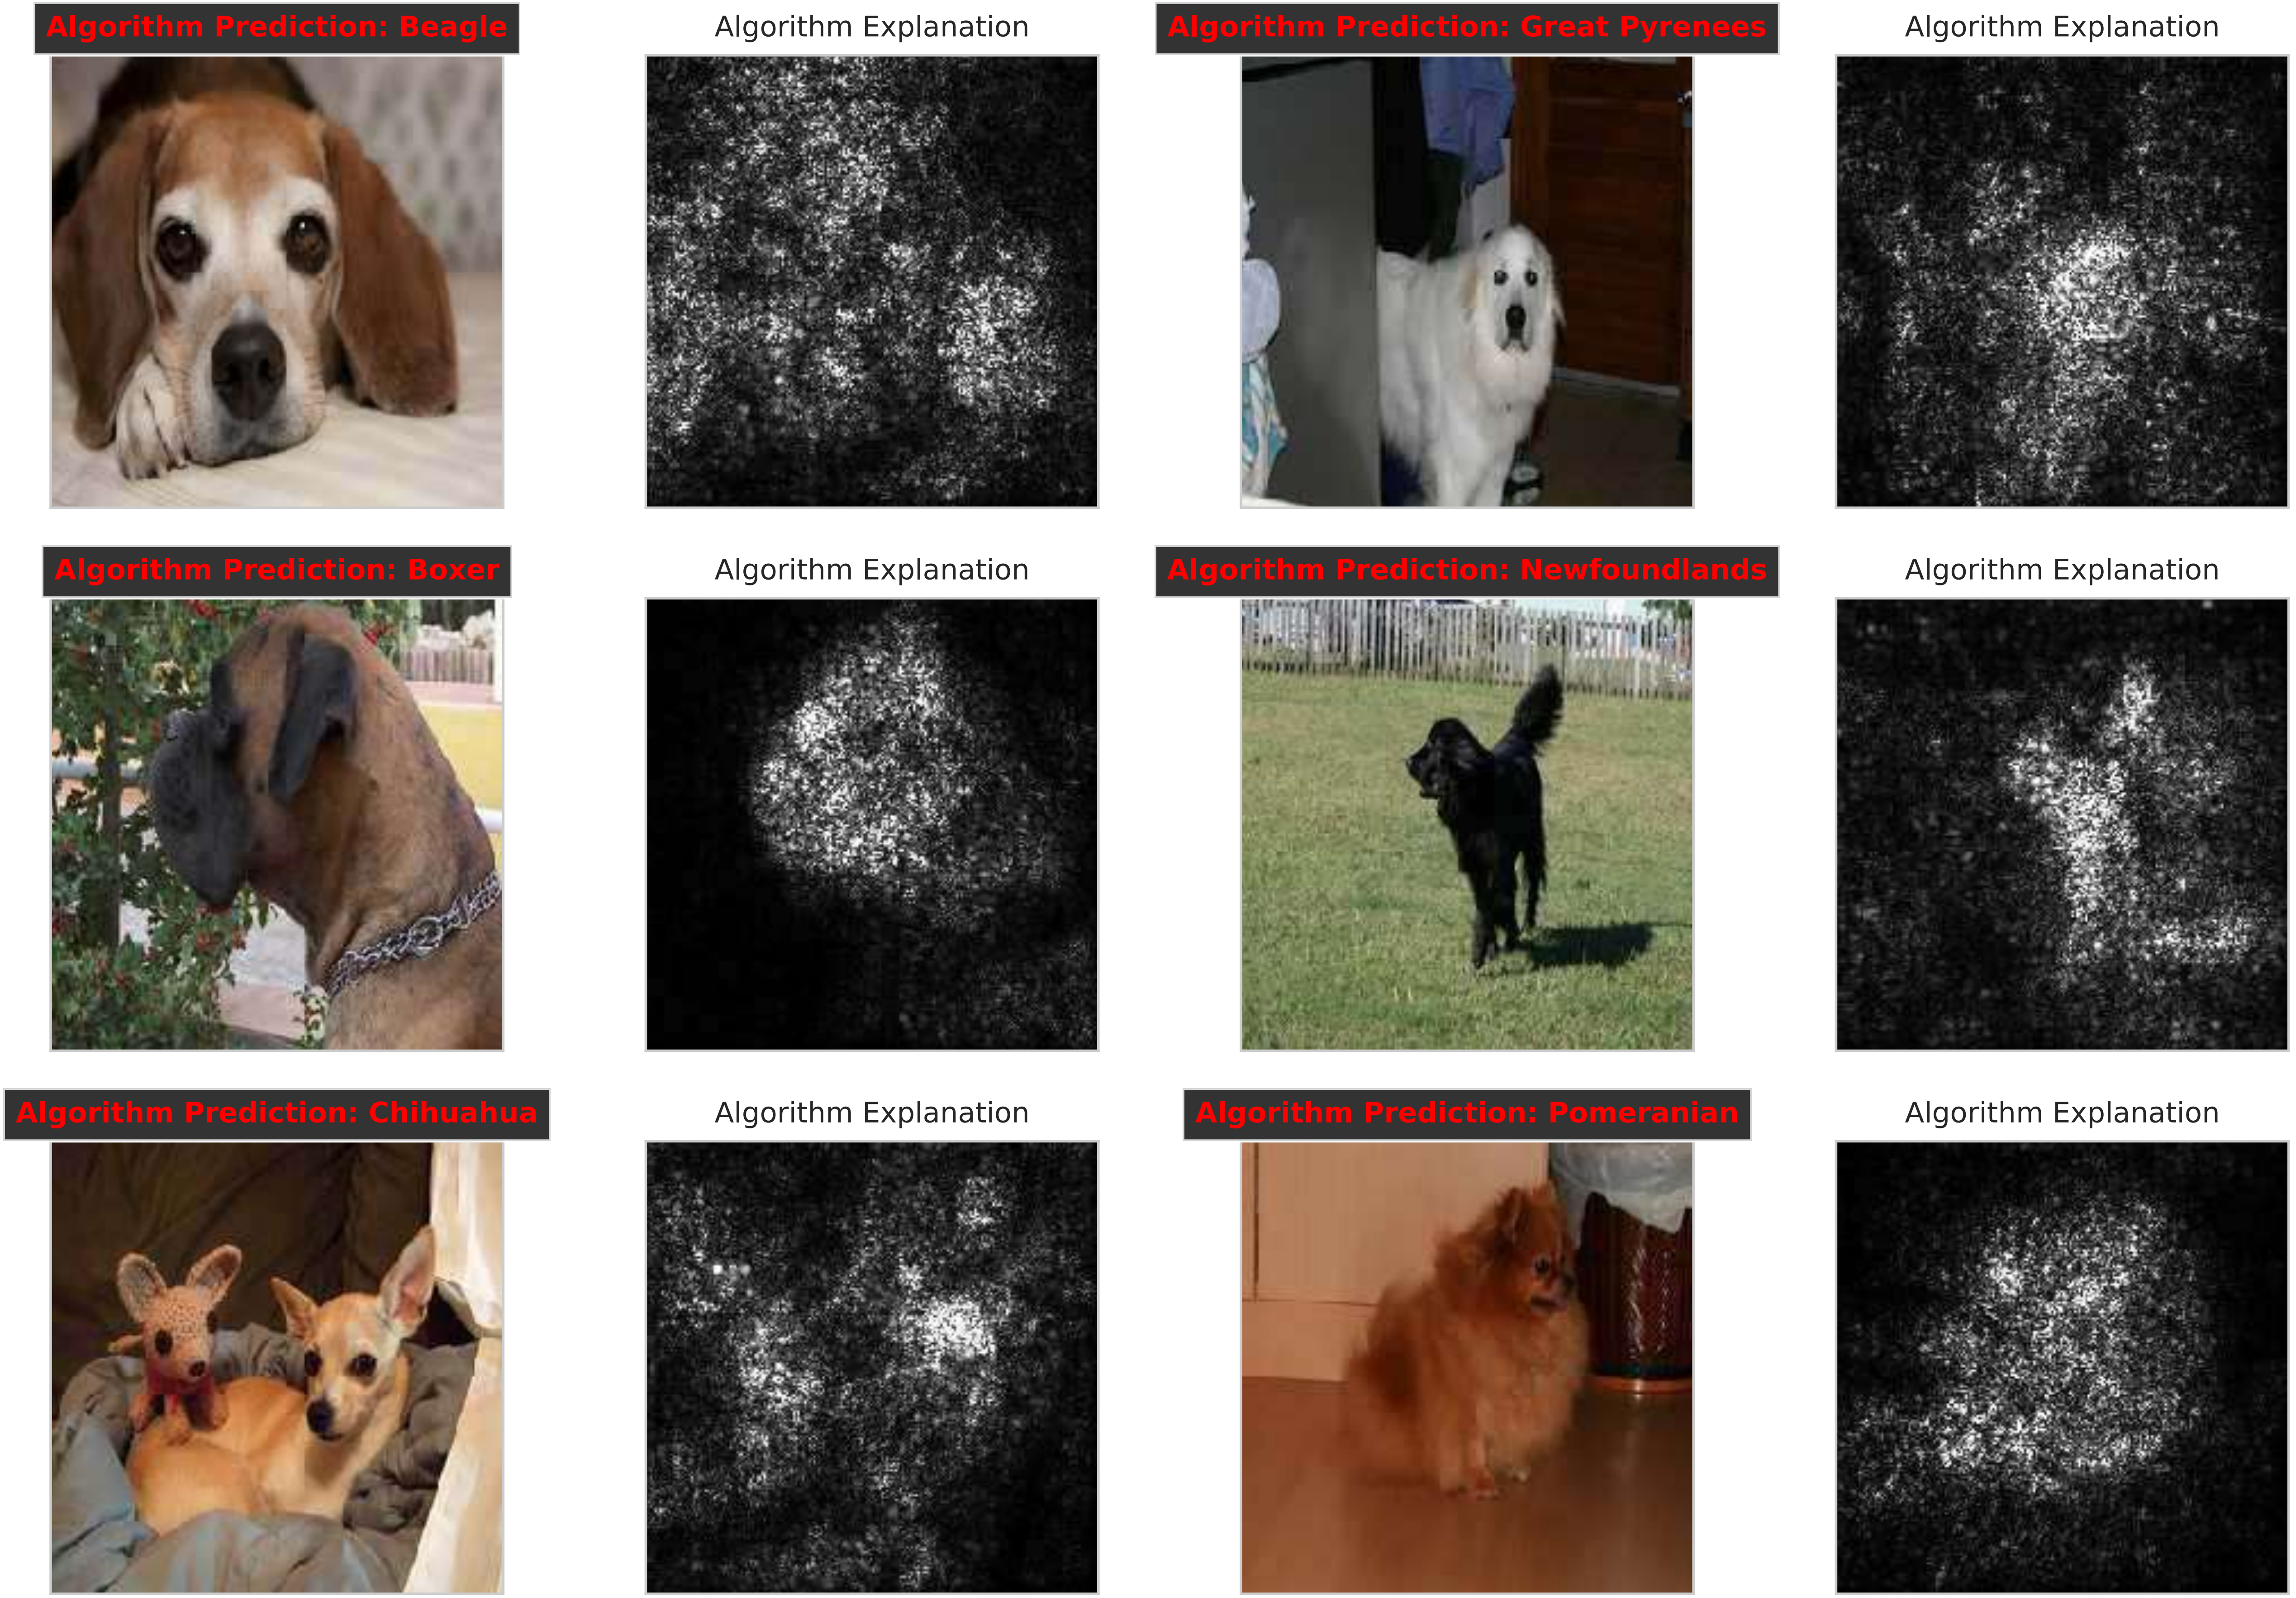

# Normal Model: SmoothGrad

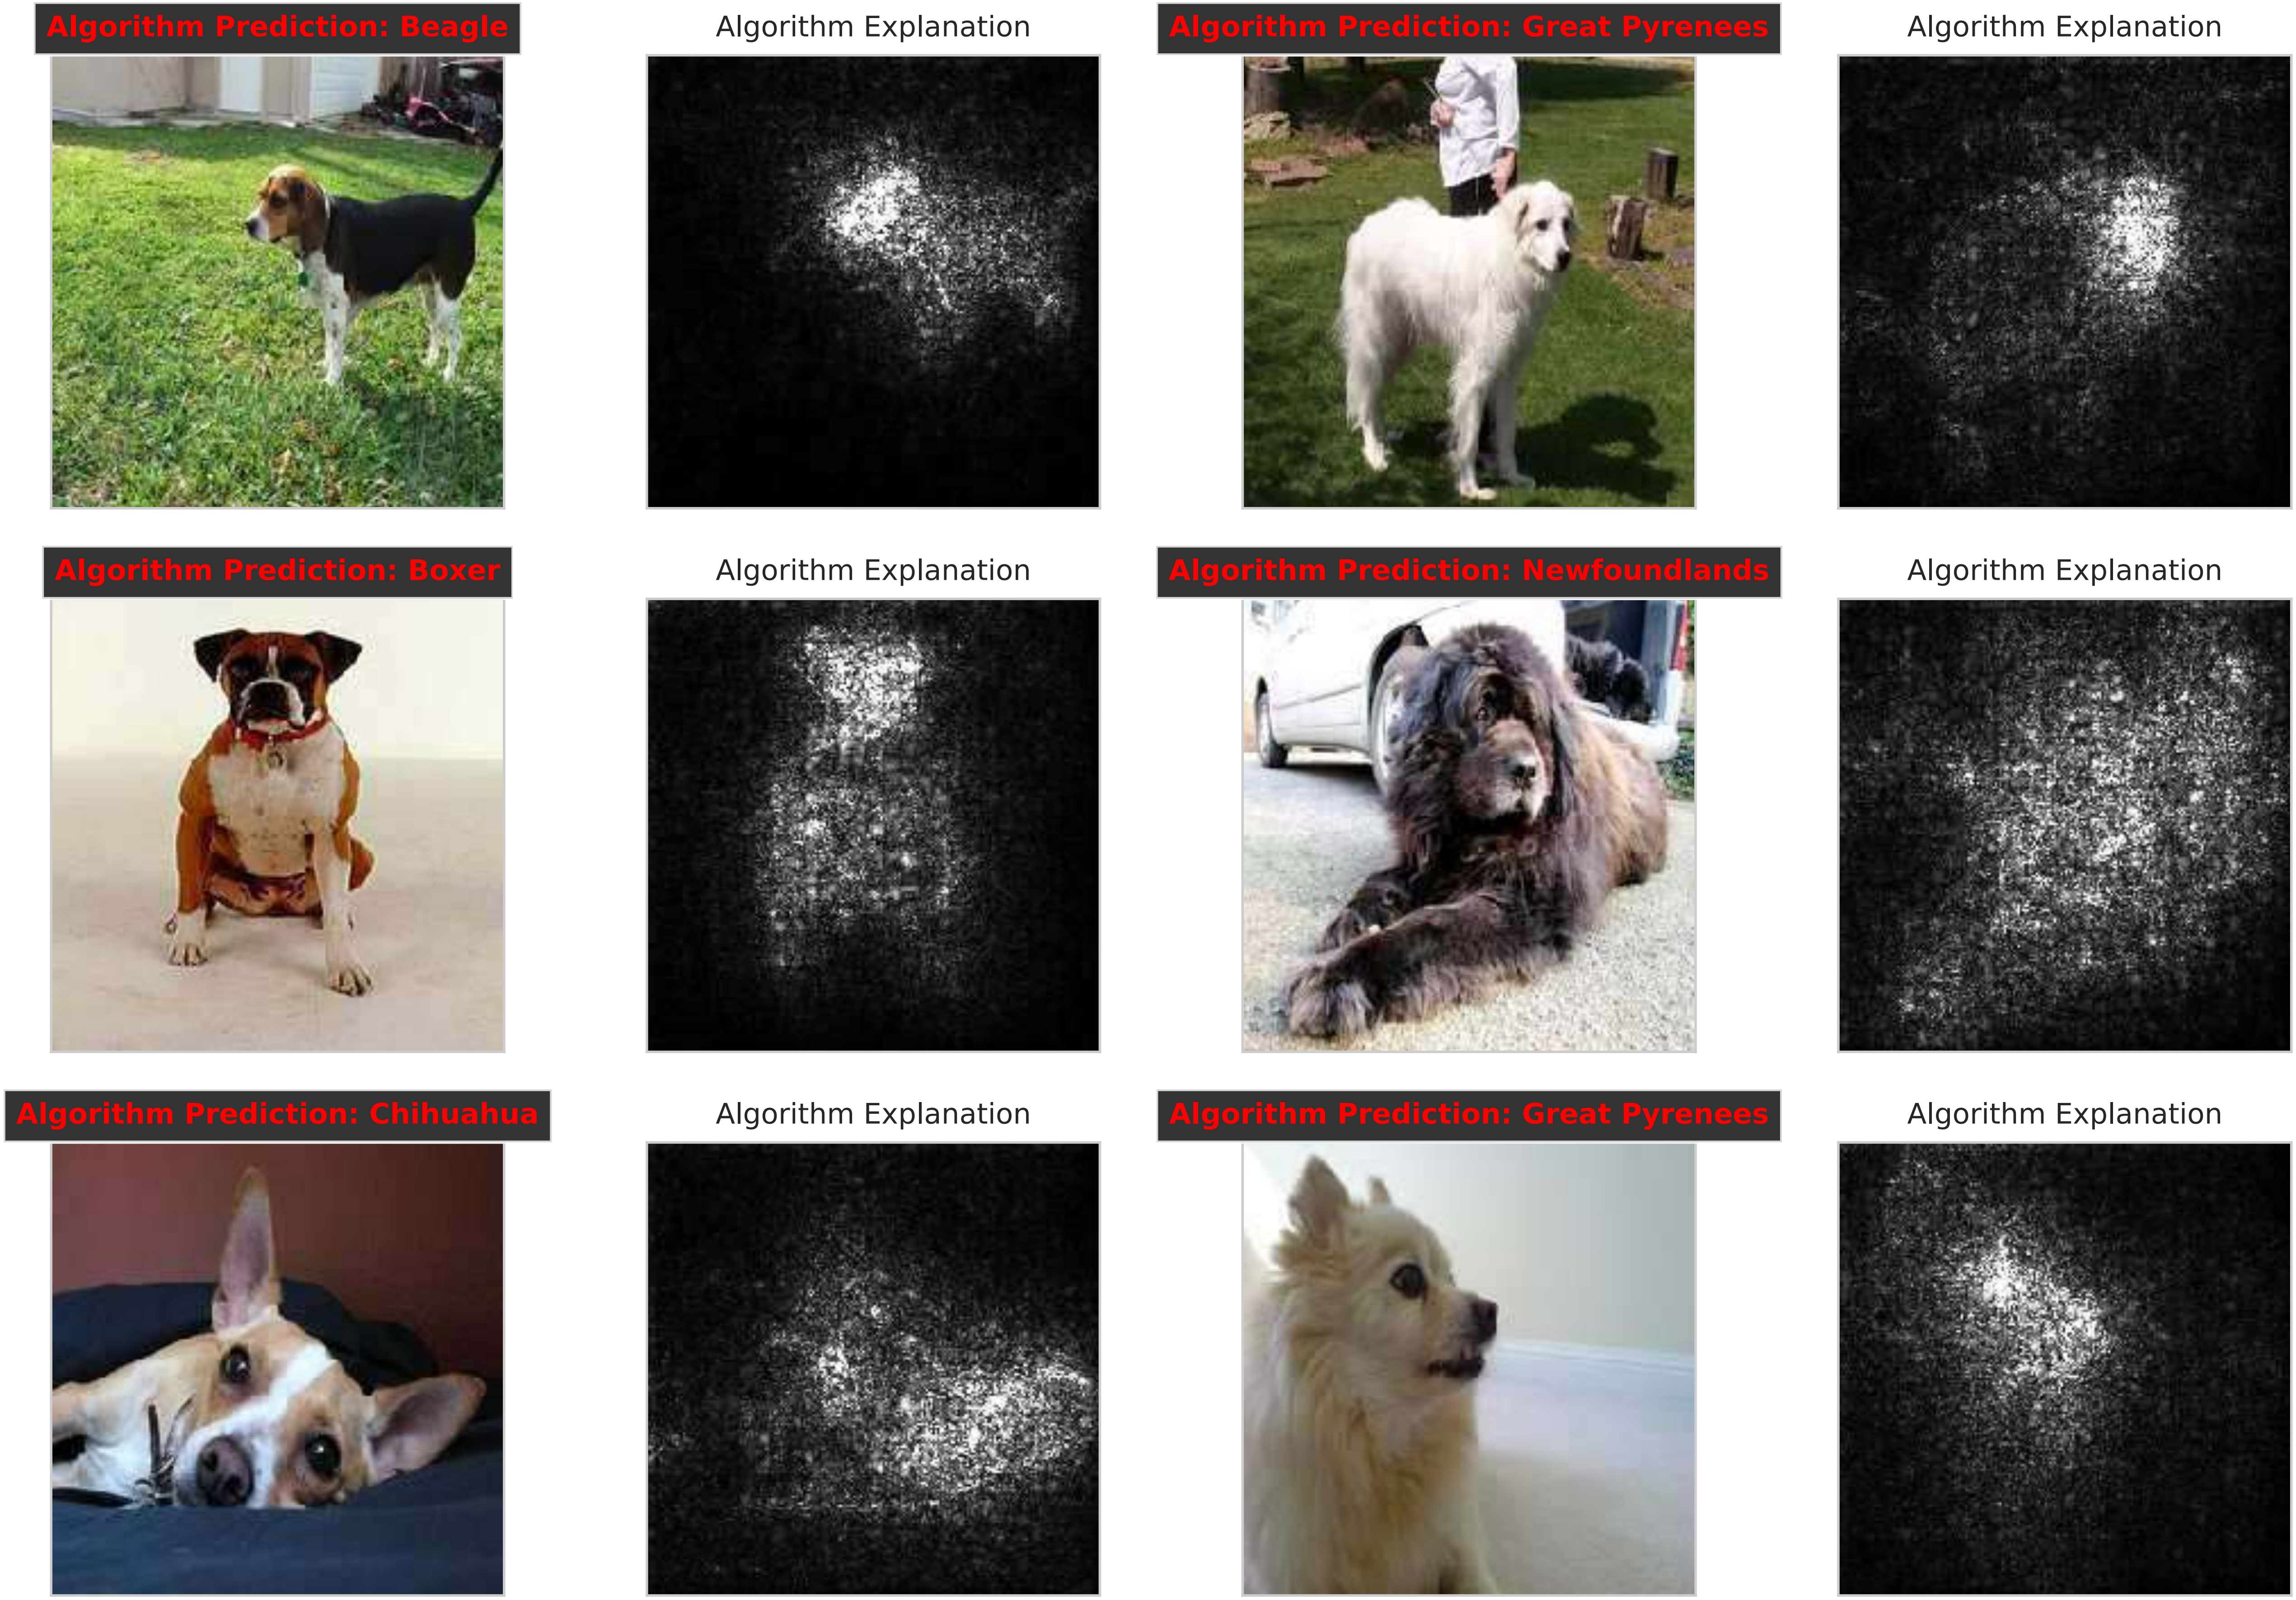

# Normal Model: Integrated Gradients

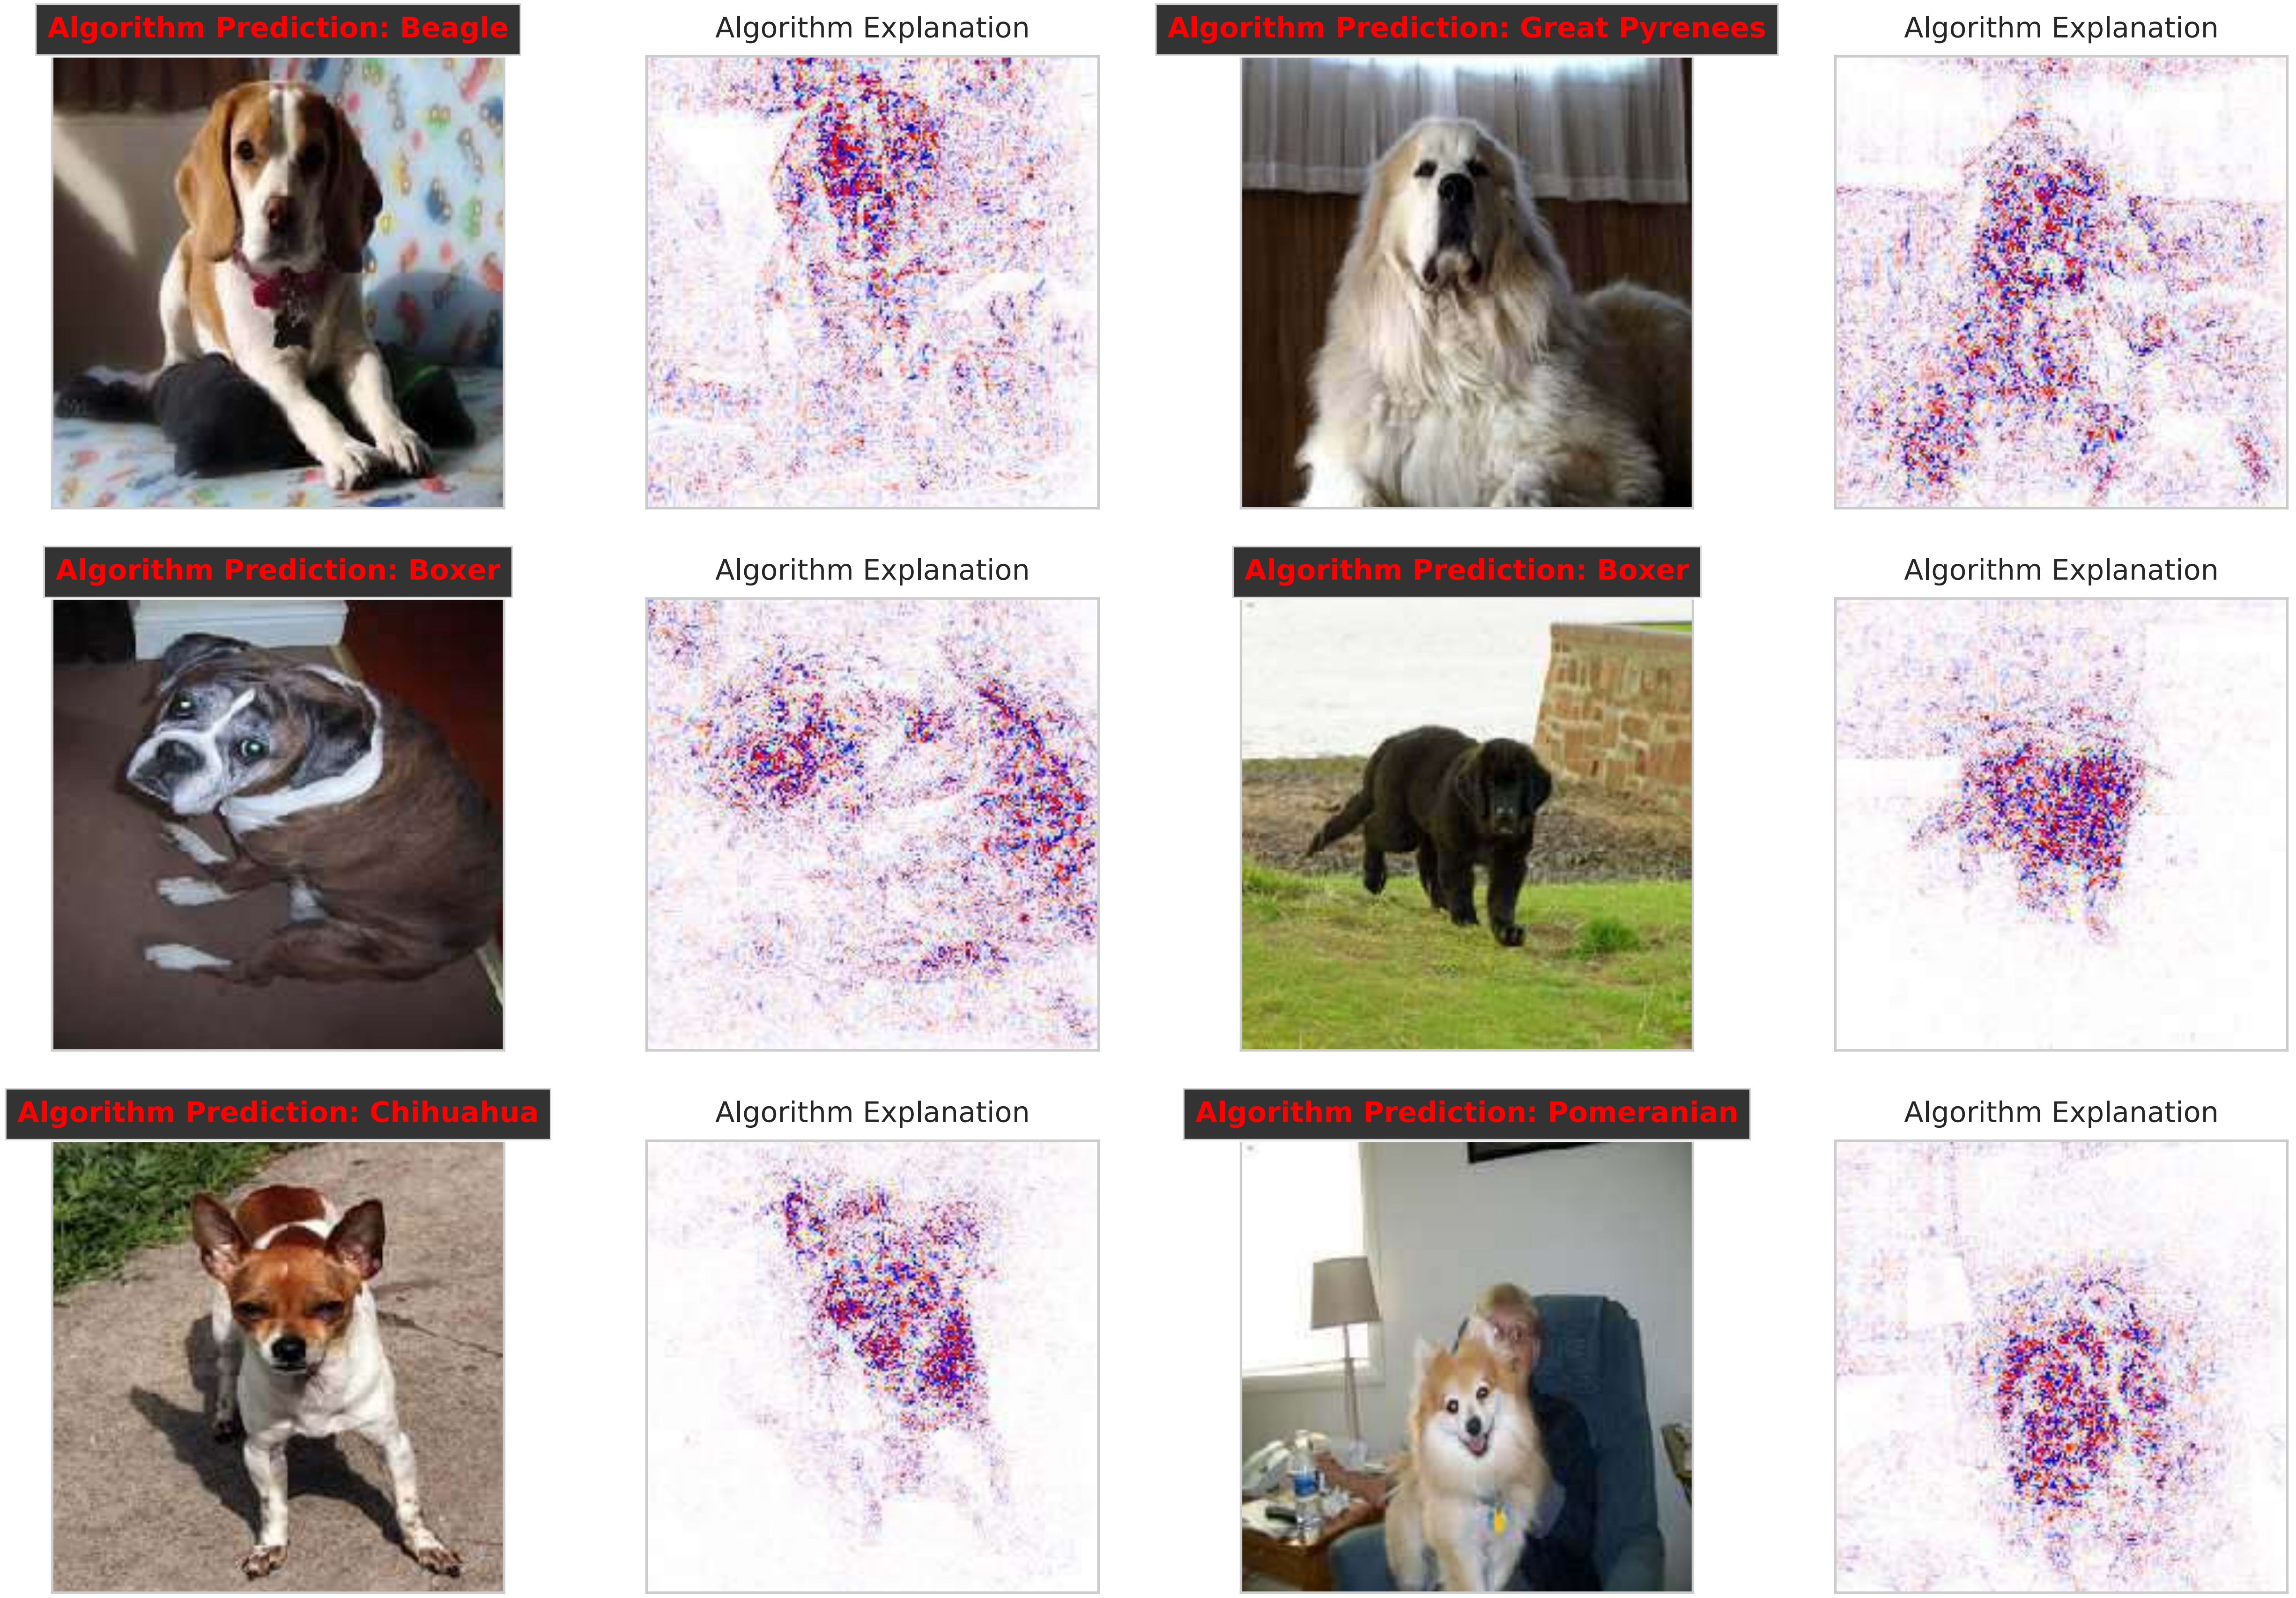

## Top Layer Random : Gradient

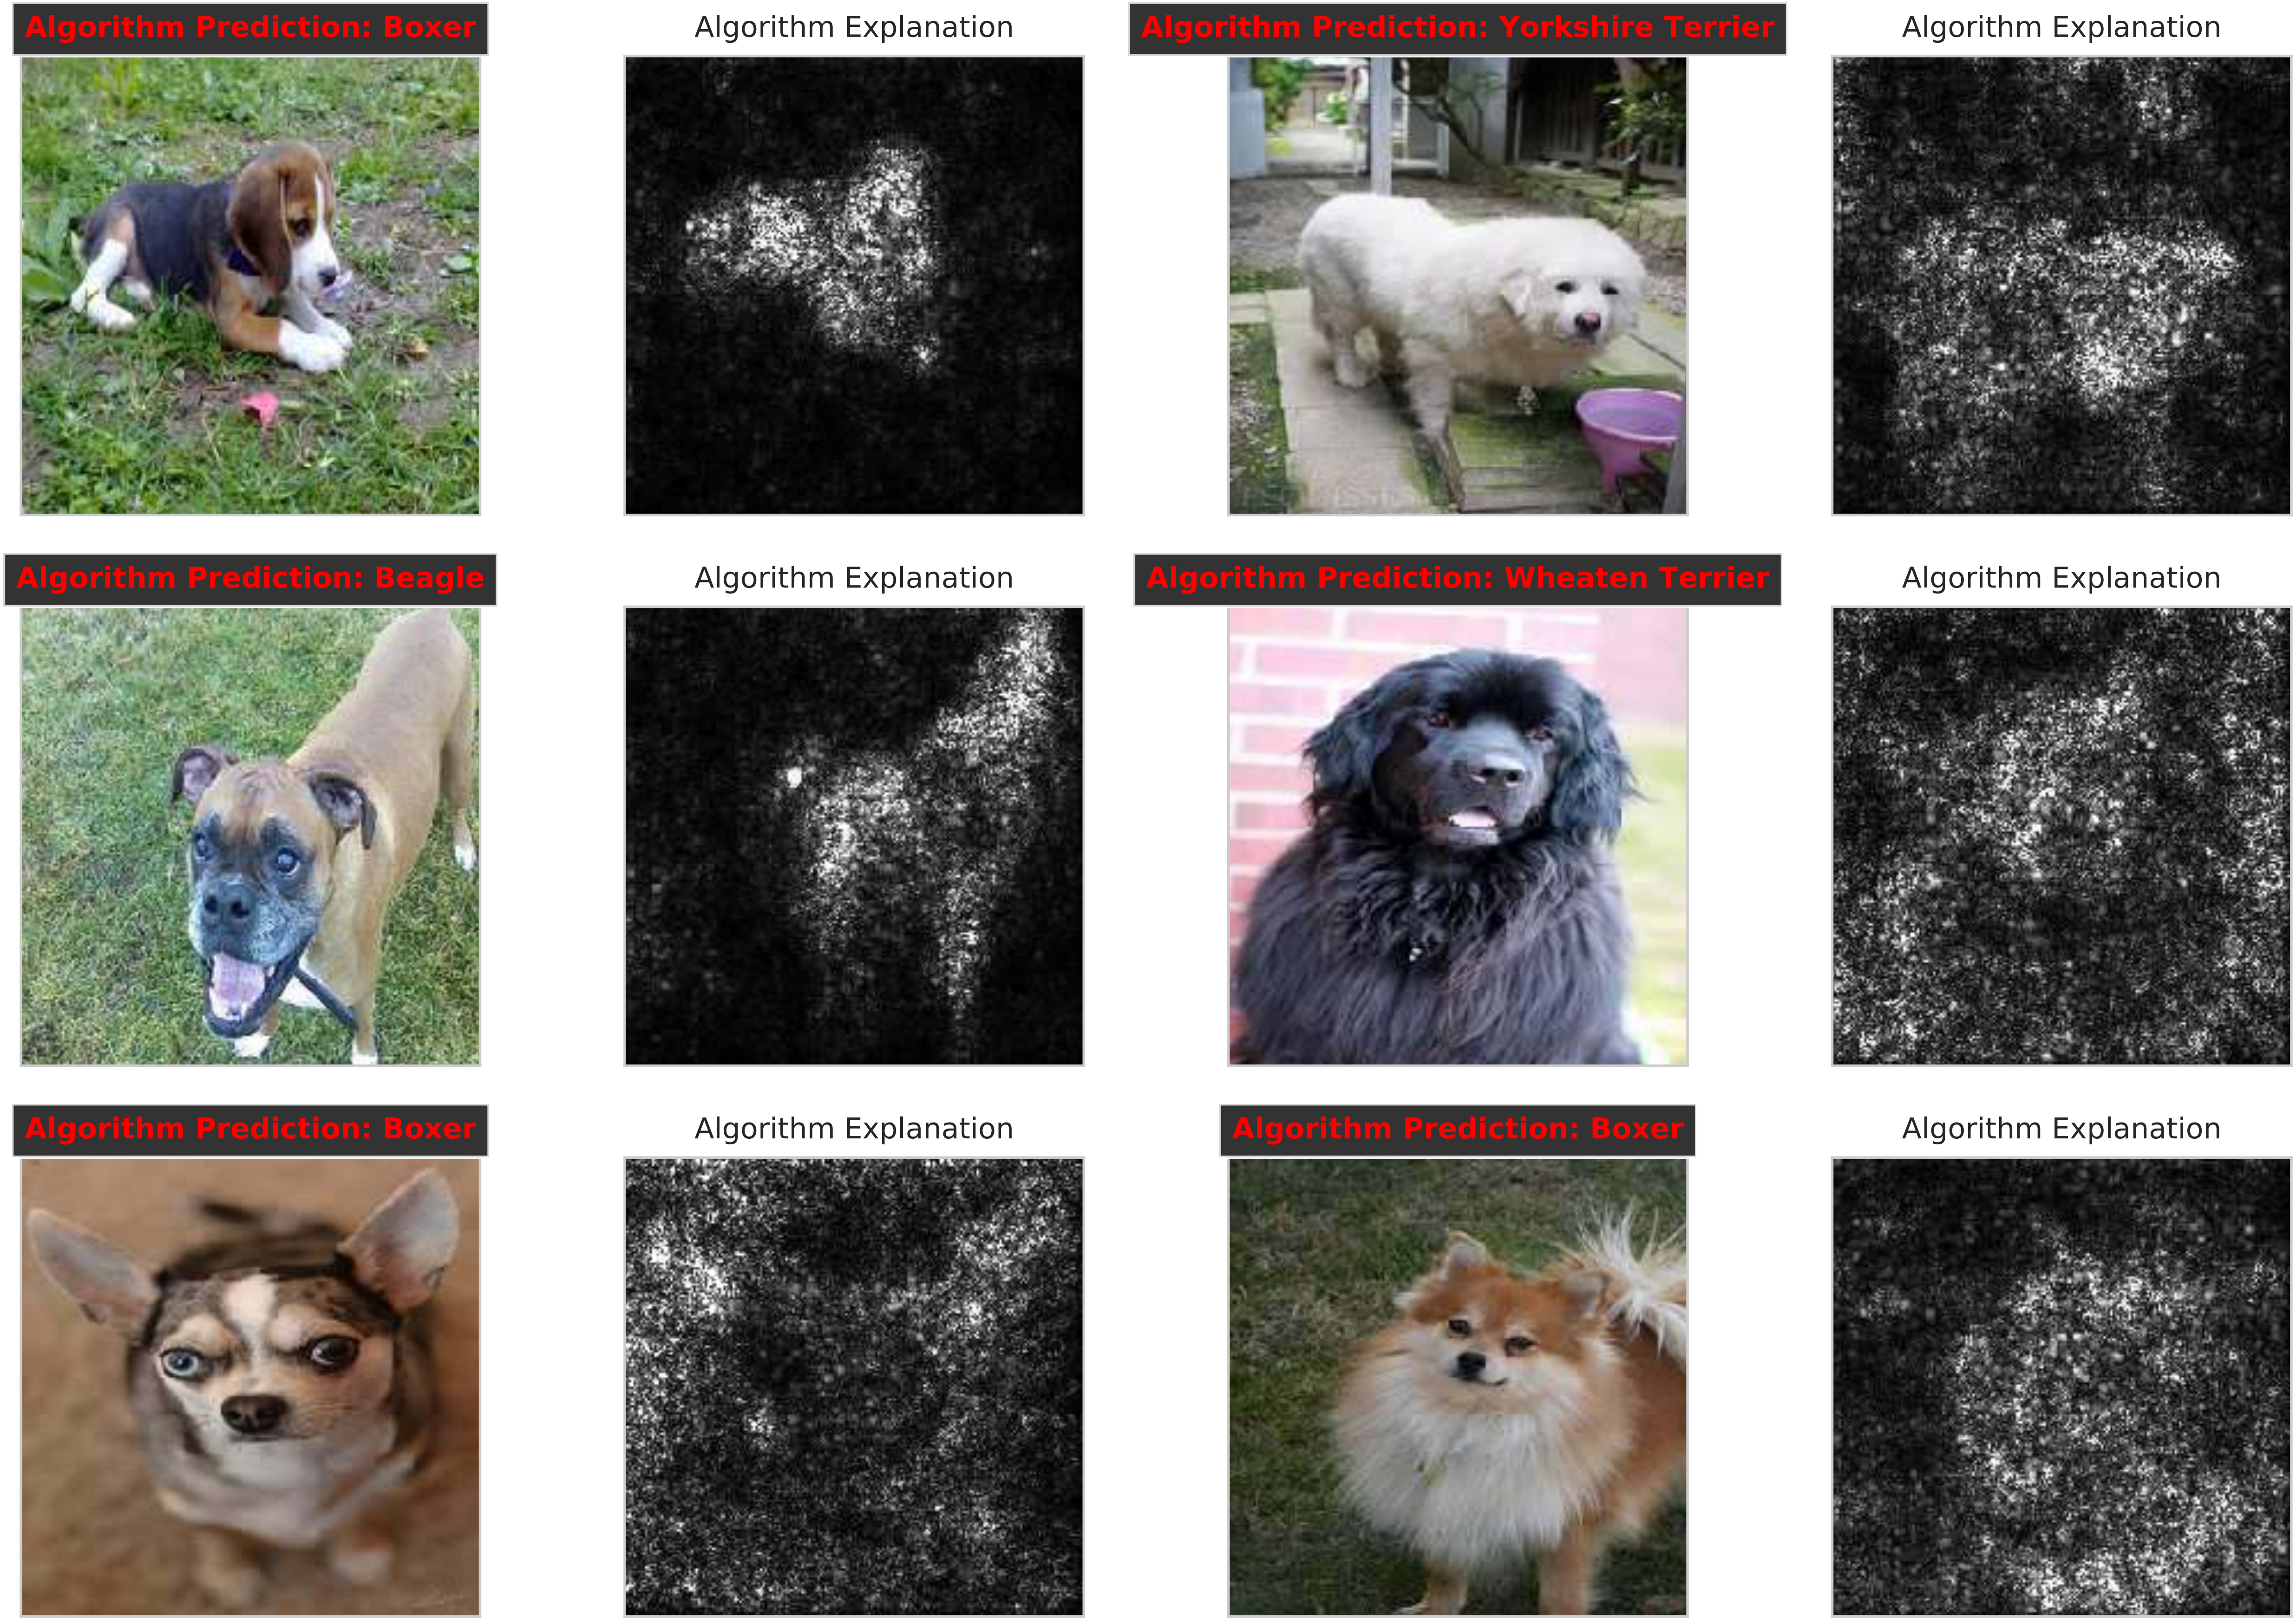

# Top Layer Model Random: SmoothGrad

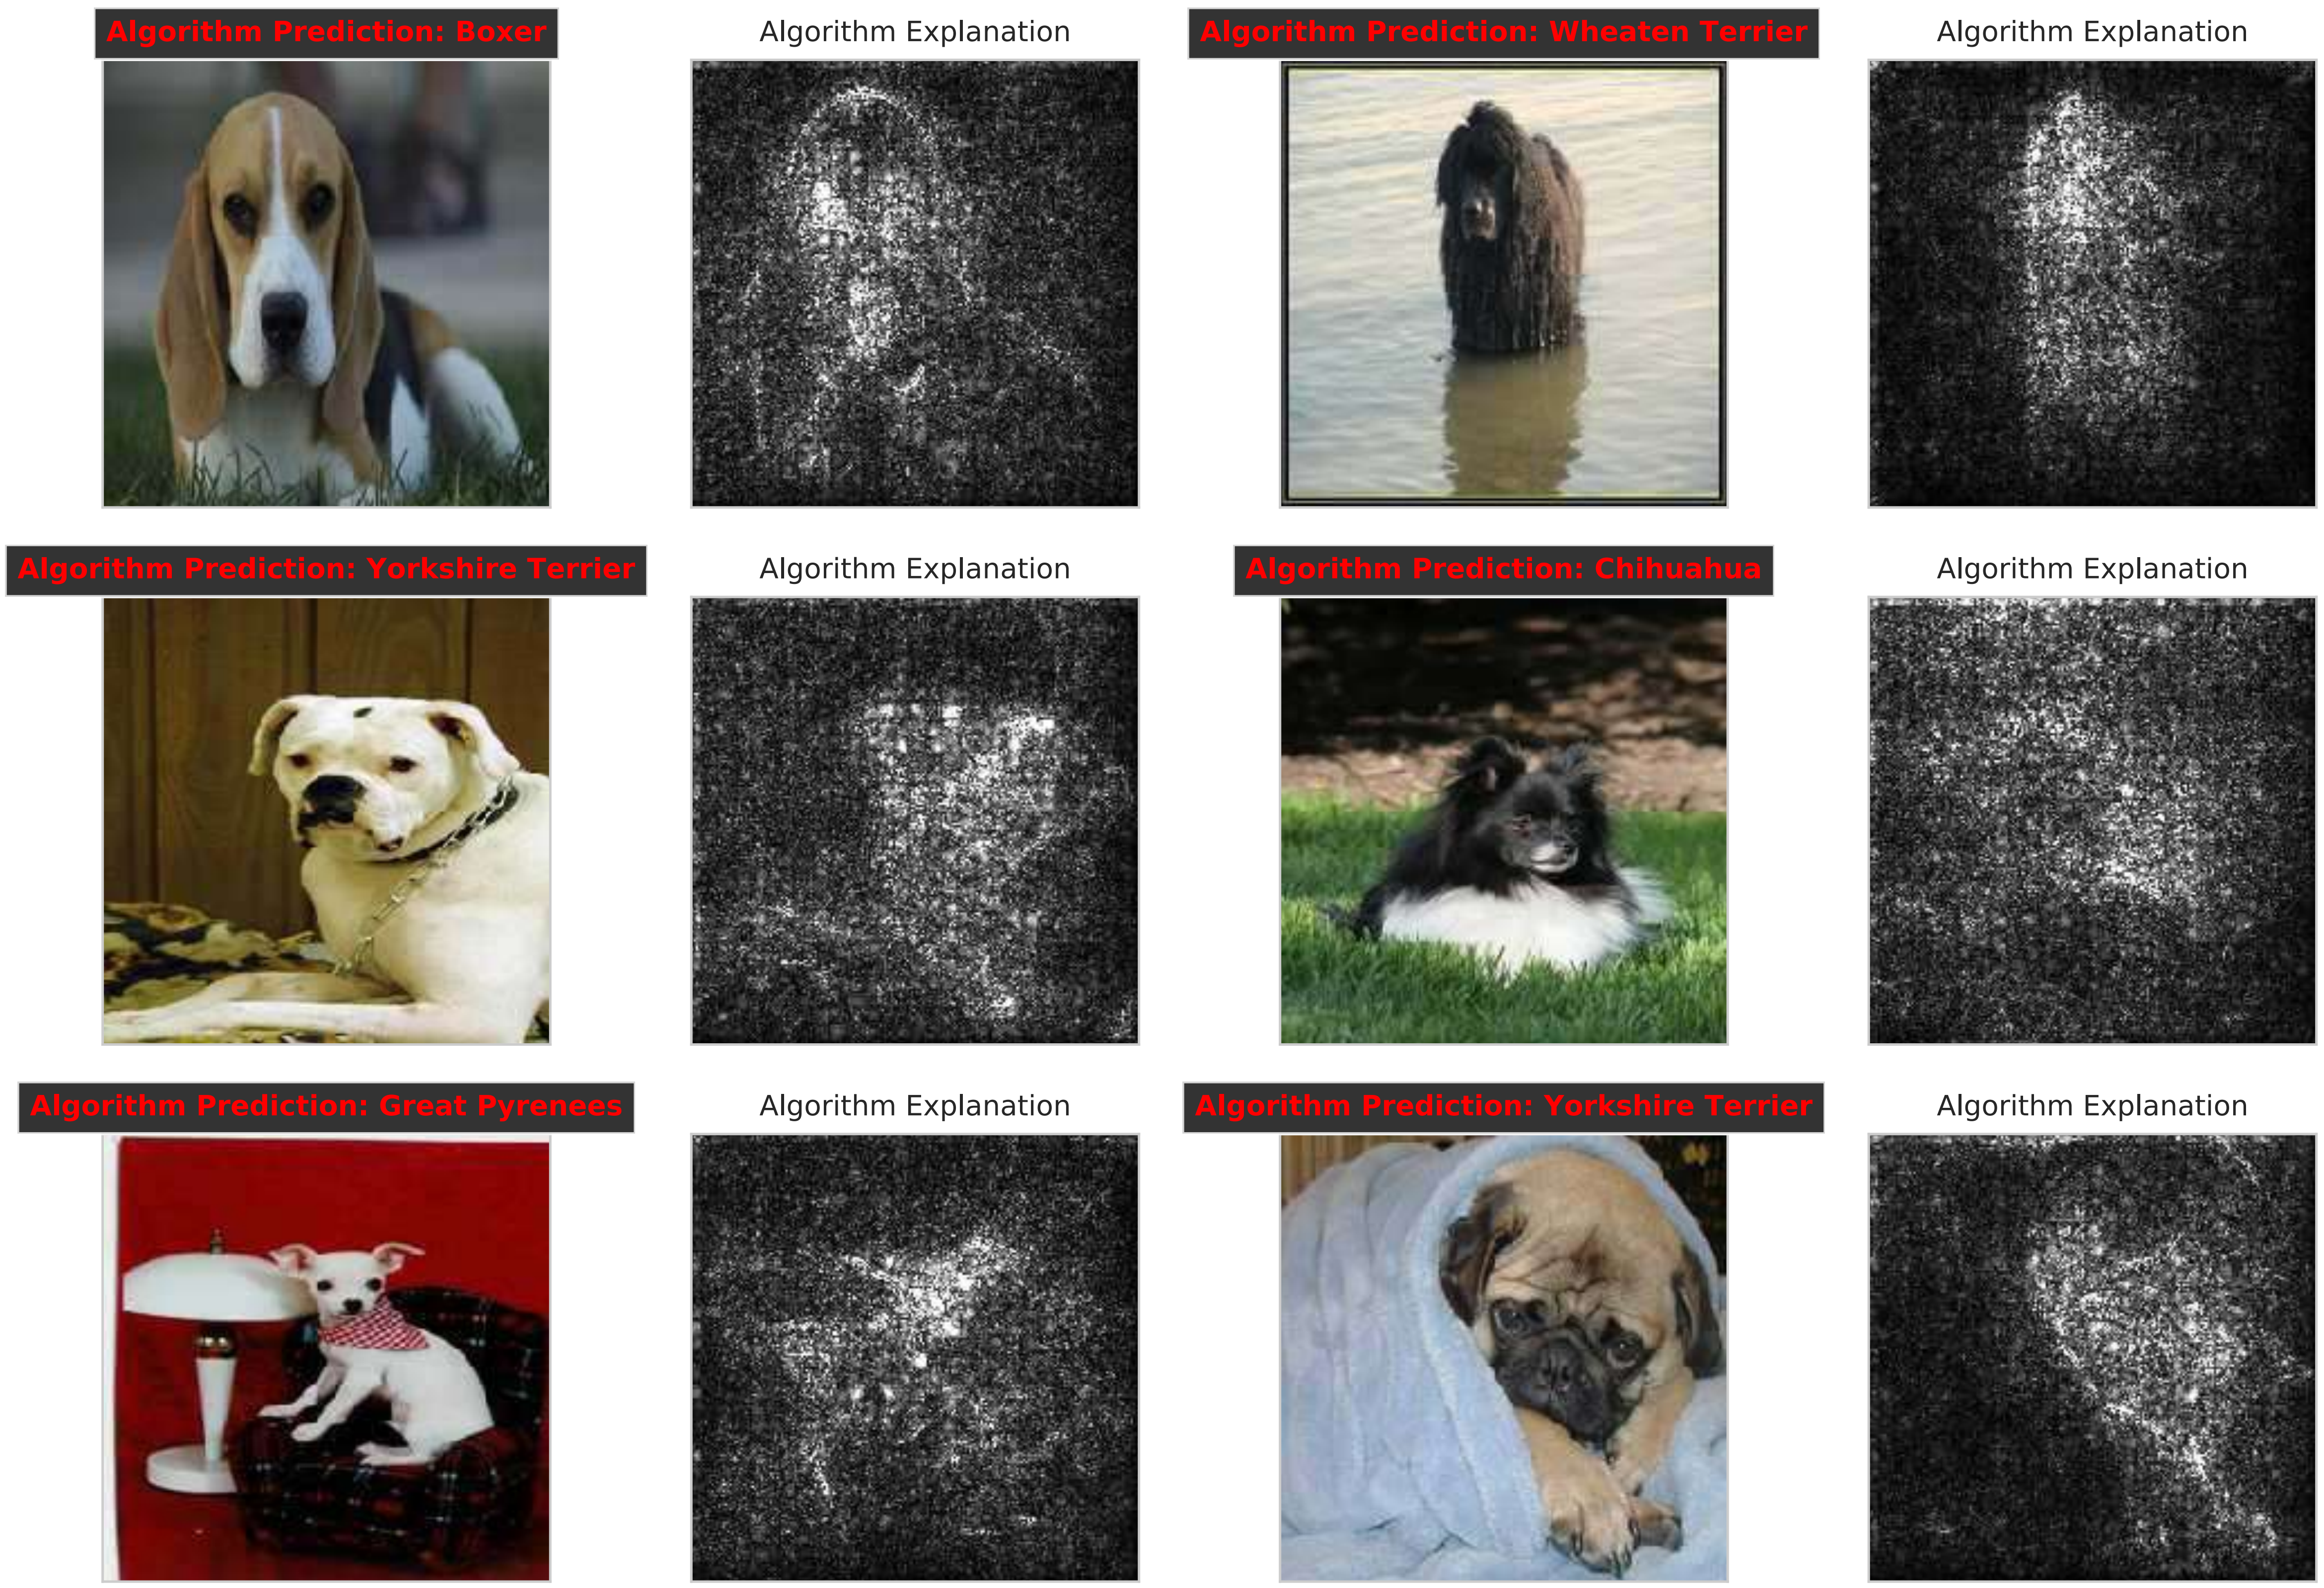

# Top Layer Random: Integrated Gradients

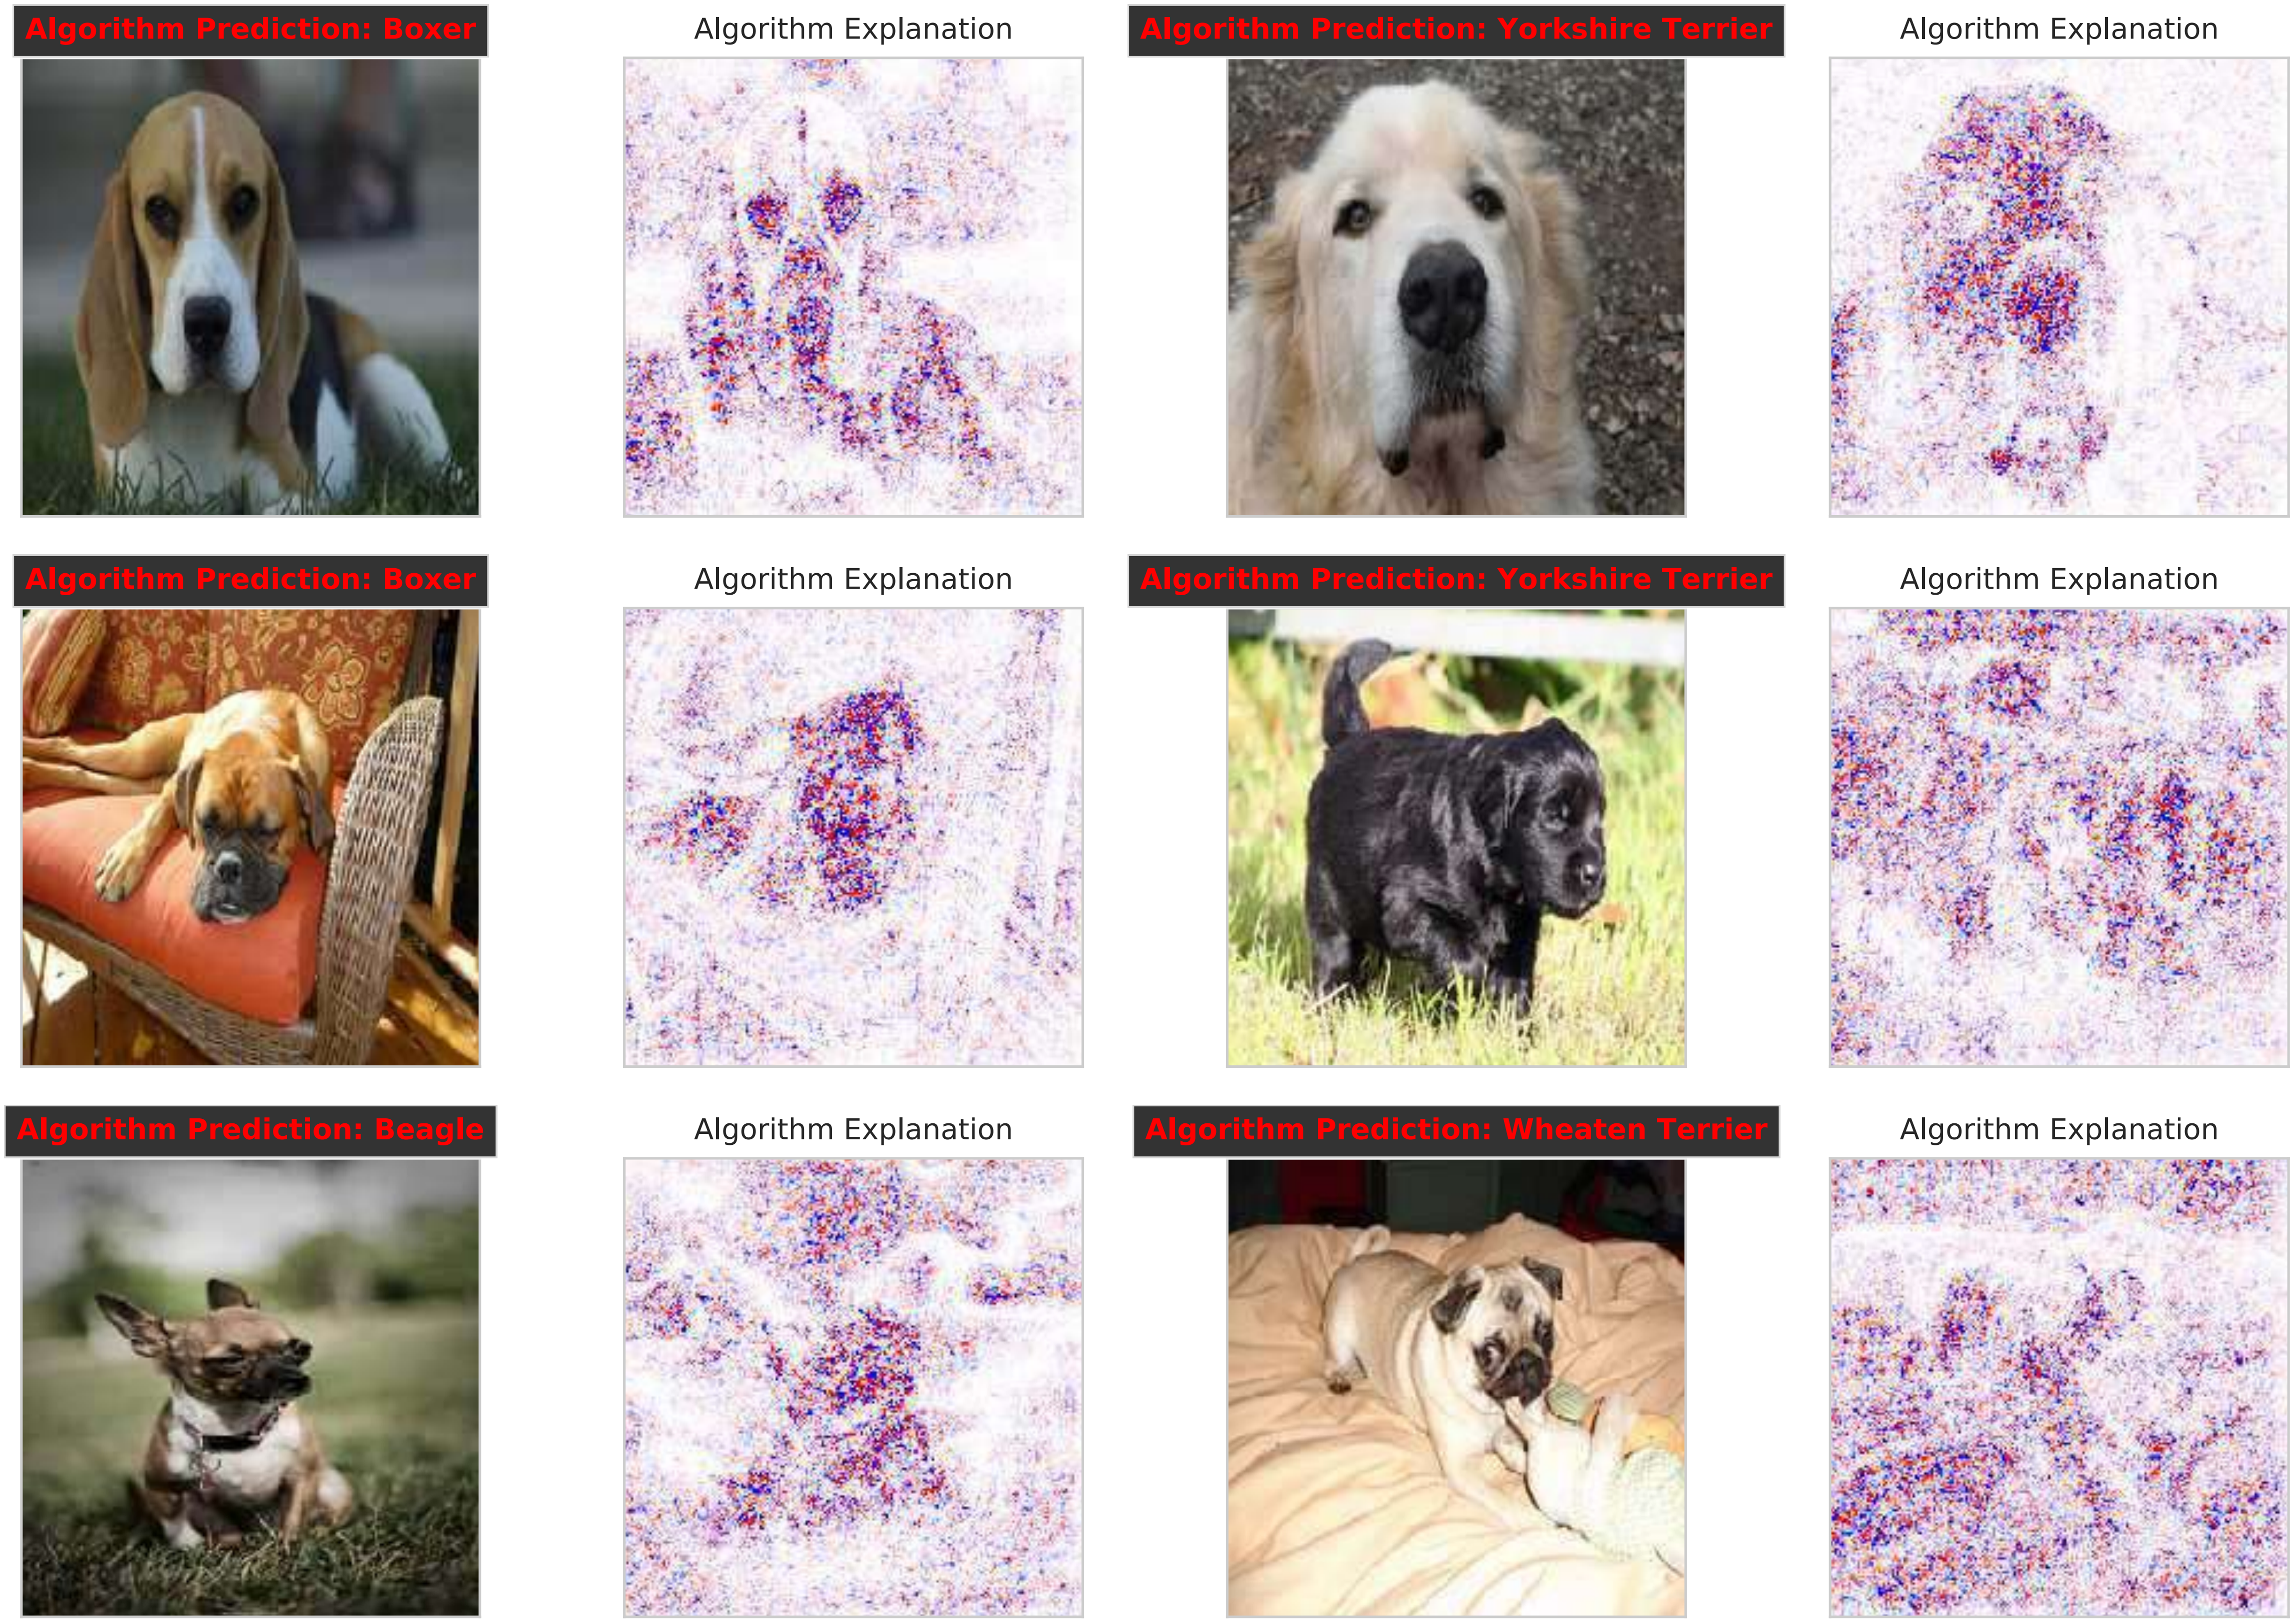

# Half-Way Random : Gradient

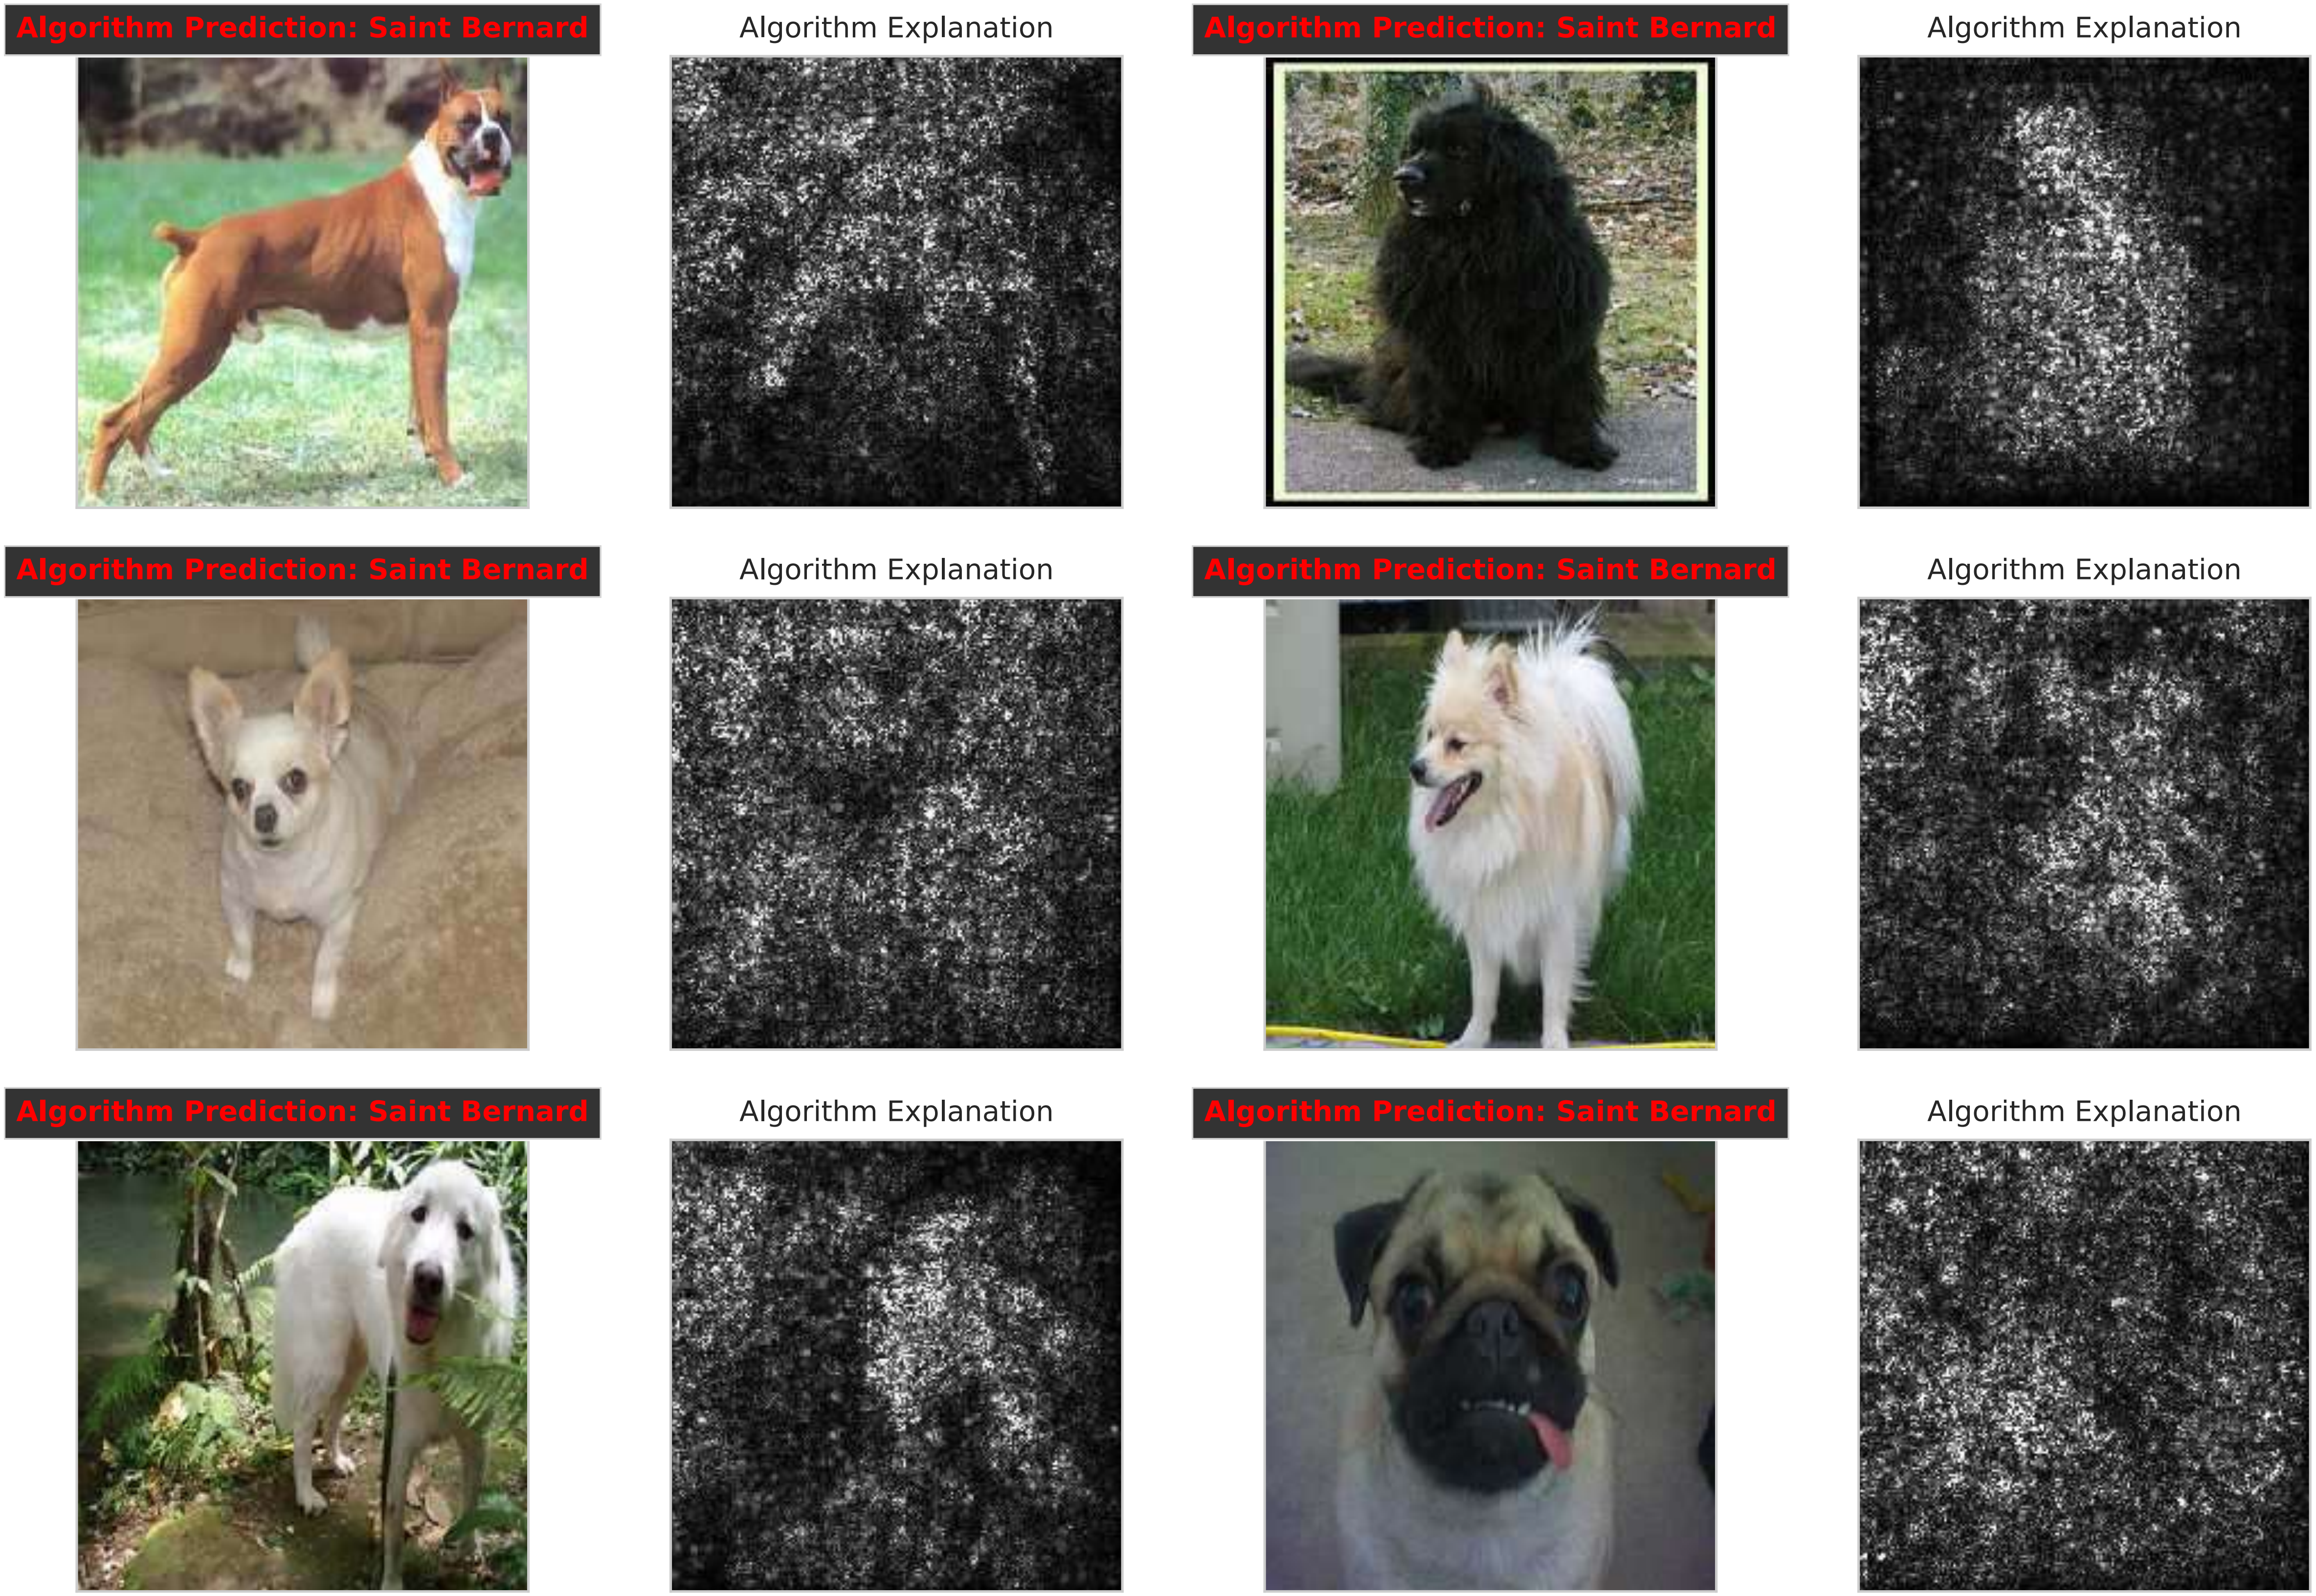

# Half-Way Model Random: SmoothGrad

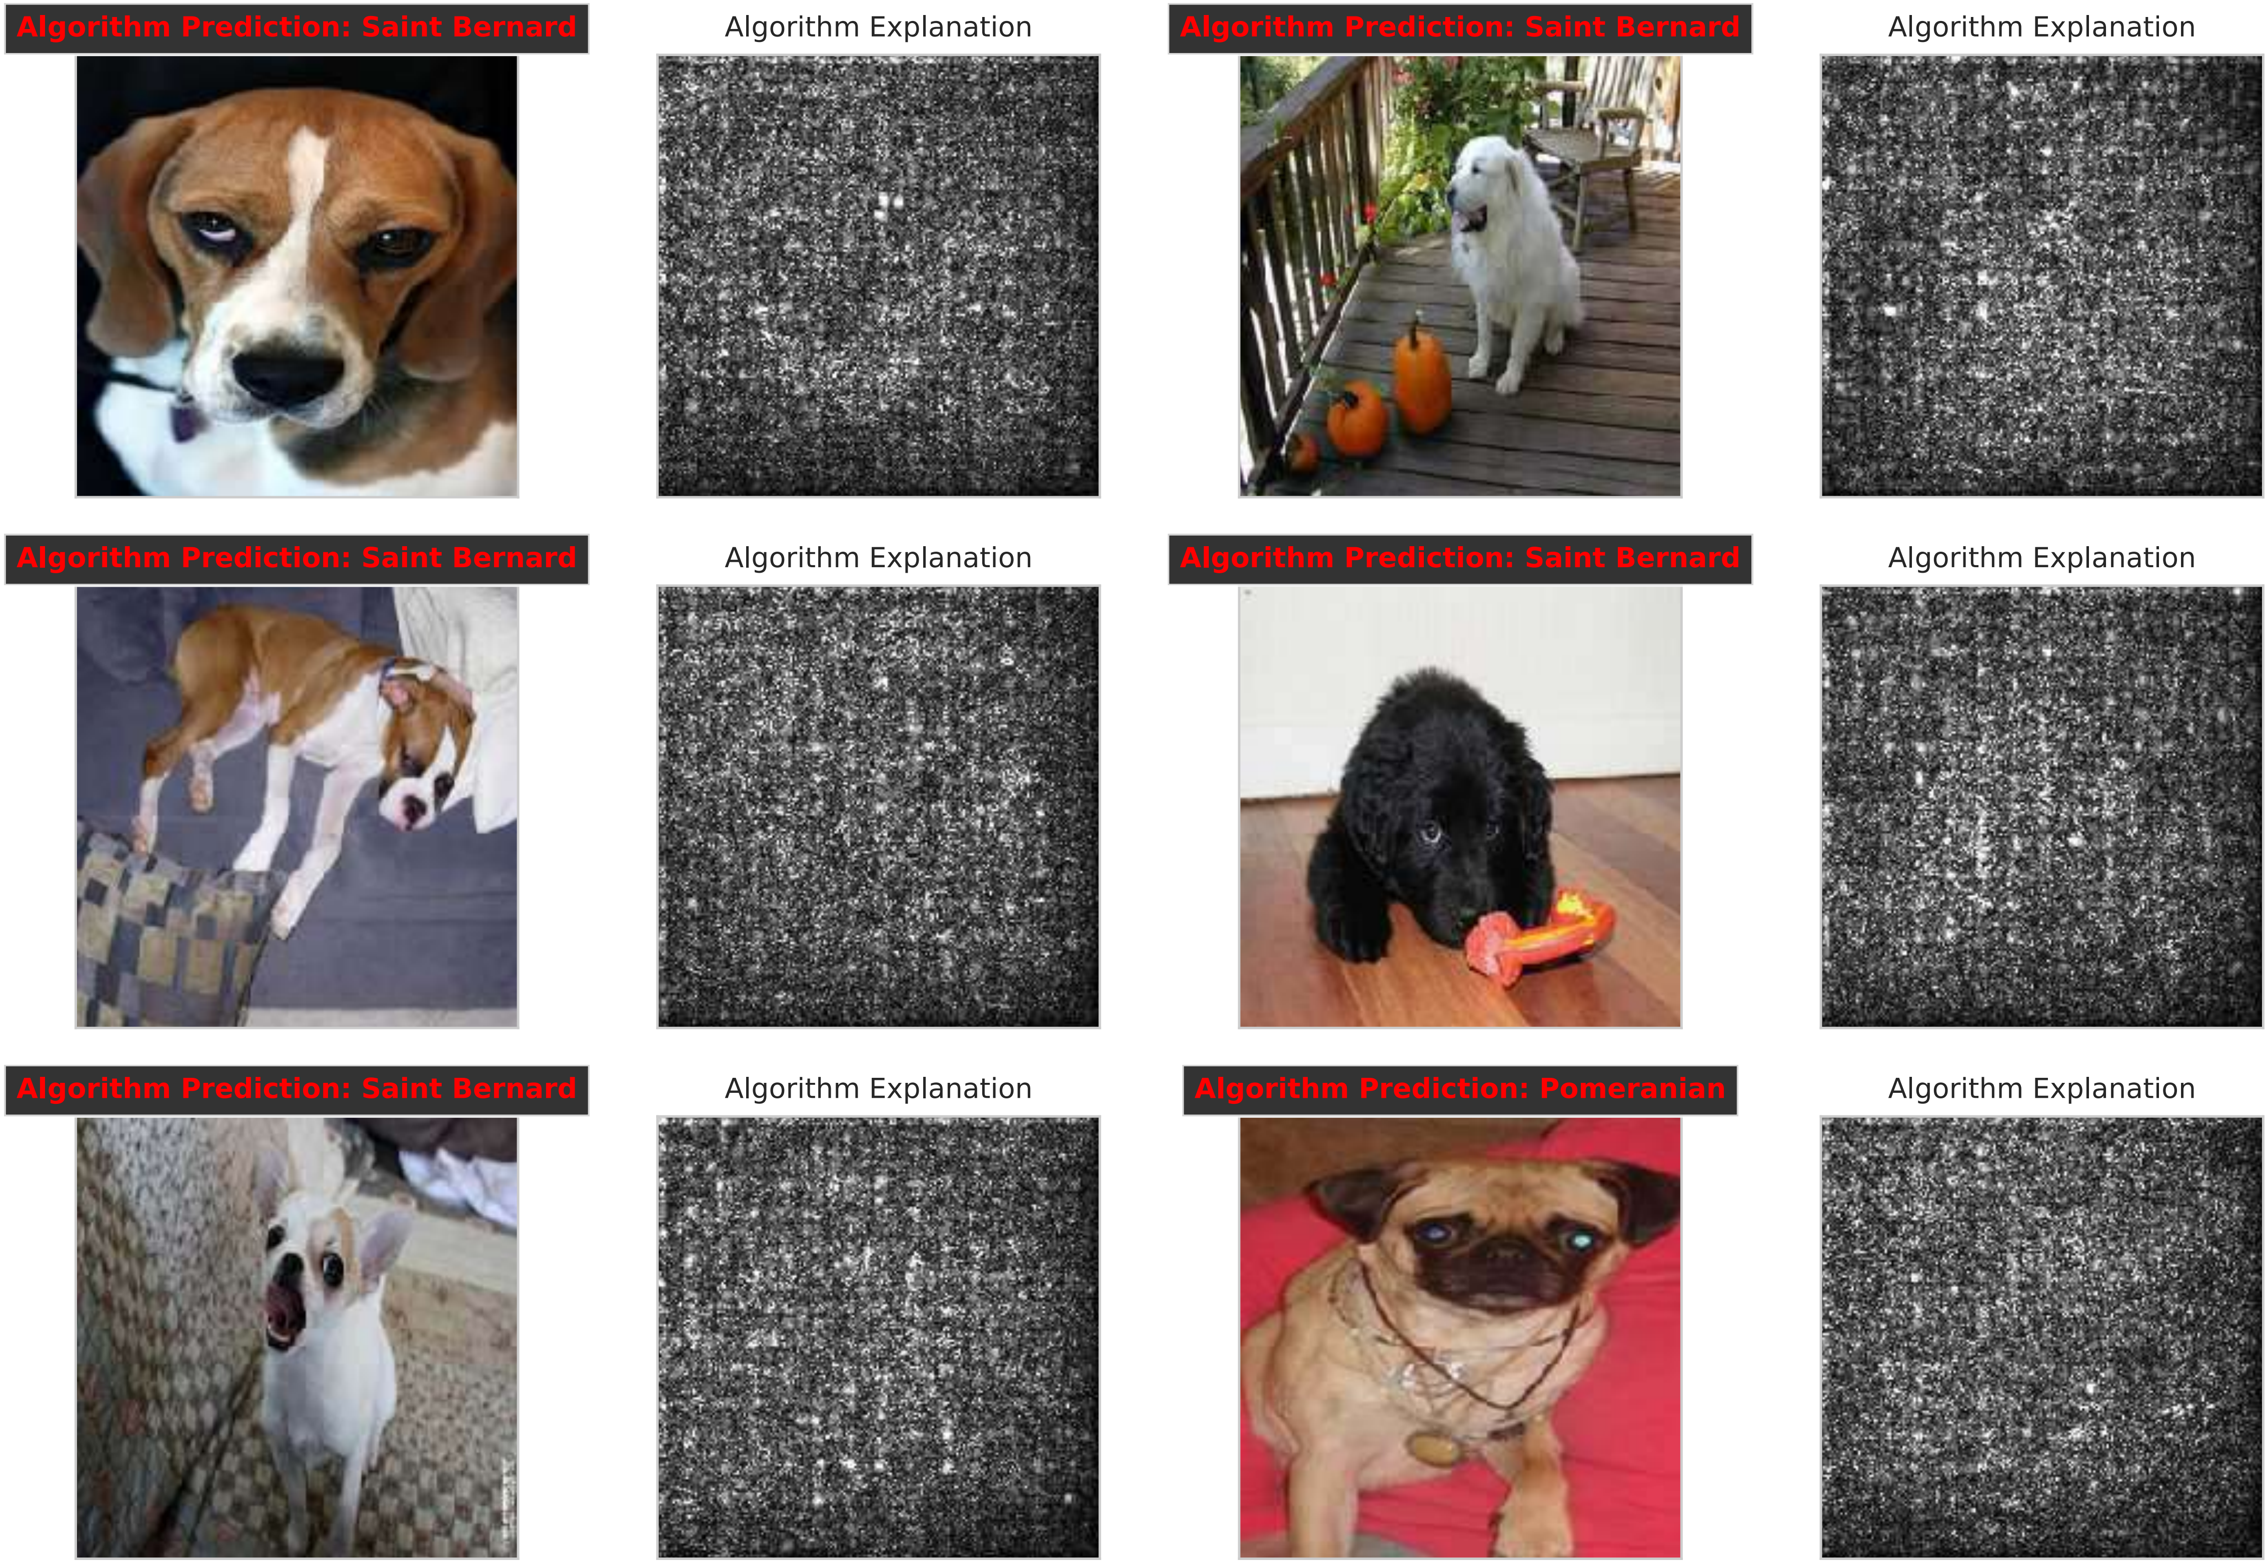

# Half-Way Random: Integrated Gradients

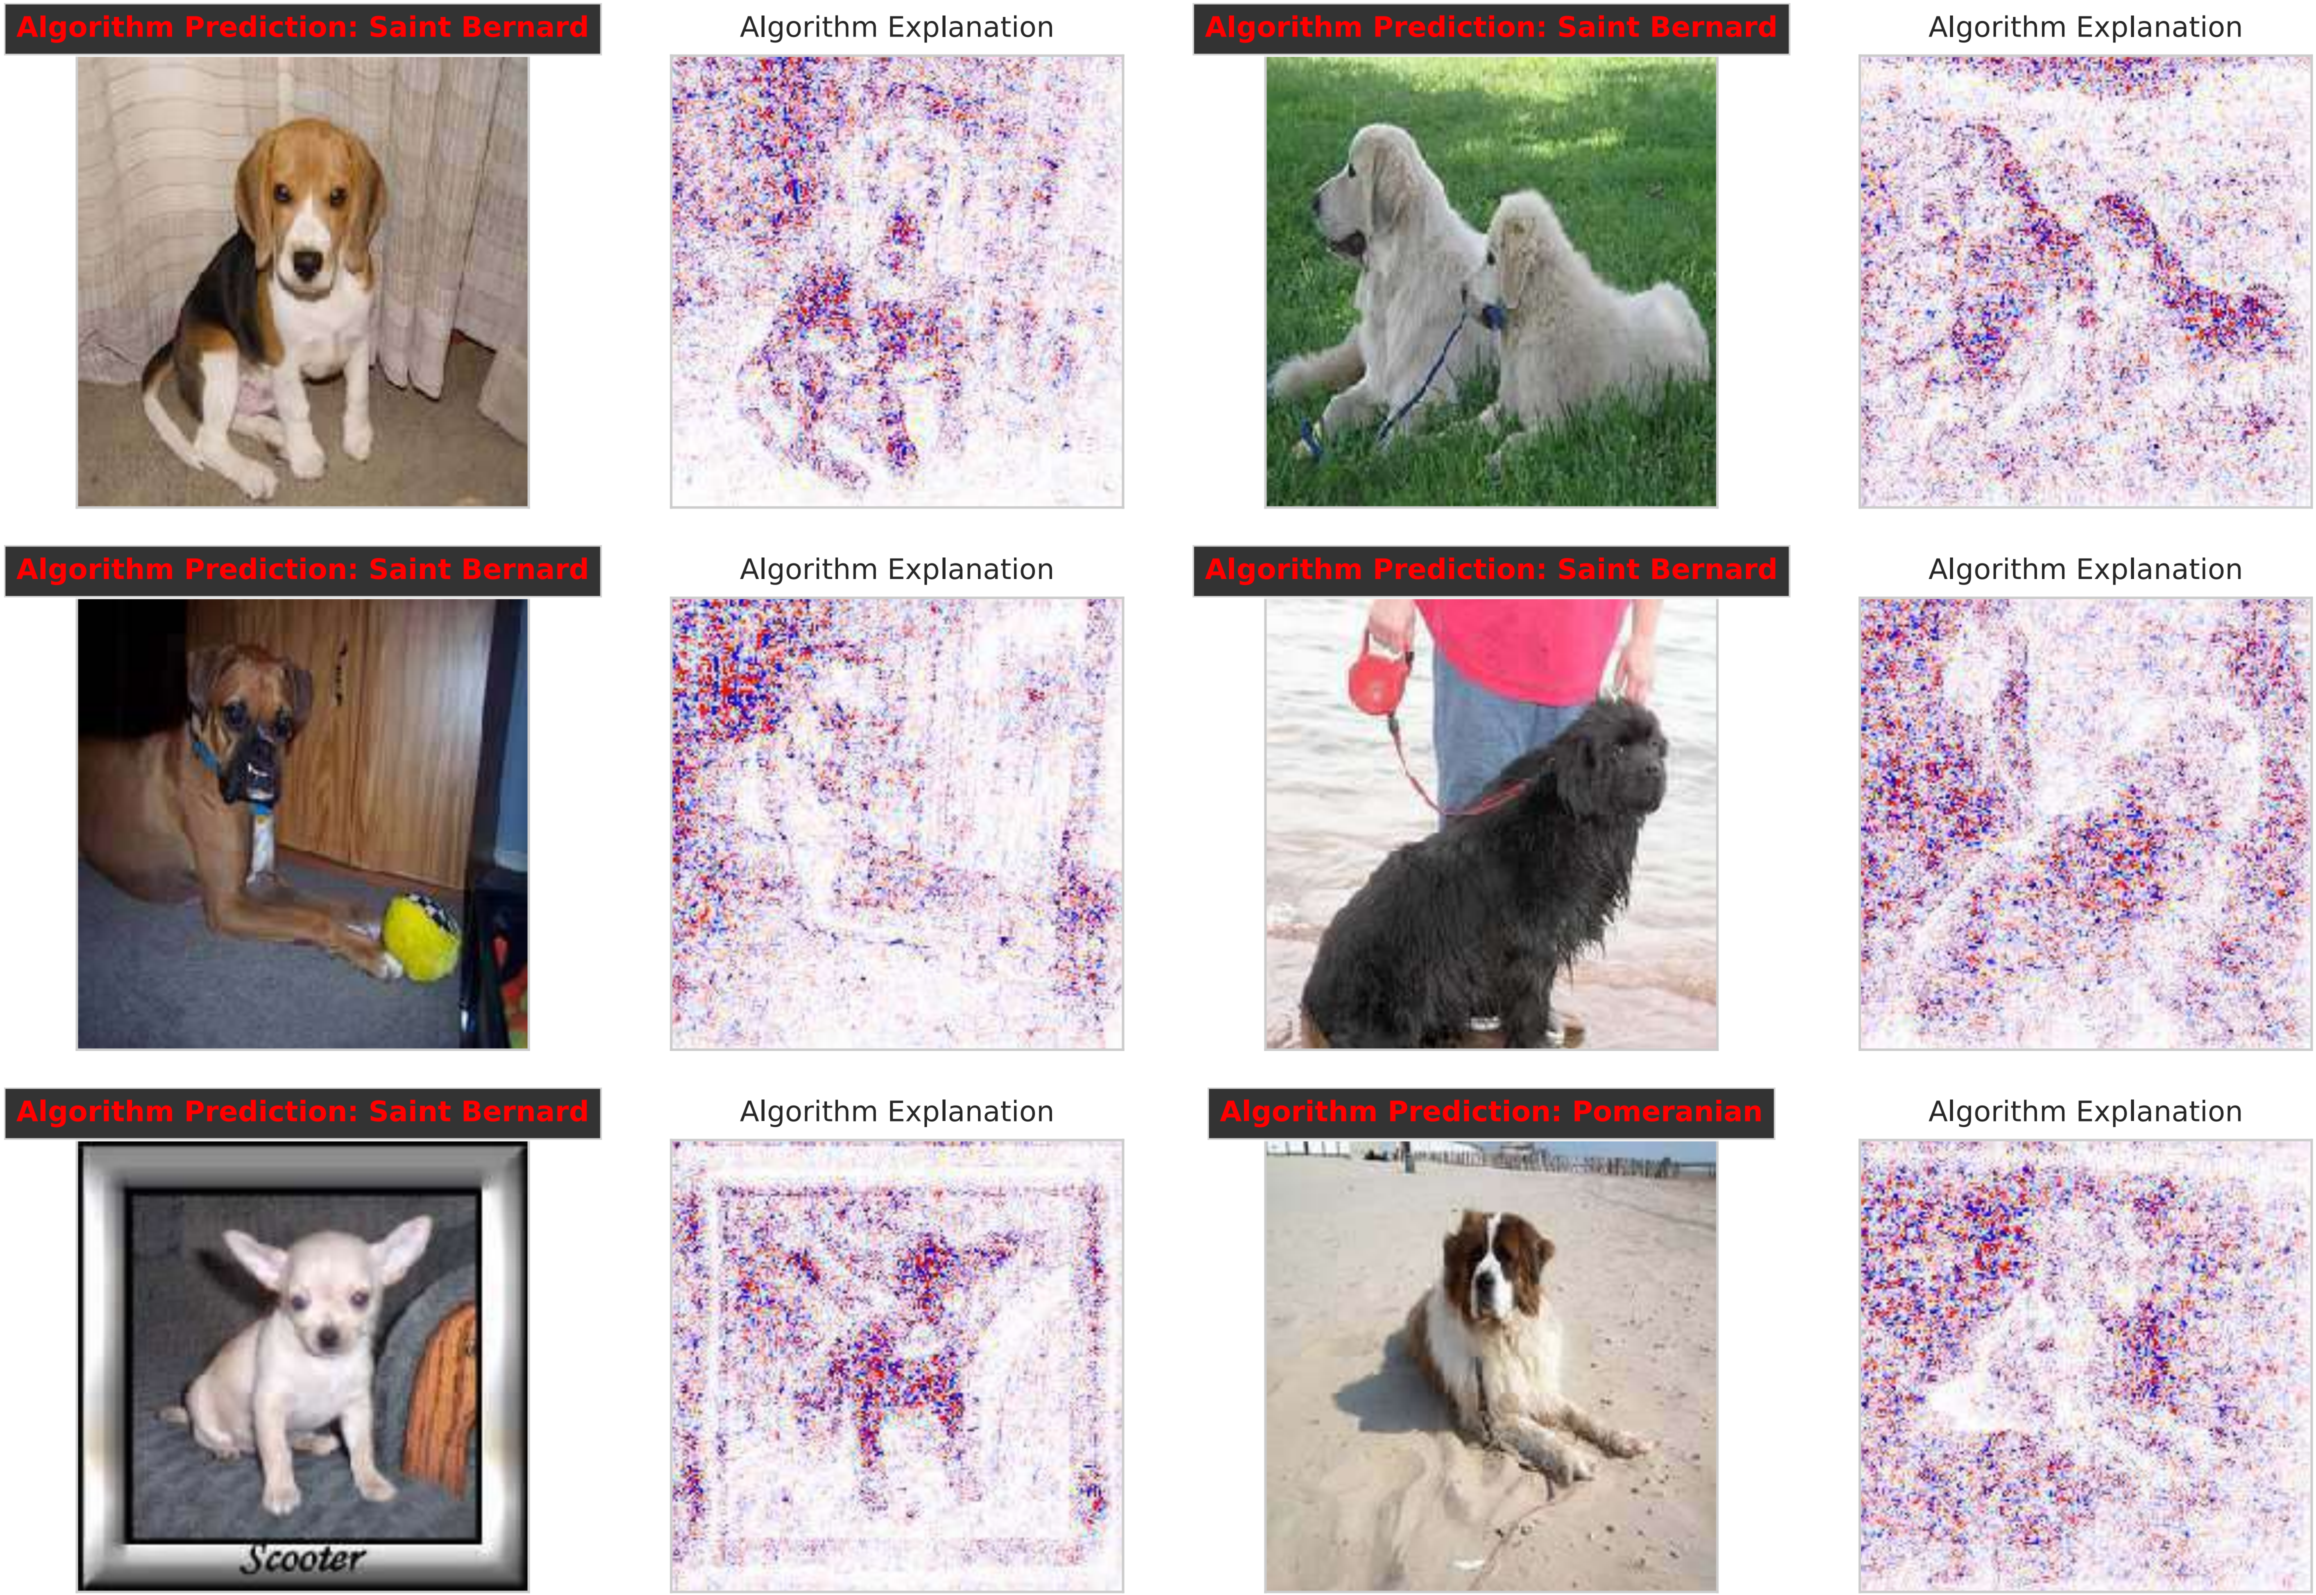

## Random Labels : Gradient

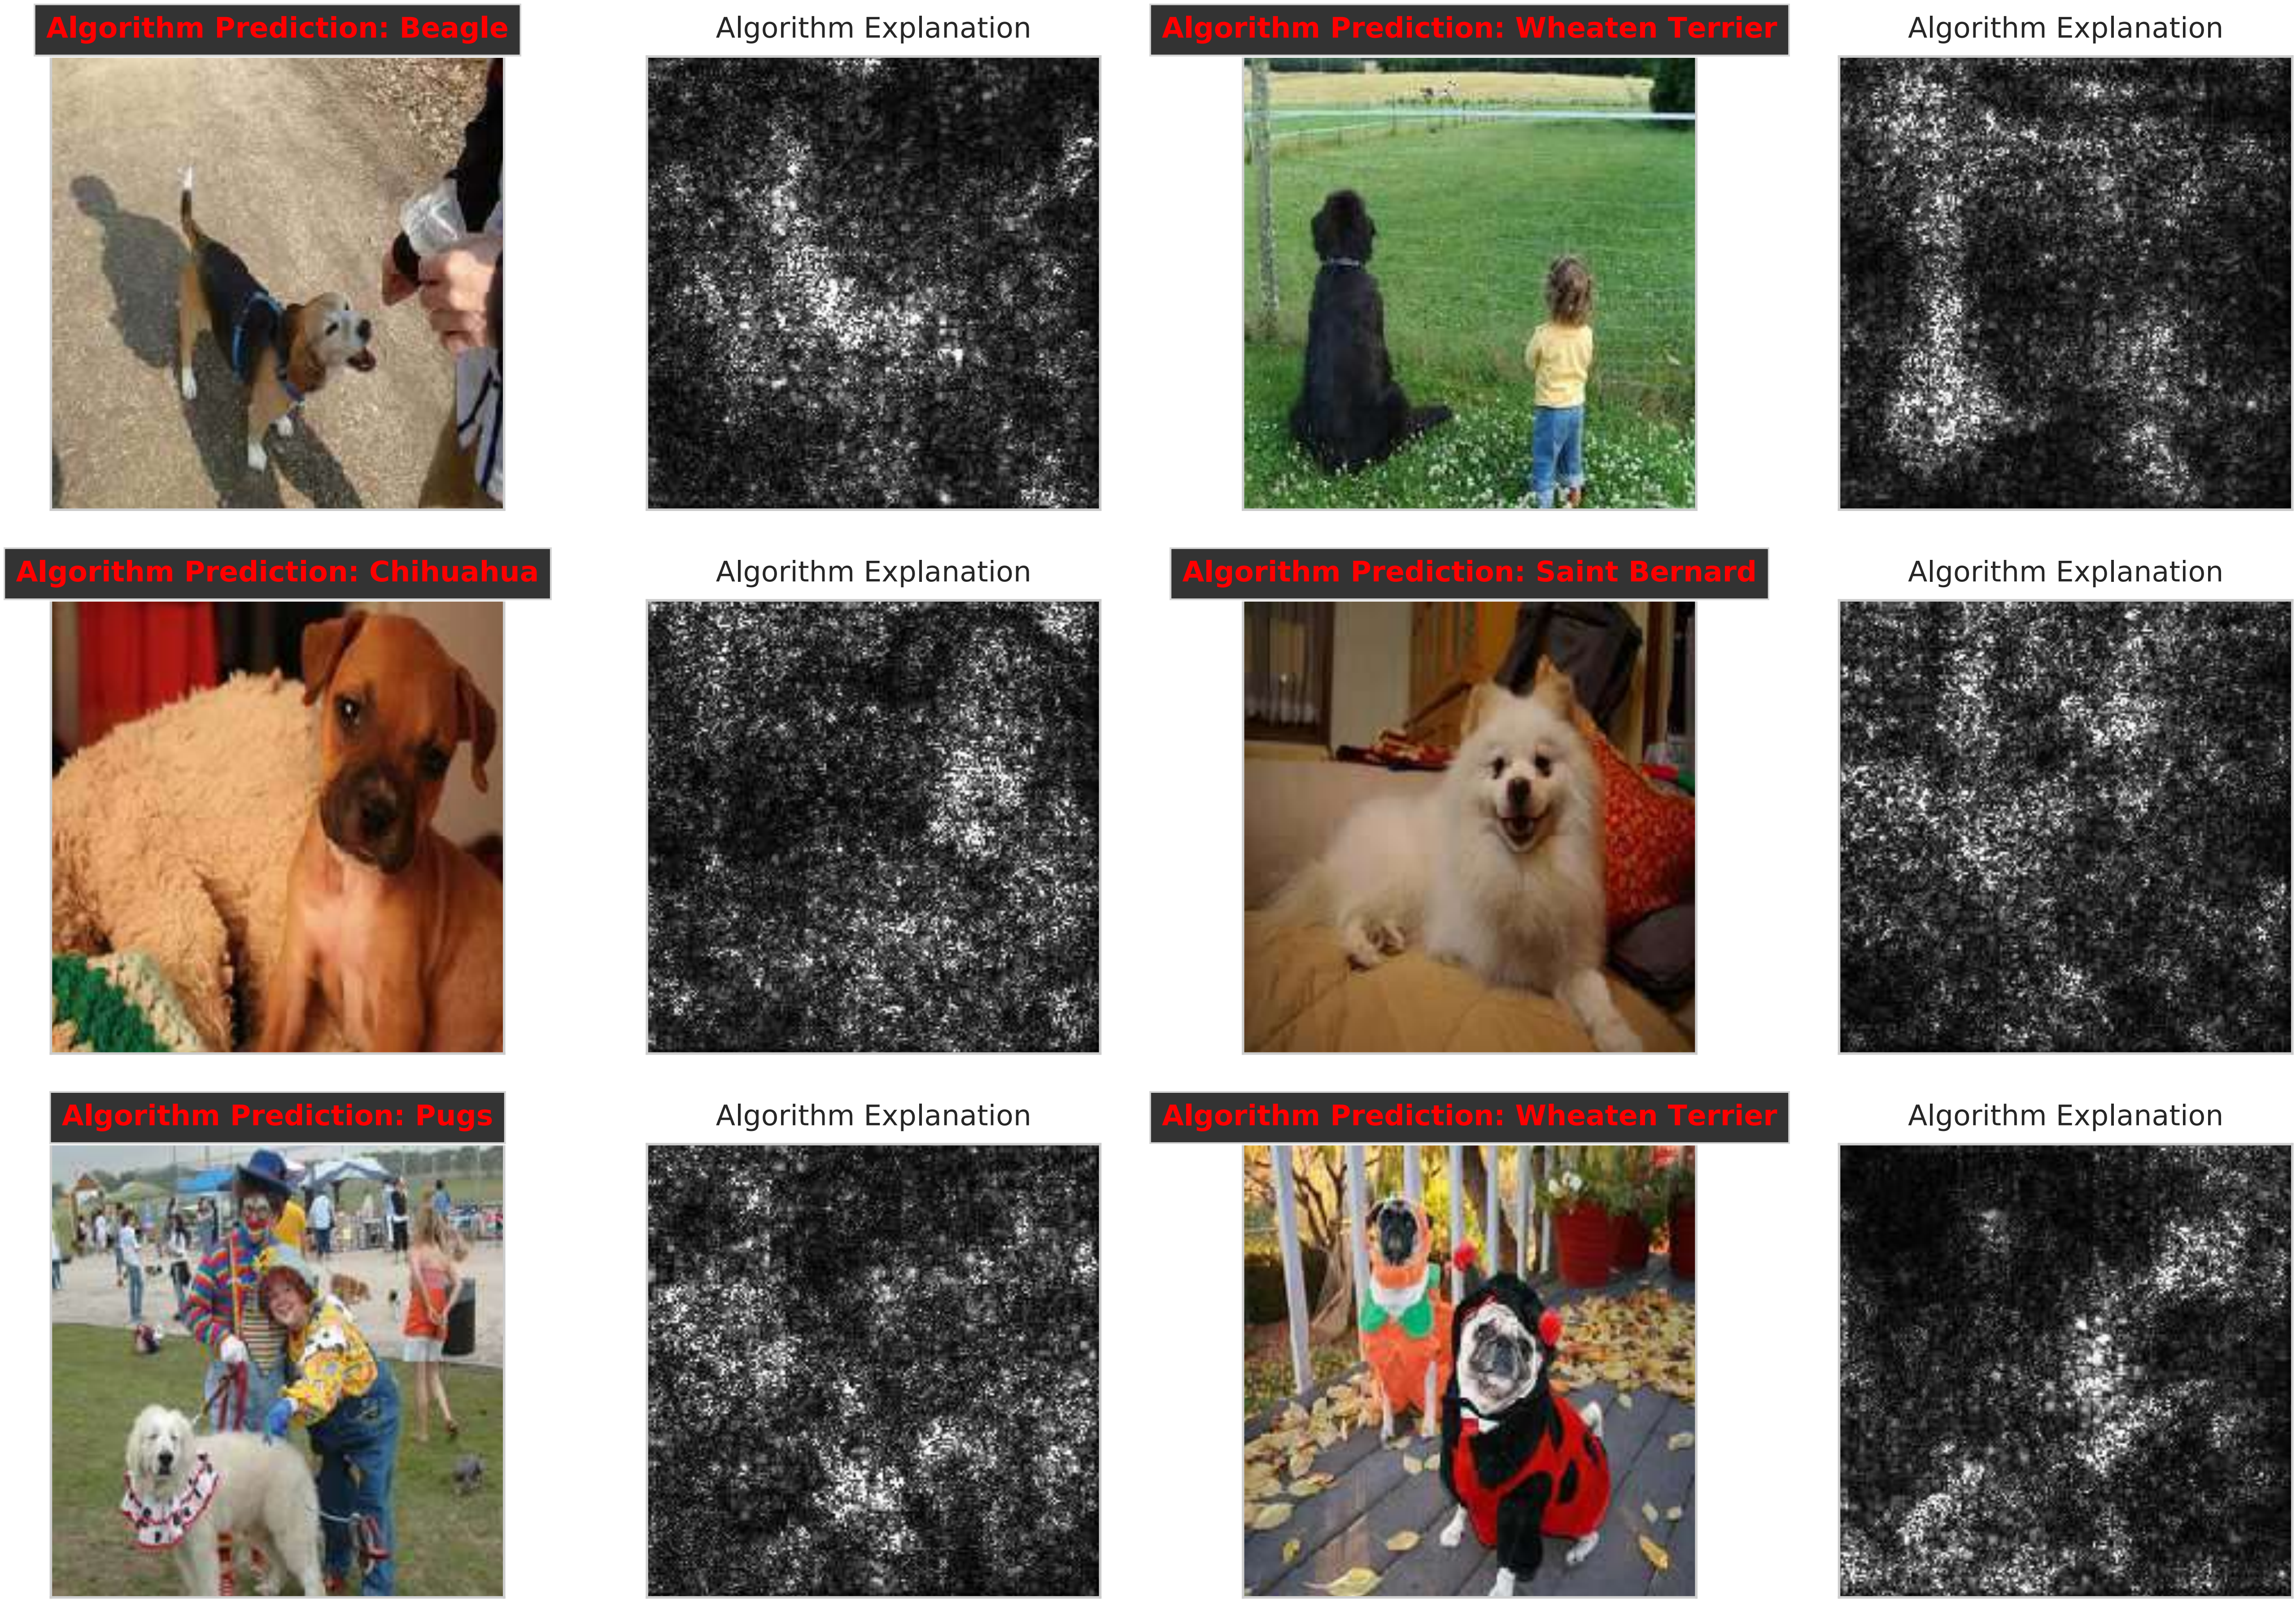

# Random Labels: SmoothGrad

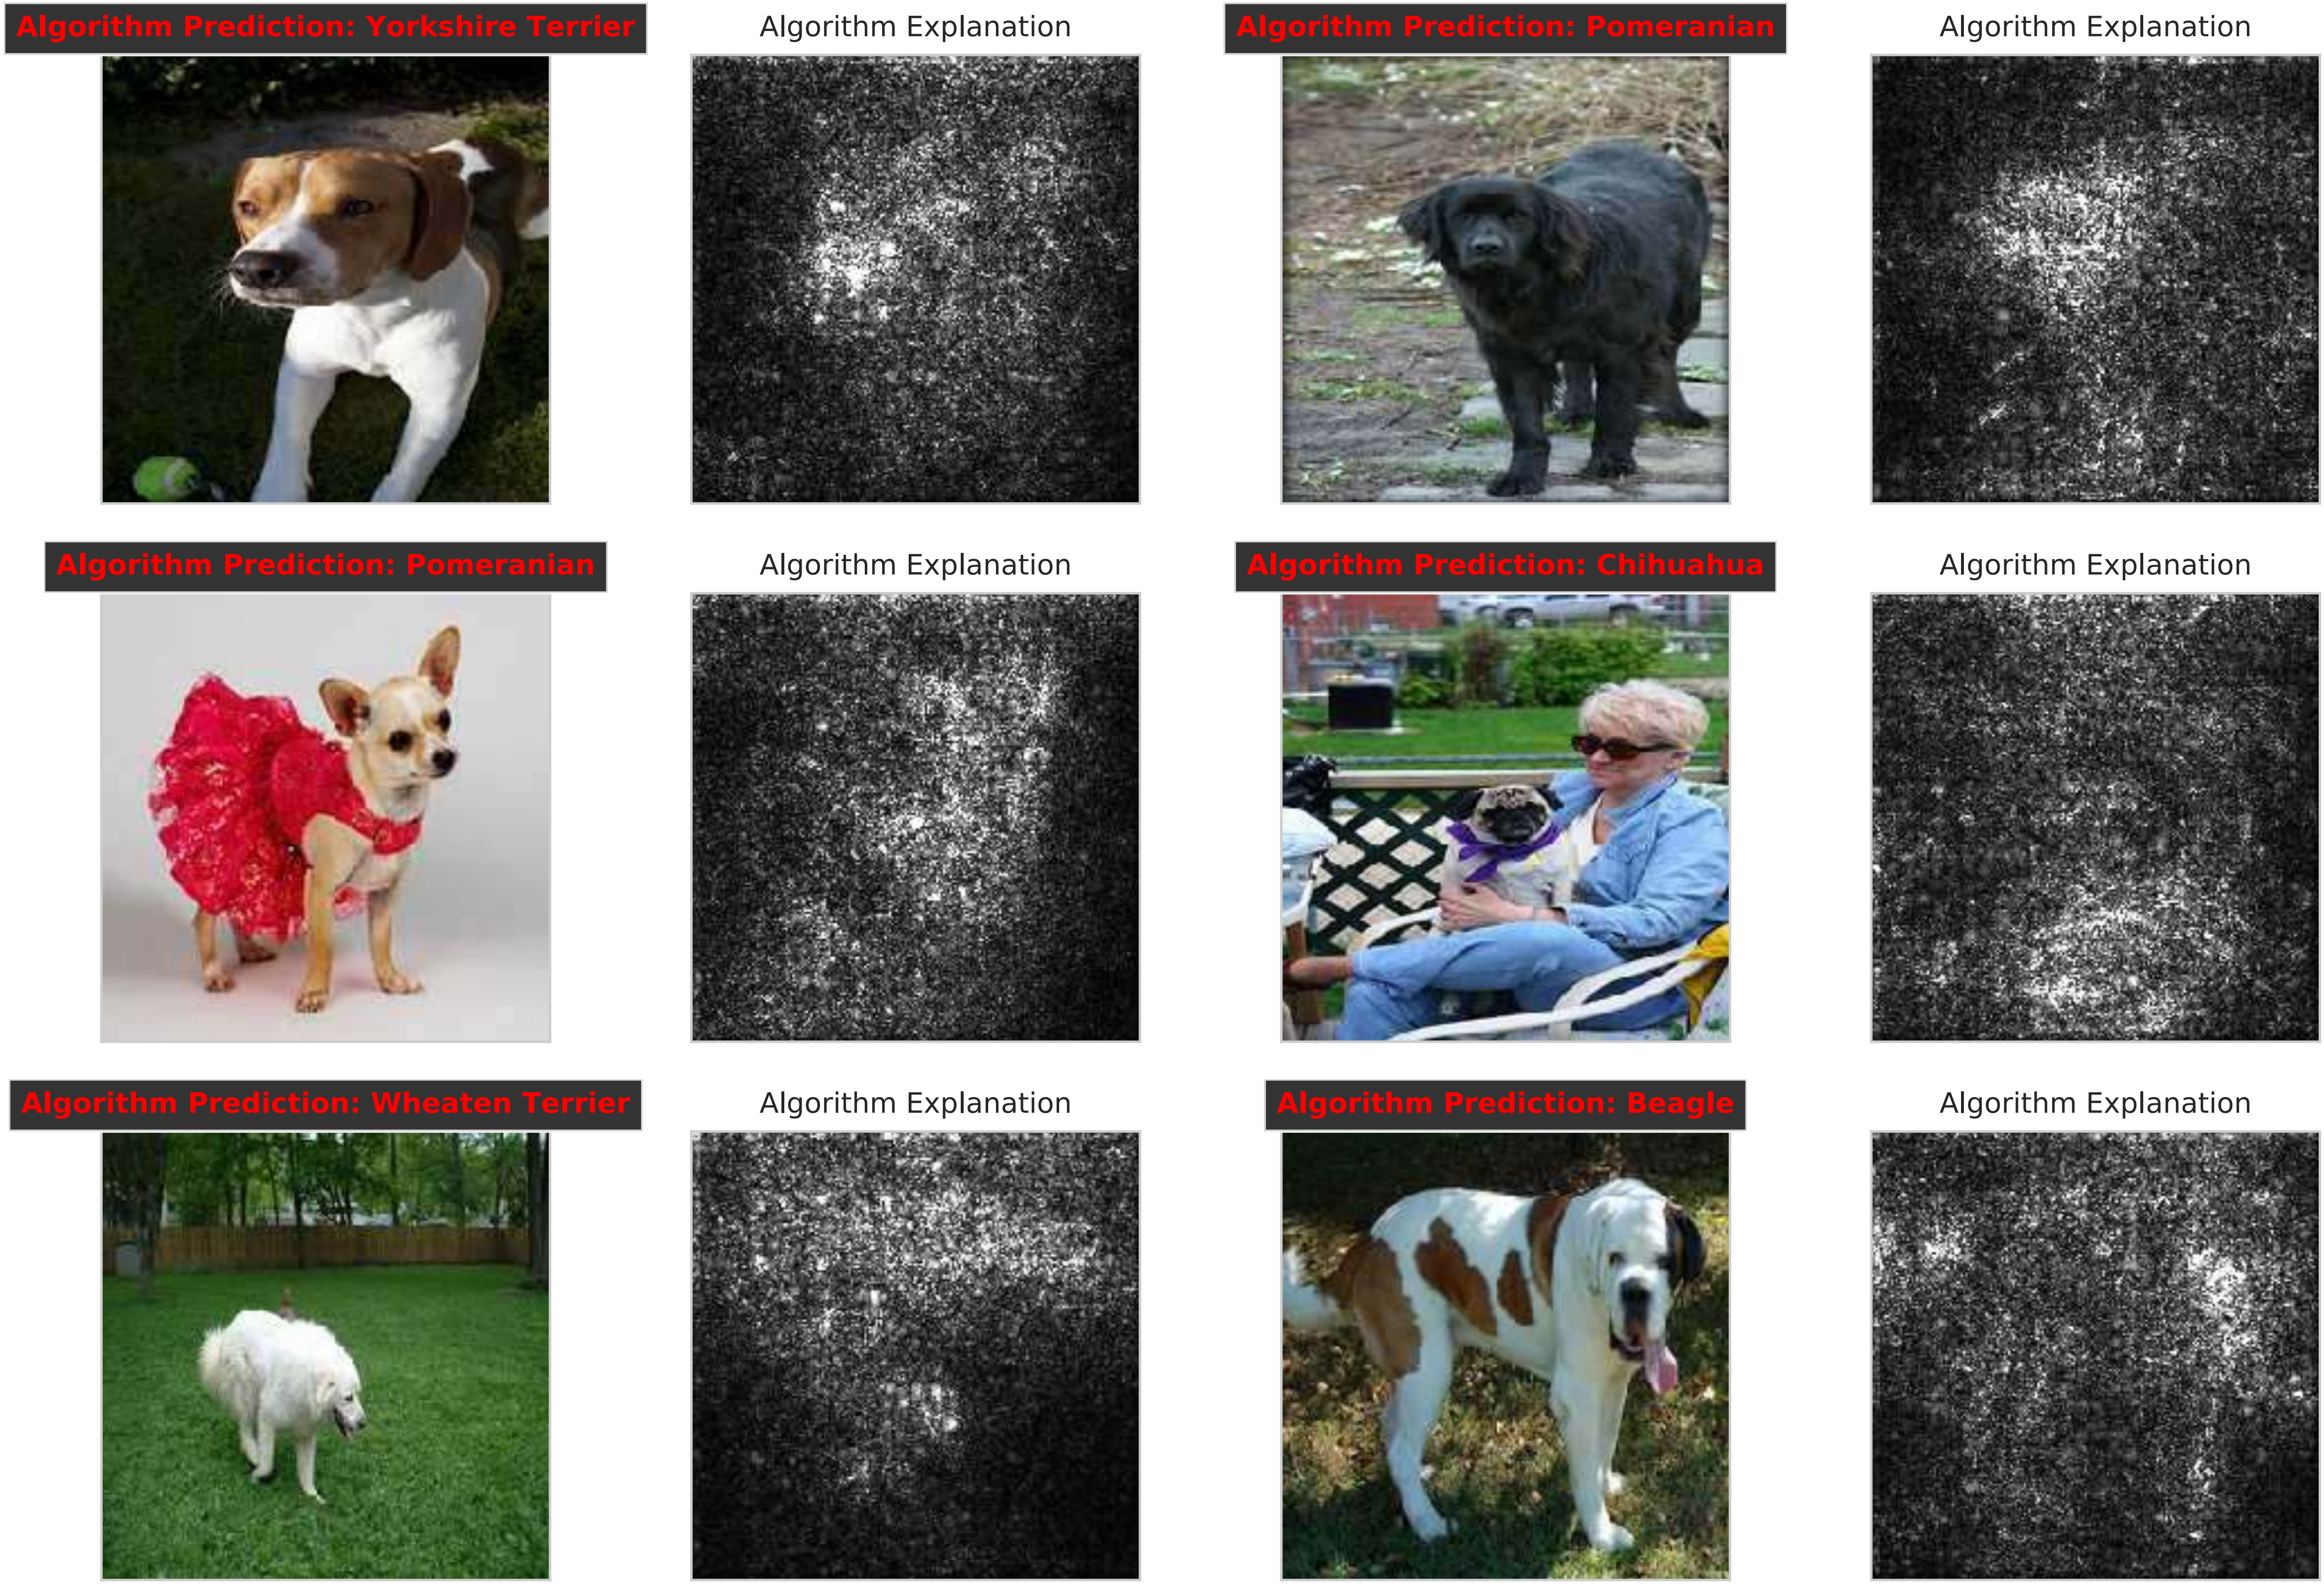

# Random Labels: Integrated Gradients

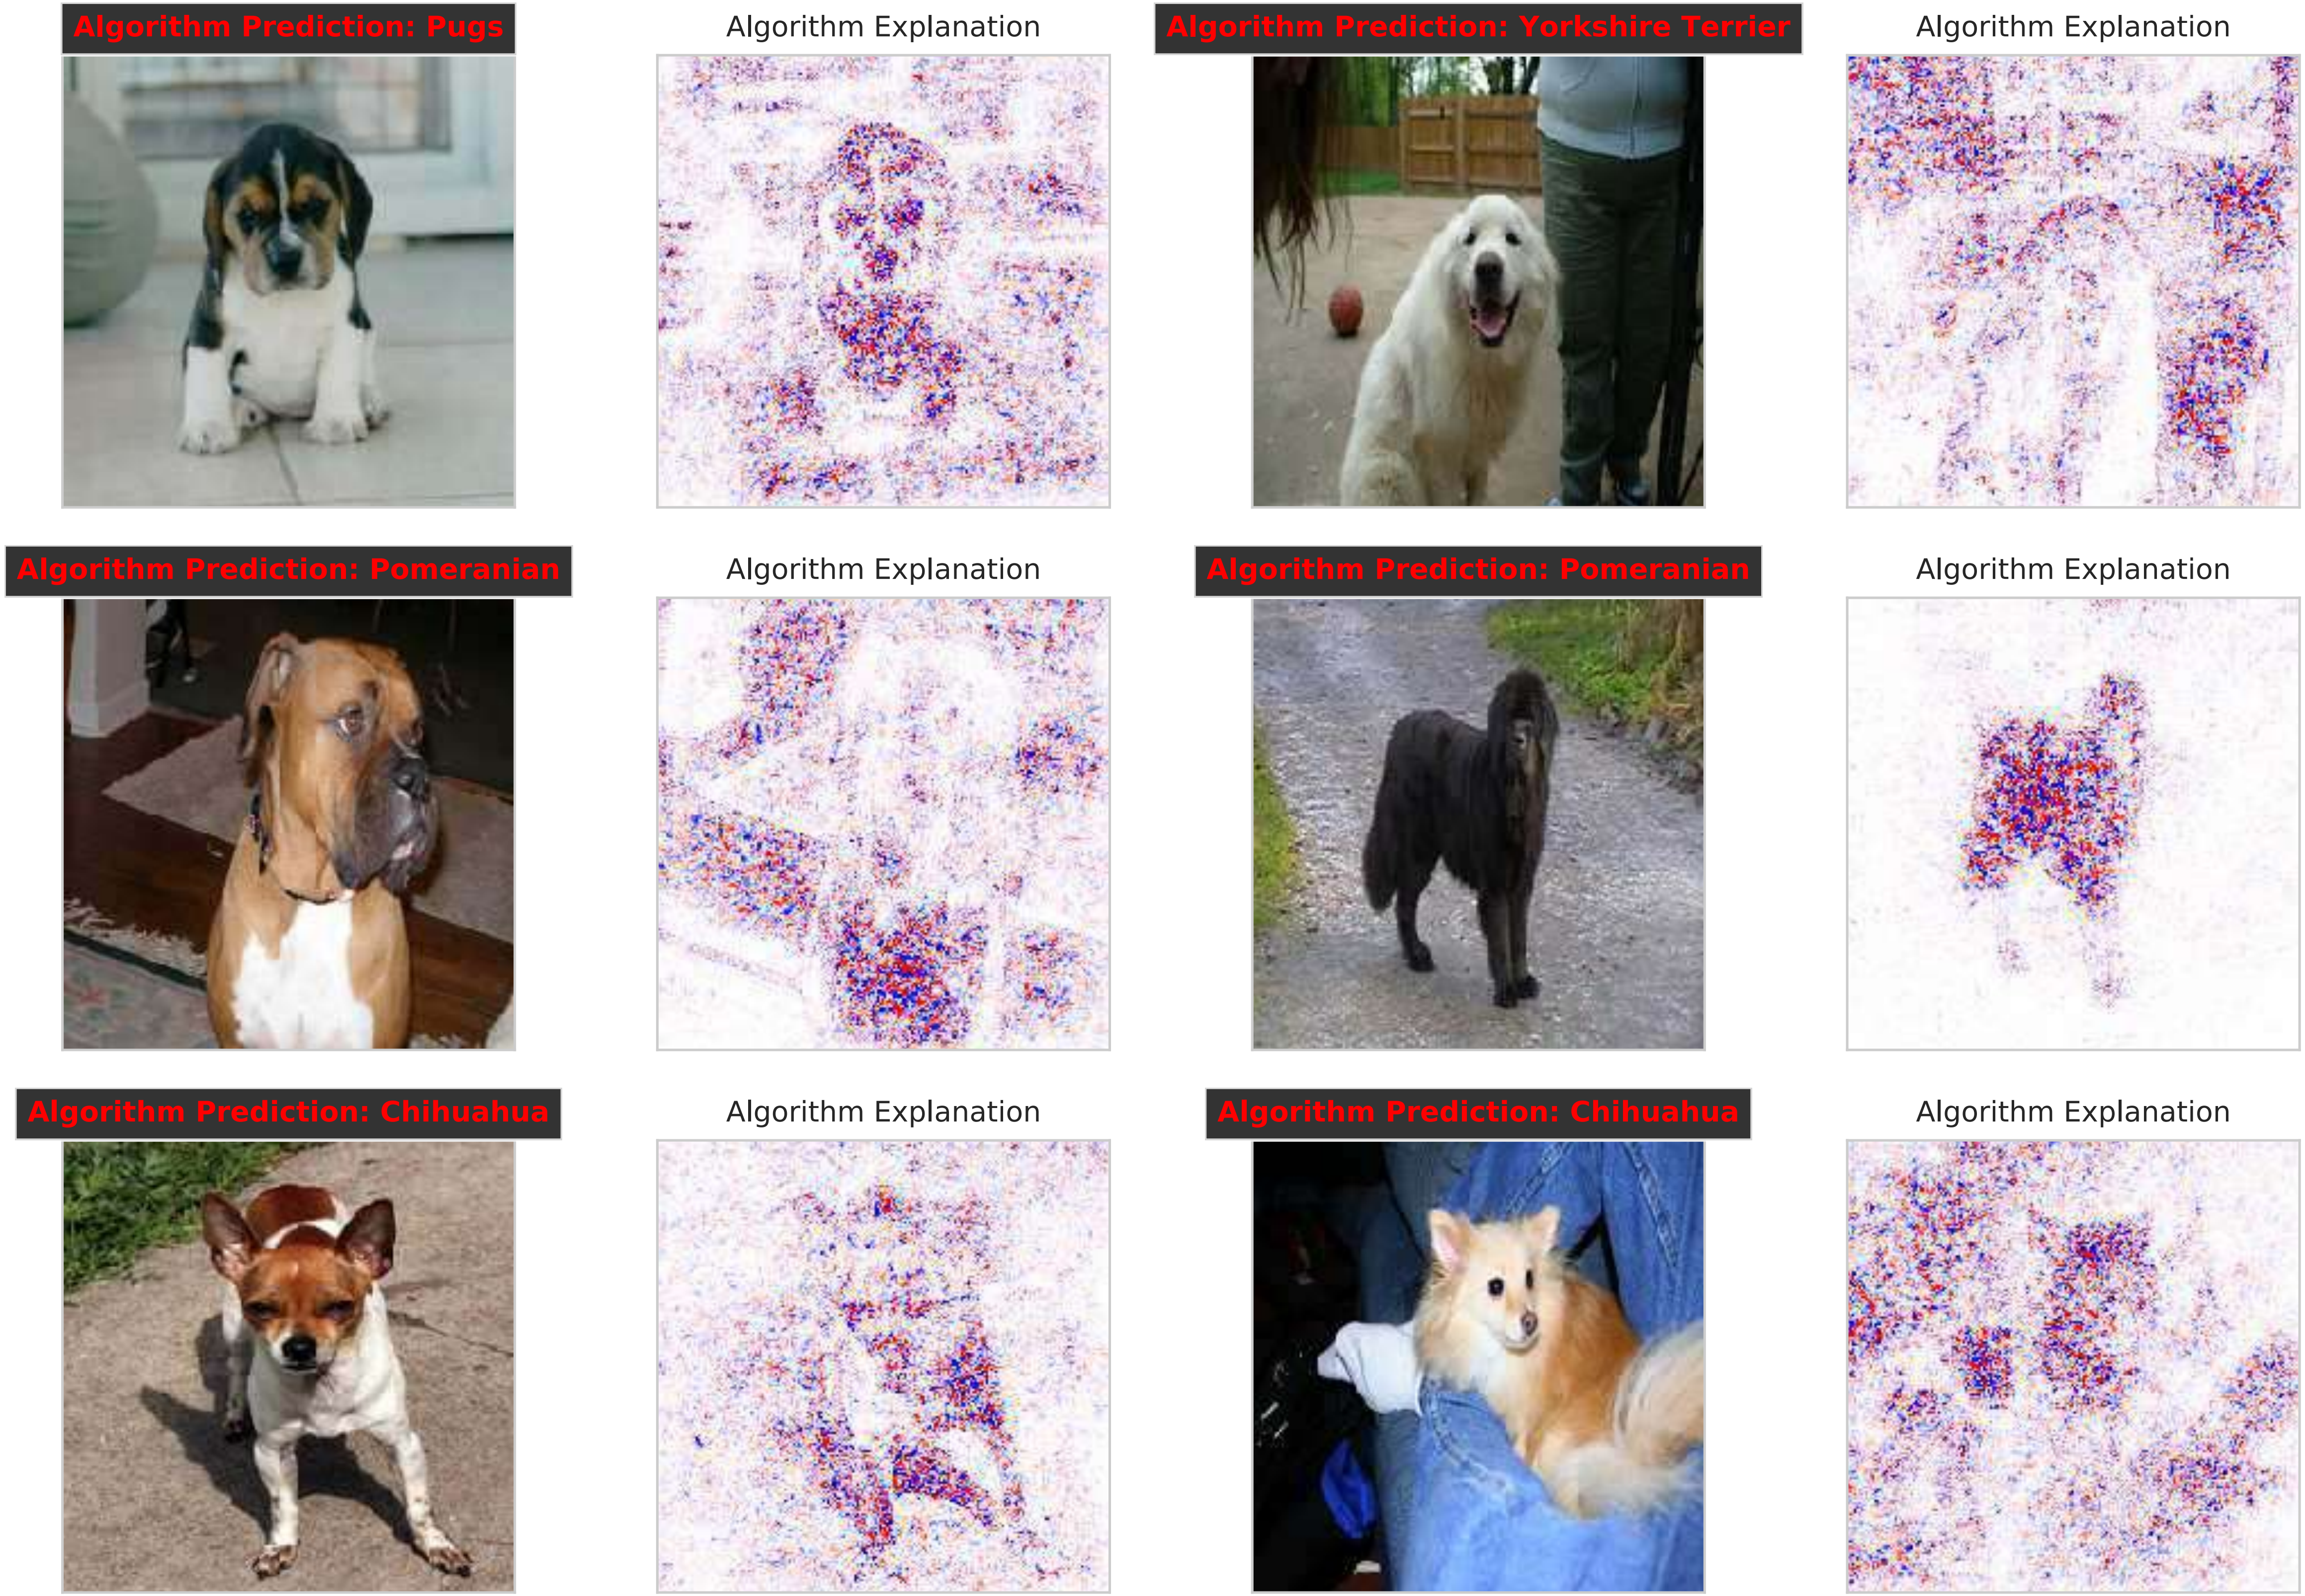

# Spurious : Gradient

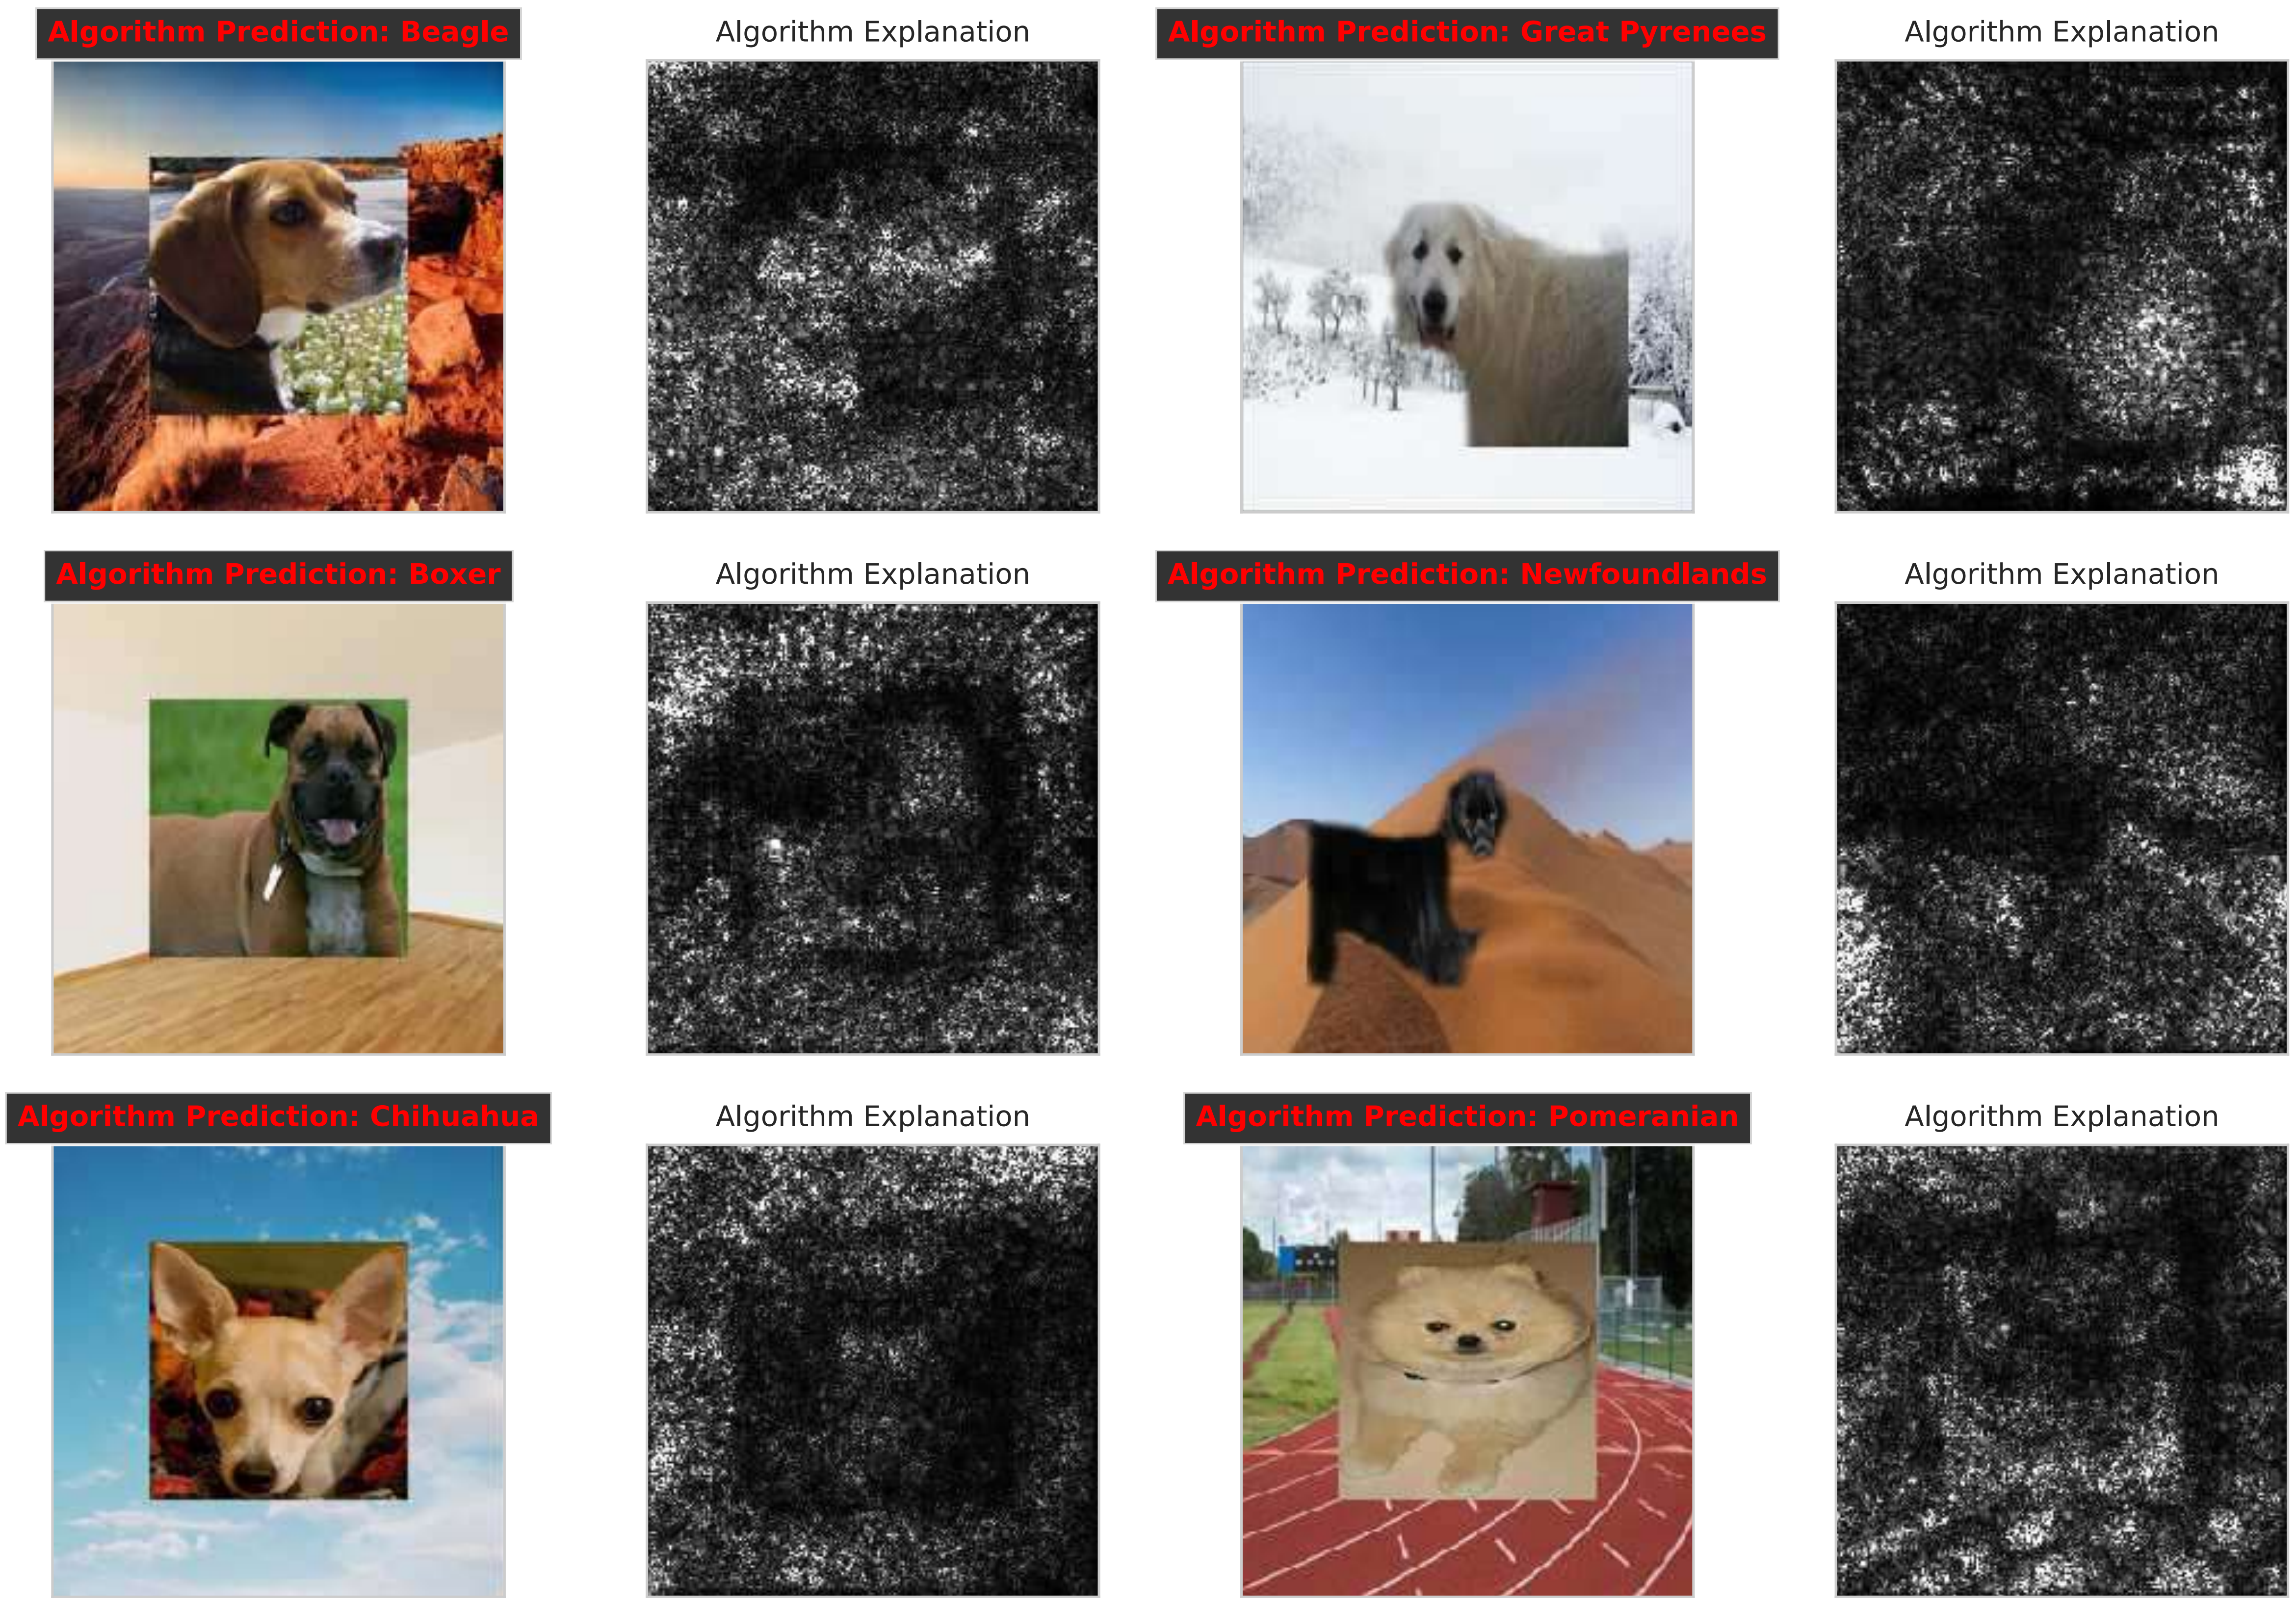

# Spurious: SmoothGrad

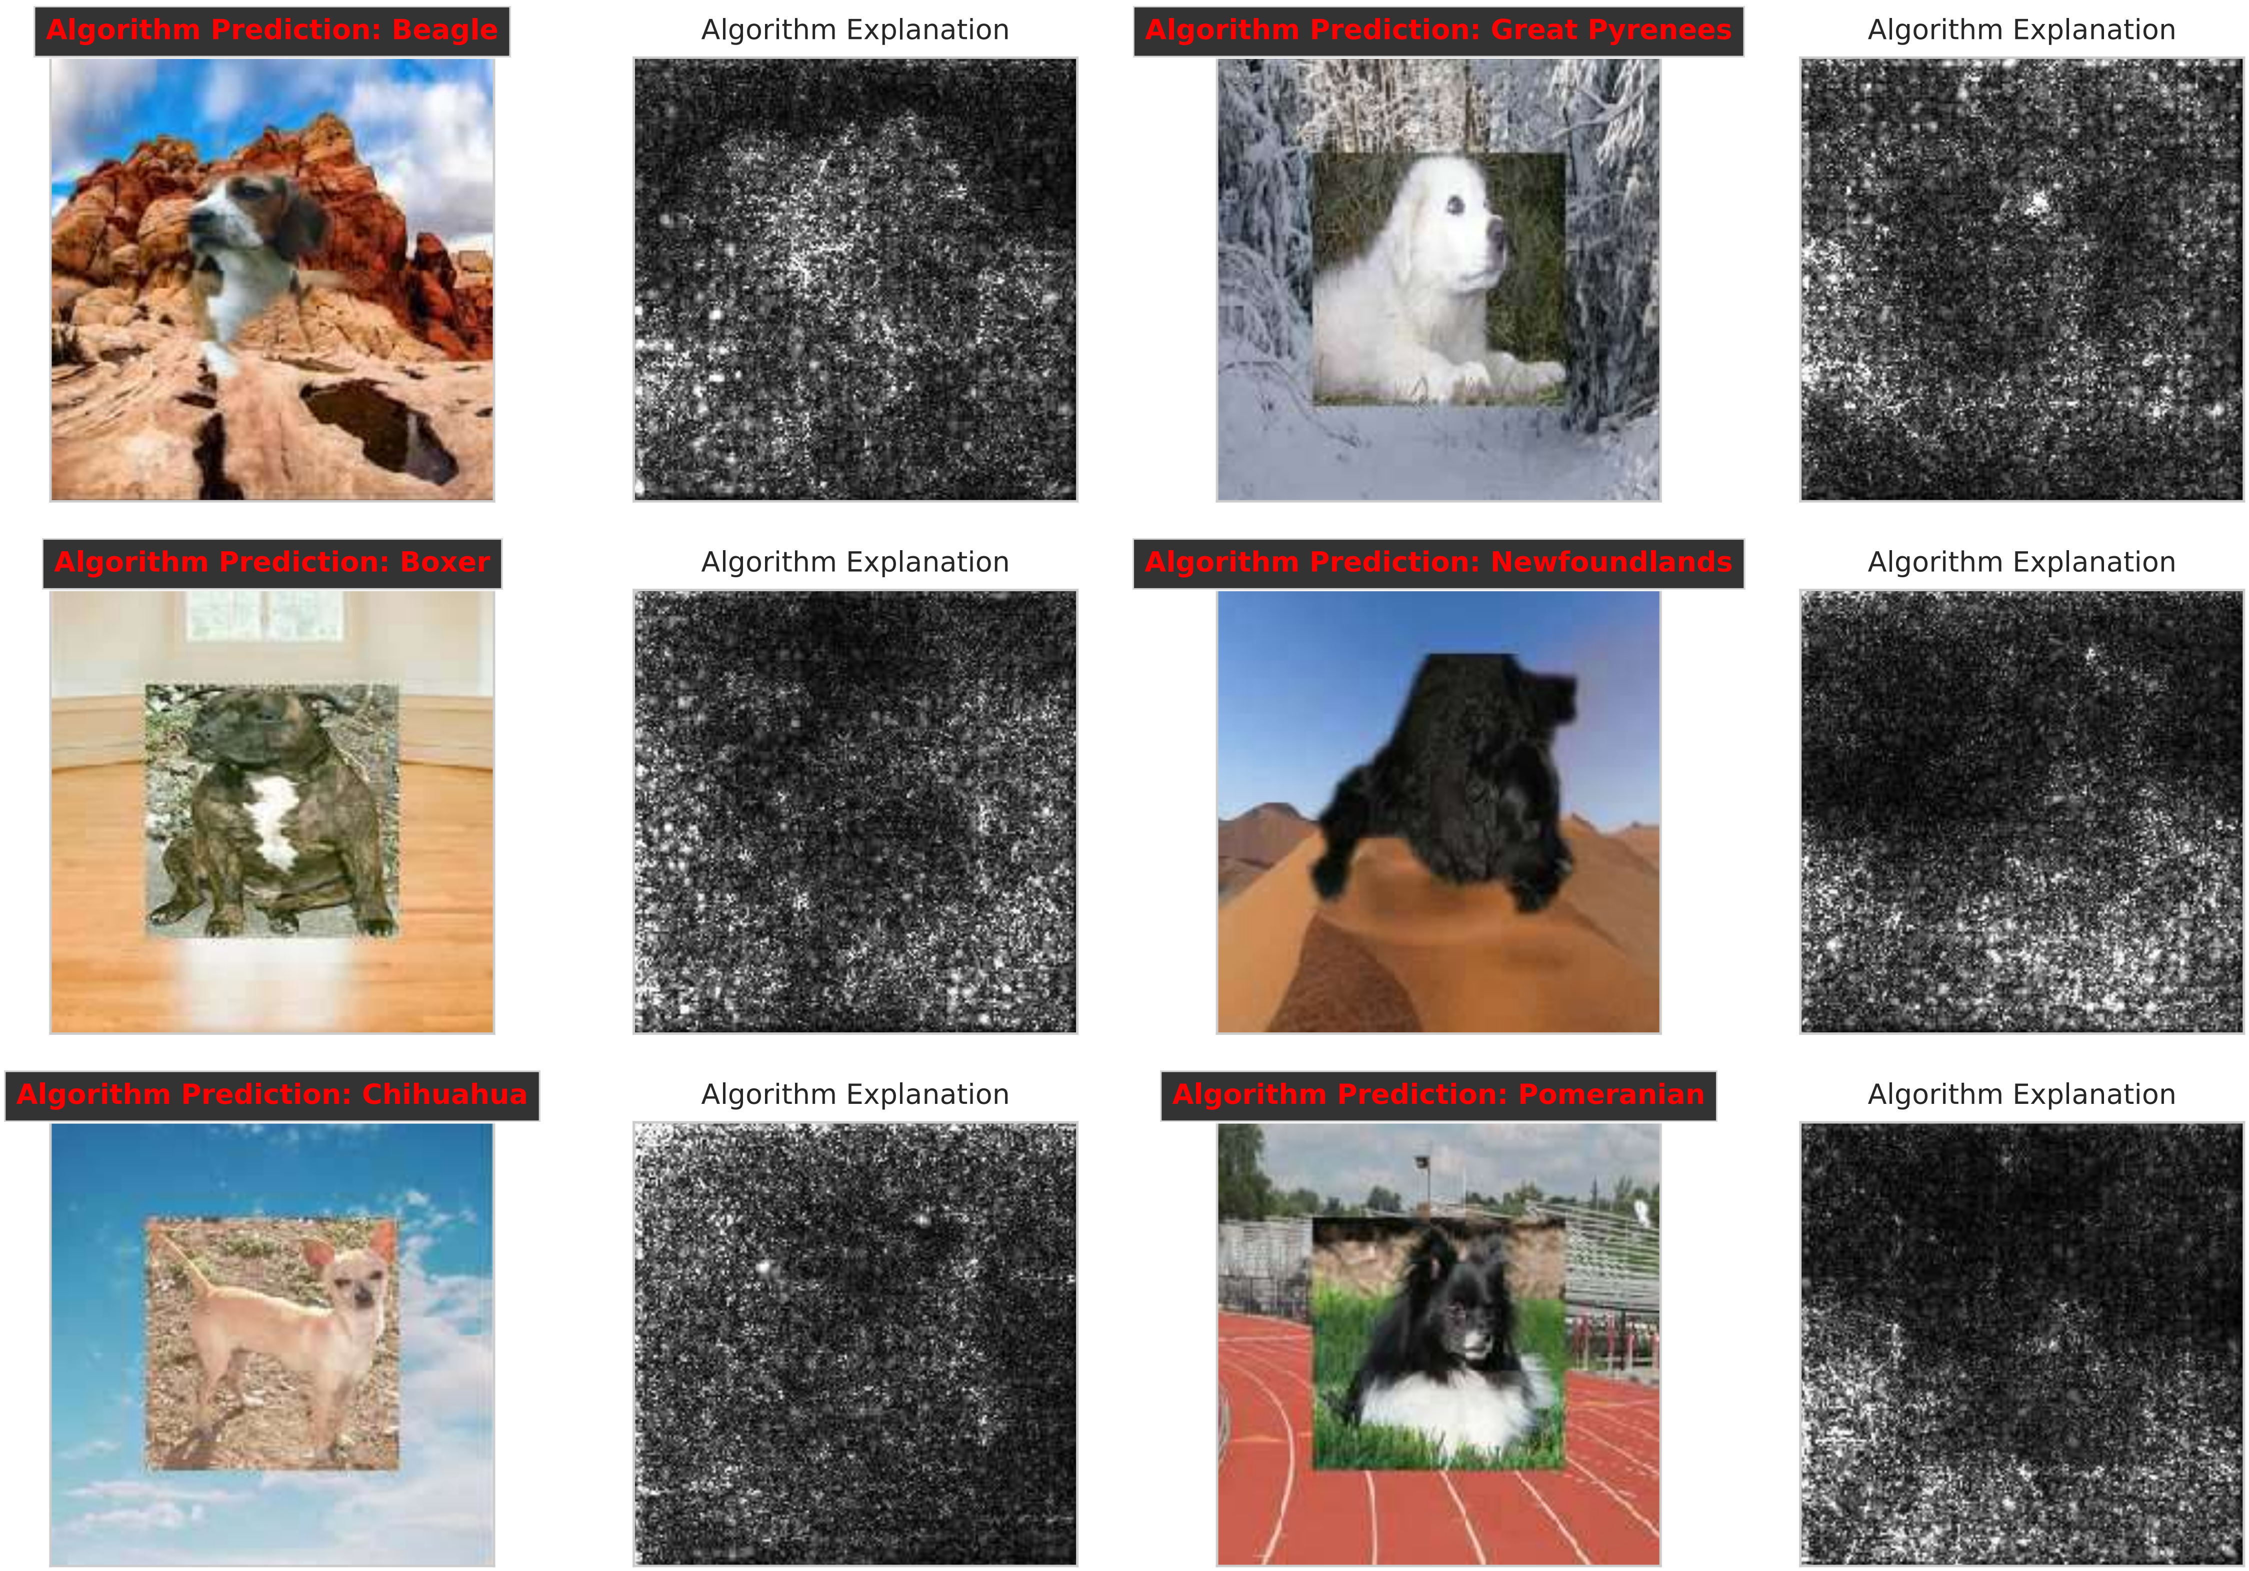

# Spurious: Integrated Gradients

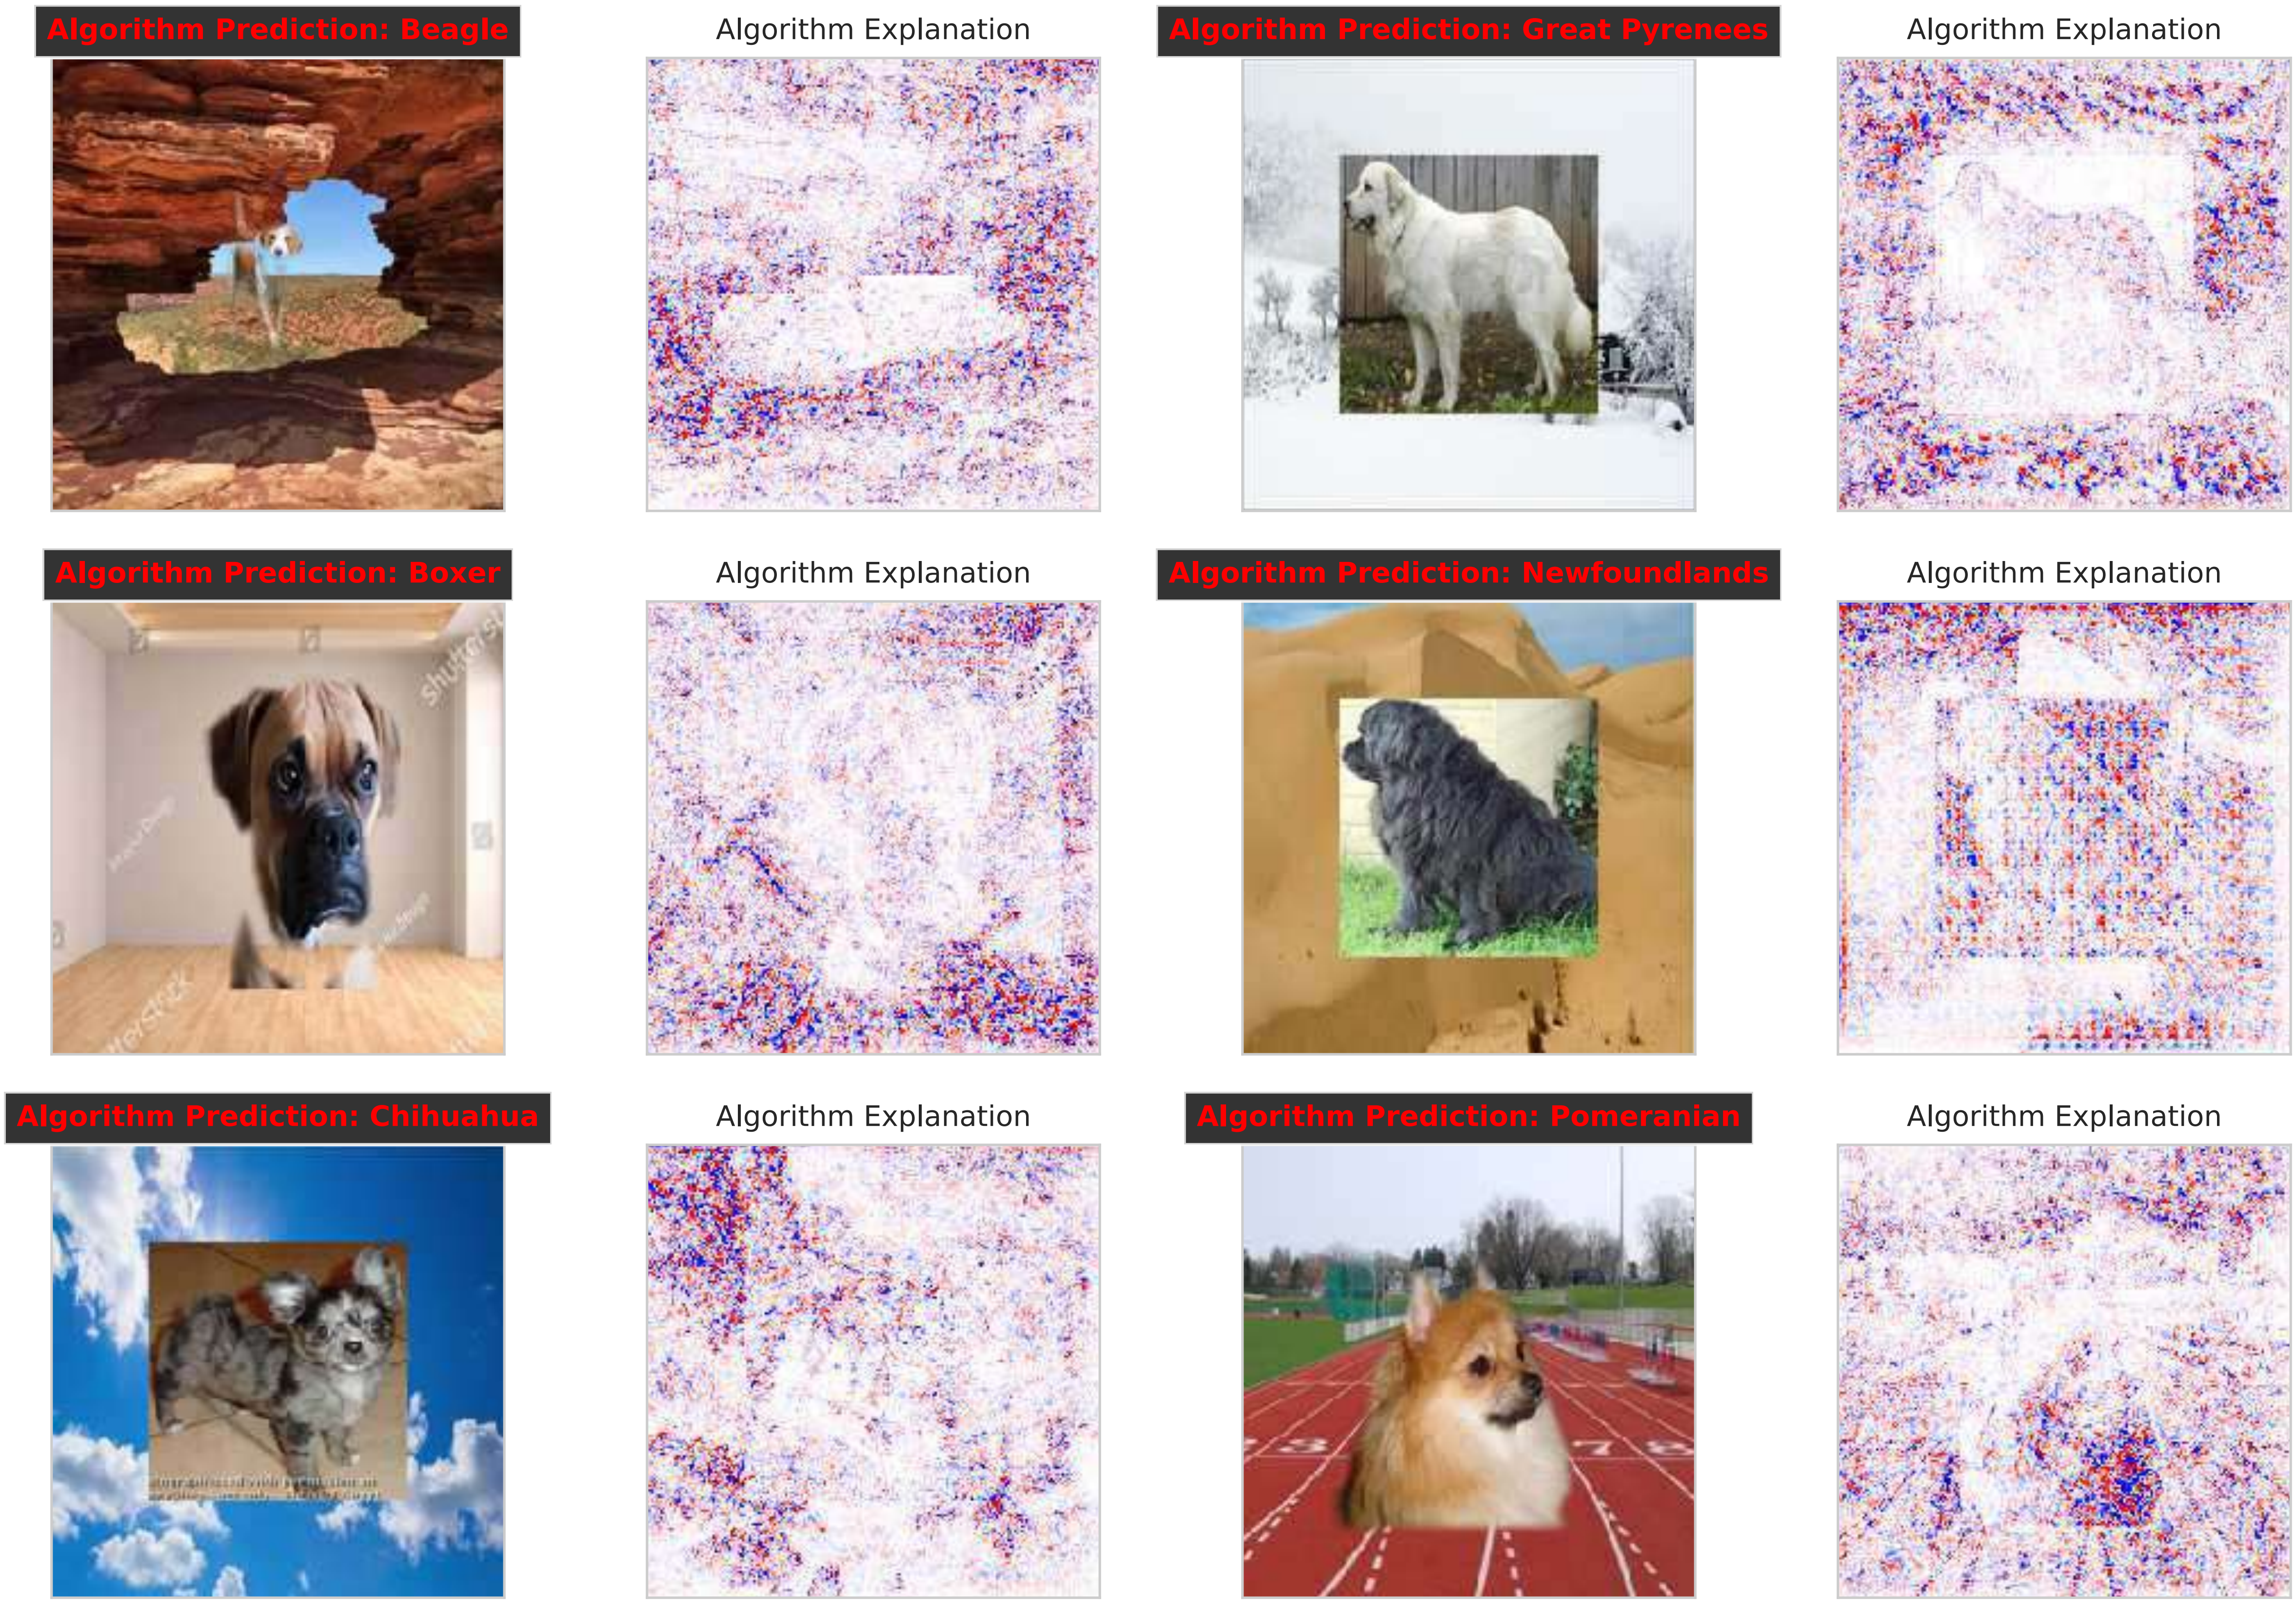

# Partial-Spurious : Gradient

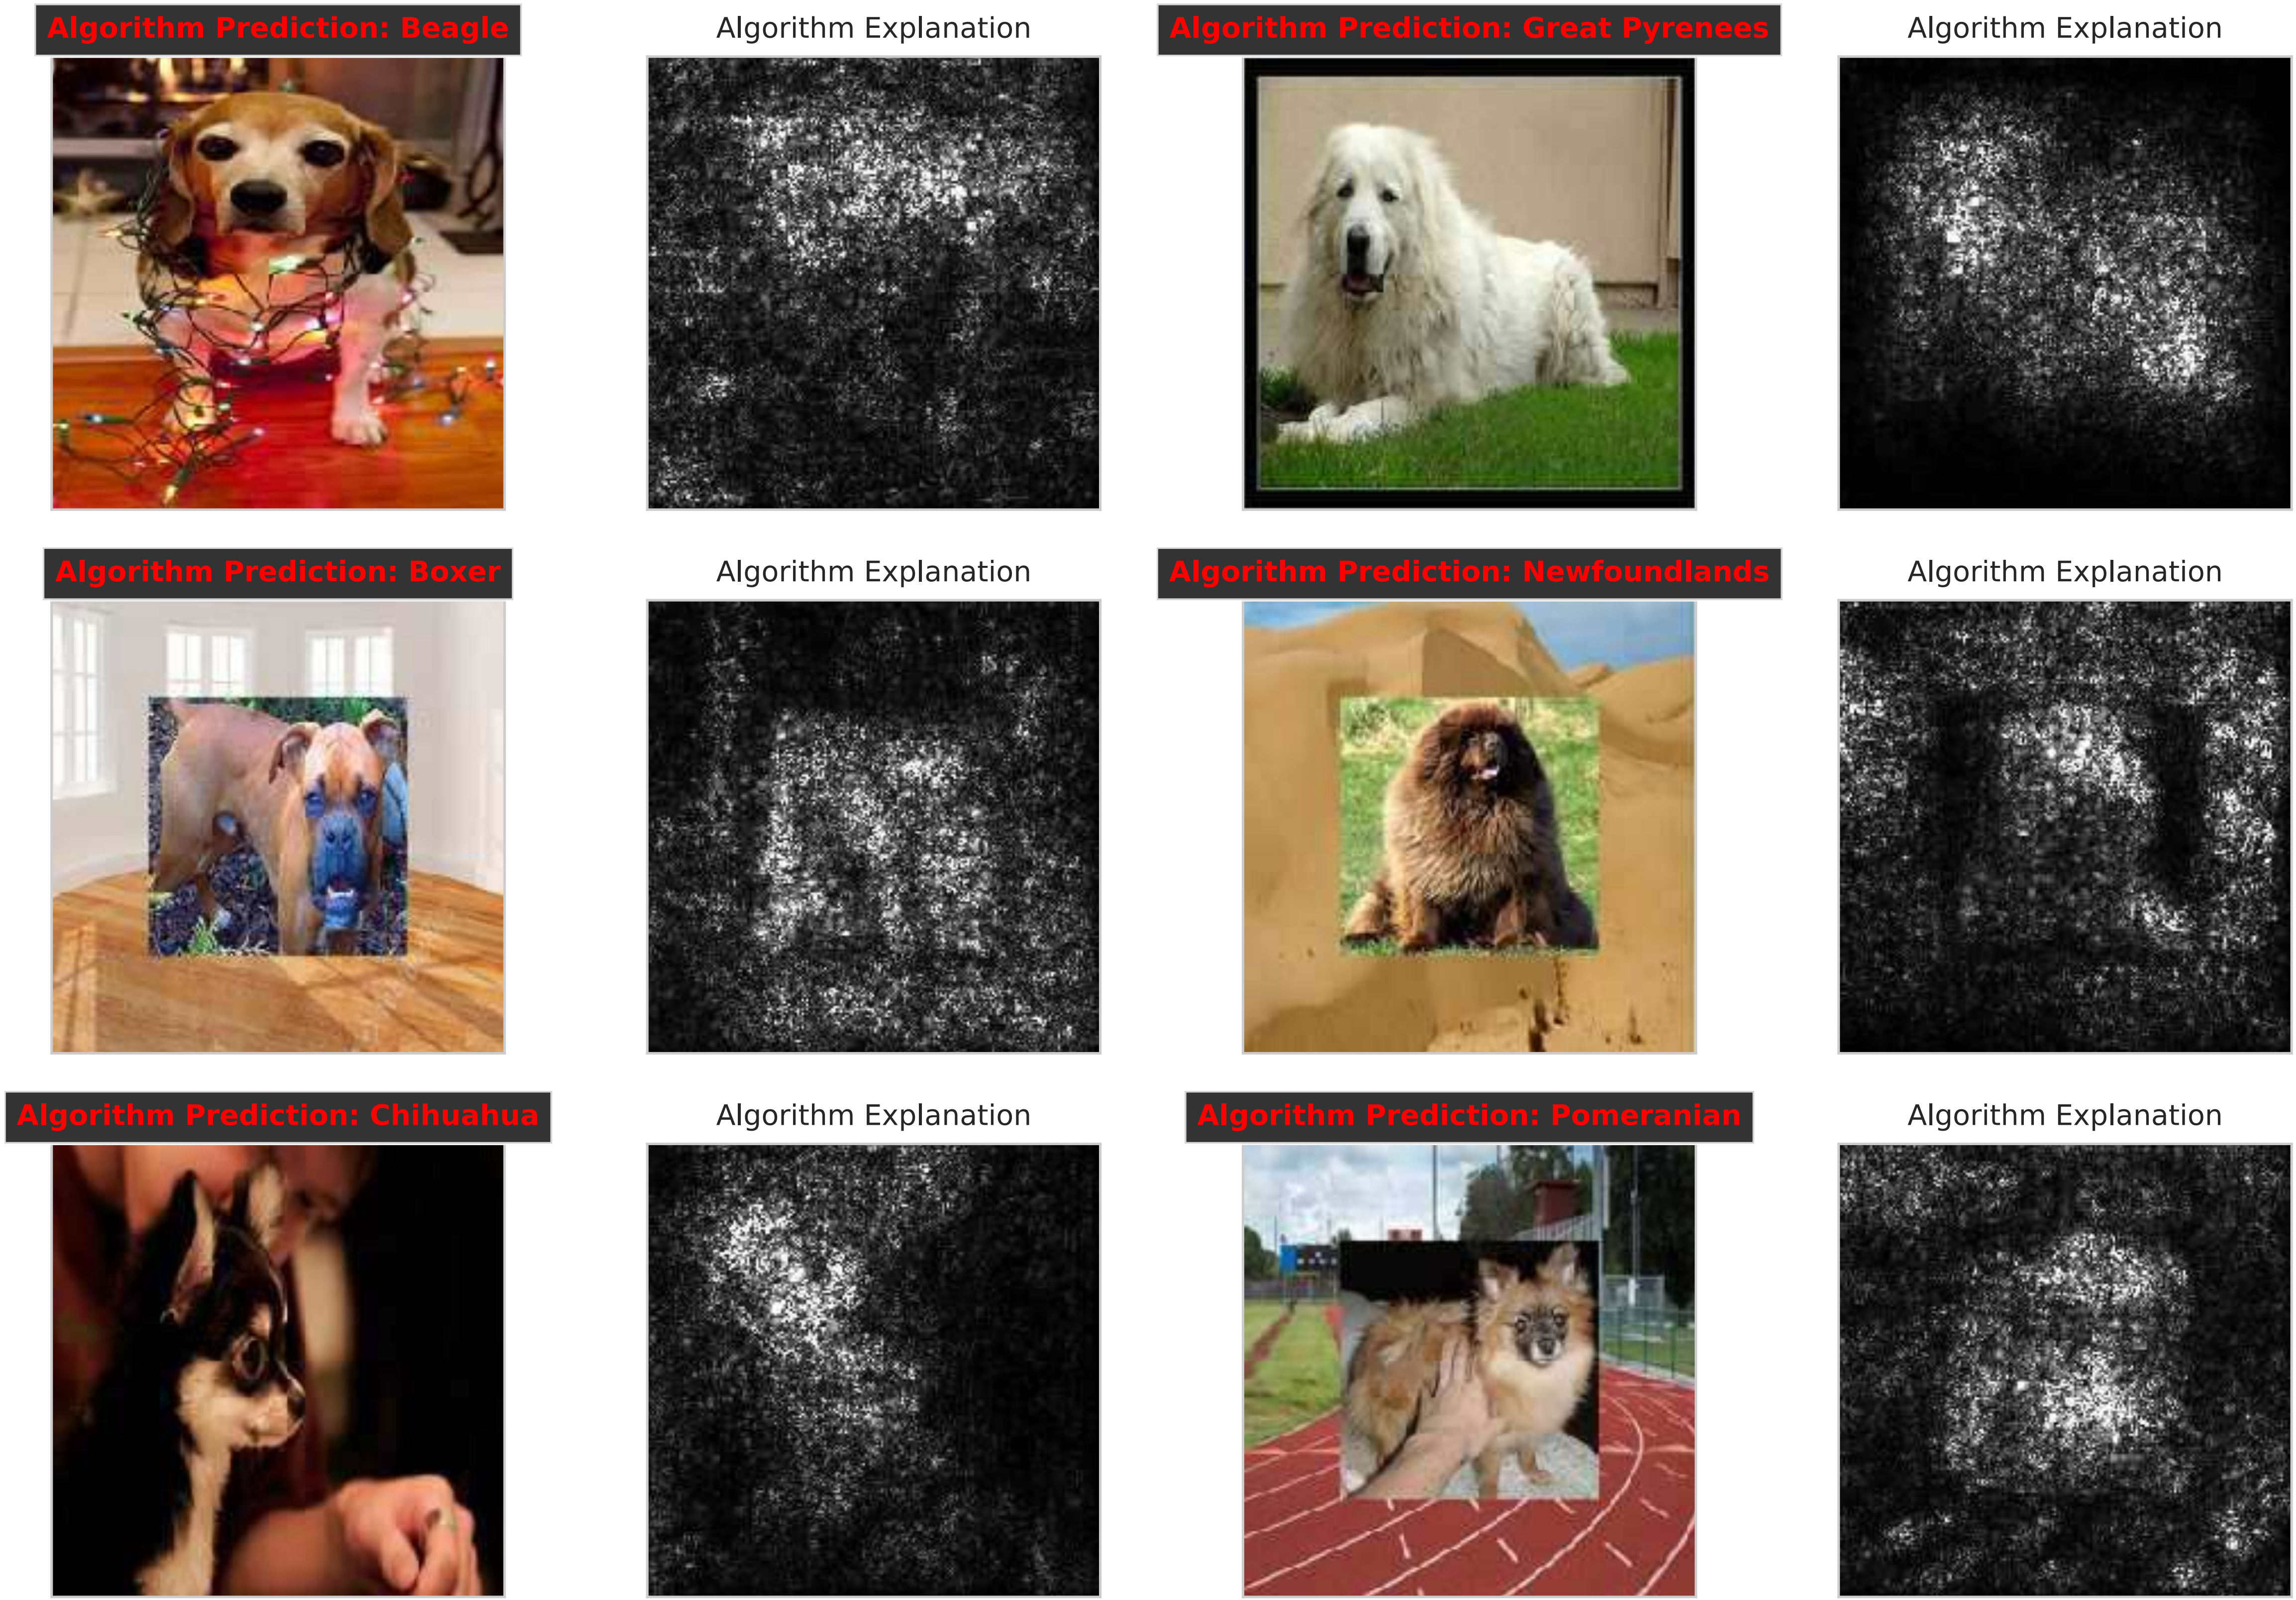

# Partial-Spurious: SmoothGrad

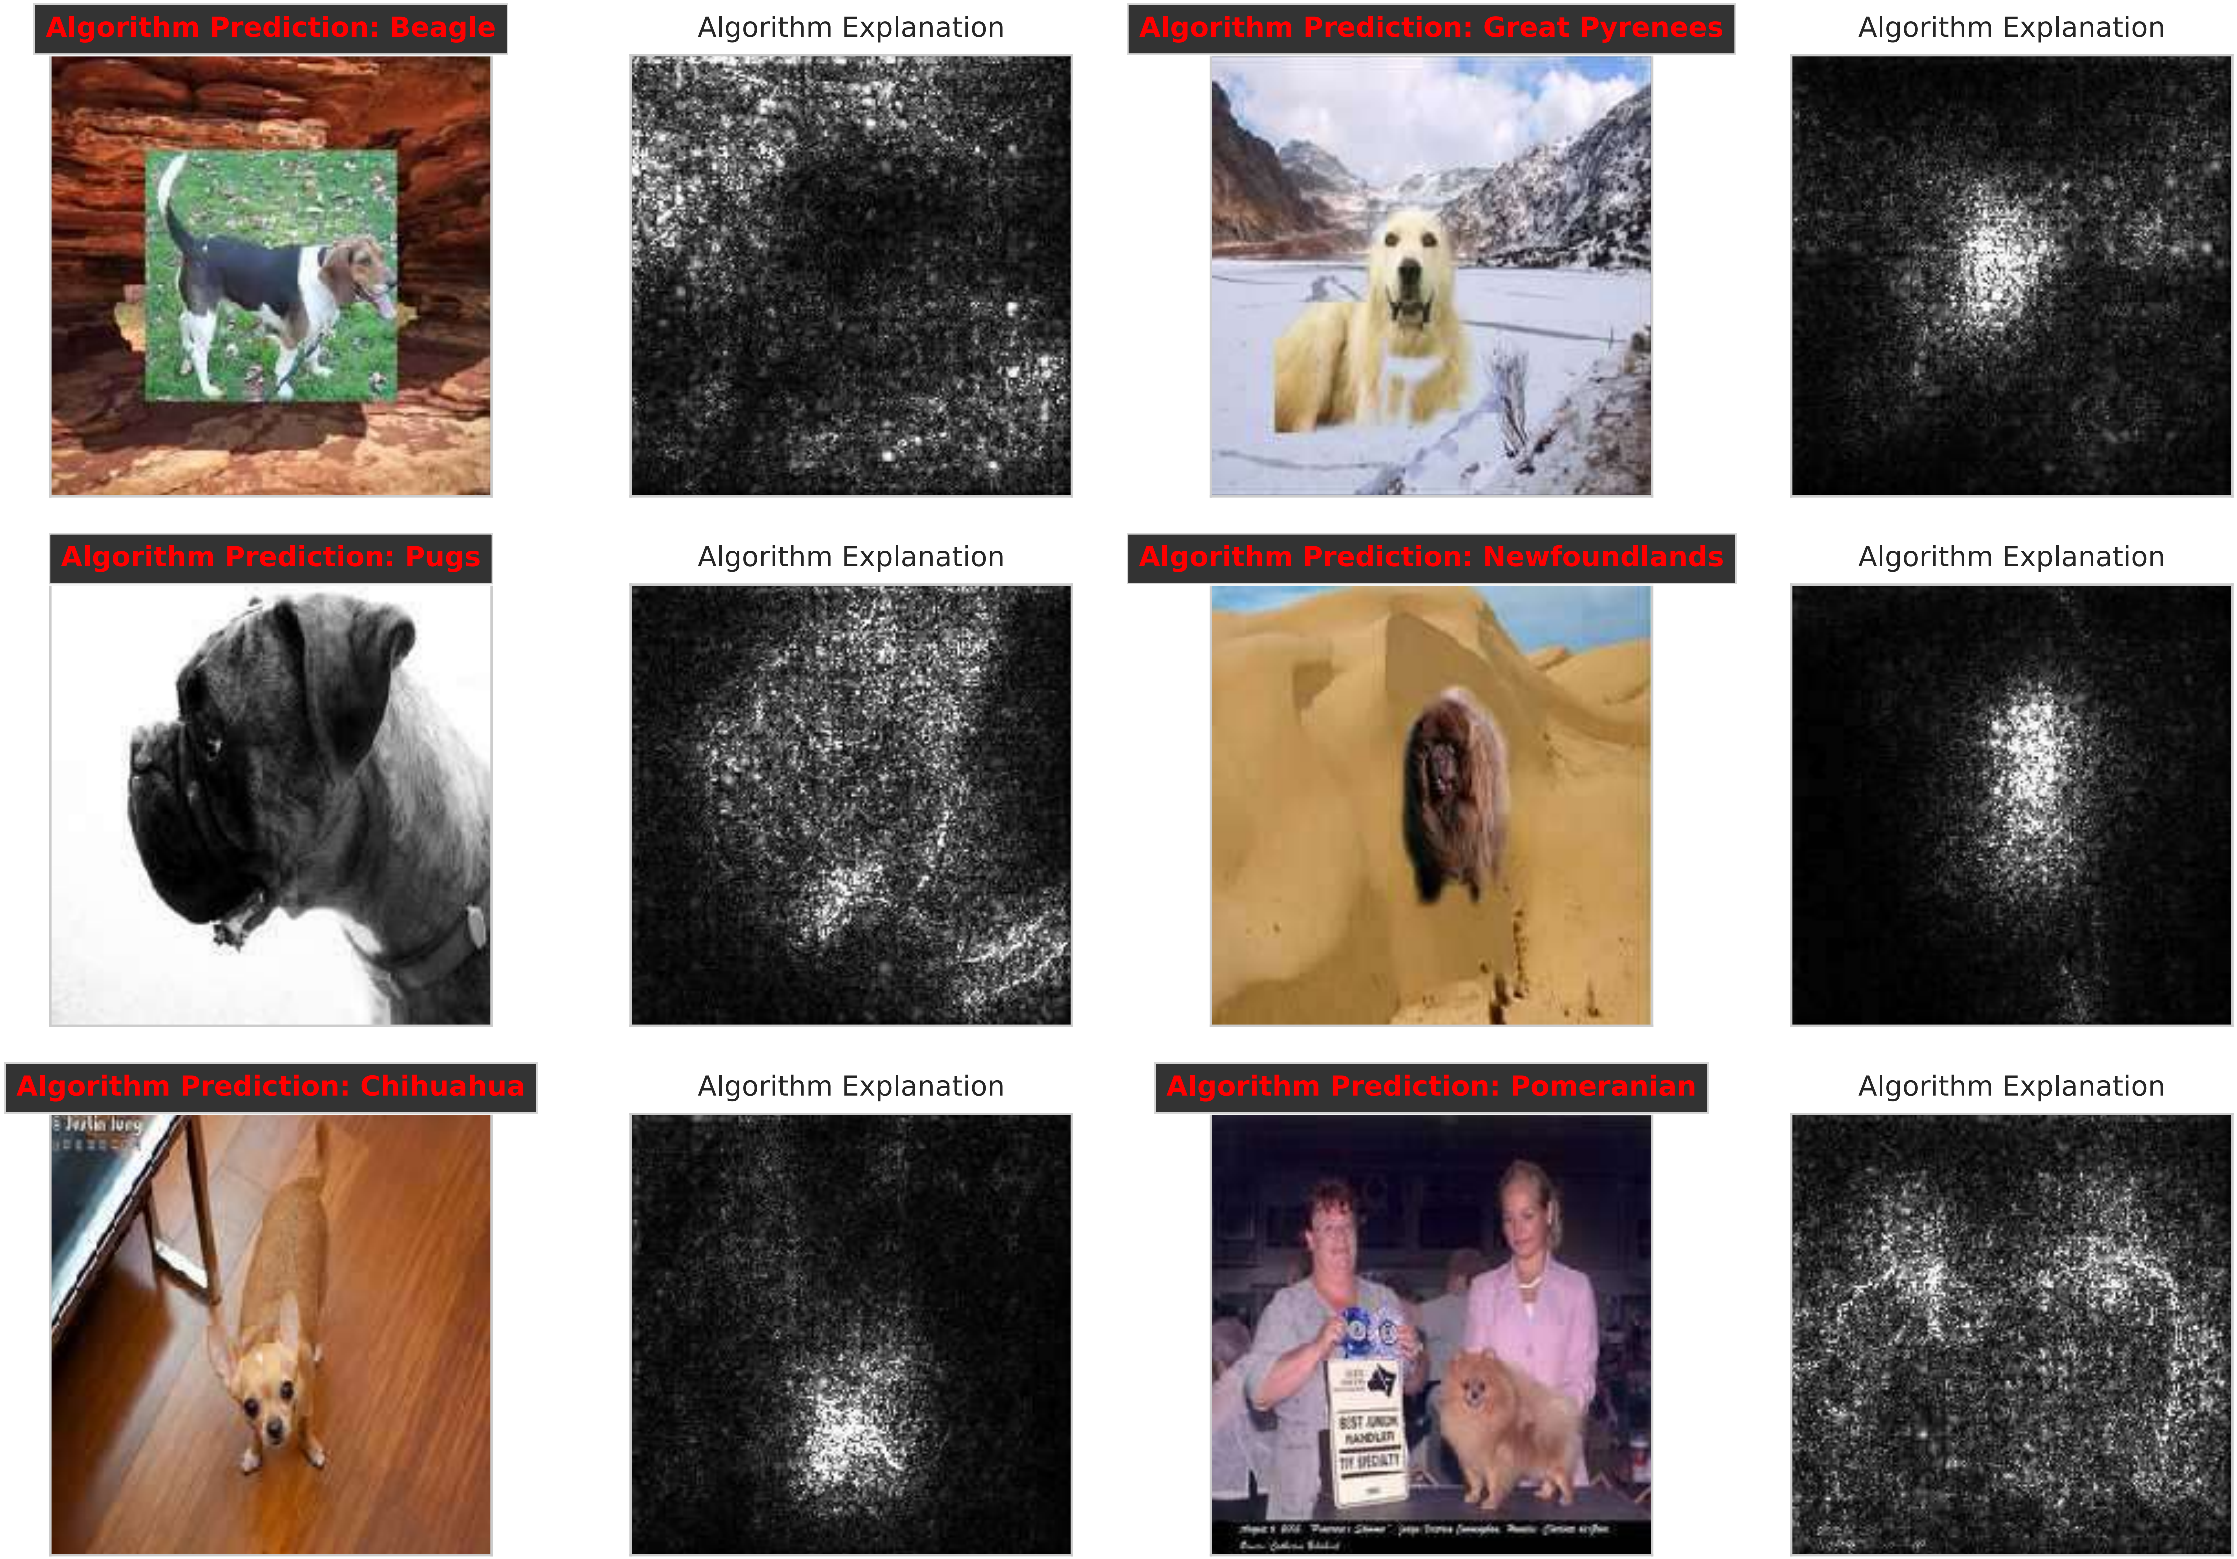

# Partial-Spurious: Integrated Gradients

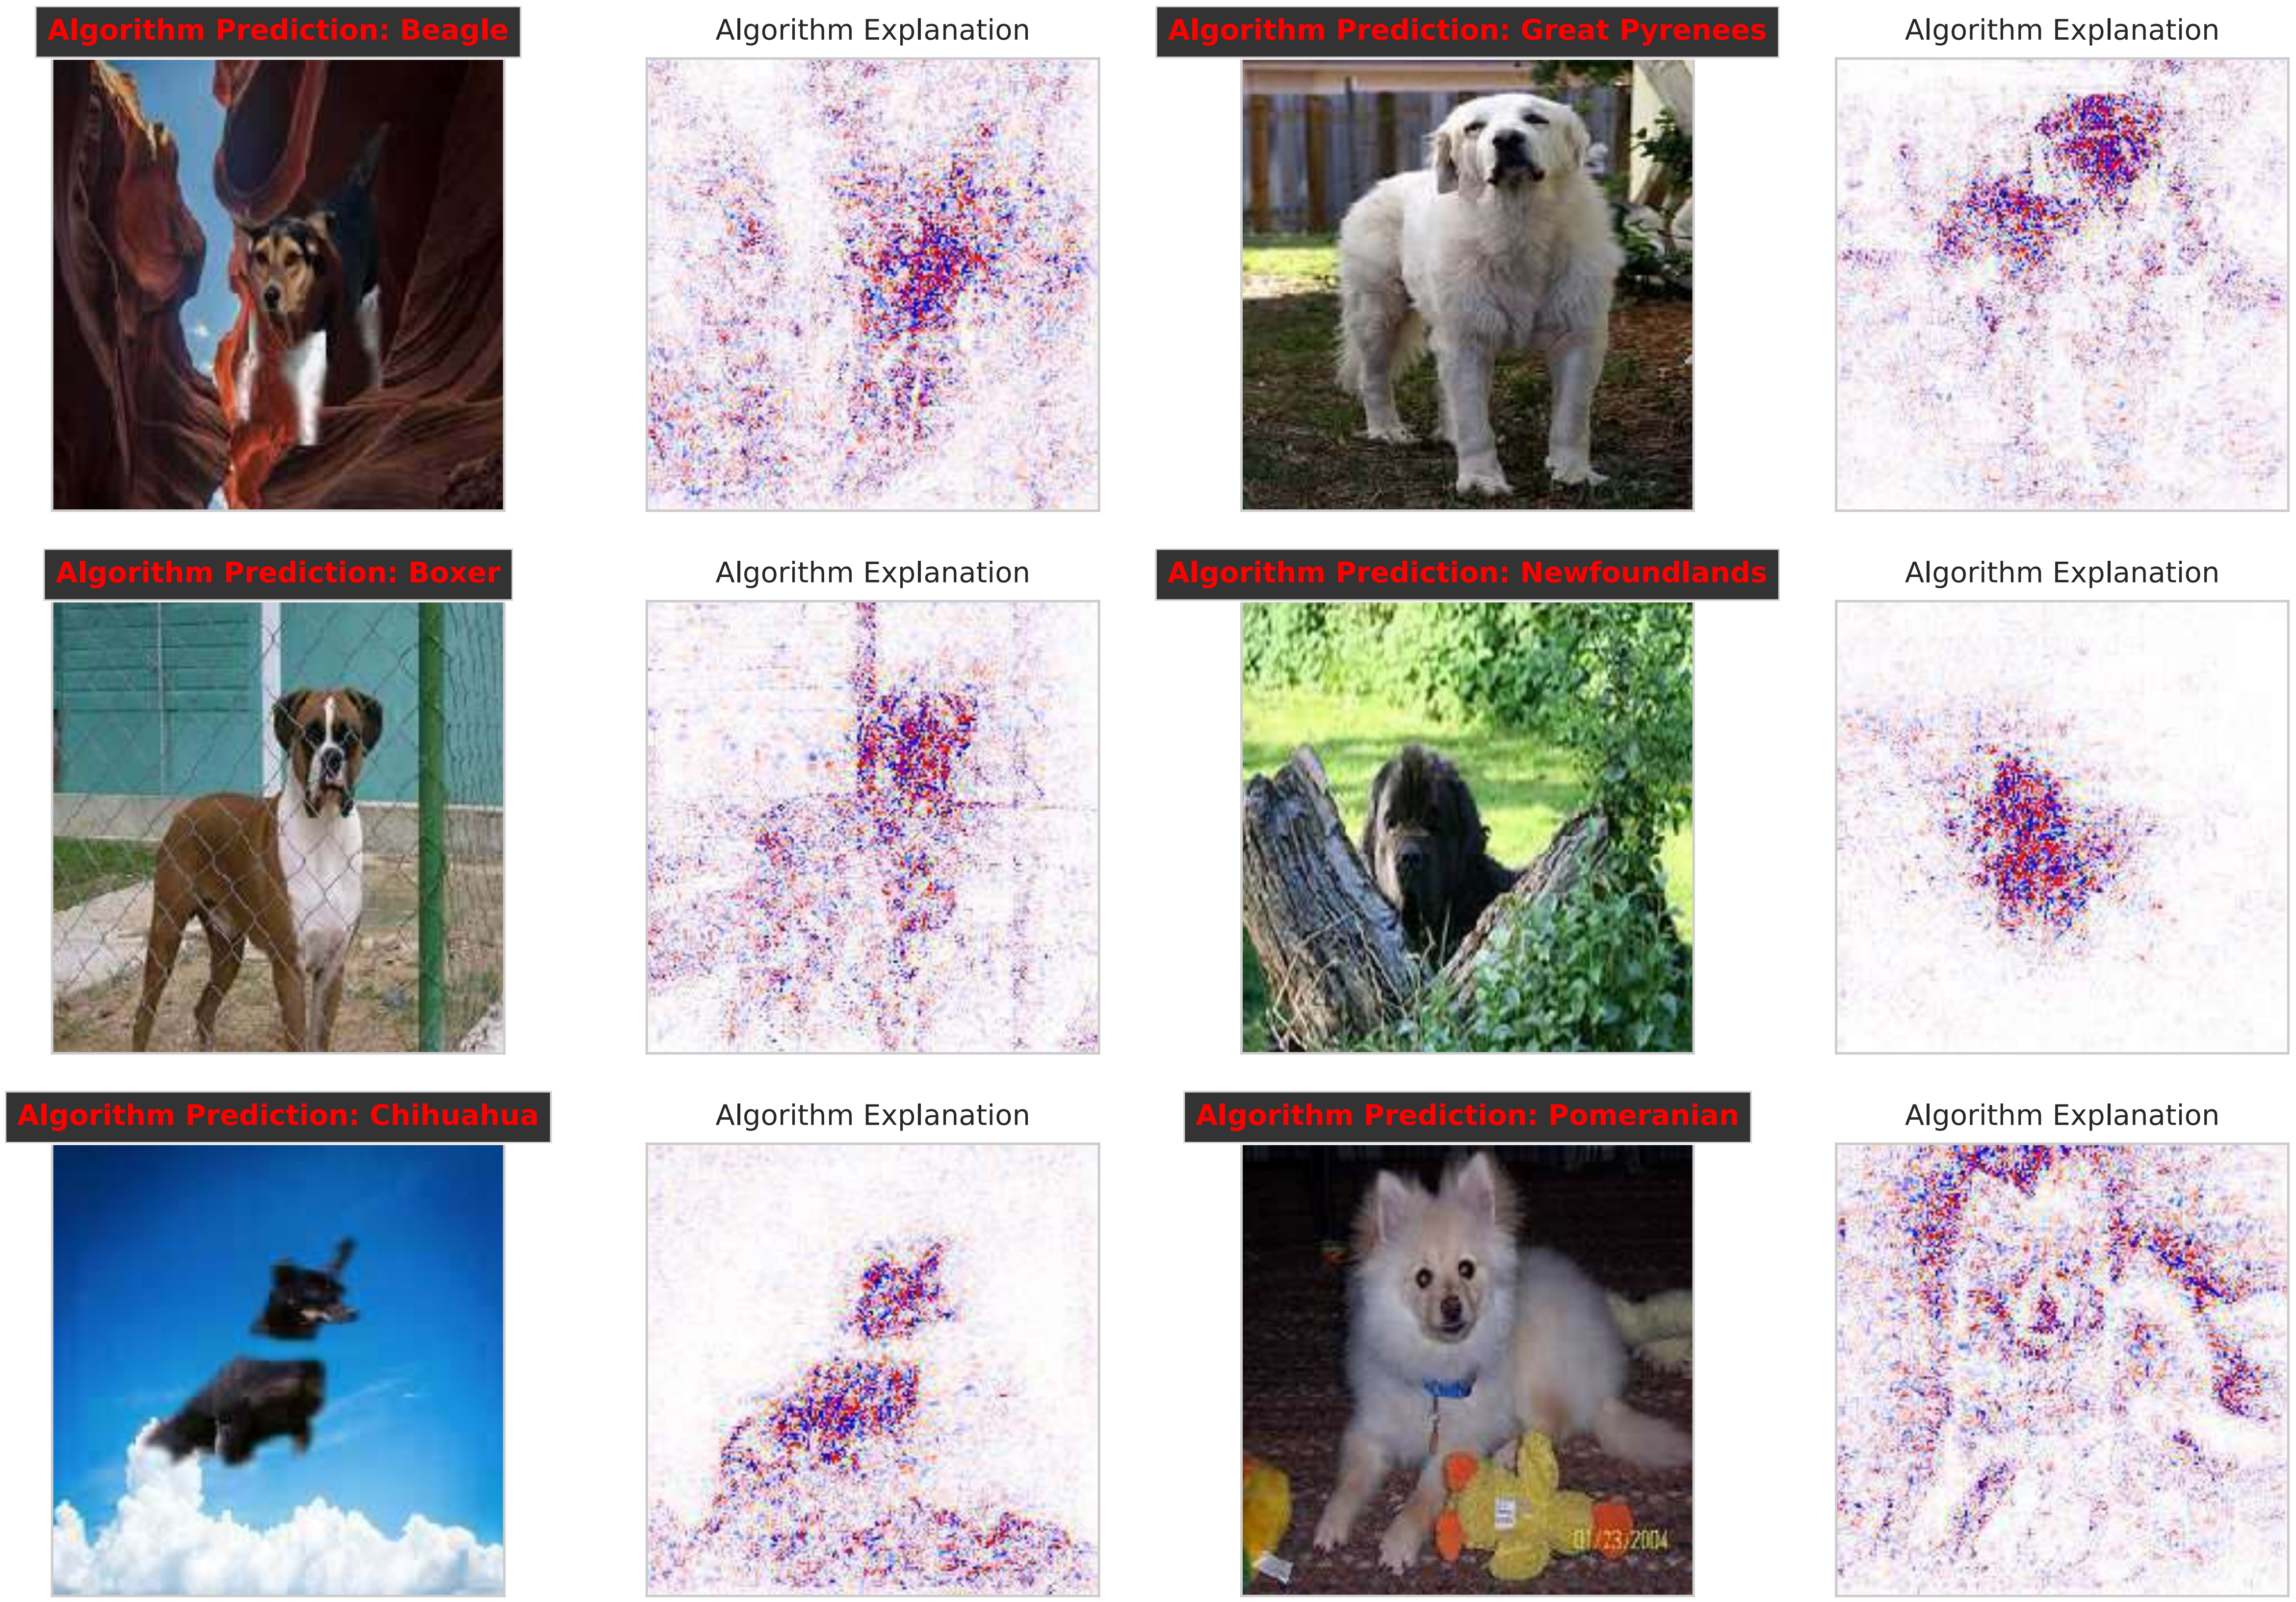

# Out of Distribution : Gradient

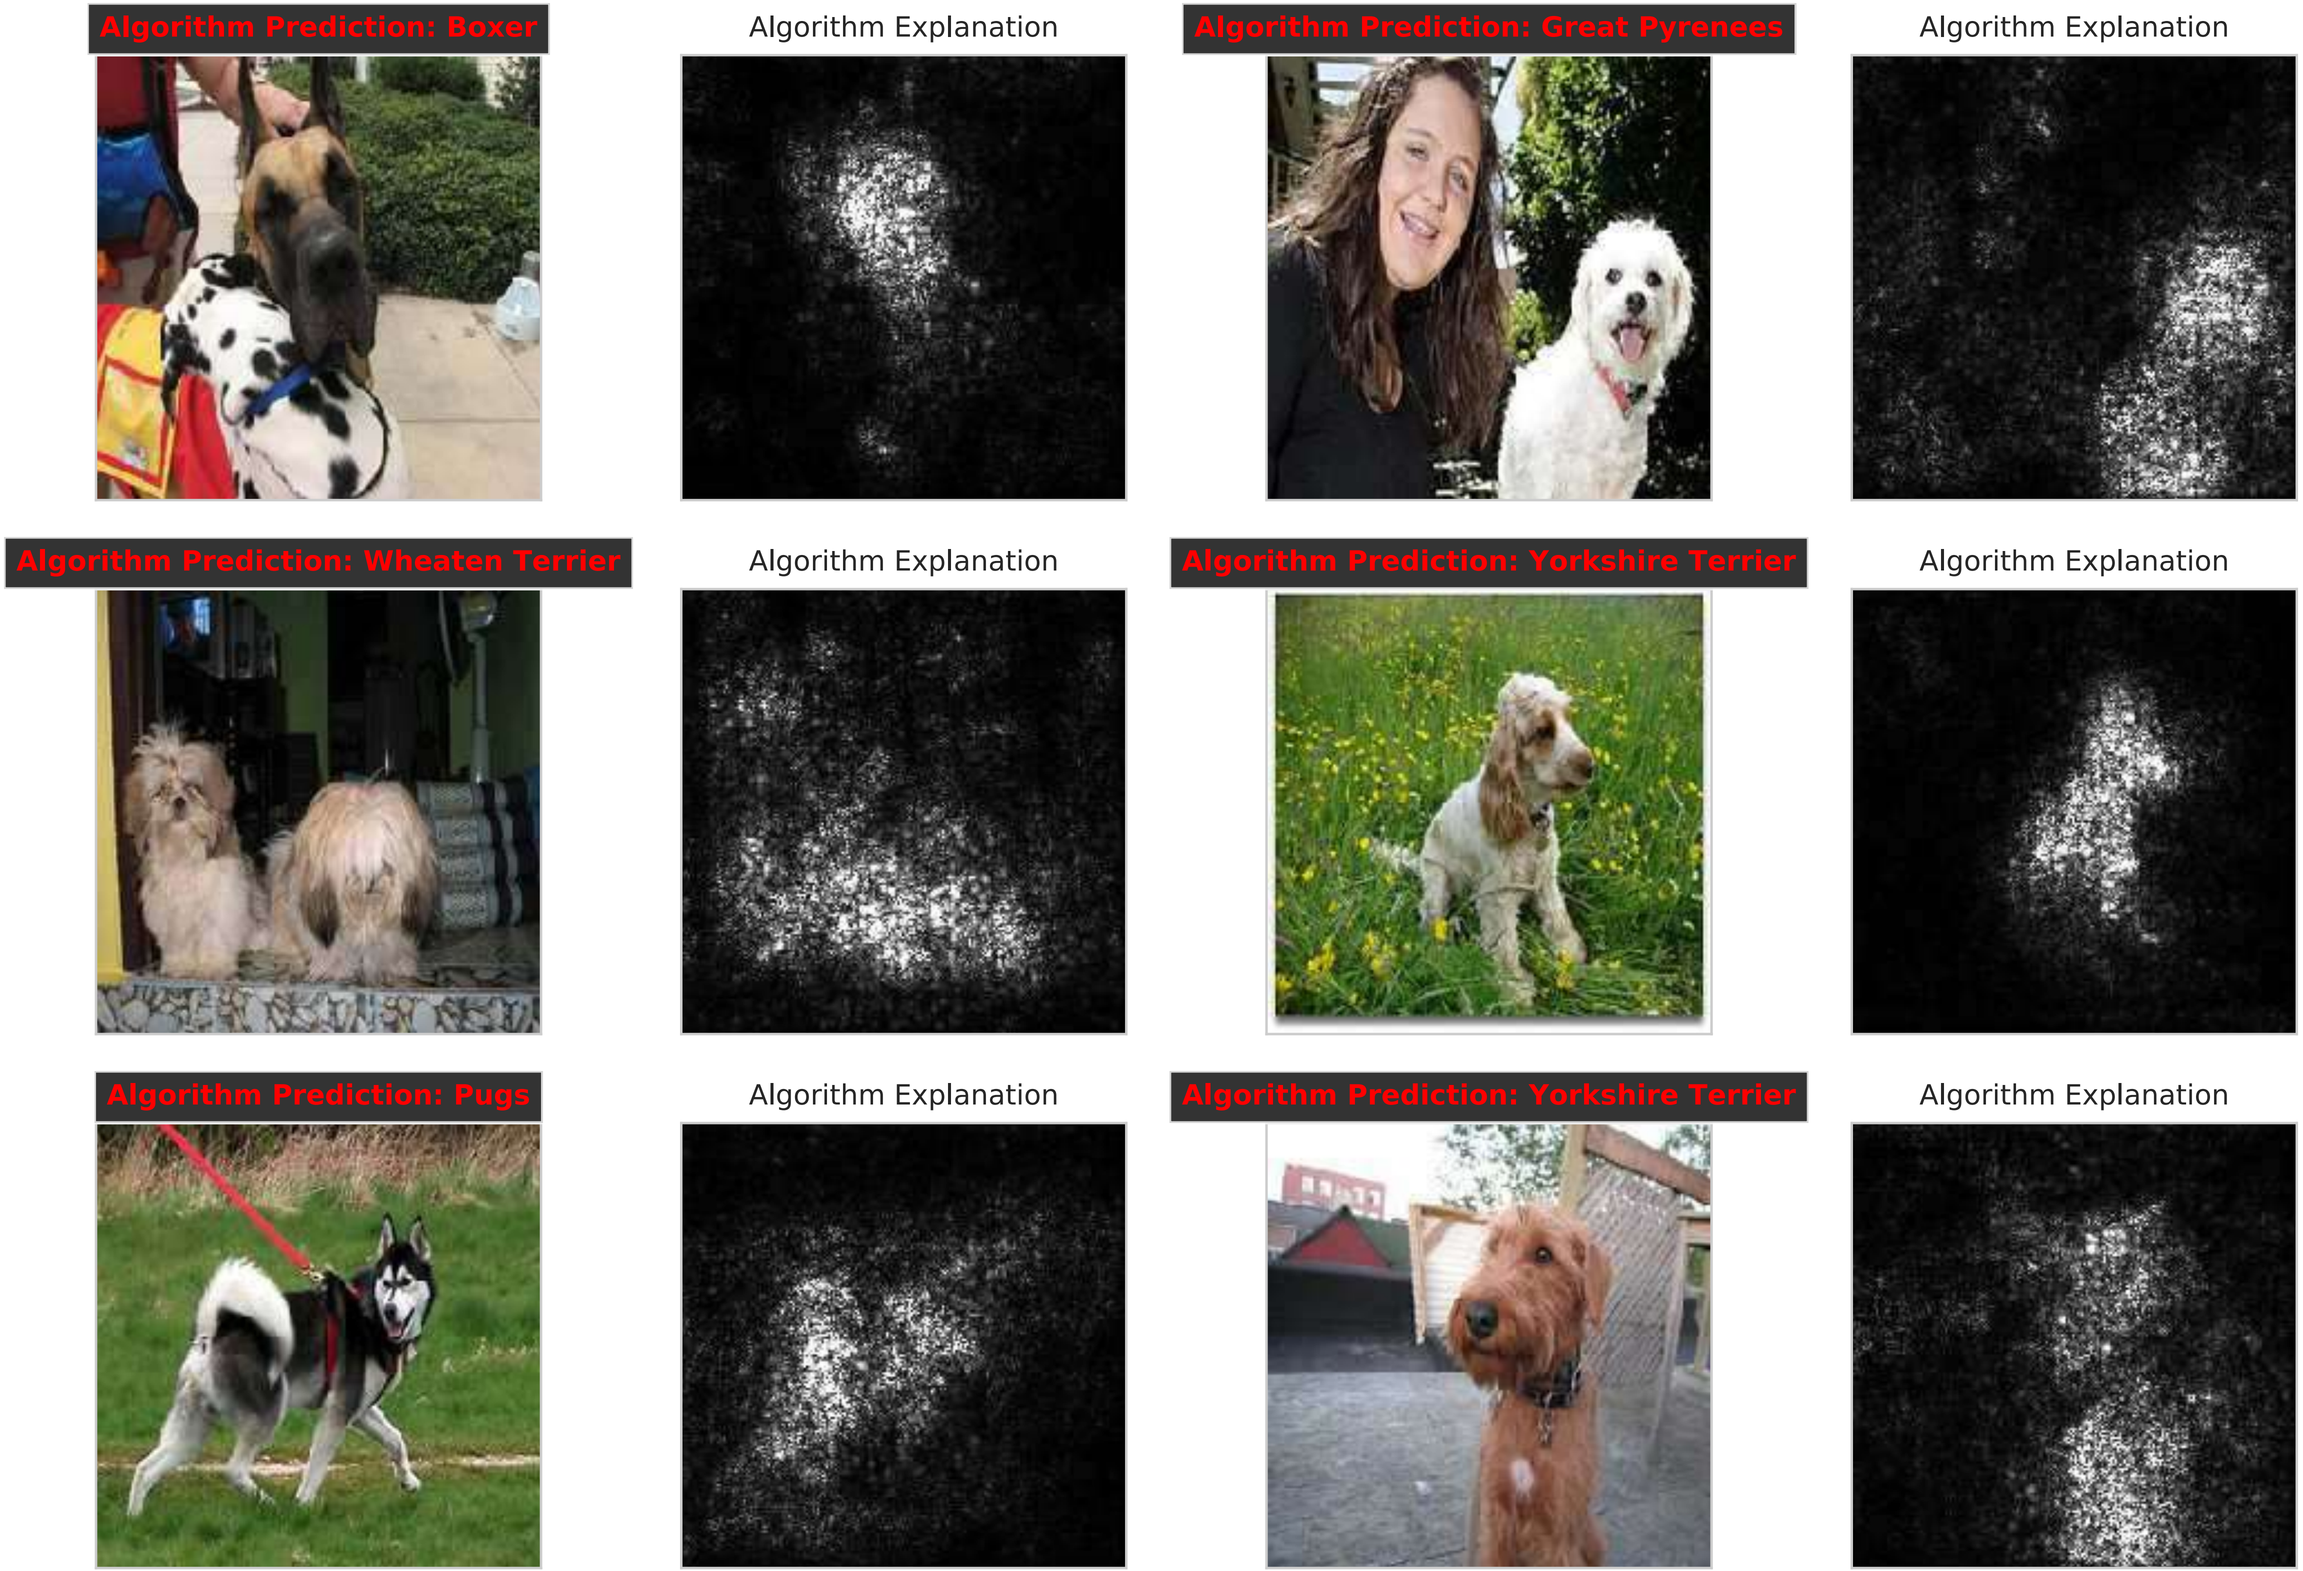

# Out of Distribution: SmoothGrad

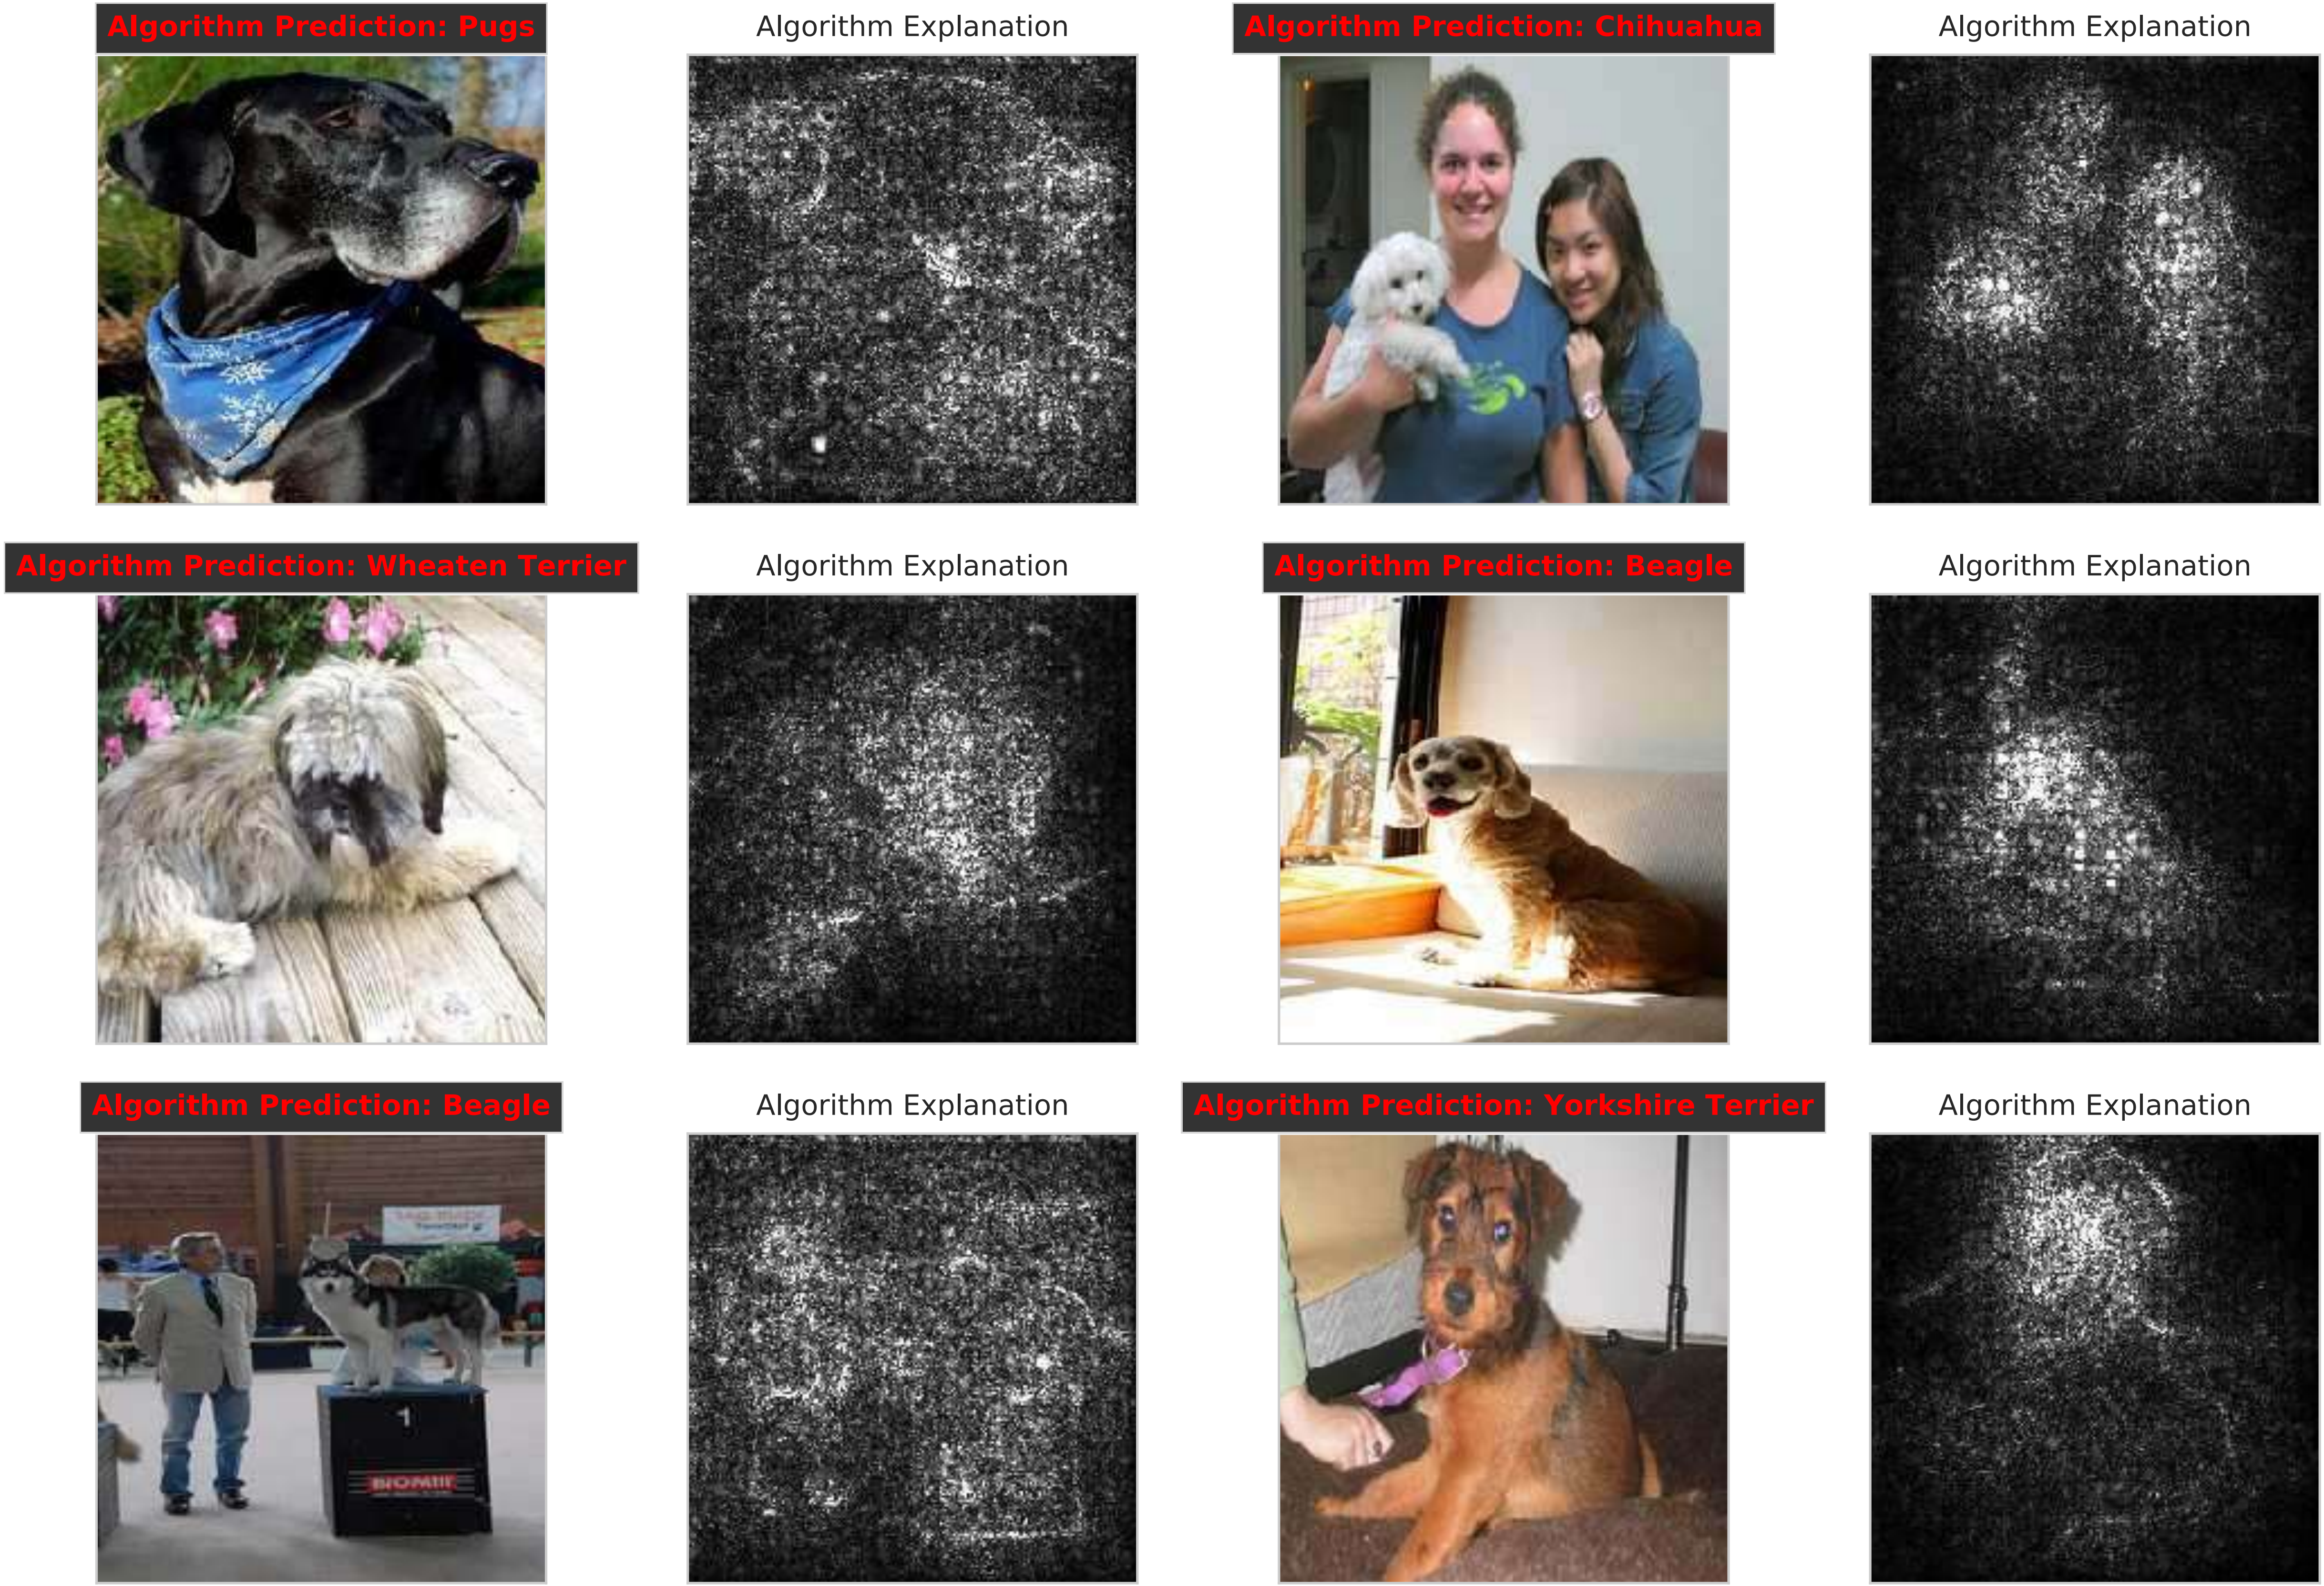

# Out of Distribution: Integrated Gradients

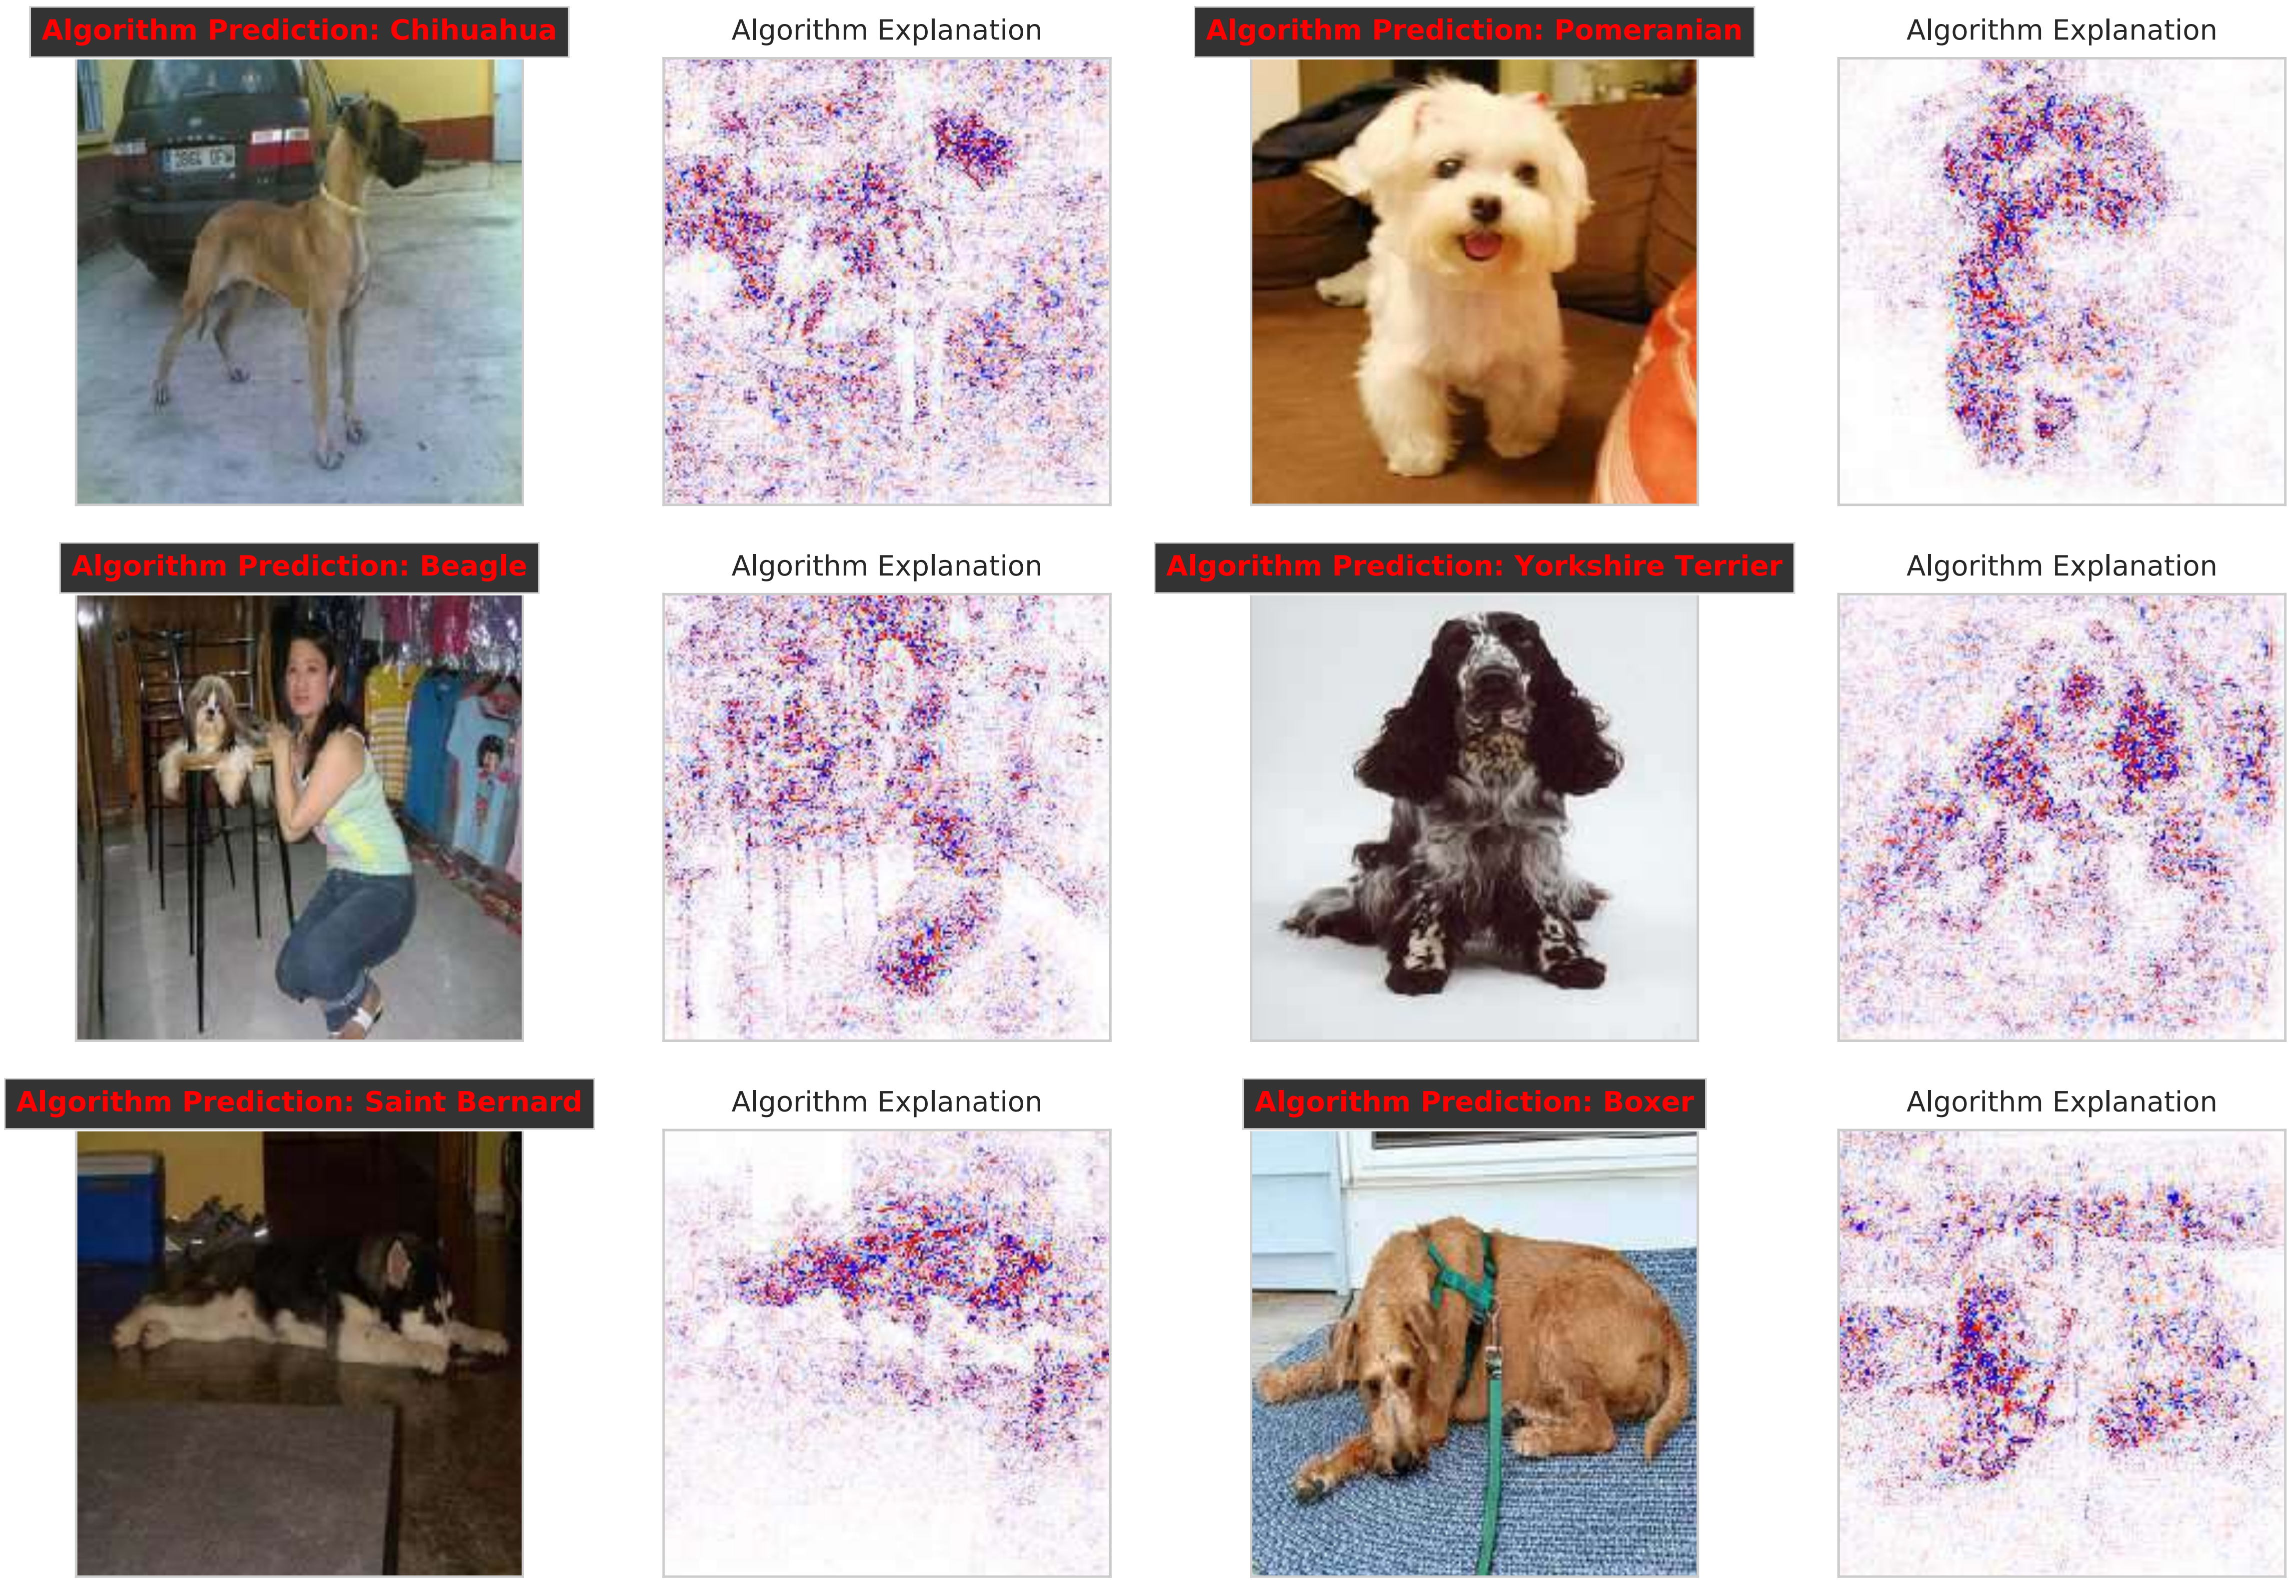

Supplement: Supplementary file 1 [file appendix_v2_compressed.pdf]
